# Supplementary material for: Thermodynamics of firms' growth
Source: arXiv:1504.07666 source file (2015-04-28)
Supplement: Supplementary file 1 [file SI.pdf]

# Supplementary Information: Thermodynamics of firms' growth

Eduardo Zambrano

*Max-Planck-Institut für Physik komplexer Systeme,  
Nöthnitzer Str. 38, 01187 Dresden, Germany*

Alberto Hernando

*SThAR, EPFL Innovation Park, Bâtiment C, 1015 Lausanne, Switzerland  
Laboratory of Theoretical Physical Chemistry,  
Institut des Sciences et Ingénierie Chimiques,  
École Polytechnique Fédérale de Lausanne(EPFL),  
CH-1015 Lausanne, Switzerland*

Aurelio Fernández-Bariviera

*Department of Business, Universitat Rovira i Virgili,  
Av. Universitat 1, 43204 Reus, Spain*

Ricardo Hernando

*SThAR, EPFL Innovation Park, Bâtiment C, 1015 Lausanne, Switzerland*

Angelo Plastino

*National University of La Plata,  
Physics Institute (IFLP-CCT-CONICET) C.C.737, 1900 La Plata, Argentina*

- 
- Details
  - Spain
  - Andalusia
  - Aragon
  - Asturias
  - Balearic islands
  - Basque country
  - Canary islands
  - Cantabria
  - Castile and Leon
  - Castile-La Mancha
  - Catalonia
  - Extremadura
  - Galicia
  - La Rioja
  - Madrid
  - Murcia
  - Navarre
  - Valencian community

# Details

- Positive and negative values of EBITDA were analysed separately.
- EBITDA for two consecutive years were averaged, and the greater year was used as label, e.g. data of 2003 correspond to the period 2002–2003.
- Micro-dynamics model:

$$\dot{x}_i(t) = \overset{\text{proportional growth}}{v_{1,i}x_i(t)} + \overset{\text{finite size noise}}{v_{\frac{1}{2},i}\sqrt{x_i(t)}} + \overset{\text{zero-point}}{v_{0,i}}$$

- Macro-dynamics model for data-fitting:

$$f(x) = T_1x^2 + T_{\frac{1}{2}}x + T_0$$

# Spain

## Tables of Temperatures

### Positive EBITDA

| Year | $T_1$           | $T_{1/2}$          | $T_0$                | $T_{1/2}/T_1$ | Num. Firms |
|------|-----------------|--------------------|----------------------|---------------|------------|
| 2003 | $0.57 \pm 0.11$ | $60.52 \pm 14.56$  | $528.40 \pm 193.19$  | 105.3         | 415865     |
| 2004 | $0.64 \pm 0.09$ | $47.87 \pm 12.14$  | $664.95 \pm 184.10$  | 74.5          | 428486     |
| 2005 | $0.62 \pm 0.10$ | $67.16 \pm 12.35$  | $837.13 \pm 159.74$  | 109.1         | 449524     |
| 2006 | $0.67 \pm 0.06$ | $74.79 \pm 9.29$   | $965.96 \pm 148.94$  | 112.0         | 470854     |
| 2007 | $0.78 \pm 0.15$ | $78.21 \pm 19.91$  | $981.09 \pm 221.10$  | 100.7         | 485222     |
| 2008 | $1.14 \pm 0.14$ | $114.96 \pm 17.80$ | $1298.55 \pm 213.37$ | 100.4         | 432543     |
| 2009 | $1.27 \pm 0.19$ | $139.21 \pm 20.18$ | $1066.93 \pm 189.10$ | 109.7         | 461783     |
| 2010 | $0.90 \pm 0.21$ | $117.83 \pm 21.63$ | $902.29 \pm 252.06$  | 131.0         | 464758     |
| 2011 | $1.10 \pm 0.14$ | $109.10 \pm 14.90$ | $1088.83 \pm 176.94$ | 99.5          | 422307     |
| 2012 | $0.92 \pm 0.13$ | $71.81 \pm 12.24$  | $604.28 \pm 136.09$  | 78.5          | 230209     |

### Negative EBITDA

| Year | $T_1$           | $T_{1/2}$           | $T_0$                | $T_{1/2}/T_1$ | Num. Firms |
|------|-----------------|---------------------|----------------------|---------------|------------|
| 2003 | $2.86 \pm 0.59$ | $244.52 \pm 33.23$  | $418.37 \pm 162.48$  | 85.4          | 103152     |
| 2004 | $2.78 \pm 0.47$ | $251.65 \pm 28.76$  | $493.50 \pm 152.97$  | 90.7          | 104869     |
| 2005 | $2.35 \pm 0.46$ | $205.63 \pm 27.35$  | $1018.63 \pm 165.08$ | 87.4          | 111046     |
| 2006 | $2.93 \pm 0.49$ | $228.14 \pm 31.66$  | $814.21 \pm 198.22$  | 77.8          | 117356     |
| 2007 | $3.48 \pm 1.17$ | $438.48 \pm 70.09$  | $359.78 \pm 243.03$  | 125.9         | 112675     |
| 2008 | $5.96 \pm 2.08$ | $538.87 \pm 127.37$ | $895.34 \pm 424.41$  | 90.4          | 109301     |
| 2009 | $6.06 \pm 0.91$ | $245.91 \pm 54.91$  | $1470.71 \pm 461.58$ | 40.6          | 171427     |
| 2010 | $5.19 \pm 0.90$ | $205.09 \pm 44.79$  | $917.49 \pm 269.41$  | 39.5          | 196737     |
| 2011 | $5.14 \pm 0.63$ | $257.43 \pm 31.94$  | $877.67 \pm 169.99$  | 50.1          | 187046     |
| 2012 | $2.73 \pm 0.48$ | $154.07 \pm 26.79$  | $1024.32 \pm 181.77$ | 56.3          | 108898     |

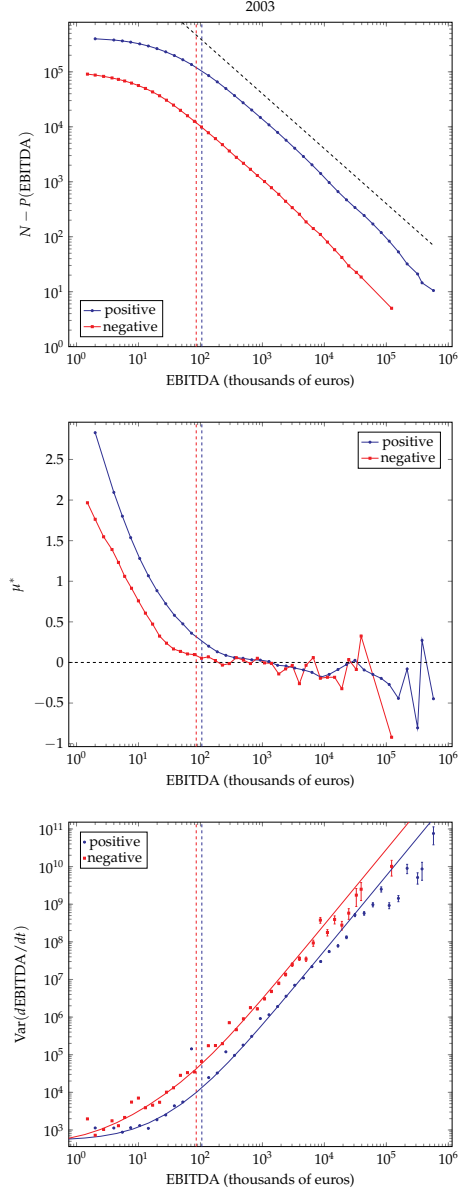

Figure 1: Spain

Rank plot, chemical potential and variance.

415865 Firms with positive EBITDA

$T_1 = 0.57 \pm 0.11$ ,  $T_{1/2} = 60.52 \pm 14.56$ , and  $T_0 = 528.40 \pm 193.19$

103152 Firms with negative EBITDA

Negative EBITDA:

$T_1 = 2.86 \pm 0.59$ ,  $T_{1/2} = 244.52 \pm 33.23$ , and  $T_0 = 418.37 \pm 162.48$ .

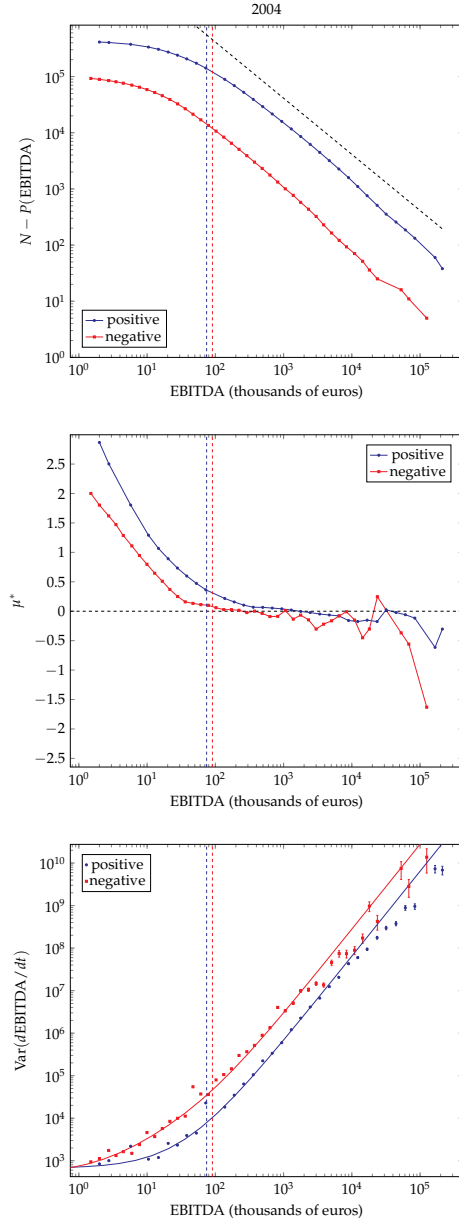

Figure 2: Spain

Rank plot, chemical potential and variance.

428486 Firms with positive EBITDA

$T_1 = 0.64 \pm 0.09$ ,  $T_{1/2} = 47.87 \pm 12.14$ , and  $T_0 = 664.95 \pm 184.10$

104869 Firms with negative EBITDA

Negative EBITDA:

$T_1 = 2.78 \pm 0.47$ ,  $T_{1/2} = 251.65 \pm 28.76$ , and  $T_0 = 493.50 \pm 152.97$ .

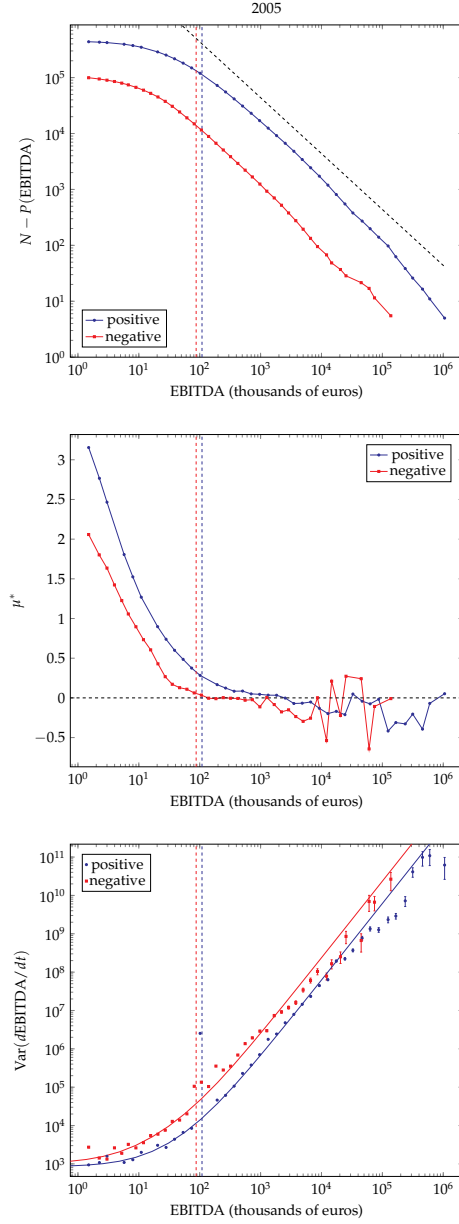

Figure 3: Spain

Rank plot, chemical potential and variance.

449524 Firms with positive EBITDA

$T_1 = 0.62 \pm 0.10$ ,  $T_{1/2} = 67.16 \pm 12.35$ , and  $T_0 = 837.13 \pm 159.74$

111046 Firms with negative EBITDA

Negative EBITDA:

$T_1 = 2.35 \pm 0.46$ ,  $T_{1/2} = 205.63 \pm 27.35$ , and  $T_0 = 1018.63 \pm 165.08$ .

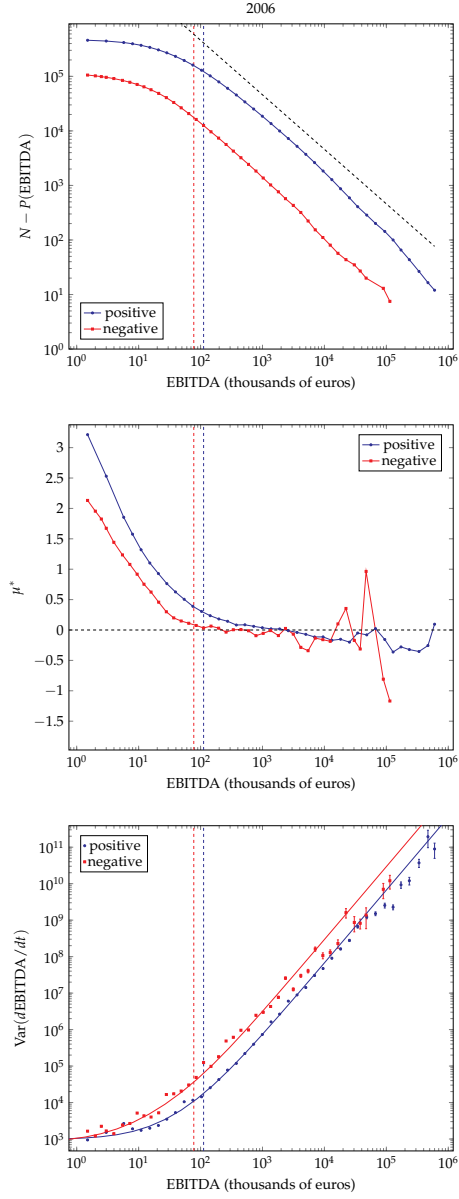

Figure 4: Spain

Rank plot, chemical potential and variance.

470854 Firms with positive EBITDA

$T_1 = 0.67 \pm 0.06$ ,  $T_{1/2} = 74.79 \pm 9.29$ , and  $T_0 = 965.96 \pm 148.94$

117356 Firms with negative EBITDA

Negative EBITDA:

$T_1 = 2.93 \pm 0.49$ ,  $T_{1/2} = 228.14 \pm 31.66$ , and  $T_0 = 814.21 \pm 198.22$ .

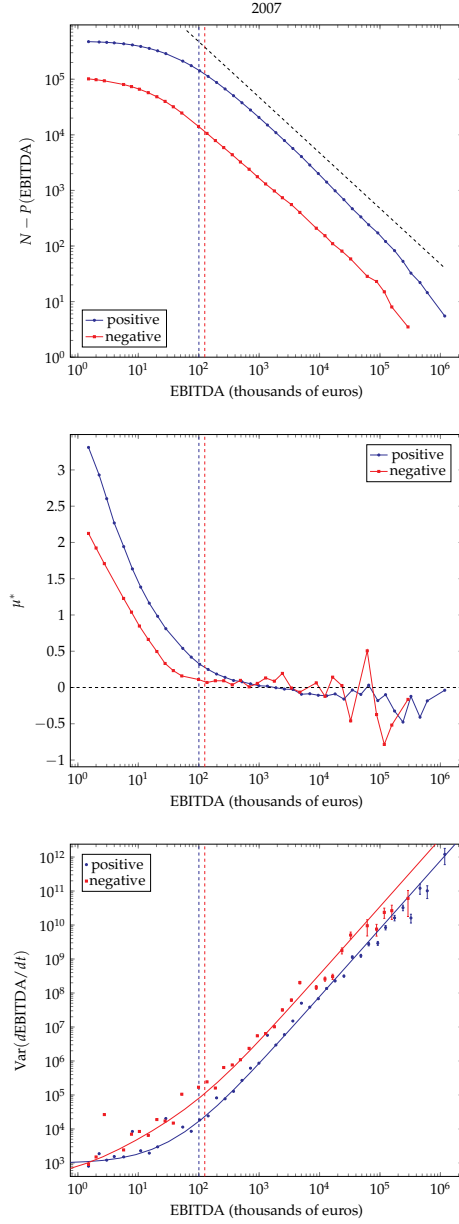

Figure 5: Spain

Rank plot, chemical potential and variance.

485222 Firms with positive EBITDA

$T_1 = 0.78 \pm 0.15$ ,  $T_{1/2} = 78.21 \pm 19.91$ , and  $T_0 = 981.09 \pm 221.10$

112675 Firms with negative EBITDA

Negative EBITDA:

$T_1 = 3.48 \pm 1.17$ ,  $T_{1/2} = 438.48 \pm 70.09$ , and  $T_0 = 359.78 \pm 243.03$ .

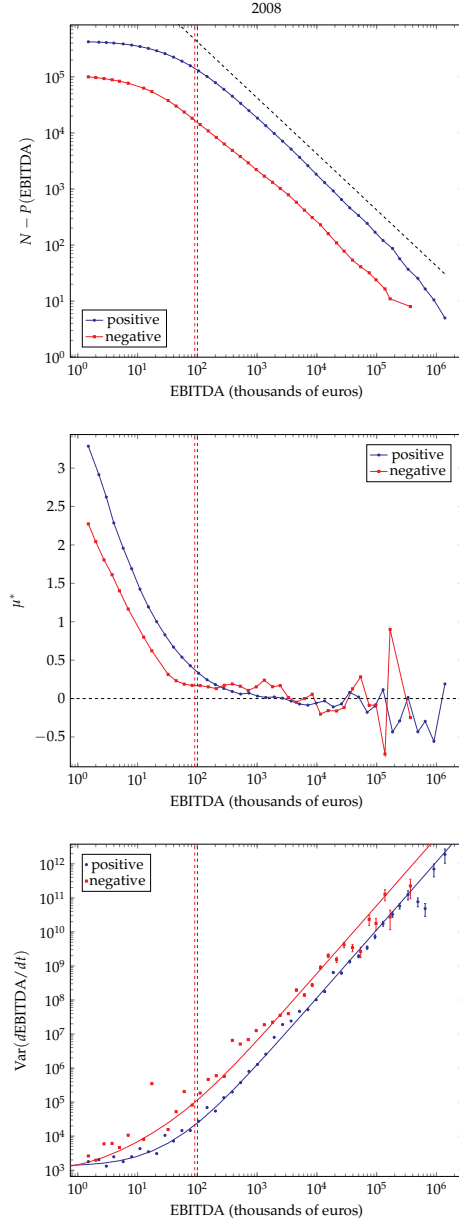

Figure 6: Spain

Rank plot, chemical potential and variance.

432543 Firms with positive EBITDA

$T_1 = 1.14 \pm 0.14$ ,  $T_{1/2} = 114.96 \pm 17.80$ , and  $T_0 = 1298.55 \pm 213.37$

109301 Firms with negative EBITDA

Negative EBITDA:

$T_1 = 5.96 \pm 2.08$ ,  $T_{1/2} = 538.87 \pm 127.37$ , and  $T_0 = 895.34 \pm 424.41$ .

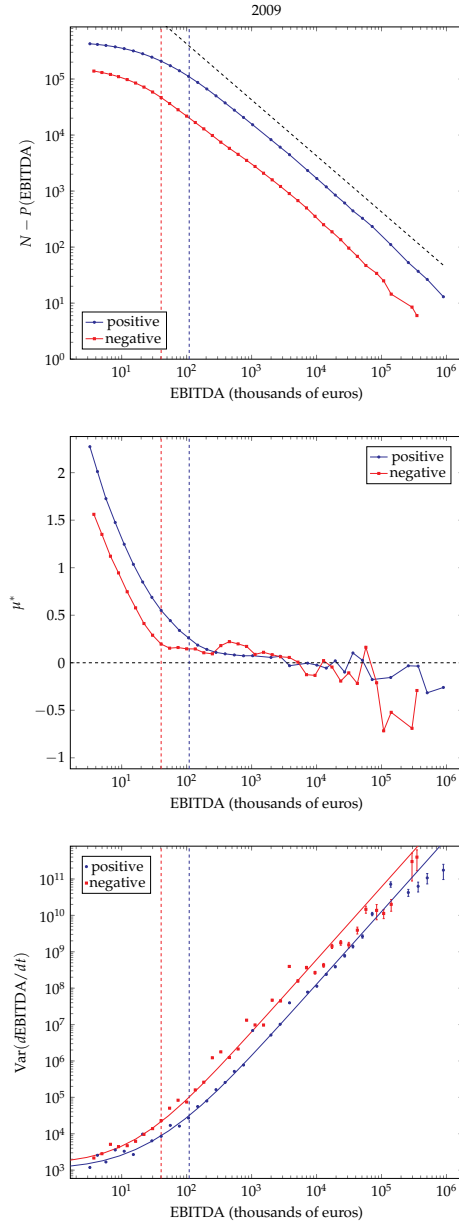

Figure 7: Spain

Rank plot, chemical potential and variance.

461783 Firms with positive EBITDA

$T_1 = 1.27 \pm 0.19$ ,  $T_{1/2} = 139.21 \pm 20.18$ , and  $T_0 = 1066.93 \pm 189.10$

171427 Firms with negative EBITDA

Negative EBITDA:

$T_1 = 6.06 \pm 0.91$ ,  $T_{1/2} = 245.91 \pm 54.91$ , and  $T_0 = 1470.71 \pm 461.58$ .

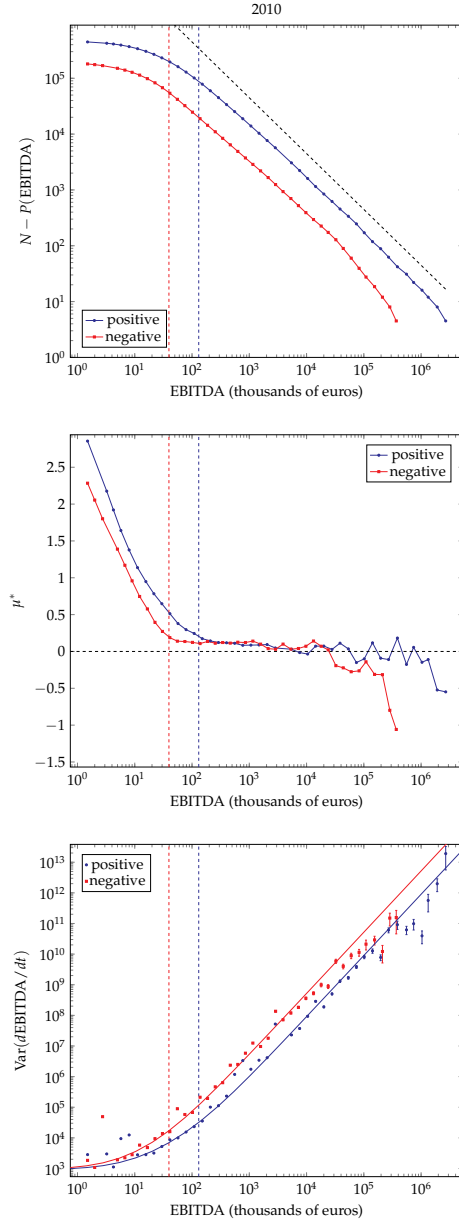

Figure 8: Spain

Rank plot, chemical potential and variance.

464758 Firms with positive EBITDA

$T_1 = 0.90 \pm 0.21$ ,  $T_{1/2} = 117.83 \pm 21.63$ , and  $T_0 = 902.29 \pm 252.06$

196737 Firms with negative EBITDA

Negative EBITDA:

$T_1 = 5.19 \pm 0.90$ ,  $T_{1/2} = 205.09 \pm 44.79$ , and  $T_0 = 917.49 \pm 269.41$ .

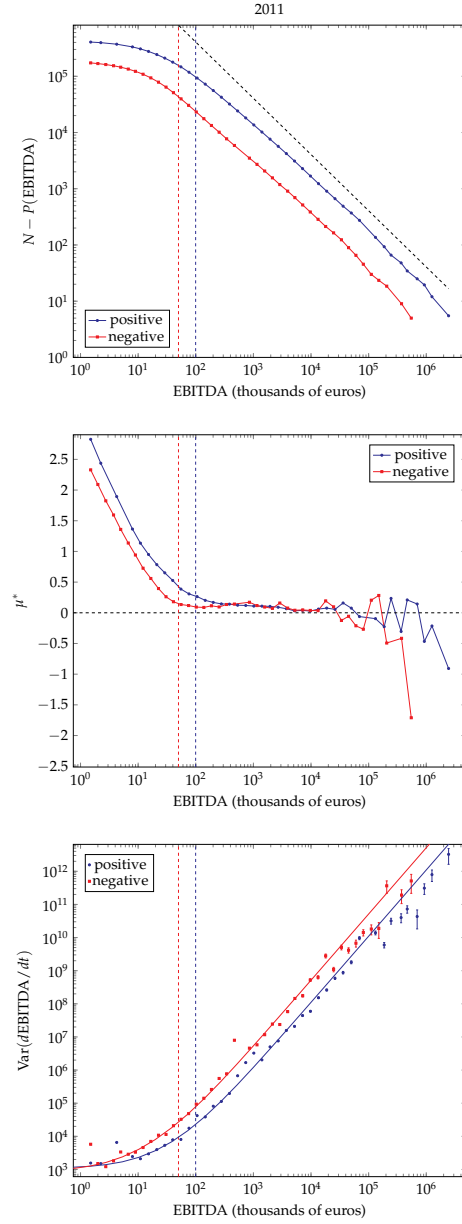

Figure 9: Spain

Rank plot, chemical potential and variance.

422307 Firms with positive EBITDA

$T_1 = 1.10 \pm 0.14$ ,  $T_{1/2} = 109.10 \pm 14.90$ , and  $T_0 = 1088.83 \pm 176.94$

187046 Firms with negative EBITDA

Negative EBITDA:

$T_1 = 5.14 \pm 0.63$ ,  $T_{1/2} = 257.43 \pm 31.94$ , and  $T_0 = 877.67 \pm 169.99$ .

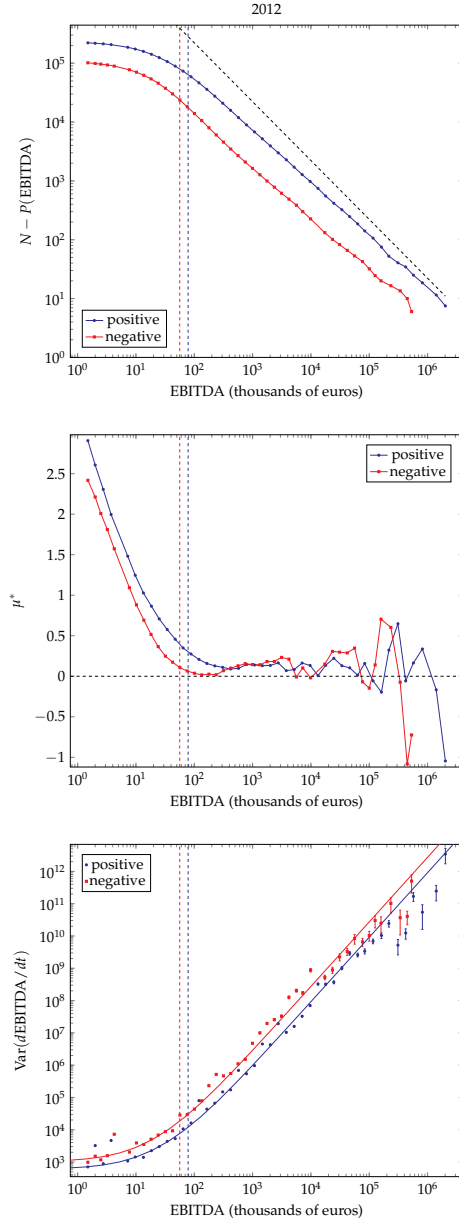

Figure 10: Spain

Rank plot, chemical potential and variance.

230209 Firms with positive EBITDA

$T_1 = 0.92 \pm 0.13$ ,  $T_{1/2} = 71.81 \pm 12.24$ , and  $T_0 = 604.28 \pm 136.09$

108898 Firms with negative EBITDA

Negative EBITDA:

$T_1 = 2.73 \pm 0.48$ ,  $T_{1/2} = 154.07 \pm 26.79$ , and  $T_0 = 1024.32 \pm 181.77$ .

# Andalusia

## Tables of Temperatures

### Positive EBITDA

| Year | $T_1$           | $T_{1/2}$         | $T_0$                | $T_{1/2}/T_1$ | Num. Firms |
|------|-----------------|-------------------|----------------------|---------------|------------|
| 2003 | $0.75 \pm 0.11$ | $47.92 \pm 9.76$  | $365.87 \pm 89.53$   | 63.5          | 48702      |
| 2004 | $0.68 \pm 0.11$ | $41.67 \pm 9.87$  | $347.72 \pm 86.56$   | 61.2          | 50132      |
| 2005 | $0.55 \pm 0.11$ | $71.89 \pm 11.65$ | $473.14 \pm 109.46$  | 130.3         | 53351      |
| 2006 | $0.64 \pm 0.15$ | $60.90 \pm 18.34$ | $523.16 \pm 170.33$  | 94.5          | 57098      |
| 2007 | $0.71 \pm 0.14$ | $70.22 \pm 15.51$ | $465.95 \pm 149.32$  | 98.3          | 56310      |
| 2008 | $0.90 \pm 0.13$ | $80.71 \pm 14.90$ | $1112.61 \pm 194.42$ | 89.4          | 49271      |
| 2009 | $0.81 \pm 0.13$ | $92.21 \pm 12.83$ | $581.93 \pm 116.96$  | 114.2         | 56793      |
| 2010 | $0.74 \pm 0.14$ | $65.50 \pm 14.36$ | $671.42 \pm 147.02$  | 88.3          | 56713      |
| 2011 | $0.54 \pm 0.11$ | $68.79 \pm 11.26$ | $578.03 \pm 115.85$  | 126.4         | 52600      |
| 2012 | $0.58 \pm 0.13$ | $69.37 \pm 12.20$ | $353.90 \pm 105.19$  | 119.6         | 31522      |

### Negative EBITDA

| Year | $T_1$           | $T_{1/2}$          | $T_0$                | $T_{1/2}/T_1$ | Num. Firms |
|------|-----------------|--------------------|----------------------|---------------|------------|
| 2003 | $1.81 \pm 0.48$ | $179.90 \pm 29.43$ | $388.65 \pm 181.23$  | 99.6          | 12308      |
| 2004 | $1.62 \pm 0.57$ | $204.40 \pm 32.97$ | $268.71 \pm 158.64$  | 126.5         | 12268      |
| 2005 | $2.78 \pm 0.66$ | $141.41 \pm 40.98$ | $612.31 \pm 352.75$  | 50.8          | 13240      |
| 2006 | $2.10 \pm 0.81$ | $274.67 \pm 57.58$ | $127.01 \pm 210.29$  | 131.0         | 14507      |
| 2007 | $1.81 \pm 0.67$ | $401.30 \pm 48.20$ | $275.53 \pm 183.50$  | 222.1         | 12919      |
| 2008 | $3.06 \pm 0.82$ | $231.00 \pm 57.49$ | $1484.42 \pm 526.15$ | 75.4          | 12536      |
| 2009 | $3.56 \pm 0.56$ | $140.35 \pm 27.37$ | $986.86 \pm 170.60$  | 39.5          | 21368      |
| 2010 | $3.59 \pm 0.78$ | $39.87 \pm 47.45$  | $1843.44 \pm 442.97$ | 11.1          | 23996      |
| 2011 | $2.73 \pm 0.59$ | $123.42 \pm 28.33$ | $500.04 \pm 148.92$  | 45.2          | 24364      |
| 2012 | $2.57 \pm 0.66$ | $115.02 \pm 37.43$ | $951.08 \pm 273.09$  | 44.7          | 15335      |

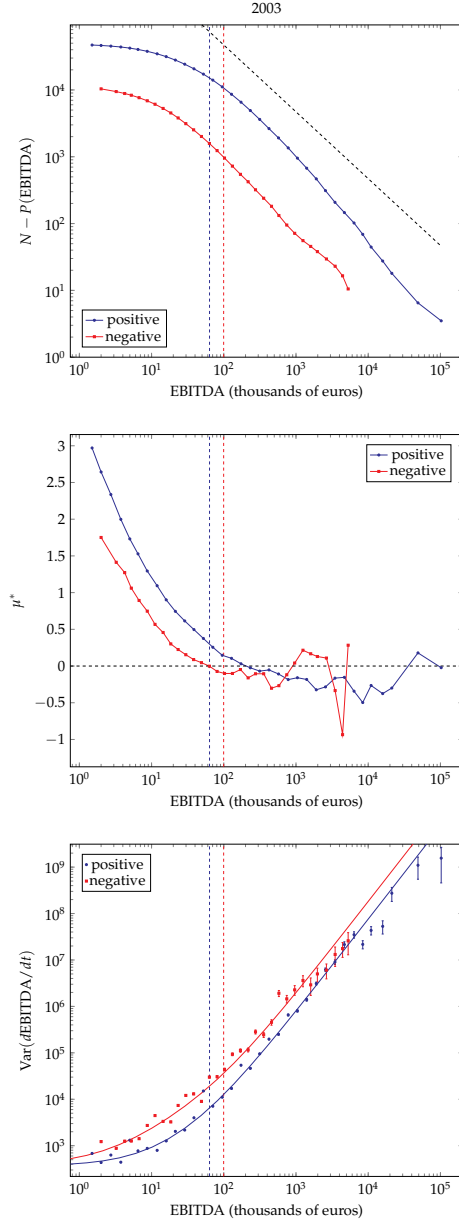

Figure 11: Andalusia

Rank plot, chemical potential and variance.

48702 Firms with positive EBITDA

$T_1 = 0.75 \pm 0.11$ ,  $T_{1/2} = 47.92 \pm 9.76$ , and  $T_0 = 365.87 \pm 89.53$

12308 Firms with negative EBITDA

Negative EBITDA:

$T_1 = 1.81 \pm 0.48$ ,  $T_{1/2} = 179.90 \pm 29.43$ , and  $T_0 = 388.65 \pm 181.23$ .

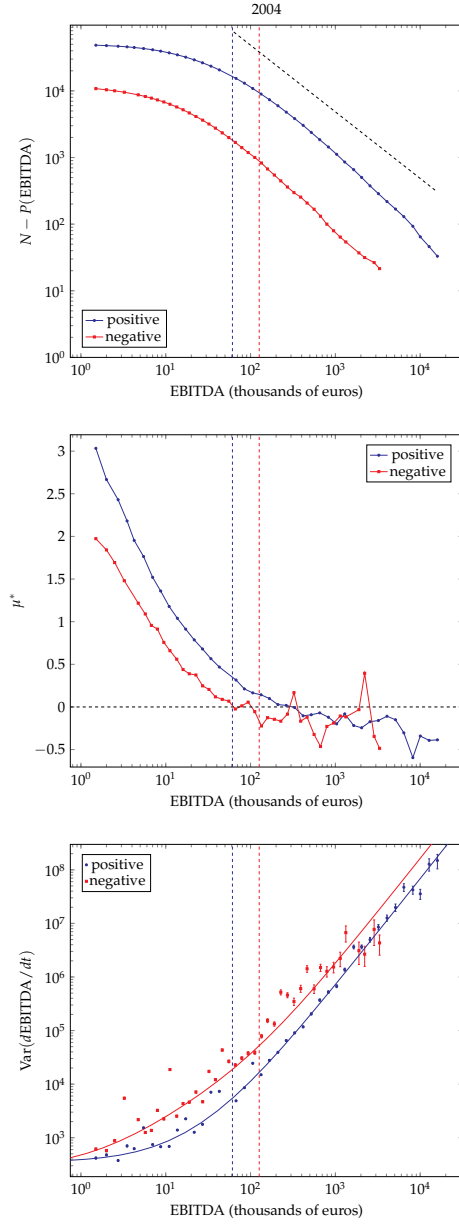

Figure 12: Andalusia

Rank plot, chemical potential and variance.

50132 Firms with positive EBITDA

$T_1 = 0.68 \pm 0.11$ ,  $T_{1/2} = 41.67 \pm 9.87$ , and  $T_0 = 347.72 \pm 86.56$

12268 Firms with negative EBITDA

Negative EBITDA:

$T_1 = 1.62 \pm 0.57$ ,  $T_{1/2} = 204.40 \pm 32.97$ , and  $T_0 = 268.71 \pm 158.64$ .

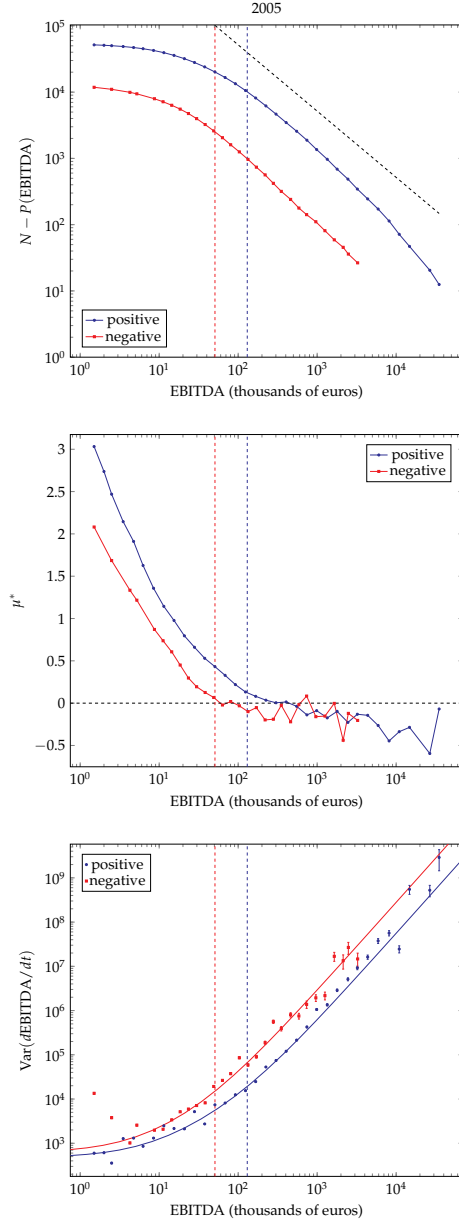

Figure 13: Andalusia

Rank plot, chemical potential and variance.

53351 Firms with positive EBITDA

$T_1 = 0.55 \pm 0.11$ ,  $T_{1/2} = 71.89 \pm 11.65$ , and  $T_0 = 473.14 \pm 109.46$

13240 Firms with negative EBITDA

Negative EBITDA:

$T_1 = 2.78 \pm 0.66$ ,  $T_{1/2} = 141.41 \pm 40.98$ , and  $T_0 = 612.31 \pm 352.75$ .

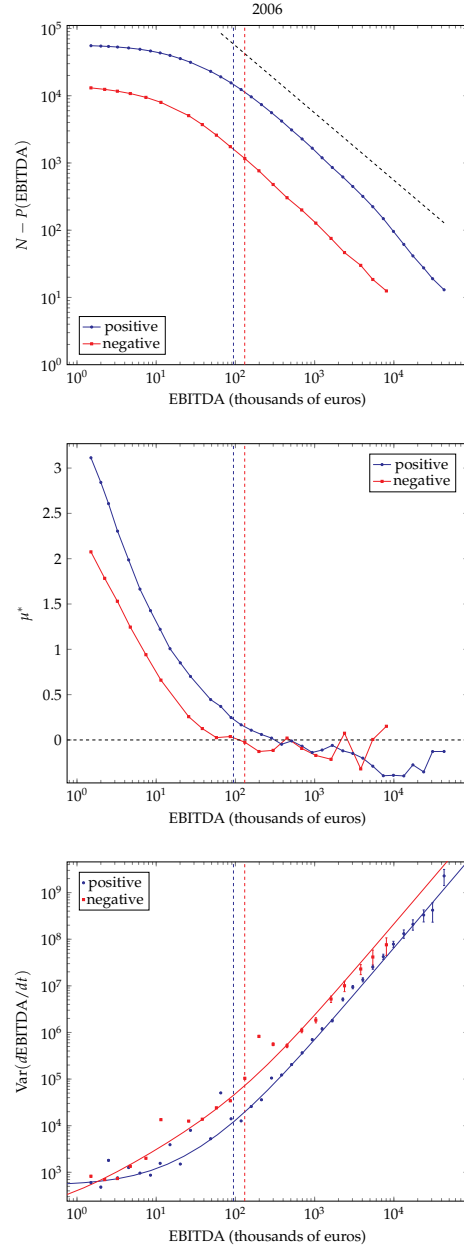

Figure 14: Andalusia

Rank plot, chemical potential and variance.

57098 Firms with positive EBITDA

$T_1 = 0.64 \pm 0.15$ ,  $T_{1/2} = 60.90 \pm 18.34$ , and  $T_0 = 523.16 \pm 170.33$

14507 Firms with negative EBITDA

Negative EBITDA:

$T_1 = 2.10 \pm 0.81$ ,  $T_{1/2} = 274.67 \pm 57.58$ , and  $T_0 = 127.01 \pm 210.29$ .

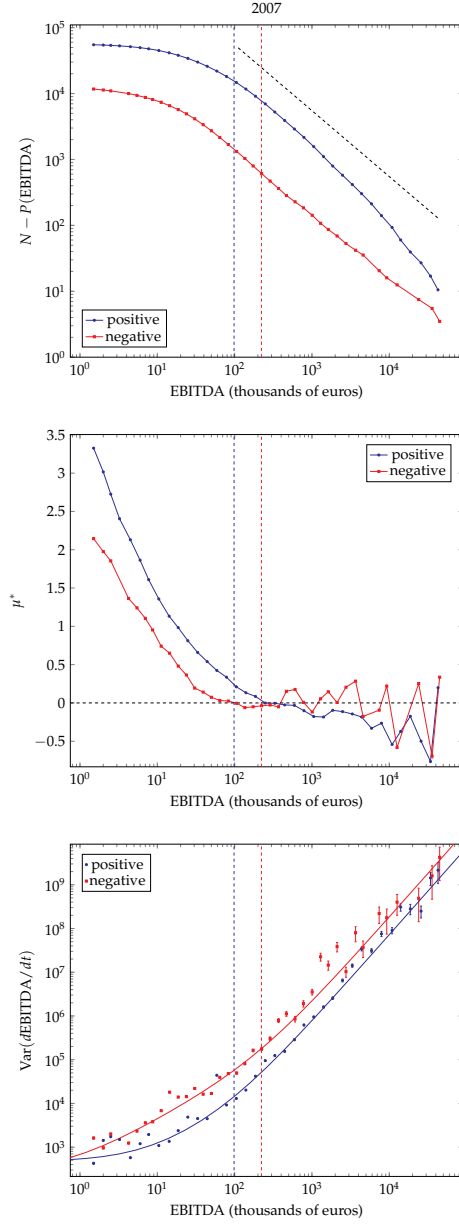

Figure 15: Andalusia

Rank plot, chemical potential and variance.

56310 Firms with positive EBITDA

$T_1 = 0.71 \pm 0.14$ ,  $T_{1/2} = 70.22 \pm 15.51$ , and  $T_0 = 465.95 \pm 149.32$

12919 Firms with negative EBITDA

Negative EBITDA:

$T_1 = 1.81 \pm 0.67$ ,  $T_{1/2} = 401.30 \pm 48.20$ , and  $T_0 = 275.53 \pm 183.50$ .

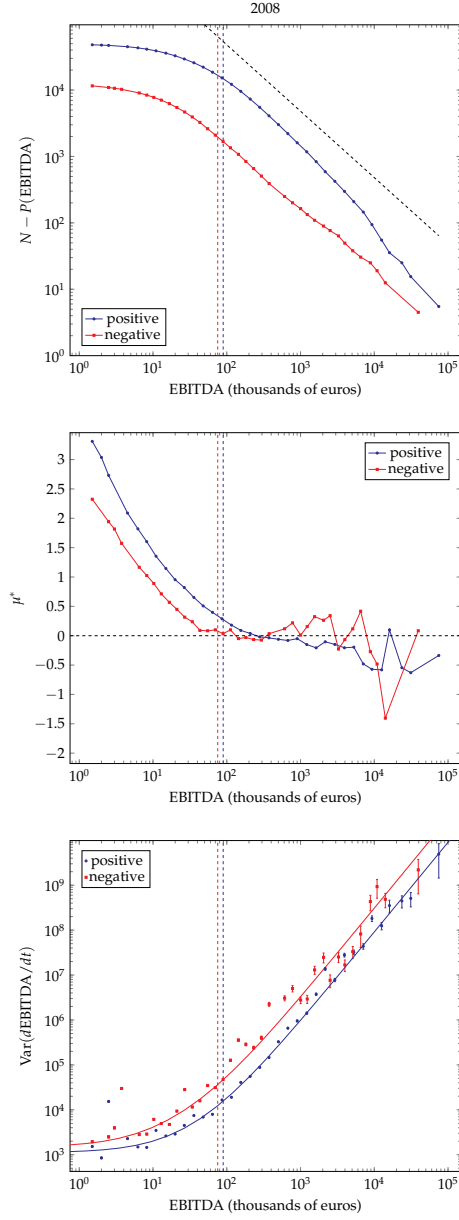

Figure 16: Andalusia

Rank plot, chemical potential and variance.

49271 Firms with positive EBITDA

$T_1 = 0.90 \pm 0.13$ ,  $T_{1/2} = 80.71 \pm 14.90$ , and  $T_0 = 1112.61 \pm 194.42$

12536 Firms with negative EBITDA

Negative EBITDA:

$T_1 = 3.06 \pm 0.82$ ,  $T_{1/2} = 231.00 \pm 57.49$ , and  $T_0 = 1484.42 \pm 526.15$ .

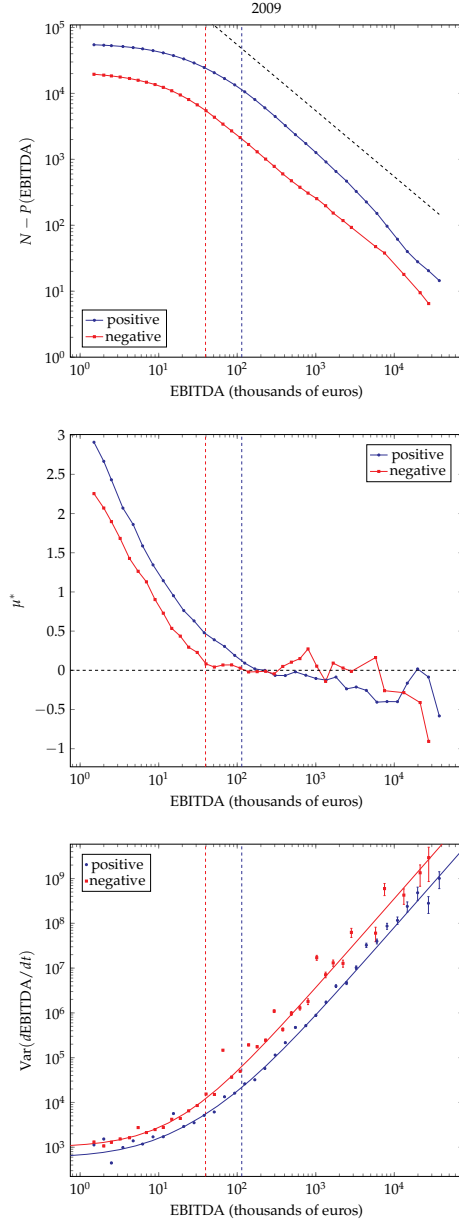

Figure 17: Andalusia

Rank plot, chemical potential and variance.

56793 Firms with positive EBITDA

$T_1 = 0.81 \pm 0.13$ ,  $T_{1/2} = 92.21 \pm 12.83$ , and  $T_0 = 581.93 \pm 116.96$

21368 Firms with negative EBITDA

Negative EBITDA:

$T_1 = 3.56 \pm 0.56$ ,  $T_{1/2} = 140.35 \pm 27.37$ , and  $T_0 = 986.86 \pm 170.60$ .

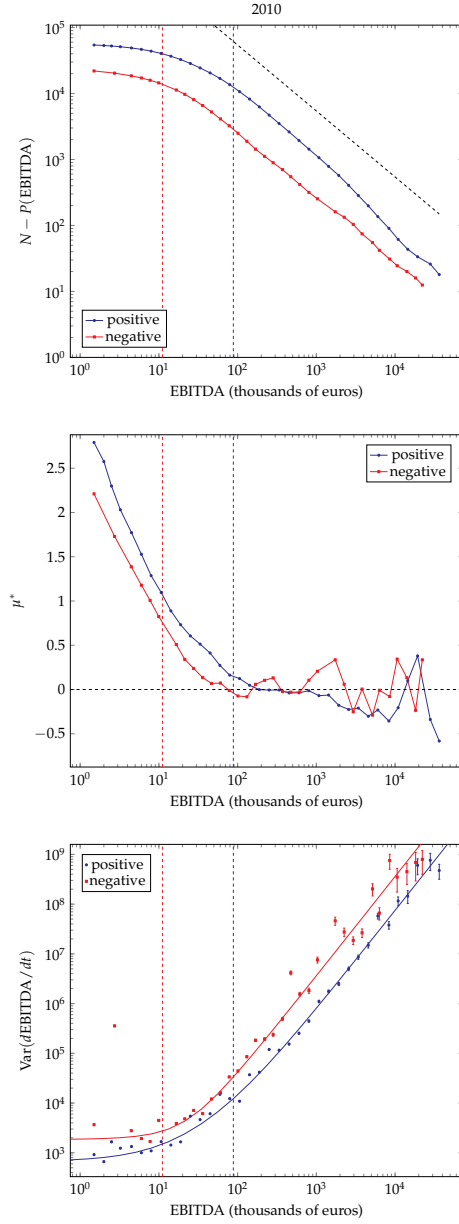

Figure 18: Andalusia

Rank plot, chemical potential and variance.

56713 Firms with positive EBITDA

$T_1 = 0.74 \pm 0.14$ ,  $T_{1/2} = 65.50 \pm 14.36$ , and  $T_0 = 671.42 \pm 147.02$

23996 Firms with negative EBITDA

Negative EBITDA:

$T_1 = 3.59 \pm 0.78$ ,  $T_{1/2} = 39.87 \pm 47.45$ , and  $T_0 = 1843.44 \pm 442.97$ .

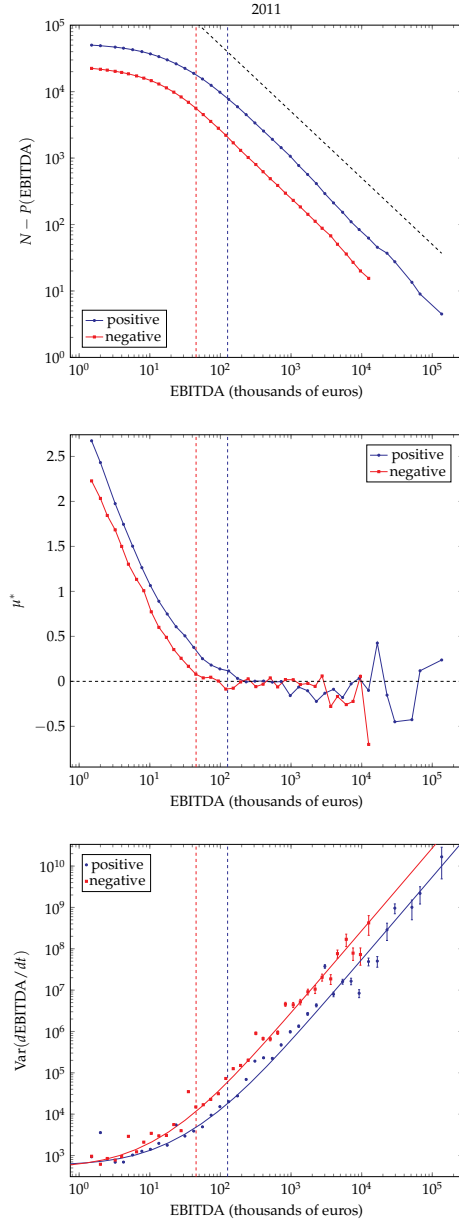

Figure 19: Andalusia

Rank plot, chemical potential and variance.

52600 Firms with positive EBITDA

$T_1 = 0.54 \pm 0.11$ ,  $T_{1/2} = 68.79 \pm 11.26$ , and  $T_0 = 578.03 \pm 115.85$

24364 Firms with negative EBITDA

Negative EBITDA:

$T_1 = 2.73 \pm 0.59$ ,  $T_{1/2} = 123.42 \pm 28.33$ , and  $T_0 = 500.04 \pm 148.92$ .

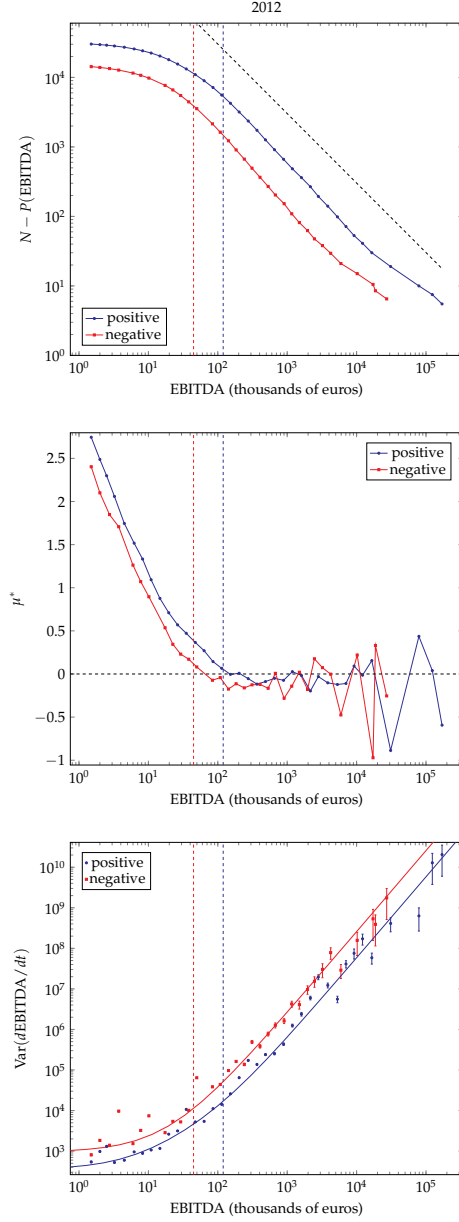

Figure 20: Andalusia

Rank plot, chemical potential and variance.

31522 Firms with positive EBITDA

$T_1 = 0.58 \pm 0.13$ ,  $T_{1/2} = 69.37 \pm 12.20$ , and  $T_0 = 353.90 \pm 105.19$

15335 Firms with negative EBITDA

Negative EBITDA:

$T_1 = 2.57 \pm 0.66$ ,  $T_{1/2} = 115.02 \pm 37.43$ , and  $T_0 = 951.08 \pm 273.09$ .

# Aragon

## Tables of Temperatures

### Positive EBITDA

| Year | $T_1$           | $T_{1/2}$          | $T_0$               | $T_{1/2}/T_1$ | Num. Firms |
|------|-----------------|--------------------|---------------------|---------------|------------|
| 2003 | $0.39 \pm 0.07$ | $30.62 \pm 6.38$   | $207.75 \pm 73.39$  | 78.1          | 14783      |
| 2004 | $0.46 \pm 0.09$ | $35.33 \pm 9.63$   | $239.62 \pm 95.26$  | 76.7          | 16069      |
| 2005 | $0.44 \pm 0.12$ | $63.63 \pm 12.61$  | $138.92 \pm 90.45$  | 145.9         | 17717      |
| 2006 | $0.55 \pm 0.13$ | $58.61 \pm 16.47$  | $86.32 \pm 173.47$  | 106.1         | 18581      |
| 2007 | $0.80 \pm 0.10$ | $19.25 \pm 8.56$   | $473.76 \pm 104.02$ | 24.1          | 17733      |
| 2008 | $0.67 \pm 0.21$ | $87.99 \pm 24.45$  | $227.80 \pm 218.58$ | 130.4         | 16136      |
| 2009 | $0.81 \pm 0.19$ | $73.86 \pm 21.06$  | $609.94 \pm 221.33$ | 91.1          | 16849      |
| 2010 | $0.27 \pm 0.20$ | $113.28 \pm 29.45$ | $227.04 \pm 211.62$ | 417.2         | 16338      |
| 2011 | $0.49 \pm 0.12$ | $57.93 \pm 13.74$  | $405.98 \pm 144.62$ | 118.0         | 15382      |
| 2012 | $0.38 \pm 0.09$ | $66.47 \pm 10.20$  | $315.02 \pm 99.21$  | 172.8         | 10568      |

### Negative EBITDA

| Year | $T_1$           | $T_{1/2}$          | $T_0$                 | $T_{1/2}/T_1$ | Num. Firms |
|------|-----------------|--------------------|-----------------------|---------------|------------|
| 2003 | $0.88 \pm 0.67$ | $163.66 \pm 40.64$ | $89.18 \pm 148.13$    | 185.0         | 3103       |
| 2004 | $1.88 \pm 0.49$ | $132.75 \pm 18.59$ | $110.16 \pm 66.47$    | 70.7          | 3524       |
| 2005 | $1.82 \pm 0.82$ | $124.52 \pm 35.35$ | $58.86 \pm 131.46$    | 68.4          | 4255       |
| 2006 | $2.55 \pm 0.92$ | $110.47 \pm 43.16$ | $176.95 \pm 218.00$   | 43.3          | 4364       |
| 2007 | $2.04 \pm 0.99$ | $190.42 \pm 59.36$ | $108.04 \pm 174.43$   | 93.5          | 3434       |
| 2008 | $4.84 \pm 1.52$ | $93.11 \pm 106.65$ | $1772.44 \pm 1085.26$ | 19.3          | 3457       |
| 2009 | $3.50 \pm 1.48$ | $130.52 \pm 74.68$ | $1759.48 \pm 527.87$  | 37.3          | 5562       |
| 2010 | $2.33 \pm 0.69$ | $205.62 \pm 42.04$ | $92.07 \pm 229.35$    | 88.1          | 6422       |
| 2011 | $1.78 \pm 1.14$ | $176.00 \pm 47.86$ | $294.02 \pm 216.39$   | 99.1          | 6670       |
| 2012 | $2.35 \pm 0.46$ | $116.80 \pm 24.32$ | $549.98 \pm 136.68$   | 49.6          | 5052       |

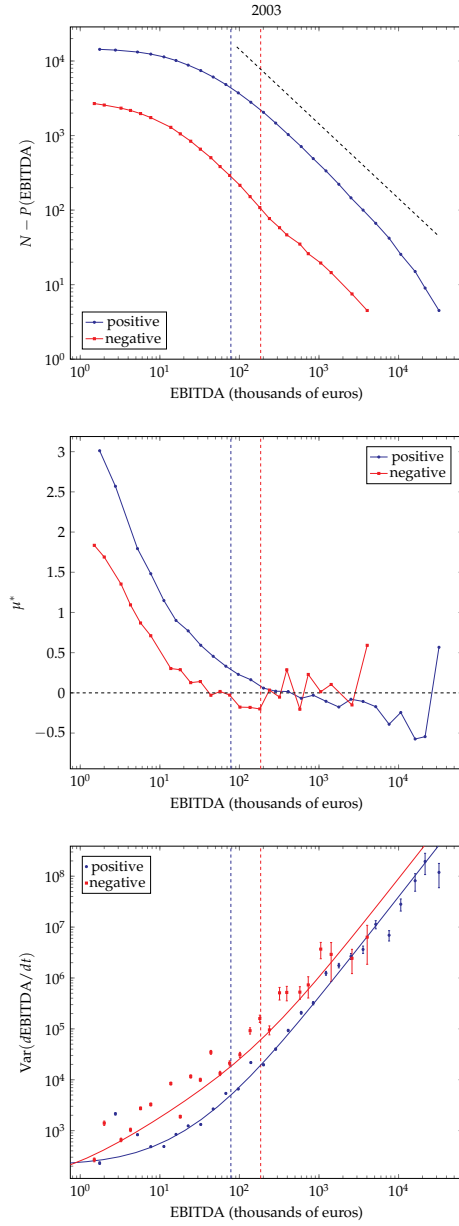

Figure 21: Aragon

Rank plot, chemical potential and variance.

14783 Firms with positive EBITDA

$T_1 = 0.39 \pm 0.07$ ,  $T_{1/2} = 30.62 \pm 6.38$ , and  $T_0 = 207.75 \pm 73.39$

3103 Firms with negative EBITDA

Negative EBITDA:

$T_1 = 0.88 \pm 0.67$ ,  $T_{1/2} = 163.66 \pm 40.64$ , and  $T_0 = 89.18 \pm 148.13$ .

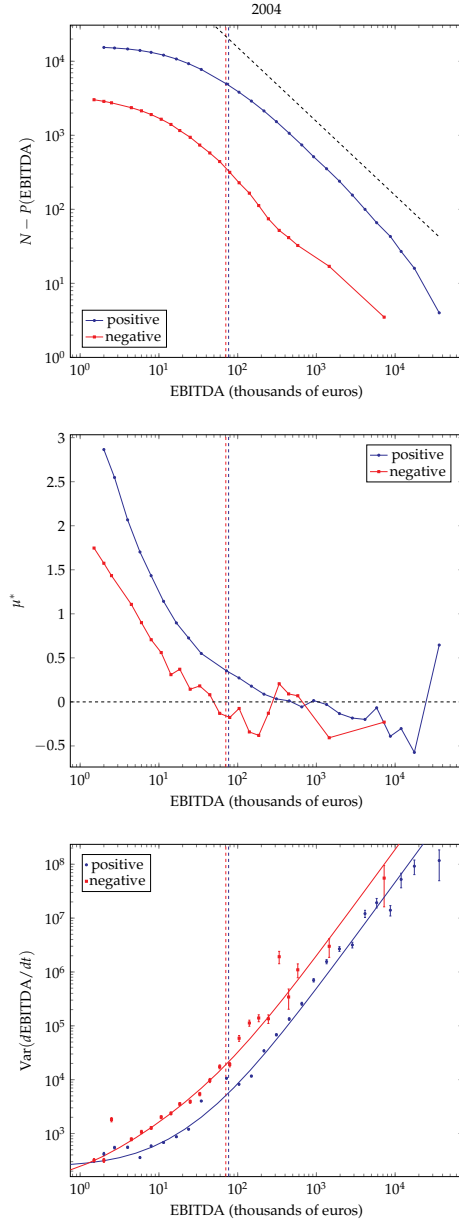

Figure 22: Aragon

Rank plot, chemical potential and variance.

16069 Firms with positive EBITDA

$T_1 = 0.46 \pm 0.09$ ,  $T_{1/2} = 35.33 \pm 9.63$ , and  $T_0 = 239.62 \pm 95.26$

3524 Firms with negative EBITDA

Negative EBITDA:

$T_1 = 1.88 \pm 0.49$ ,  $T_{1/2} = 132.75 \pm 18.59$ , and  $T_0 = 110.16 \pm 66.47$ .

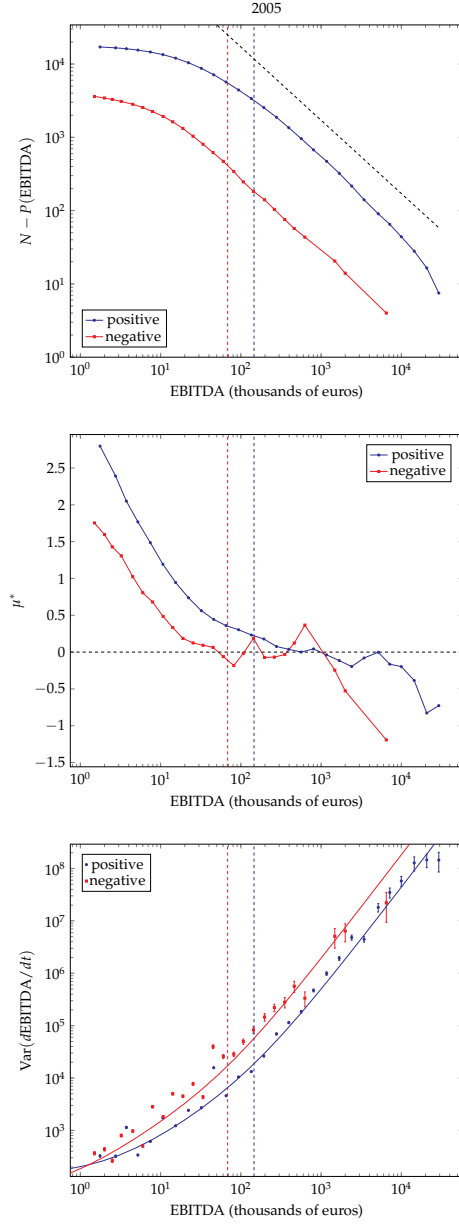

Figure 23: Aragon

Rank plot, chemical potential and variance.

17717 Firms with positive EBITDA

$T_1 = 0.44 \pm 0.12$ ,  $T_{1/2} = 63.63 \pm 12.61$ , and  $T_0 = 138.92 \pm 90.45$

4255 Firms with negative EBITDA

Negative EBITDA:

$T_1 = 1.82 \pm 0.82$ ,  $T_{1/2} = 124.52 \pm 35.35$ , and  $T_0 = 58.86 \pm 131.46$ .

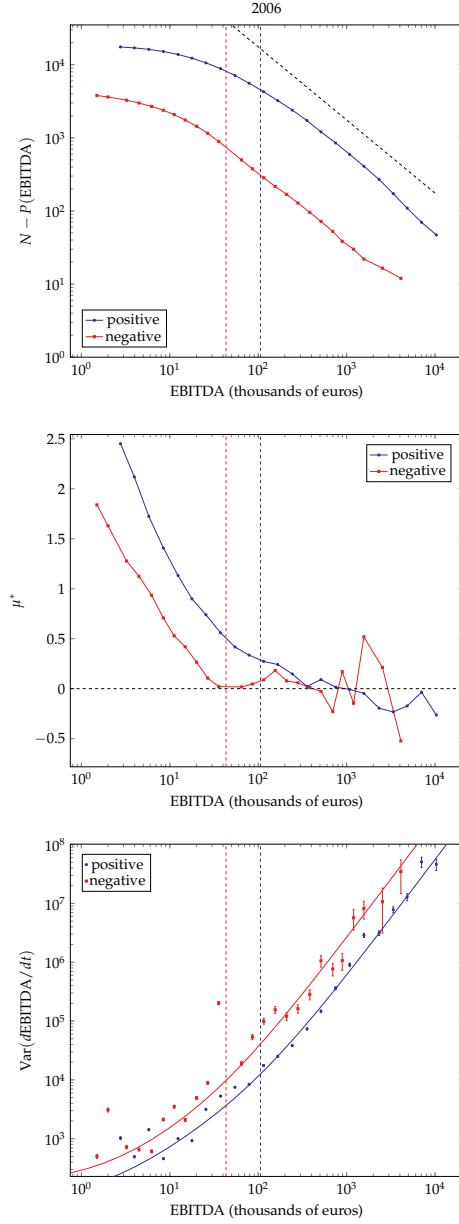

Figure 24: Aragon

Rank plot, chemical potential and variance.

18581 Firms with positive EBITDA

$T_1 = 0.55 \pm 0.13$ ,  $T_{1/2} = 58.61 \pm 16.47$ , and  $T_0 = 86.32 \pm 173.47$

4364 Firms with negative EBITDA

Negative EBITDA:

$T_1 = 2.55 \pm 0.92$ ,  $T_{1/2} = 110.47 \pm 43.16$ , and  $T_0 = 176.95 \pm 218.00$ .

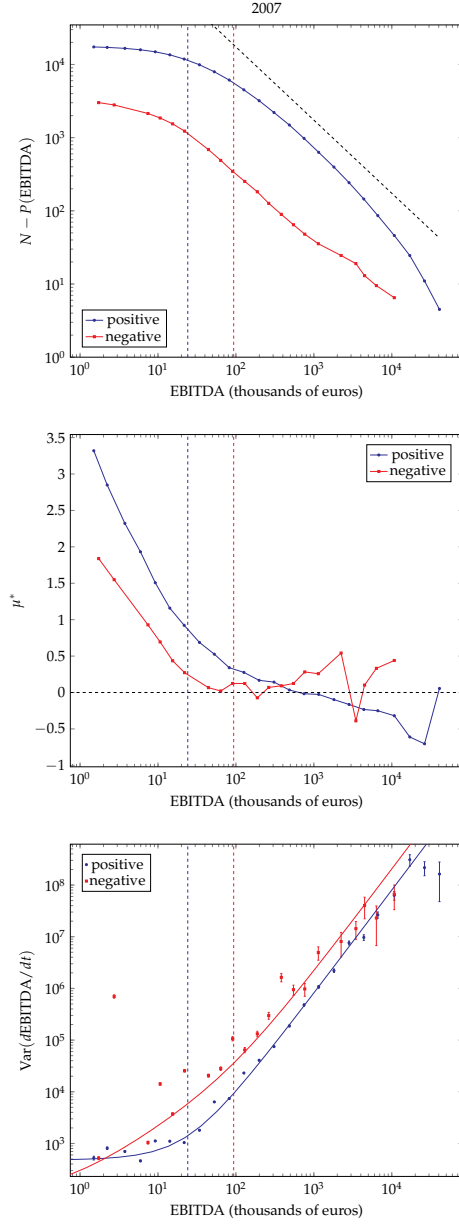

Figure 25: Aragon

Rank plot, chemical potential and variance.

17733 Firms with positive EBITDA

$T_1 = 0.80 \pm 0.10$ ,  $T_{1/2} = 19.25 \pm 8.56$ , and  $T_0 = 473.76 \pm 104.02$

3434 Firms with negative EBITDA

Negative EBITDA:

$T_1 = 2.04 \pm 0.99$ ,  $T_{1/2} = 190.42 \pm 59.36$ , and  $T_0 = 108.04 \pm 174.43$ .

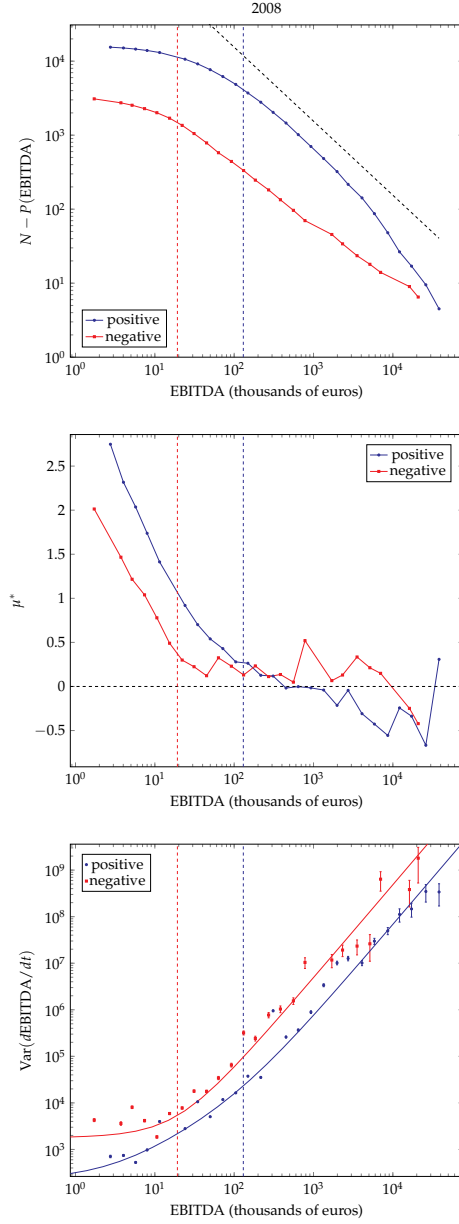

Figure 26: Aragon

Rank plot, chemical potential and variance.

16136 Firms with positive EBITDA

$T_1 = 0.67 \pm 0.21$ ,  $T_{1/2} = 87.99 \pm 24.45$ , and  $T_0 = 227.80 \pm 218.58$

3457 Firms with negative EBITDA

Negative EBITDA:

$T_1 = 4.84 \pm 1.52$ ,  $T_{1/2} = 93.11 \pm 106.65$ , and  $T_0 = 1772.44 \pm 1085.26$ .

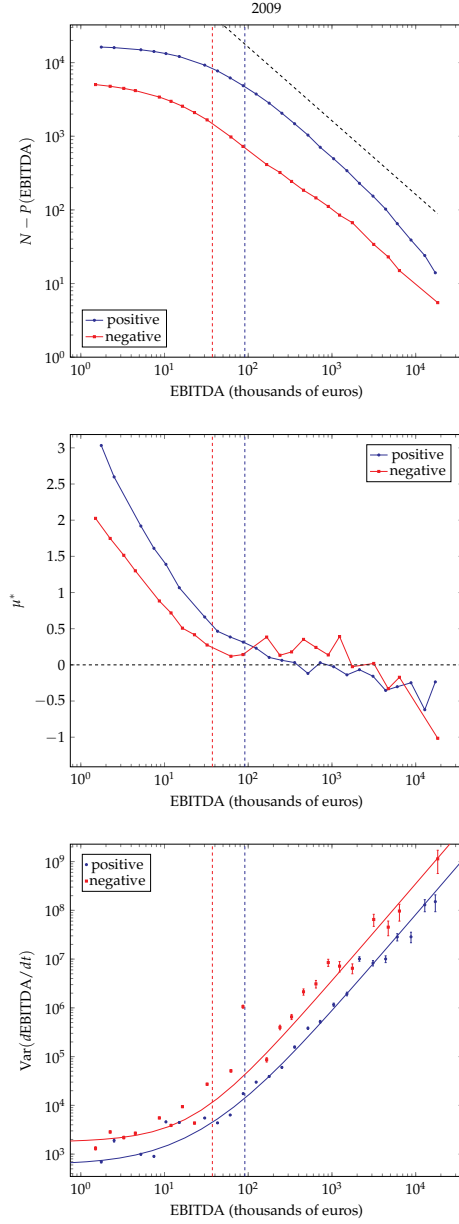

Figure 27: Aragon

Rank plot, chemical potential and variance.

16849 Firms with positive EBITDA

$T_1 = 0.81 \pm 0.19$ ,  $T_{1/2} = 73.86 \pm 21.06$ , and  $T_0 = 609.94 \pm 221.33$

5562 Firms with negative EBITDA

Negative EBITDA:

$T_1 = 3.50 \pm 1.48$ ,  $T_{1/2} = 130.52 \pm 74.68$ , and  $T_0 = 1759.48 \pm 527.87$ .

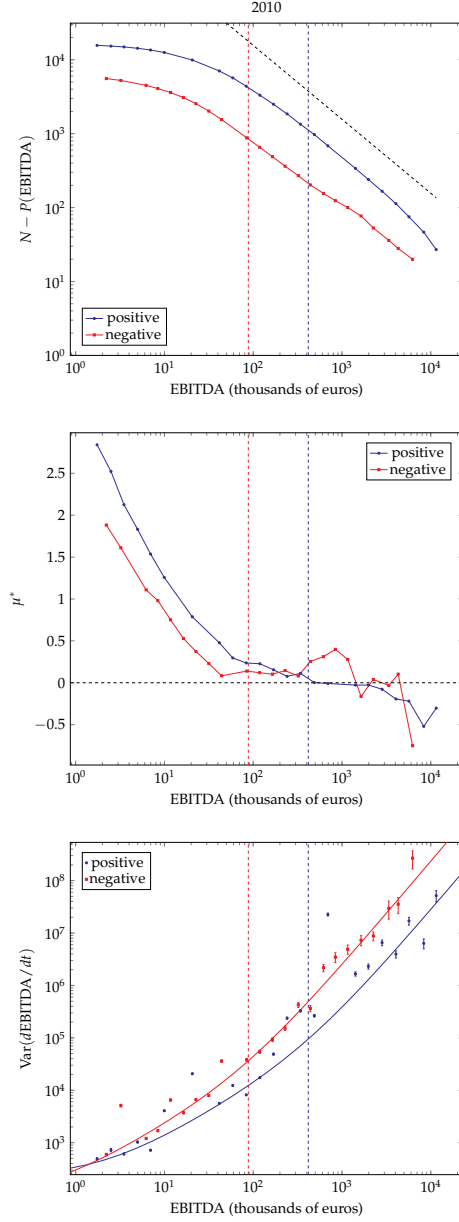

Figure 28: Aragon

Rank plot, chemical potential and variance.

16338 Firms with positive EBITDA

$T_1 = 0.27 \pm 0.20$ ,  $T_{1/2} = 113.28 \pm 29.45$ , and  $T_0 = 227.04 \pm 211.62$

6422 Firms with negative EBITDA

Negative EBITDA:

$T_1 = 2.33 \pm 0.69$ ,  $T_{1/2} = 205.62 \pm 42.04$ , and  $T_0 = 92.07 \pm 229.35$ .

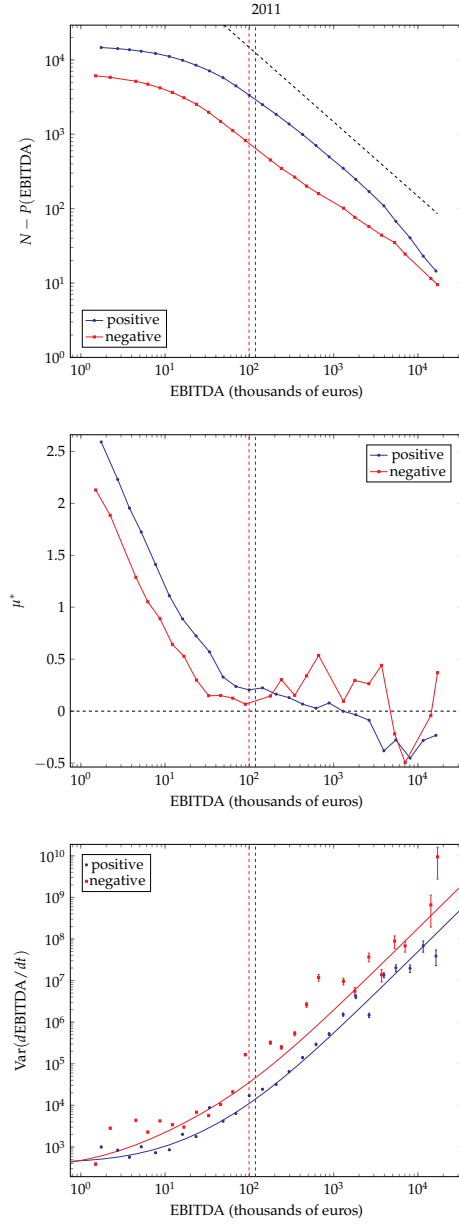

Figure 29: Aragon

Rank plot, chemical potential and variance.

15382 Firms with positive EBITDA

$T_1 = 0.49 \pm 0.12$ ,  $T_{1/2} = 57.93 \pm 13.74$ , and  $T_0 = 405.98 \pm 144.62$

6670 Firms with negative EBITDA

Negative EBITDA:

$T_1 = 1.78 \pm 1.14$ ,  $T_{1/2} = 176.00 \pm 47.86$ , and  $T_0 = 294.02 \pm 216.39$ .

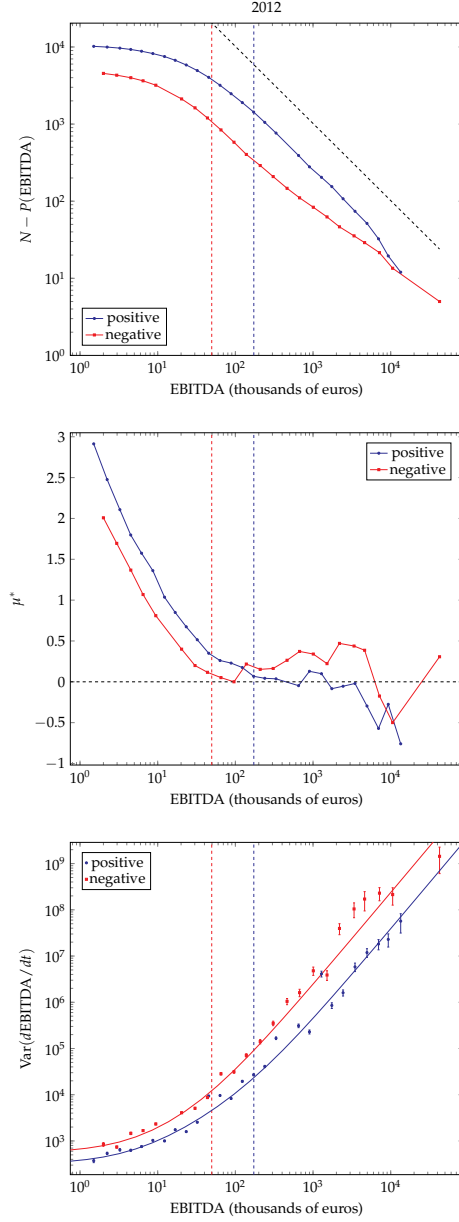

Figure 30: Aragon

Rank plot, chemical potential and variance.

10568 Firms with positive EBITDA

$T_1 = 0.38 \pm 0.09$ ,  $T_{1/2} = 66.47 \pm 10.20$ , and  $T_0 = 315.02 \pm 99.21$

5052 Firms with negative EBITDA

Negative EBITDA:

$T_1 = 2.35 \pm 0.46$ ,  $T_{1/2} = 116.80 \pm 24.32$ , and  $T_0 = 549.98 \pm 136.68$ .

# Asturias

## Tables of Temperatures

### Positive EBITDA

| Year | $T_1$           | $T_{1/2}$         | $T_0$               | $T_{1/2}/T_1$ | Num. Firms |
|------|-----------------|-------------------|---------------------|---------------|------------|
| 2003 | $0.44 \pm 0.15$ | $25.85 \pm 12.65$ | $171.97 \pm 147.62$ | 59.4          | 7937       |
| 2004 | $0.55 \pm 0.14$ | $37.58 \pm 11.90$ | $135.89 \pm 102.27$ | 68.6          | 7760       |
| 2005 | $0.17 \pm 0.07$ | $55.57 \pm 10.03$ | $102.72 \pm 122.03$ | 319.4         | 8147       |
| 2006 | $0.55 \pm 0.09$ | $53.01 \pm 10.24$ | $118.38 \pm 98.60$  | 96.3          | 8683       |
| 2007 | $0.69 \pm 0.10$ | $14.46 \pm 10.53$ | $661.07 \pm 165.64$ | 20.9          | 8674       |
| 2008 | $0.59 \pm 0.14$ | $43.35 \pm 15.22$ | $384.95 \pm 157.04$ | 73.2          | 8255       |
| 2009 | $0.59 \pm 0.11$ | $59.29 \pm 10.92$ | $247.94 \pm 99.02$  | 100.0         | 9567       |
| 2010 | $0.40 \pm 0.11$ | $67.61 \pm 12.72$ | $224.24 \pm 120.05$ | 168.6         | 9436       |
| 2011 | $0.45 \pm 0.16$ | $62.45 \pm 20.62$ | $160.69 \pm 219.32$ | 139.2         | 8549       |
| 2012 | $0.46 \pm 0.15$ | $54.77 \pm 17.13$ | $445.50 \pm 171.78$ | 118.7         | 5688       |

### Negative EBITDA

| Year | $T_1$           | $T_{1/2}$           | $T_0$                | $T_{1/2}/T_1$ | Num. Firms |
|------|-----------------|---------------------|----------------------|---------------|------------|
| 2003 | $3.36 \pm 1.45$ | $6.23 \pm 51.46$    | $679.52 \pm 304.72$  | 1.9           | 1984       |
| 2004 | $2.13 \pm 0.59$ | $108.32 \pm 26.01$  | $173.92 \pm 107.91$  | 50.8          | 1902       |
| 2005 | $1.08 \pm 0.80$ | $155.25 \pm 53.78$  | $575.76 \pm 369.28$  | 143.5         | 1877       |
| 2006 | $1.97 \pm 0.84$ | $74.27 \pm 44.13$   | $448.45 \pm 343.59$  | 37.6          | 2064       |
| 2007 | $1.30 \pm 1.08$ | $329.05 \pm 112.09$ | $0.03 \pm 327.93$    | 252.7         | 1712       |
| 2008 | $1.79 \pm 1.10$ | $235.64 \pm 55.73$  | $132.28 \pm 177.78$  | 131.9         | 1729       |
| 2009 | $3.34 \pm 1.17$ | $84.17 \pm 40.36$   | $692.79 \pm 194.26$  | 25.2          | 3214       |
| 2010 | $2.77 \pm 0.60$ | $48.23 \pm 28.70$   | $1045.07 \pm 202.44$ | 17.4          | 3789       |
| 2011 | $2.67 \pm 0.56$ | $66.10 \pm 22.61$   | $504.15 \pm 122.22$  | 24.7          | 4130       |
| 2012 | $1.36 \pm 0.60$ | $133.16 \pm 36.64$  | $159.52 \pm 167.35$  | 97.6          | 3223       |

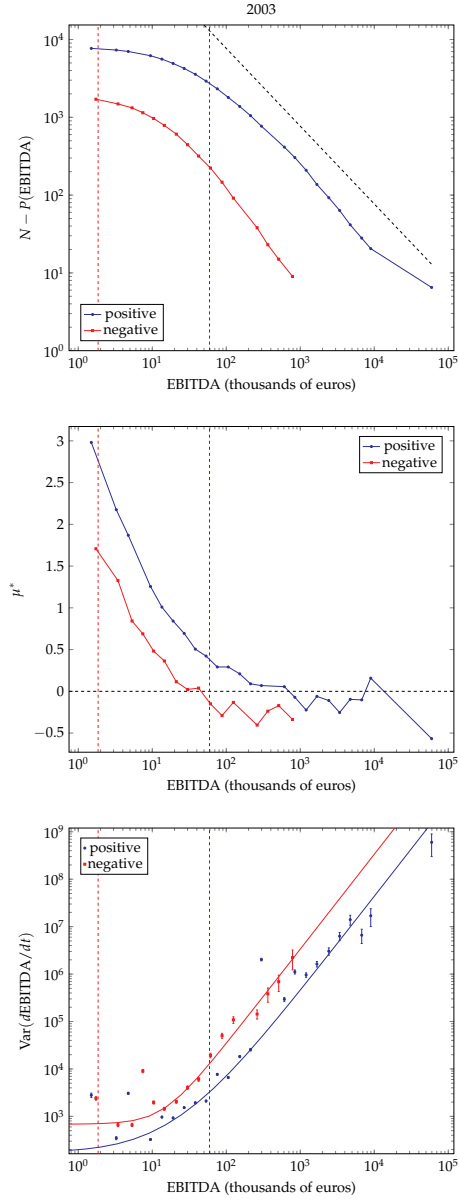

Figure 31: Asturias

Rank plot, chemical potential and variance.

7937 Firms with positive EBITDA

$T_1 = 0.44 \pm 0.15$ ,  $T_{1/2} = 25.85 \pm 12.65$ , and  $T_0 = 171.97 \pm 147.62$

1984 Firms with negative EBITDA

Negative EBITDA:

$T_1 = 3.36 \pm 1.45$ ,  $T_{1/2} = 6.23 \pm 51.46$ , and  $T_0 = 679.52 \pm 304.72$ .

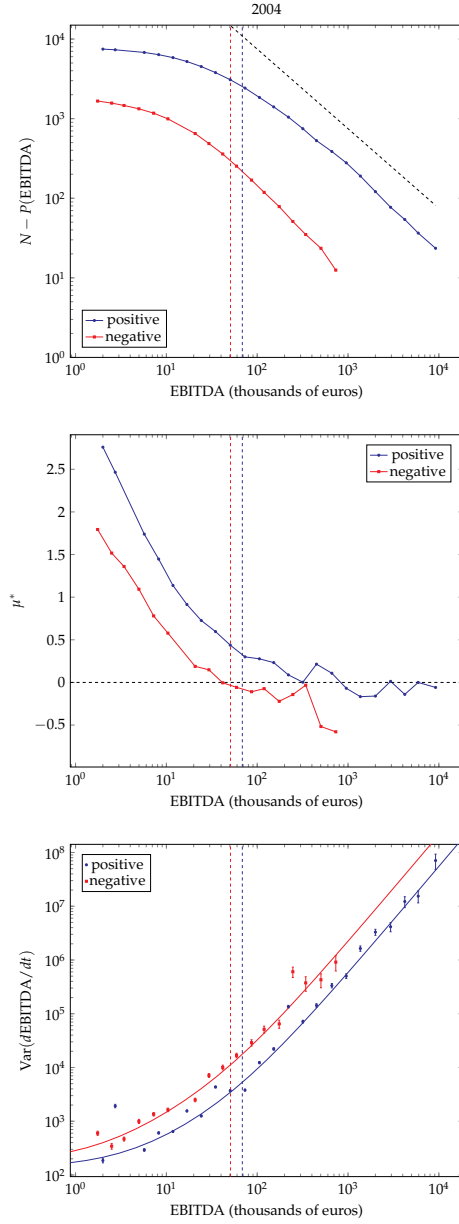

Figure 32: Asturias

Rank plot, chemical potential and variance.

7760 Firms with positive EBITDA

$T_1 = 0.55 \pm 0.14$ ,  $T_{1/2} = 37.58 \pm 11.90$ , and  $T_0 = 135.89 \pm 102.27$

1902 Firms with negative EBITDA

Negative EBITDA:

$T_1 = 2.13 \pm 0.59$ ,  $T_{1/2} = 108.32 \pm 26.01$ , and  $T_0 = 173.92 \pm 107.91$ .

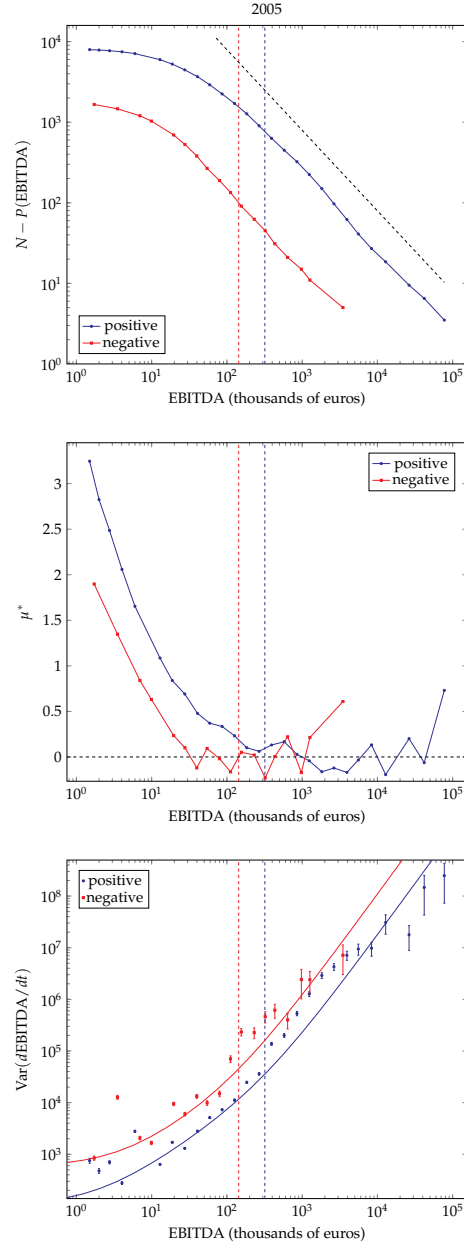

Figure 33: Asturias

Rank plot, chemical potential and variance.

8147 Firms with positive EBITDA

$T_1 = 0.17 \pm 0.07$ ,  $T_{1/2} = 55.57 \pm 10.03$ , and  $T_0 = 102.72 \pm 122.03$

1877 Firms with negative EBITDA

Negative EBITDA:

$T_1 = 1.08 \pm 0.80$ ,  $T_{1/2} = 155.25 \pm 53.78$ , and  $T_0 = 575.76 \pm 369.28$ .

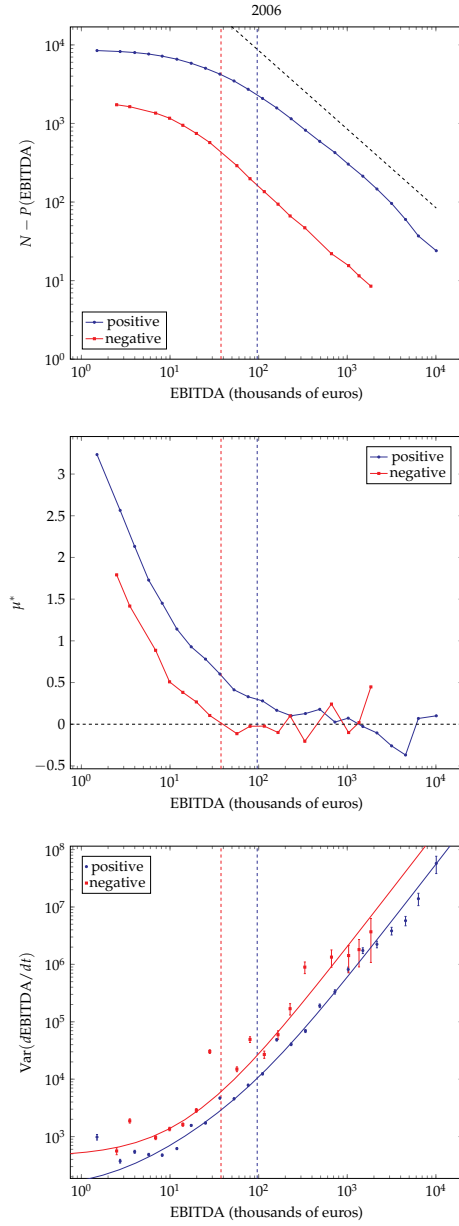

Figure 34: Asturias

Rank plot, chemical potential and variance.

8683 Firms with positive EBITDA

$T_1 = 0.55 \pm 0.09$ ,  $T_{1/2} = 53.01 \pm 10.24$ , and  $T_0 = 118.38 \pm 98.60$

2064 Firms with negative EBITDA

Negative EBITDA:

$T_1 = 1.97 \pm 0.84$ ,  $T_{1/2} = 74.27 \pm 44.13$ , and  $T_0 = 448.45 \pm 343.59$ .

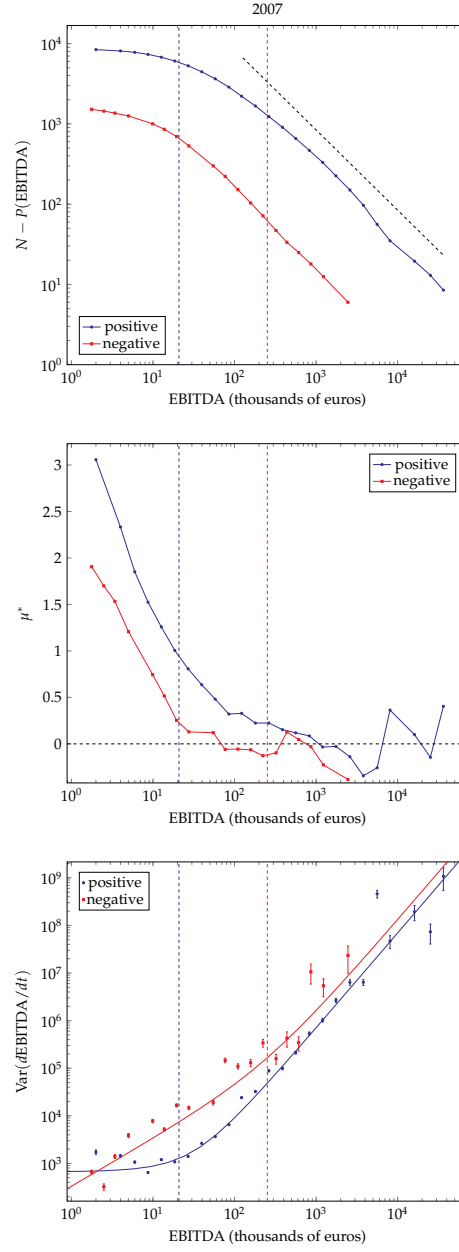

Figure 35: Asturias

Rank plot, chemical potential and variance.

8674 Firms with positive EBITDA

$T_1 = 0.69 \pm 0.10$ ,  $T_{1/2} = 14.46 \pm 10.53$ , and  $T_0 = 661.07 \pm 165.64$

1712 Firms with negative EBITDA

Negative EBITDA:

$T_1 = 1.30 \pm 1.08$ ,  $T_{1/2} = 329.05 \pm 112.09$ , and  $T_0 = 0.03 \pm 327.93$ .

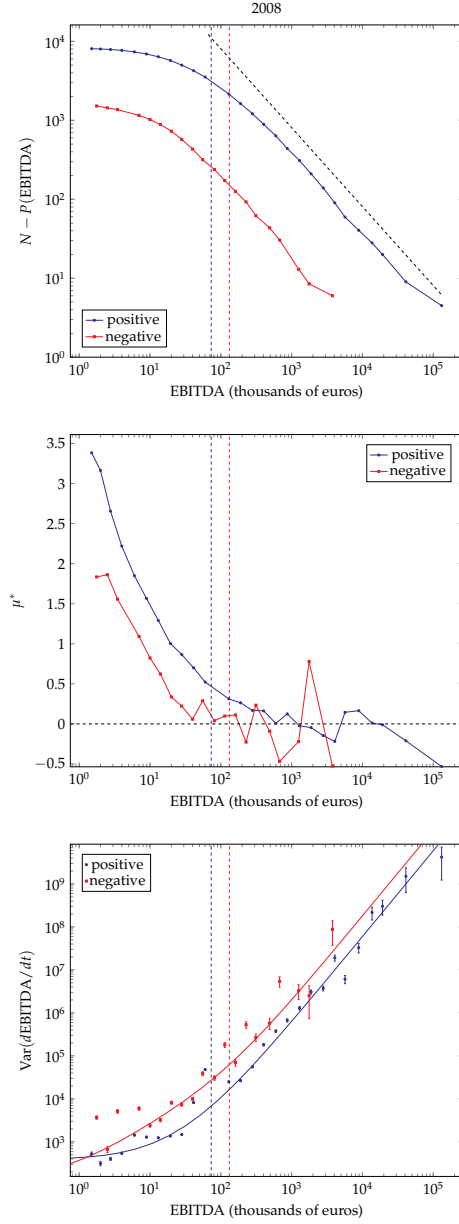

Figure 36: Asturias

Rank plot, chemical potential and variance.

8255 Firms with positive EBITDA

$T_1 = 0.59 \pm 0.14$ ,  $T_{1/2} = 43.35 \pm 15.22$ , and  $T_0 = 384.95 \pm 157.04$

1729 Firms with negative EBITDA

Negative EBITDA:

$T_1 = 1.79 \pm 1.10$ ,  $T_{1/2} = 235.64 \pm 55.73$ , and  $T_0 = 132.28 \pm 177.78$ .

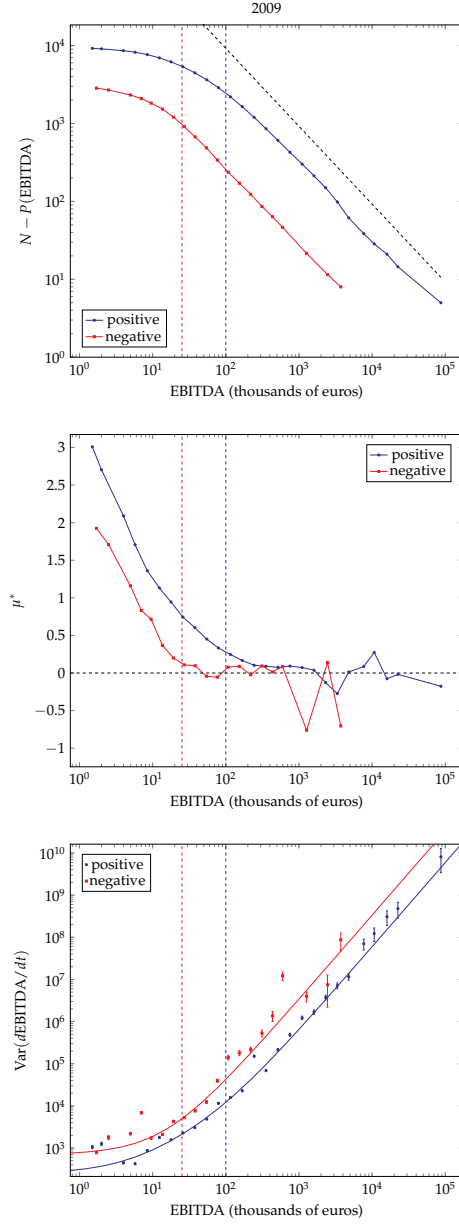

Figure 37: Asturias

Rank plot, chemical potential and variance.

9567 Firms with positive EBITDA

$T_1 = 0.59 \pm 0.11$ ,  $T_{1/2} = 59.29 \pm 10.92$ , and  $T_0 = 247.94 \pm 99.02$

3214 Firms with negative EBITDA

Negative EBITDA:

$T_1 = 3.34 \pm 1.17$ ,  $T_{1/2} = 84.17 \pm 40.36$ , and  $T_0 = 692.79 \pm 194.26$ .

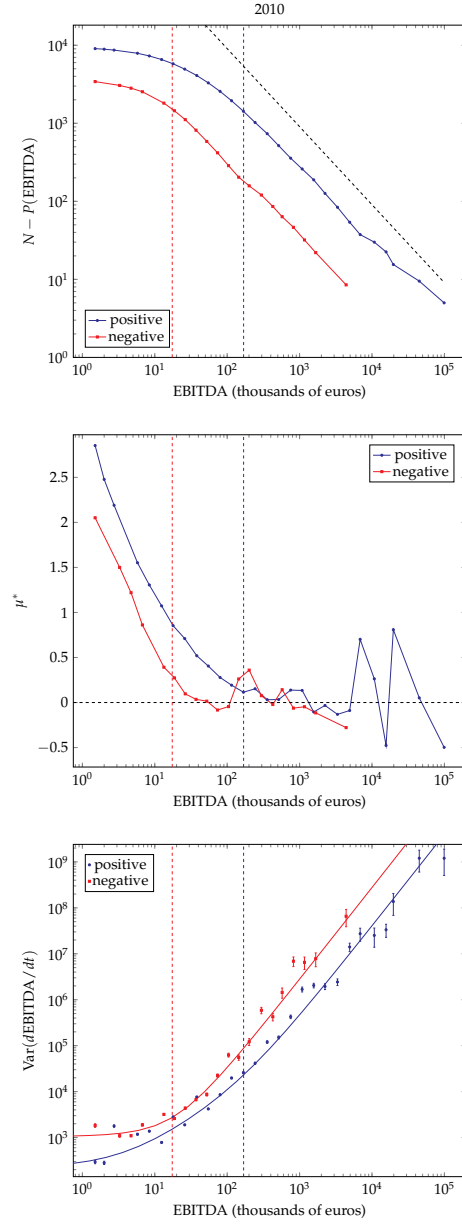

Figure 38: Asturias

Rank plot, chemical potential and variance.

9436 Firms with positive EBITDA

$T_1 = 0.40 \pm 0.11$ ,  $T_{1/2} = 67.61 \pm 12.72$ , and  $T_0 = 224.24 \pm 120.05$

3789 Firms with negative EBITDA

Negative EBITDA:

$T_1 = 2.77 \pm 0.60$ ,  $T_{1/2} = 48.23 \pm 28.70$ , and  $T_0 = 1045.07 \pm 202.44$ .

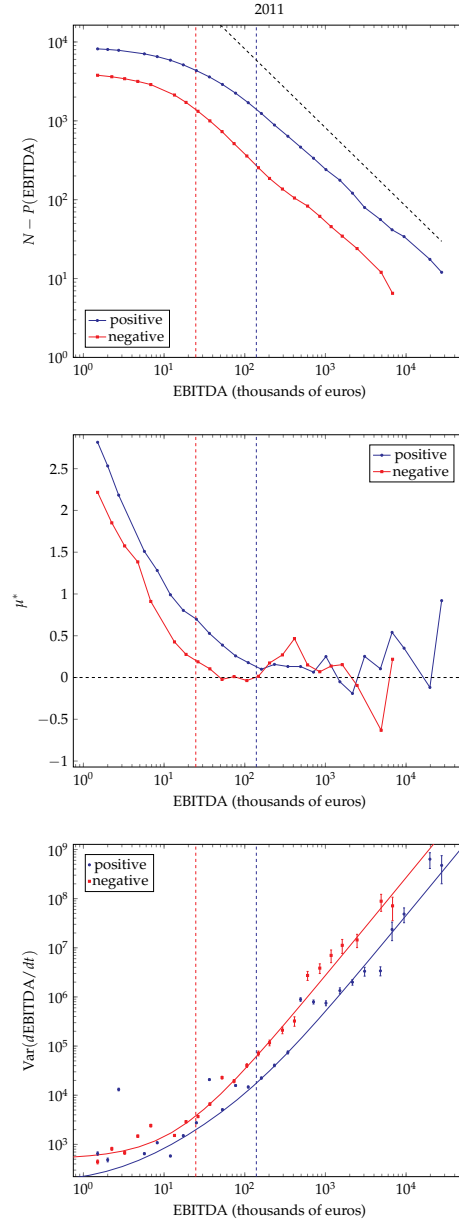

Figure 39: Asturias

Rank plot, chemical potential and variance.

8549 Firms with positive EBITDA

$T_1 = 0.45 \pm 0.16$ ,  $T_{1/2} = 62.45 \pm 20.62$ , and  $T_0 = 160.69 \pm 219.32$

4130 Firms with negative EBITDA

Negative EBITDA:

$T_1 = 2.67 \pm 0.56$ ,  $T_{1/2} = 66.10 \pm 22.61$ , and  $T_0 = 504.15 \pm 122.22$ .

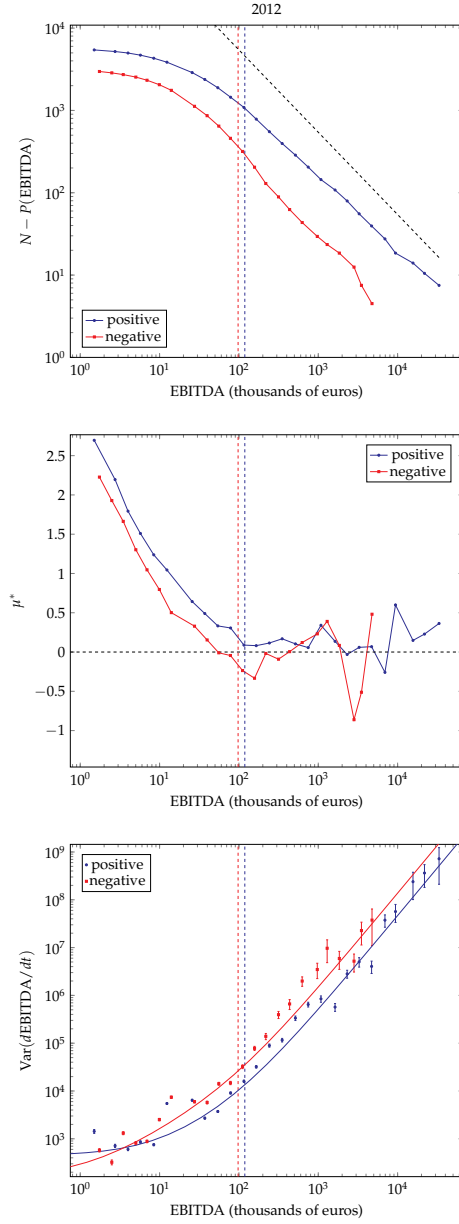

Figure 40: Asturias

Rank plot, chemical potential and variance.

5688 Firms with positive EBITDA

$T_1 = 0.46 \pm 0.15$ ,  $T_{1/2} = 54.77 \pm 17.13$ , and  $T_0 = 445.50 \pm 171.78$

3223 Firms with negative EBITDA

Negative EBITDA:

$T_1 = 1.36 \pm 0.60$ ,  $T_{1/2} = 133.16 \pm 36.64$ , and  $T_0 = 159.52 \pm 167.35$ .

# Balearic islands

## Tables of Temperatures

### Positive EBITDA

| Year | $T_1$           | $T_{1/2}$         | $T_0$                | $T_{1/2}/T_1$ | Num. Firms |
|------|-----------------|-------------------|----------------------|---------------|------------|
| 2003 | $0.34 \pm 0.09$ | $61.04 \pm 9.77$  | $170.22 \pm 83.73$   | 178.9         | 11636      |
| 2004 | $0.35 \pm 0.05$ | $54.77 \pm 6.21$  | $214.90 \pm 66.26$   | 154.5         | 11800      |
| 2005 | $0.41 \pm 0.13$ | $41.22 \pm 13.74$ | $419.99 \pm 175.33$  | 101.1         | 12071      |
| 2006 | $0.49 \pm 0.12$ | $45.35 \pm 12.47$ | $256.95 \pm 130.77$  | 92.0          | 12450      |
| 2007 | $0.51 \pm 0.11$ | $39.93 \pm 16.79$ | $751.51 \pm 281.20$  | 78.7          | 12081      |
| 2008 | $0.66 \pm 0.15$ | $48.93 \pm 21.33$ | $1061.51 \pm 377.54$ | 74.6          | 10794      |
| 2009 | $1.16 \pm 0.29$ | $50.21 \pm 22.03$ | $520.08 \pm 199.66$  | 43.4          | 13852      |
| 2010 | $0.63 \pm 0.19$ | $65.93 \pm 22.25$ | $490.92 \pm 251.73$  | 105.4         | 13145      |
| 2011 | $0.46 \pm 0.16$ | $63.57 \pm 18.19$ | $364.13 \pm 174.51$  | 136.8         | 12437      |
| 2012 | $0.56 \pm 0.11$ | $34.76 \pm 14.82$ | $679.14 \pm 206.87$  | 62.0          | 5051       |

### Negative EBITDA

| Year | $T_1$           | $T_{1/2}$          | $T_0$                | $T_{1/2}/T_1$ | Num. Firms |
|------|-----------------|--------------------|----------------------|---------------|------------|
| 2003 | $1.36 \pm 0.82$ | $127.09 \pm 43.91$ | $150.32 \pm 152.99$  | 93.6          | 3333       |
| 2004 | $1.01 \pm 0.61$ | $212.72 \pm 45.25$ | $106.42 \pm 232.83$  | 211.4         | 3243       |
| 2005 | $1.70 \pm 0.84$ | $193.80 \pm 40.79$ | $90.35 \pm 157.19$   | 113.8         | 3221       |
| 2006 | $1.59 \pm 0.56$ | $145.71 \pm 33.84$ | $365.48 \pm 196.13$  | 91.5          | 3393       |
| 2007 | $1.00 \pm 0.51$ | $224.82 \pm 40.50$ | $541.95 \pm 250.57$  | 224.4         | 2875       |
| 2008 | $2.47 \pm 0.84$ | $204.36 \pm 51.11$ | $797.82 \pm 303.62$  | 82.9          | 2682       |
| 2009 | $2.55 \pm 0.69$ | $85.52 \pm 42.33$  | $1434.99 \pm 367.10$ | 33.5          | 5507       |
| 2010 | $1.22 \pm 0.45$ | $155.86 \pm 27.09$ | $408.94 \pm 132.42$  | 128.2         | 6033       |
| 2011 | $2.41 \pm 0.55$ | $78.20 \pm 26.49$  | $477.38 \pm 192.76$  | 32.5          | 5812       |
| 2012 | $1.99 \pm 0.56$ | $85.70 \pm 33.94$  | $1109.74 \pm 276.49$ | 43.1          | 2197       |

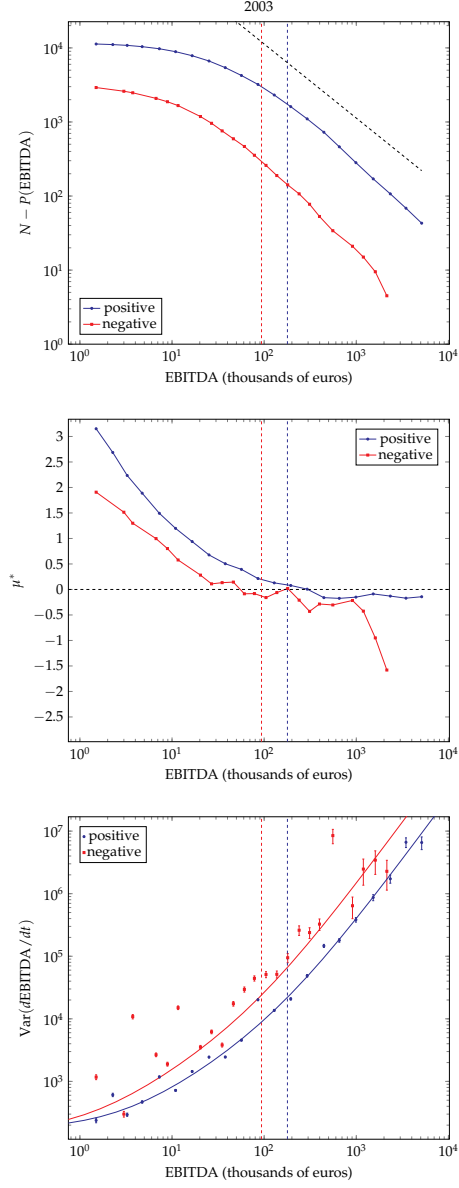

Figure 41: Balearic islands

Rank plot, chemical potential and variance.

11636 Firms with positive EBITDA

$T_1 = 0.34 \pm 0.09$ ,  $T_{1/2} = 61.04 \pm 9.77$ , and  $T_0 = 170.22 \pm 83.73$

3333 Firms with negative EBITDA

Negative EBITDA:

$T_1 = 1.36 \pm 0.82$ ,  $T_{1/2} = 127.09 \pm 43.91$ , and  $T_0 = 150.32 \pm 152.99$ .

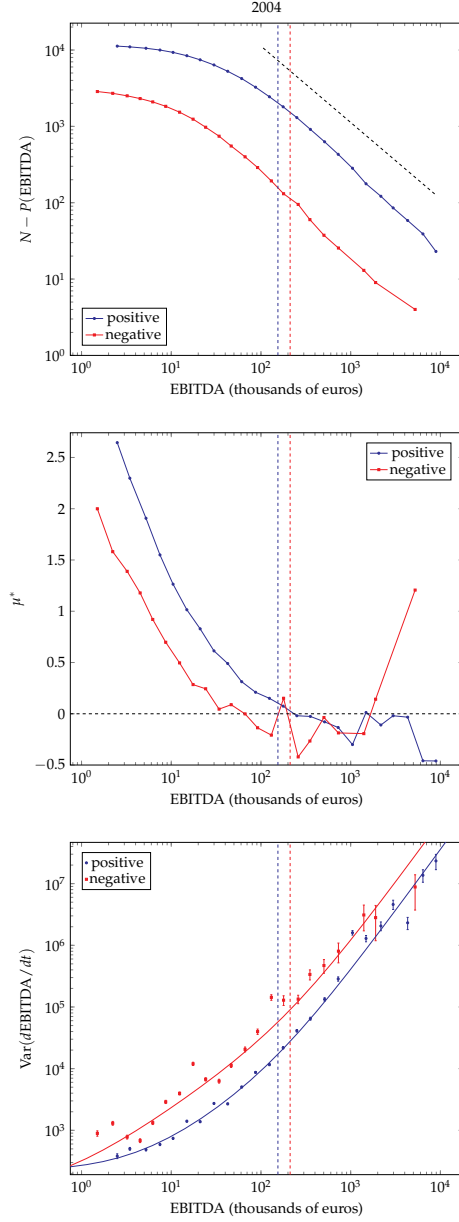

Figure 42: Balearic islands

Rank plot, chemical potential and variance.

11800 Firms with positive EBITDA

$T_1 = 0.35 \pm 0.05$ ,  $T_{1/2} = 54.77 \pm 6.21$ , and  $T_0 = 214.90 \pm 66.26$

3243 Firms with negative EBITDA

Negative EBITDA:

$T_1 = 1.01 \pm 0.61$ ,  $T_{1/2} = 212.72 \pm 45.25$ , and  $T_0 = 106.42 \pm 232.83$ .

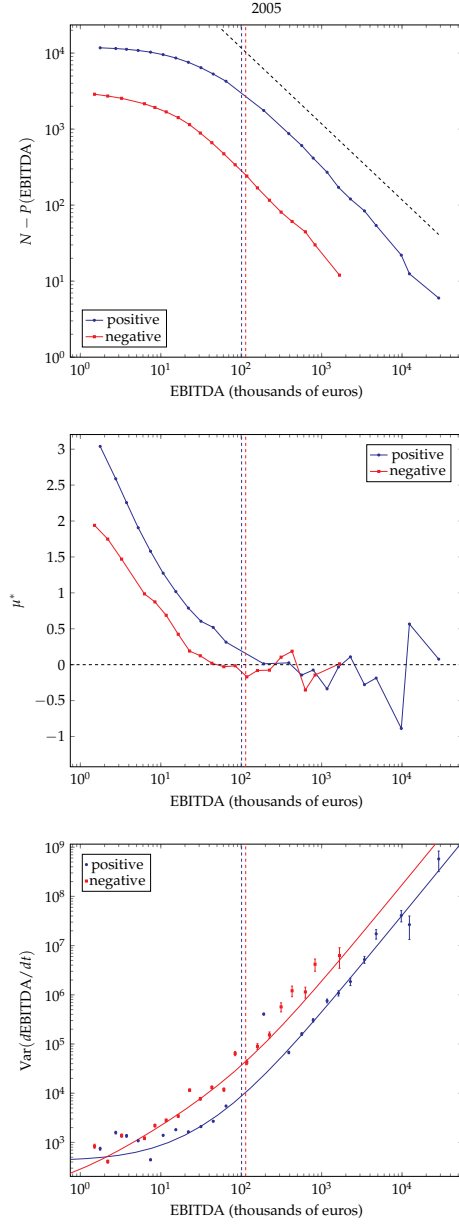

Figure 43: Balearic islands

Rank plot, chemical potential and variance.

12071 Firms with positive EBITDA

$T_1 = 0.41 \pm 0.13$ ,  $T_{1/2} = 41.22 \pm 13.74$ , and  $T_0 = 419.99 \pm 175.33$

3221 Firms with negative EBITDA

Negative EBITDA:

$T_1 = 1.70 \pm 0.84$ ,  $T_{1/2} = 193.80 \pm 40.79$ , and  $T_0 = 90.35 \pm 157.19$ .

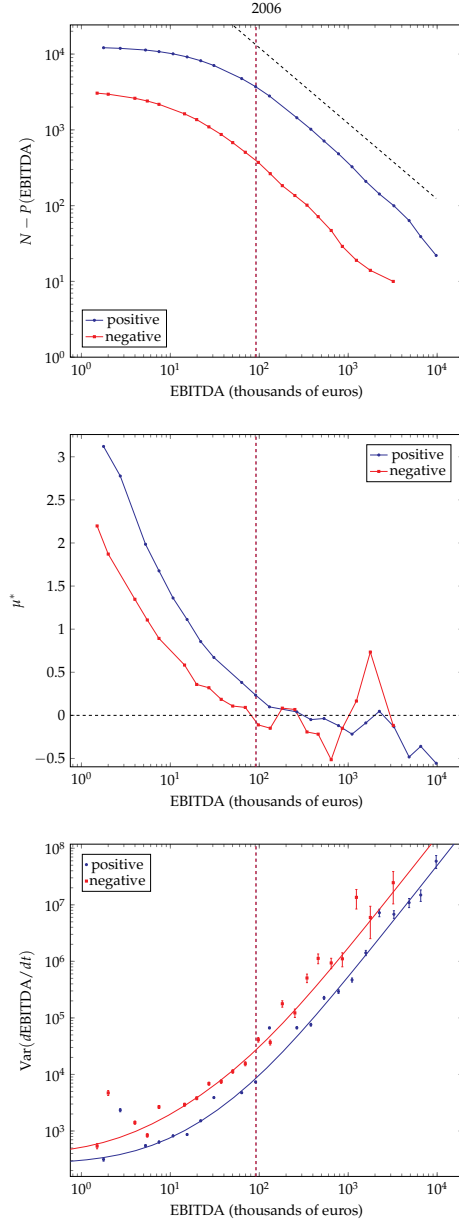

Figure 44: Balearic islands

Rank plot, chemical potential and variance.

12450 Firms with positive EBITDA

$T_1 = 0.49 \pm 0.12$ ,  $T_{1/2} = 45.35 \pm 12.47$ , and  $T_0 = 256.95 \pm 130.77$

3393 Firms with negative EBITDA

Negative EBITDA:

$T_1 = 1.59 \pm 0.56$ ,  $T_{1/2} = 145.71 \pm 33.84$ , and  $T_0 = 365.48 \pm 196.13$ .

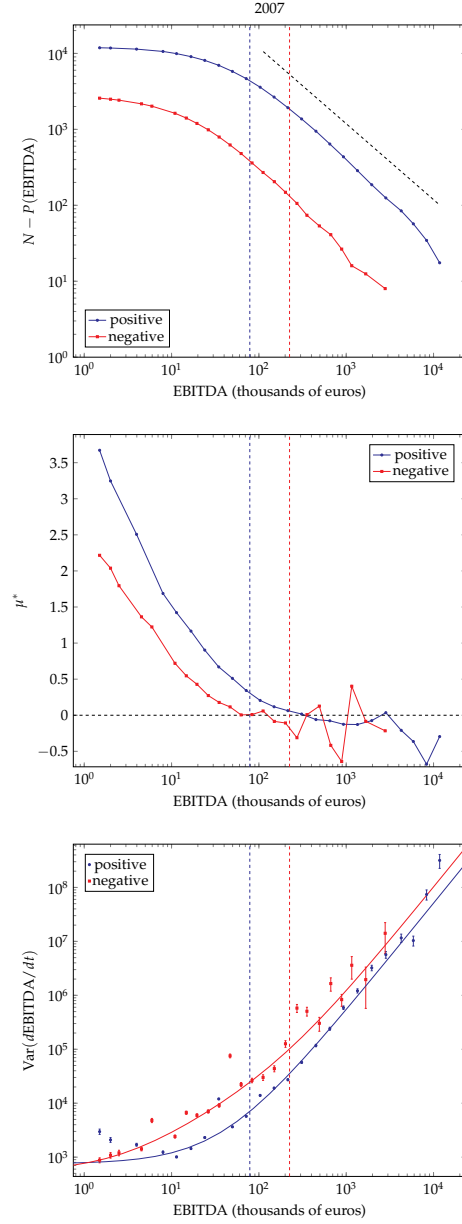

Figure 45: Balearic islands

Rank plot, chemical potential and variance.

12081 Firms with positive EBITDA

$T_1 = 0.51 \pm 0.11$ ,  $T_{1/2} = 39.93 \pm 16.79$ , and  $T_0 = 751.51 \pm 281.20$

2875 Firms with negative EBITDA

Negative EBITDA:

$T_1 = 1.00 \pm 0.51$ ,  $T_{1/2} = 224.82 \pm 40.50$ , and  $T_0 = 541.95 \pm 250.57$ .

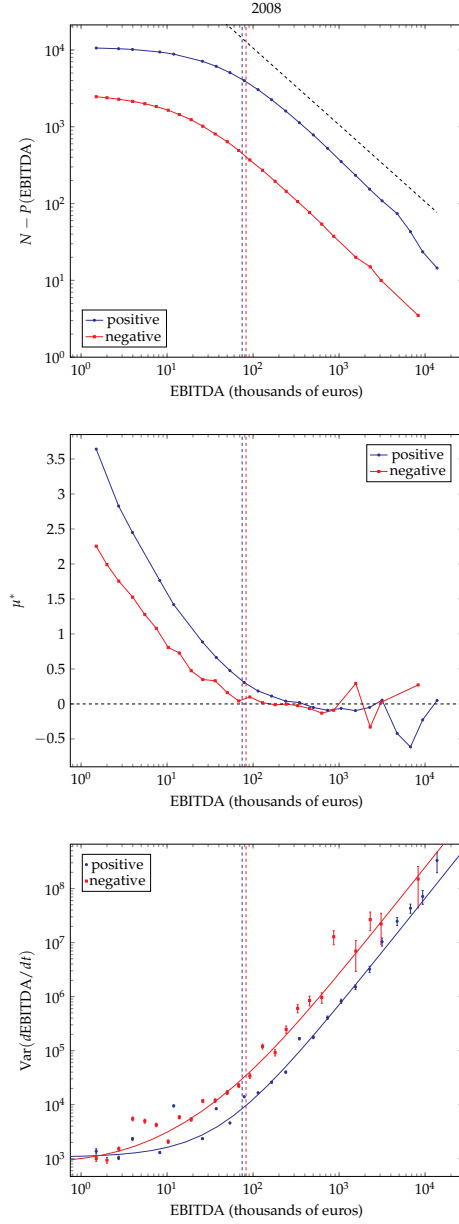

Figure 46: Balearic islands

Rank plot, chemical potential and variance.

10794 Firms with positive EBITDA

$T_1 = 0.66 \pm 0.15$ ,  $T_{1/2} = 48.93 \pm 21.33$ , and  $T_0 = 1061.51 \pm 377.54$

2682 Firms with negative EBITDA

Negative EBITDA:

$T_1 = 2.47 \pm 0.84$ ,  $T_{1/2} = 204.36 \pm 51.11$ , and  $T_0 = 797.82 \pm 303.62$ .

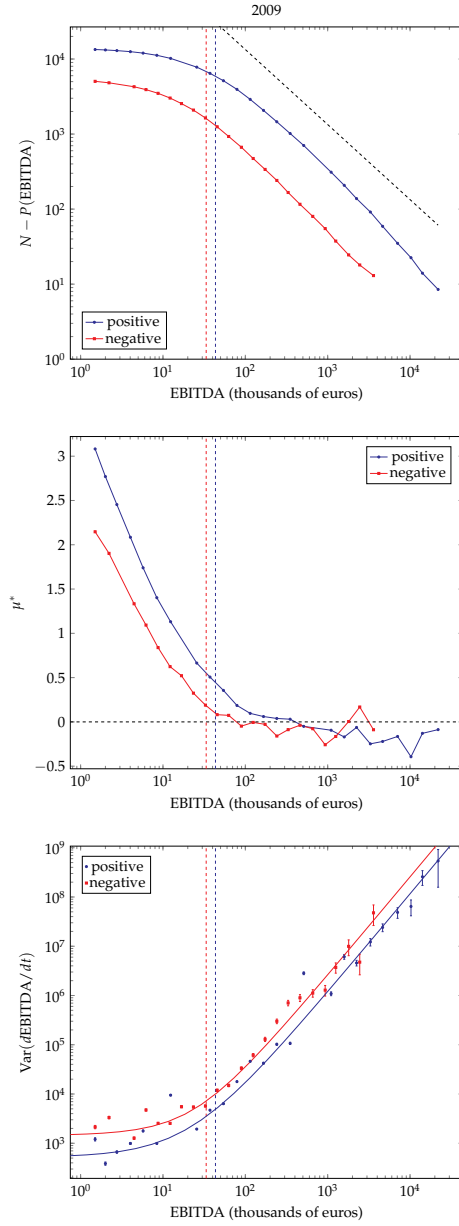

Figure 47: Balearic islands

Rank plot, chemical potential and variance.

13852 Firms with positive EBITDA

$T_1 = 1.16 \pm 0.29$ ,  $T_{1/2} = 50.21 \pm 22.03$ , and  $T_0 = 520.08 \pm 199.66$

5507 Firms with negative EBITDA

Negative EBITDA:

$T_1 = 2.55 \pm 0.69$ ,  $T_{1/2} = 85.52 \pm 42.33$ , and  $T_0 = 1434.99 \pm 367.10$ .

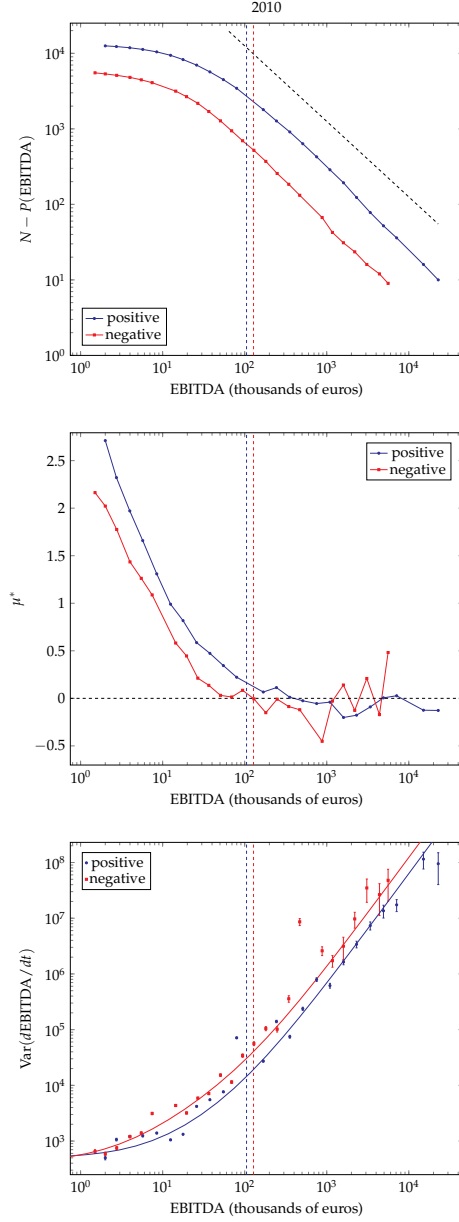

Figure 48: Balearic islands

Rank plot, chemical potential and variance.

13145 Firms with positive EBITDA

$T_1 = 0.63 \pm 0.19$ ,  $T_{1/2} = 65.93 \pm 22.25$ , and  $T_0 = 490.92 \pm 251.73$

6033 Firms with negative EBITDA

Negative EBITDA:

$T_1 = 1.22 \pm 0.45$ ,  $T_{1/2} = 155.86 \pm 27.09$ , and  $T_0 = 408.94 \pm 132.42$ .

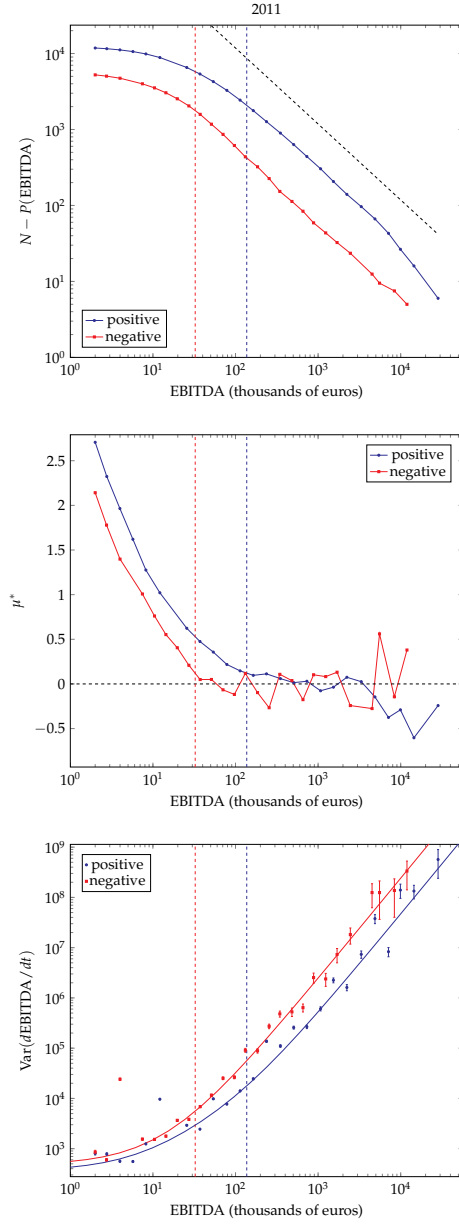

Figure 49: Balearic islands

Rank plot, chemical potential and variance.

12437 Firms with positive EBITDA

$T_1 = 0.46 \pm 0.16$ ,  $T_{1/2} = 63.57 \pm 18.19$ , and  $T_0 = 364.13 \pm 174.51$

5812 Firms with negative EBITDA

Negative EBITDA:

$T_1 = 2.41 \pm 0.55$ ,  $T_{1/2} = 78.20 \pm 26.49$ , and  $T_0 = 477.38 \pm 192.76$ .

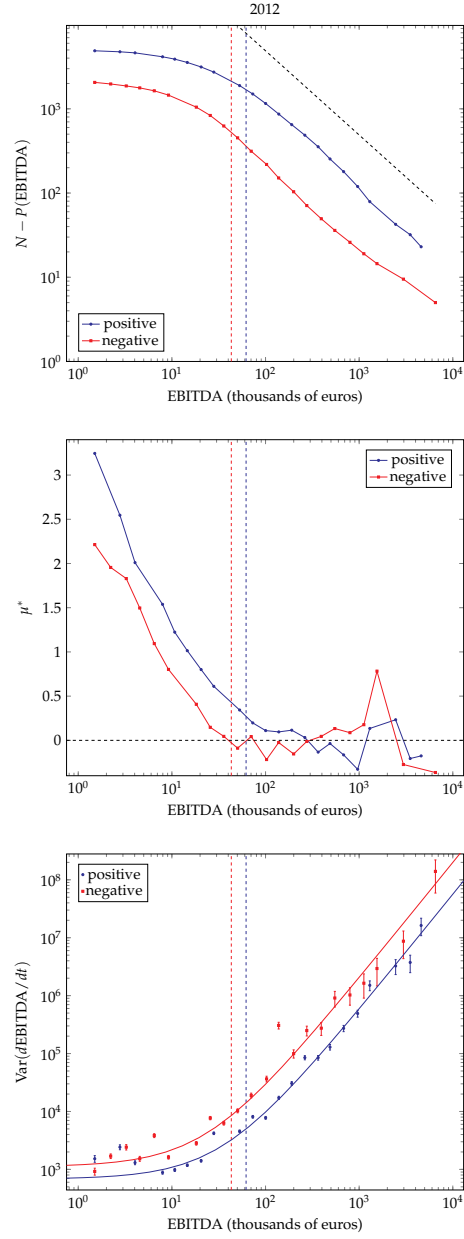

Figure 50: Balearic islands

Rank plot, chemical potential and variance.

5051 Firms with positive EBITDA

$T_1 = 0.56 \pm 0.11$ ,  $T_{1/2} = 34.76 \pm 14.82$ , and  $T_0 = 679.14 \pm 206.87$

2197 Firms with negative EBITDA

Negative EBITDA:

$T_1 = 1.99 \pm 0.56$ ,  $T_{1/2} = 85.70 \pm 33.94$ , and  $T_0 = 1109.74 \pm 276.49$ .

# Basque country

## Tables of Temperatures

### Positive EBITDA

| Year | $T_1$           | $T_{1/2}$          | $T_0$               | $T_{1/2}/T_1$ | Num. Firms |
|------|-----------------|--------------------|---------------------|---------------|------------|
| 2003 | $0.15 \pm 0.05$ | $79.55 \pm 11.35$  | $198.91 \pm 131.45$ | 537.1         | 19408      |
| 2004 | $0.26 \pm 0.07$ | $82.73 \pm 9.07$   | $176.10 \pm 87.26$  | 319.4         | 19878      |
| 2005 | $0.54 \pm 0.10$ | $56.15 \pm 15.87$  | $628.41 \pm 233.39$ | 103.8         | 20989      |
| 2006 | $0.50 \pm 0.10$ | $81.11 \pm 12.65$  | $293.50 \pm 125.24$ | 161.4         | 22313      |
| 2007 | $0.52 \pm 0.09$ | $57.00 \pm 12.63$  | $377.48 \pm 189.34$ | 108.6         | 22219      |
| 2008 | $0.87 \pm 0.19$ | $71.78 \pm 20.29$  | $501.67 \pm 247.38$ | 82.4          | 20441      |
| 2009 | $0.86 \pm 0.18$ | $152.17 \pm 25.48$ | $536.93 \pm 312.23$ | 176.9         | 21588      |
| 2010 | $0.85 \pm 0.20$ | $106.88 \pm 23.98$ | $549.07 \pm 205.42$ | 126.2         | 22587      |
| 2011 | $0.95 \pm 0.24$ | $187.83 \pm 29.18$ | $513.94 \pm 258.58$ | 198.2         | 20060      |
| 2012 | $0.30 \pm 0.09$ | $100.10 \pm 13.82$ | $491.02 \pm 156.71$ | 333.8         | 12961      |

### Negative EBITDA

| Year | $T_1$           | $T_{1/2}$           | $T_0$               | $T_{1/2}/T_1$ | Num. Firms |
|------|-----------------|---------------------|---------------------|---------------|------------|
| 2003 | $0.20 \pm 0.20$ | $299.28 \pm 43.04$  | $118.42 \pm 136.22$ | 1472.0        | 4885       |
| 2004 | $0.86 \pm 0.36$ | $187.89 \pm 27.92$  | $164.73 \pm 112.46$ | 219.7         | 5007       |
| 2005 | $1.36 \pm 0.43$ | $236.38 \pm 31.44$  | $261.73 \pm 157.29$ | 174.3         | 5379       |
| 2006 | $1.62 \pm 0.58$ | $243.86 \pm 43.75$  | $140.80 \pm 210.49$ | 150.7         | 5887       |
| 2007 | $1.41 \pm 0.59$ | $342.29 \pm 46.55$  | $17.72 \pm 173.69$  | 242.2         | 5002       |
| 2008 | $1.65 \pm 0.73$ | $354.43 \pm 77.25$  | $211.75 \pm 403.47$ | 214.9         | 4752       |
| 2009 | $3.78 \pm 0.91$ | $307.34 \pm 47.99$  | $318.24 \pm 222.45$ | 81.4          | 7048       |
| 2010 | $2.30 \pm 1.17$ | $312.54 \pm 121.22$ | $484.03 \pm 532.31$ | 135.7         | 9039       |
| 2011 | $1.97 \pm 0.64$ | $382.01 \pm 47.52$  | $799.54 \pm 266.99$ | 194.2         | 7989       |
| 2012 | $1.84 \pm 0.44$ | $141.24 \pm 30.74$  | $897.55 \pm 233.26$ | 76.6          | 5651       |

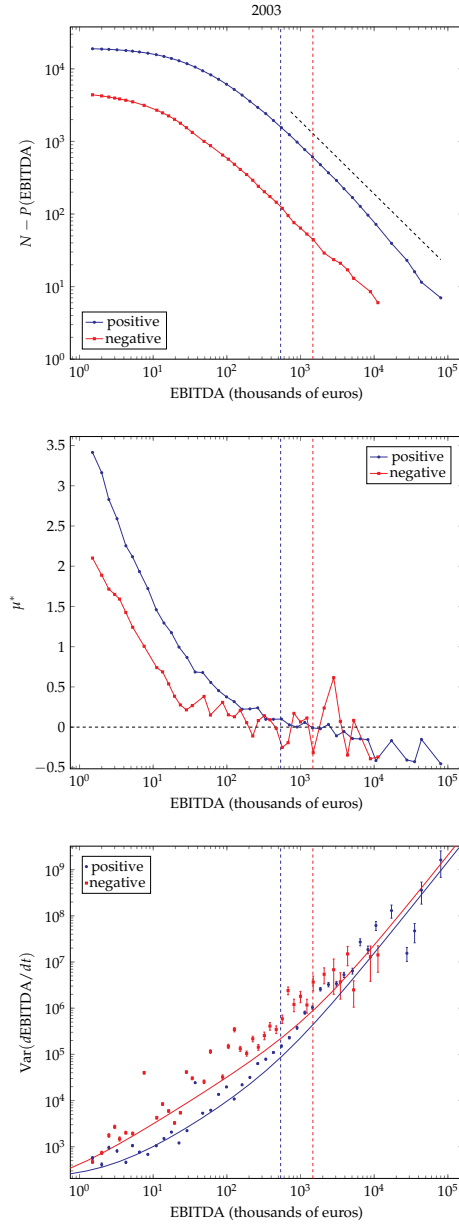

Figure 51: Basque country

Rank plot, chemical potential and variance.

19408 Firms with positive EBITDA

$T_1 = 0.15 \pm 0.05$ ,  $T_{1/2} = 79.55 \pm 11.35$ , and  $T_0 = 198.91 \pm 131.45$

4885 Firms with negative EBITDA

Negative EBITDA:

$T_1 = 0.20 \pm 0.20$ ,  $T_{1/2} = 299.28 \pm 43.04$ , and  $T_0 = 118.42 \pm 136.22$ .

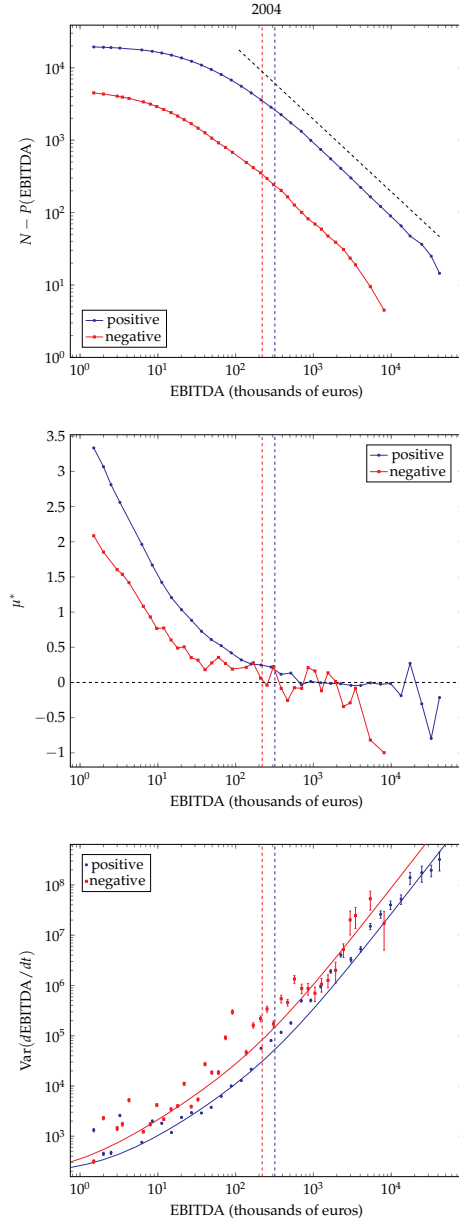

Figure 52: Basque country

Rank plot, chemical potential and variance.

19878 Firms with positive EBITDA

$T_1 = 0.26 \pm 0.07$ ,  $T_{1/2} = 82.73 \pm 9.07$ , and  $T_0 = 176.10 \pm 87.26$

5007 Firms with negative EBITDA

Negative EBITDA:

$T_1 = 0.86 \pm 0.36$ ,  $T_{1/2} = 187.89 \pm 27.92$ , and  $T_0 = 164.73 \pm 112.46$ .

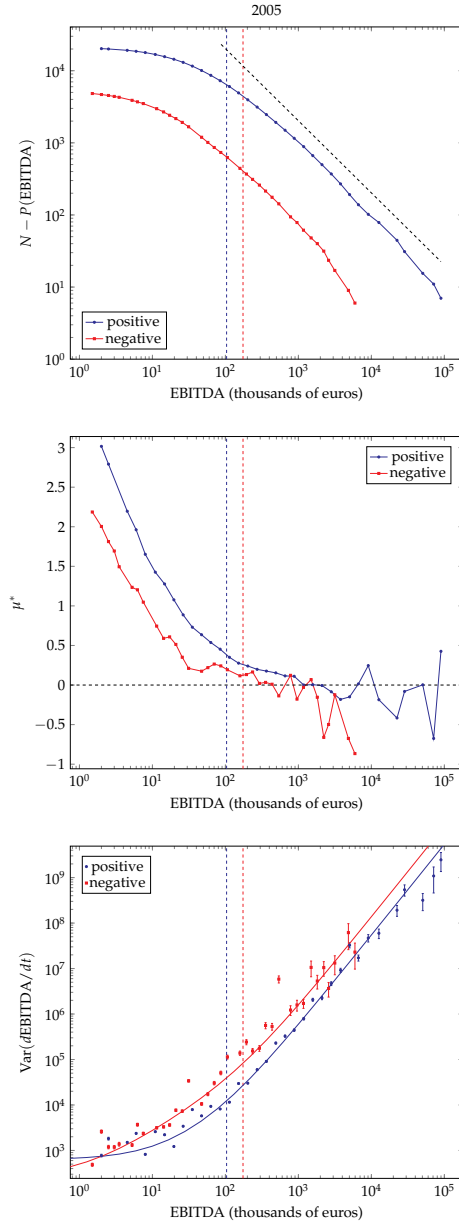

Figure 53: Basque country

Rank plot, chemical potential and variance.

20989 Firms with positive EBITDA

$T_1 = 0.54 \pm 0.10$ ,  $T_{1/2} = 56.15 \pm 15.87$ , and  $T_0 = 628.41 \pm 233.39$

5379 Firms with negative EBITDA

Negative EBITDA:

$T_1 = 1.36 \pm 0.43$ ,  $T_{1/2} = 236.38 \pm 31.44$ , and  $T_0 = 261.73 \pm 157.29$ .

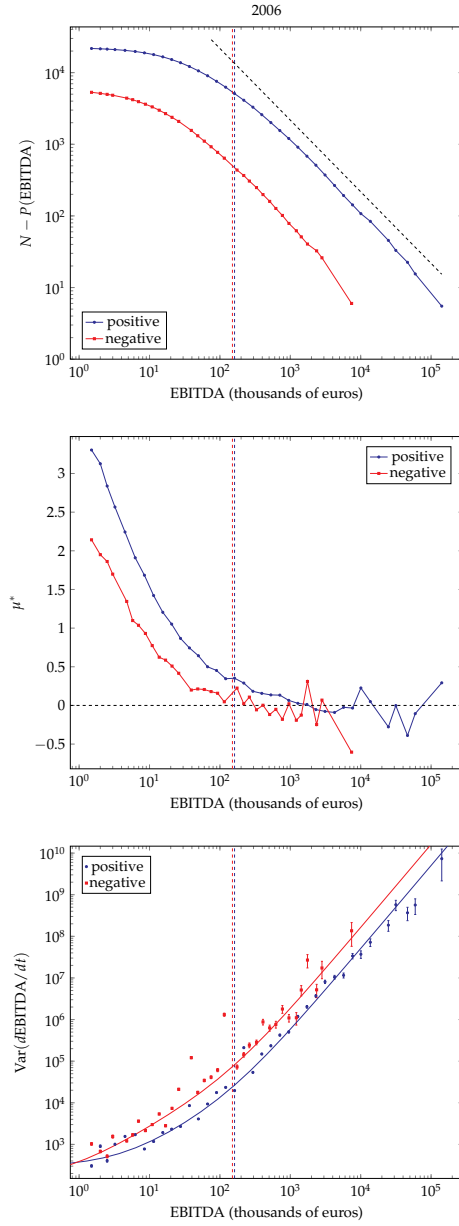

Figure 54: Basque country

Rank plot, chemical potential and variance.

22313 Firms with positive EBITDA

$T_1 = 0.50 \pm 0.10$ ,  $T_{1/2} = 81.11 \pm 12.65$ , and  $T_0 = 293.50 \pm 125.24$

5887 Firms with negative EBITDA

Negative EBITDA:

$T_1 = 1.62 \pm 0.58$ ,  $T_{1/2} = 243.86 \pm 43.75$ , and  $T_0 = 140.80 \pm 210.49$ .

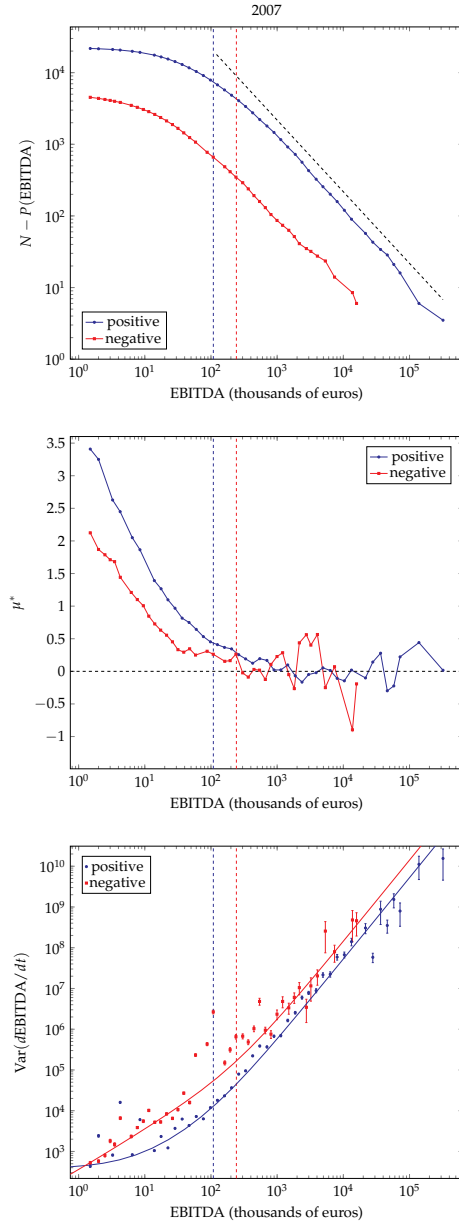

Figure 55: Basque country

Rank plot, chemical potential and variance.

22219 Firms with positive EBITDA

$T_1 = 0.52 \pm 0.09$ ,  $T_{1/2} = 57.00 \pm 12.63$ , and  $T_0 = 377.48 \pm 189.34$

5002 Firms with negative EBITDA

Negative EBITDA:

$T_1 = 1.41 \pm 0.59$ ,  $T_{1/2} = 342.29 \pm 46.55$ , and  $T_0 = 17.72 \pm 173.69$ .

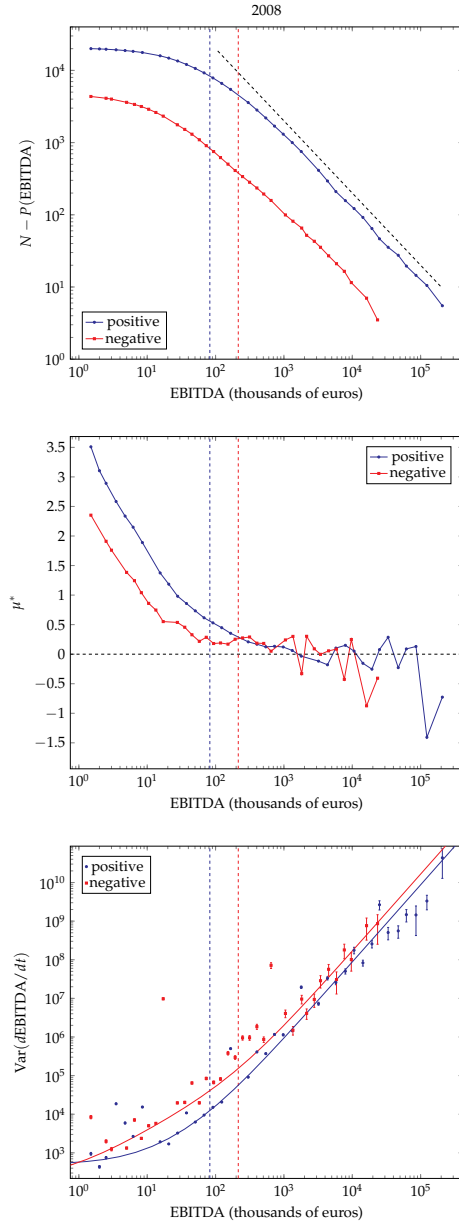

Figure 56: Basque country

Rank plot, chemical potential and variance.

20441 Firms with positive EBITDA

$T_1 = 0.87 \pm 0.19$ ,  $T_{1/2} = 71.78 \pm 20.29$ , and  $T_0 = 501.67 \pm 247.38$

4752 Firms with negative EBITDA

Negative EBITDA:

$T_1 = 1.65 \pm 0.73$ ,  $T_{1/2} = 354.43 \pm 77.25$ , and  $T_0 = 211.75 \pm 403.47$ .

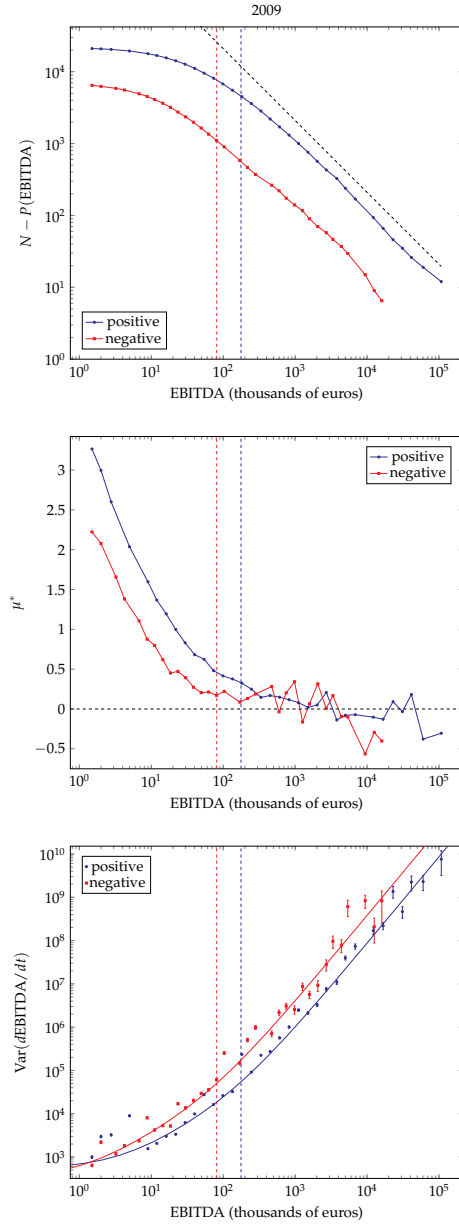

Figure 57: Basque country

Rank plot, chemical potential and variance.

21588 Firms with positive EBITDA

$T_1 = 0.86 \pm 0.18$ ,  $T_{1/2} = 152.17 \pm 25.48$ , and  $T_0 = 536.93 \pm 312.23$

7048 Firms with negative EBITDA

Negative EBITDA:

$T_1 = 3.78 \pm 0.91$ ,  $T_{1/2} = 307.34 \pm 47.99$ , and  $T_0 = 318.24 \pm 222.45$ .

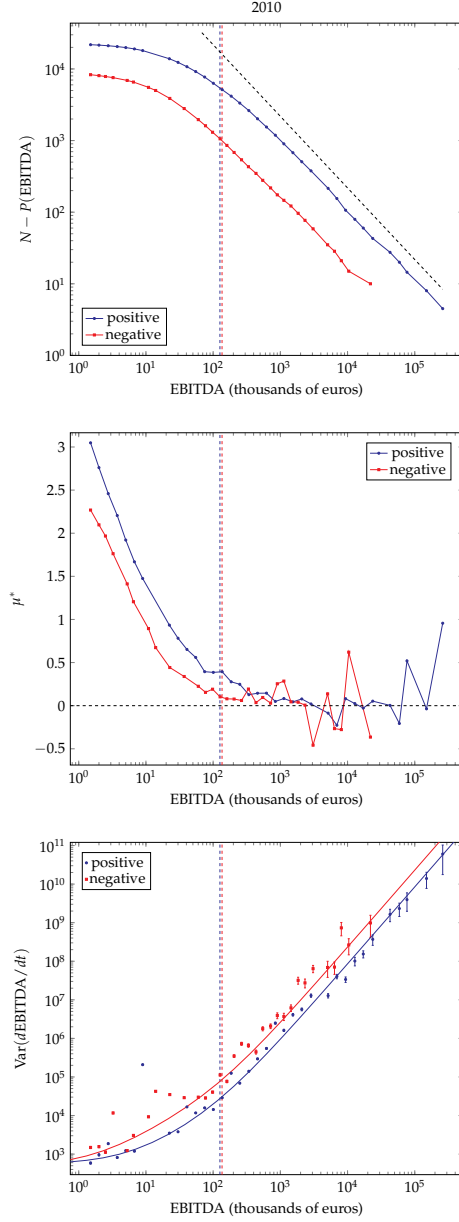

Figure 58: Basque country

Rank plot, chemical potential and variance.

22587 Firms with positive EBITDA

$T_1 = 0.85 \pm 0.20$ ,  $T_{1/2} = 106.88 \pm 23.98$ , and  $T_0 = 549.07 \pm 205.42$

9039 Firms with negative EBITDA

Negative EBITDA:

$T_1 = 2.30 \pm 1.17$ ,  $T_{1/2} = 312.54 \pm 121.22$ , and  $T_0 = 484.03 \pm 532.31$ .

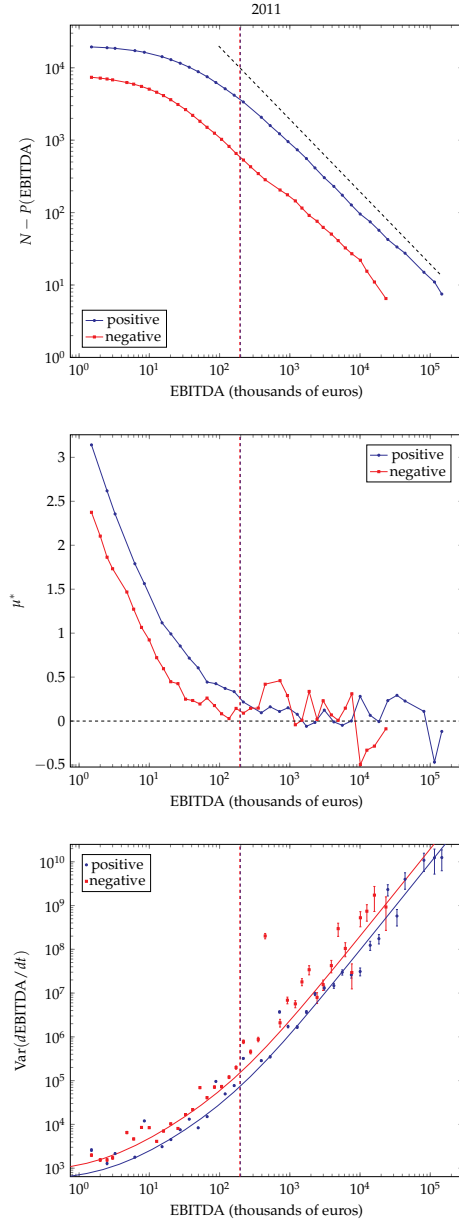

Figure 59: Basque country

Rank plot, chemical potential and variance.

20060 Firms with positive EBITDA

$T_1 = 0.95 \pm 0.24$ ,  $T_{1/2} = 187.83 \pm 29.18$ , and  $T_0 = 513.94 \pm 258.58$

7989 Firms with negative EBITDA

Negative EBITDA:

$T_1 = 1.97 \pm 0.64$ ,  $T_{1/2} = 382.01 \pm 47.52$ , and  $T_0 = 799.54 \pm 266.99$ .

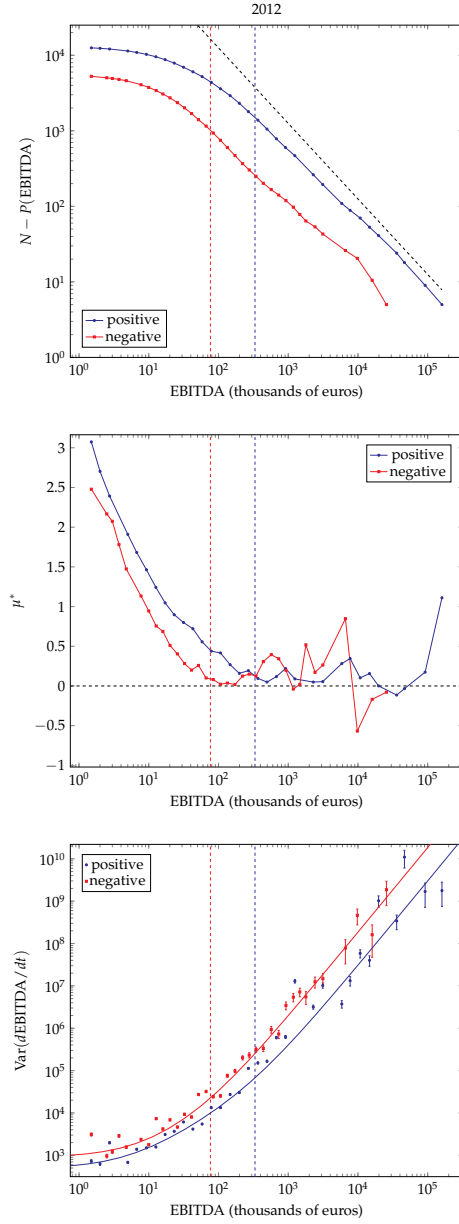

Figure 60: Basque country

Rank plot, chemical potential and variance.

12961 Firms with positive EBITDA

$T_1 = 0.30 \pm 0.09$ ,  $T_{1/2} = 100.10 \pm 13.82$ , and  $T_0 = 491.02 \pm 156.71$

5651 Firms with negative EBITDA

Negative EBITDA:

$T_1 = 1.84 \pm 0.44$ ,  $T_{1/2} = 141.24 \pm 30.74$ , and  $T_0 = 897.55 \pm 233.26$ .

# Canary islands

## Tables of Temperatures

### Positive EBITDA

| Year | $T_1$           | $T_{1/2}$          | $T_0$                | $T_{1/2}/T_1$ | Num. Firms |
|------|-----------------|--------------------|----------------------|---------------|------------|
| 2003 | $0.55 \pm 0.13$ | $89.64 \pm 21.70$  | $486.96 \pm 302.36$  | 161.7         | 13429      |
| 2004 | $0.21 \pm 0.07$ | $110.82 \pm 16.26$ | $490.62 \pm 276.49$  | 522.4         | 14803      |
| 2005 | $0.41 \pm 0.12$ | $134.22 \pm 21.82$ | $392.61 \pm 208.23$  | 328.0         | 15948      |
| 2006 | $0.06 \pm 0.04$ | $181.92 \pm 18.84$ | $548.55 \pm 386.47$  | 2994.2        | 16221      |
| 2007 | $0.60 \pm 0.08$ | $93.05 \pm 14.23$  | $1175.17 \pm 285.58$ | 156.0         | 15918      |
| 2008 | $0.61 \pm 0.12$ | $174.31 \pm 25.71$ | $636.54 \pm 412.86$  | 286.1         | 13784      |
| 2009 | $0.71 \pm 0.17$ | $137.78 \pm 27.22$ | $791.26 \pm 303.37$  | 194.0         | 15869      |
| 2010 | $0.63 \pm 0.17$ | $119.58 \pm 25.74$ | $1128.71 \pm 354.37$ | 188.9         | 15248      |
| 2011 | $0.67 \pm 0.21$ | $112.87 \pm 28.20$ | $542.27 \pm 280.52$  | 169.4         | 14625      |
| 2012 | $0.55 \pm 0.07$ | $60.80 \pm 10.02$  | $1376.44 \pm 195.56$ | 110.6         | 8495       |

### Negative EBITDA

| Year | $T_1$           | $T_{1/2}$          | $T_0$                | $T_{1/2}/T_1$ | Num. Firms |
|------|-----------------|--------------------|----------------------|---------------|------------|
| 2003 | $1.77 \pm 0.63$ | $213.19 \pm 46.64$ | $0.08 \pm 161.29$    | 120.3         | 3207       |
| 2004 | $1.92 \pm 0.62$ | $186.92 \pm 40.14$ | $284.44 \pm 168.59$  | 97.5          | 3713       |
| 2005 | $1.44 \pm 0.47$ | $198.18 \pm 31.21$ | $601.46 \pm 179.62$  | 137.3         | 4287       |
| 2006 | $0.79 \pm 0.34$ | $252.95 \pm 47.02$ | $1247.71 \pm 495.60$ | 320.5         | 4258       |
| 2007 | $1.89 \pm 0.91$ | $370.15 \pm 97.64$ | $921.18 \pm 652.82$  | 195.5         | 4042       |
| 2008 | $2.93 \pm 0.84$ | $274.13 \pm 77.18$ | $798.06 \pm 515.96$  | 93.7          | 3833       |
| 2009 | $2.54 \pm 0.88$ | $220.46 \pm 67.78$ | $564.82 \pm 423.27$  | 86.6          | 6463       |
| 2010 | $2.38 \pm 0.71$ | $149.10 \pm 51.03$ | $973.13 \pm 474.58$  | 62.7          | 6806       |
| 2011 | $2.18 \pm 0.55$ | $125.38 \pm 34.44$ | $701.78 \pm 243.11$  | 57.4          | 6288       |
| 2012 | $1.92 \pm 0.62$ | $157.43 \pm 50.40$ | $975.86 \pm 491.90$  | 81.9          | 3573       |

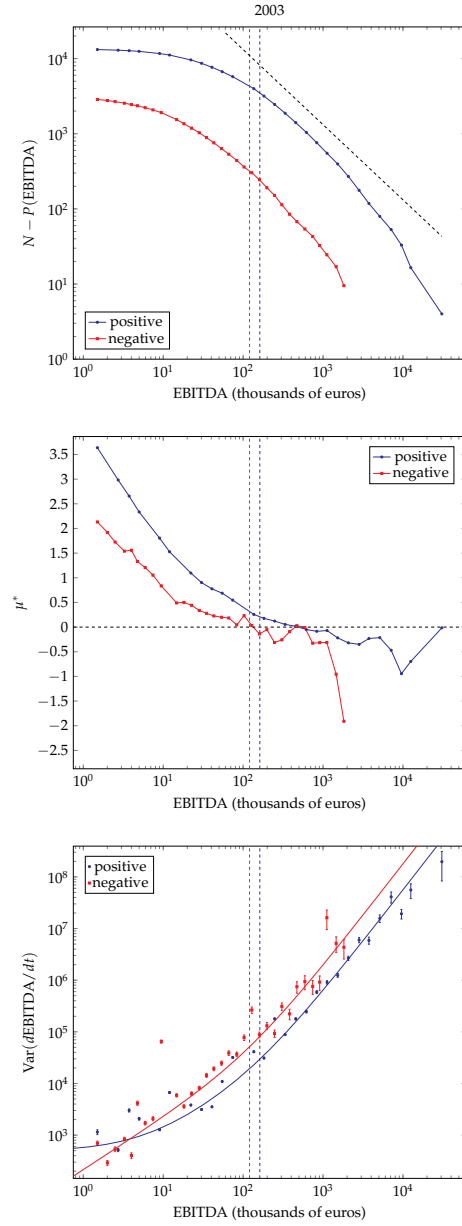

Figure 61: Canary islands

Rank plot, chemical potential and variance.

13429 Firms with positive EBITDA

$T_1 = 0.55 \pm 0.13$ ,  $T_{1/2} = 89.64 \pm 21.70$ , and  $T_0 = 486.96 \pm 302.36$

3207 Firms with negative EBITDA

Negative EBITDA:

$T_1 = 1.77 \pm 0.63$ ,  $T_{1/2} = 213.19 \pm 46.64$ , and  $T_0 = 0.08 \pm 161.29$ .

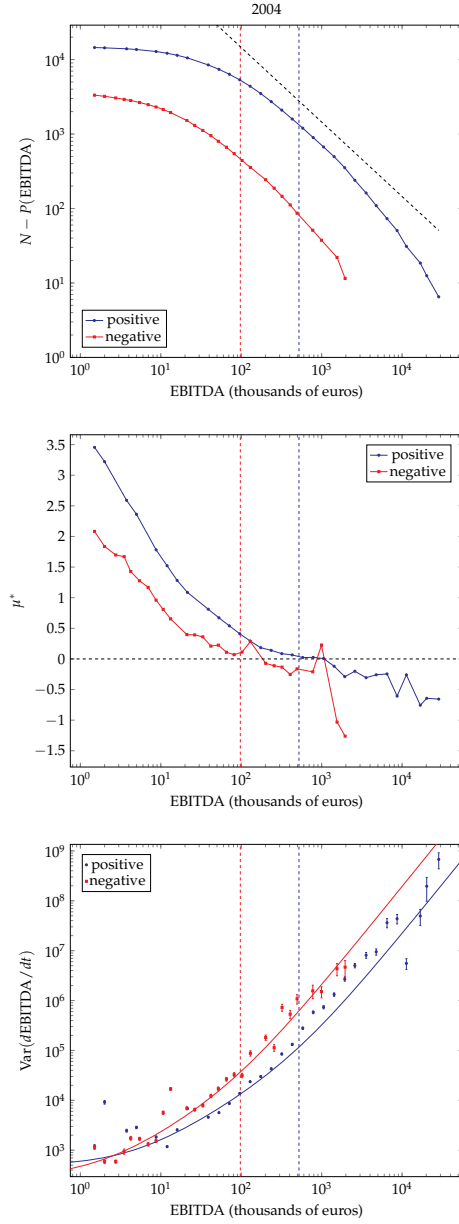

Figure 62: Canary islands

Rank plot, chemical potential and variance.

14803 Firms with positive EBITDA

$T_1 = 0.21 \pm 0.07$ ,  $T_{1/2} = 110.82 \pm 16.26$ , and  $T_0 = 490.62 \pm 276.49$

3713 Firms with negative EBITDA

Negative EBITDA:

$T_1 = 1.92 \pm 0.62$ ,  $T_{1/2} = 186.92 \pm 40.14$ , and  $T_0 = 284.44 \pm 168.59$ .

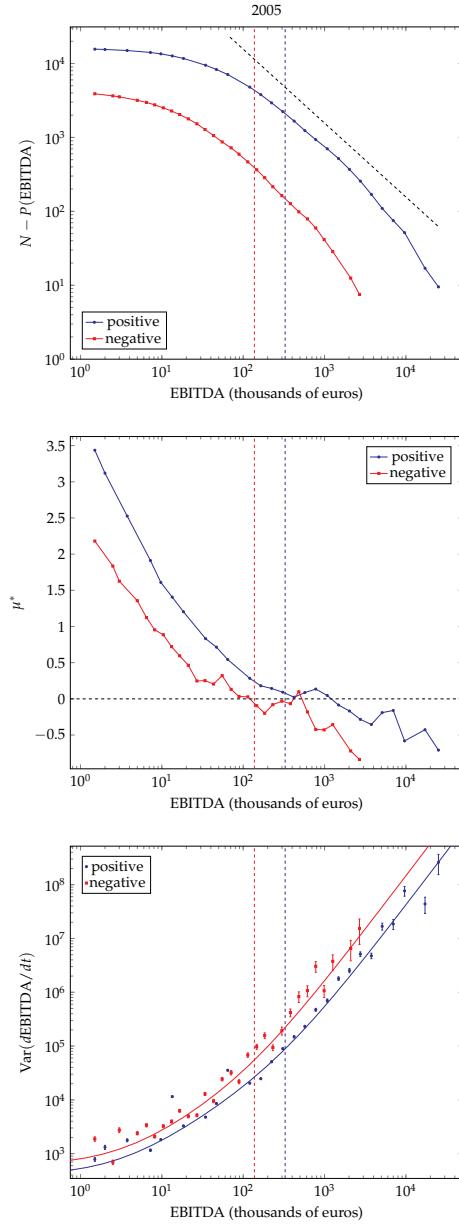

Figure 63: Canary islands

Rank plot, chemical potential and variance.

15948 Firms with positive EBITDA

$T_1 = 0.41 \pm 0.12$ ,  $T_{1/2} = 134.22 \pm 21.82$ , and  $T_0 = 392.61 \pm 208.23$

4287 Firms with negative EBITDA

Negative EBITDA:

$T_1 = 1.44 \pm 0.47$ ,  $T_{1/2} = 198.18 \pm 31.21$ , and  $T_0 = 601.46 \pm 179.62$ .

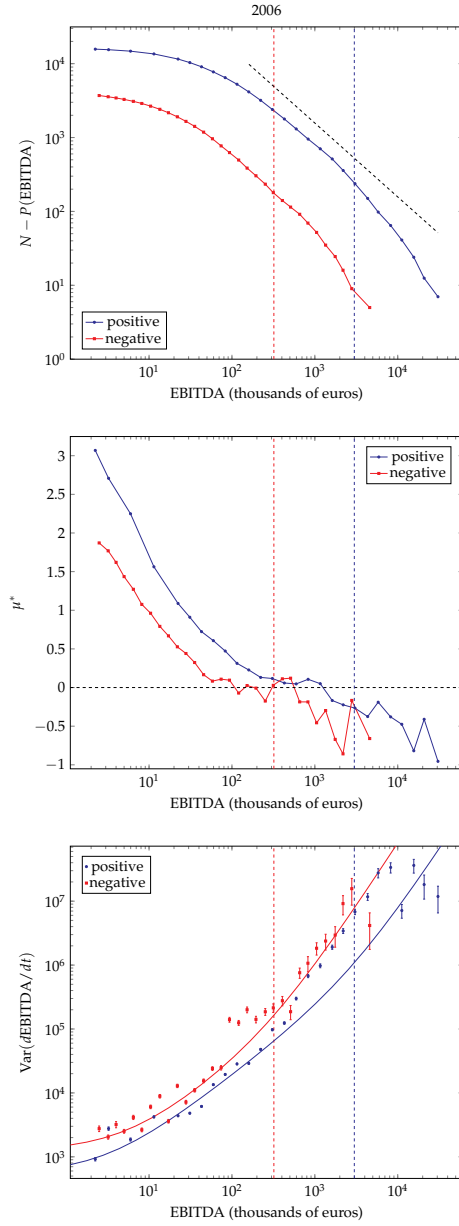

Figure 64: Canary islands

Rank plot, chemical potential and variance.

16221 Firms with positive EBITDA

$T_1 = 0.06 \pm 0.04$ ,  $T_{1/2} = 181.92 \pm 18.84$ , and  $T_0 = 548.55 \pm 386.47$

4258 Firms with negative EBITDA

Negative EBITDA:

$T_1 = 0.79 \pm 0.34$ ,  $T_{1/2} = 252.95 \pm 47.02$ , and  $T_0 = 1247.71 \pm 495.60$ .

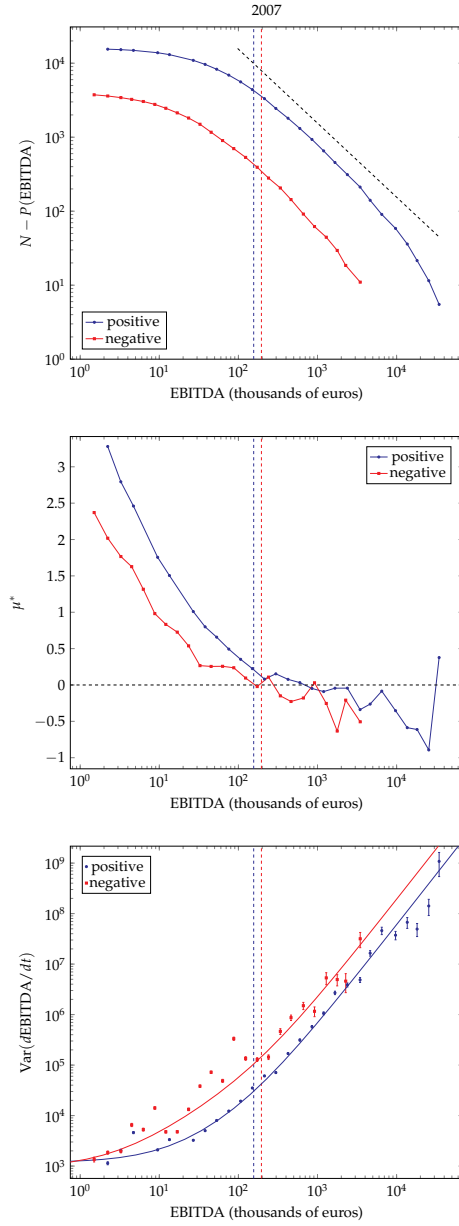

Figure 65: Canary islands

Rank plot, chemical potential and variance.

15918 Firms with positive EBITDA

$T_1 = 0.60 \pm 0.08$ ,  $T_{1/2} = 93.05 \pm 14.23$ , and  $T_0 = 1175.17 \pm 285.58$

4042 Firms with negative EBITDA

Negative EBITDA:

$T_1 = 1.89 \pm 0.91$ ,  $T_{1/2} = 370.15 \pm 97.64$ , and  $T_0 = 921.18 \pm 652.82$ .

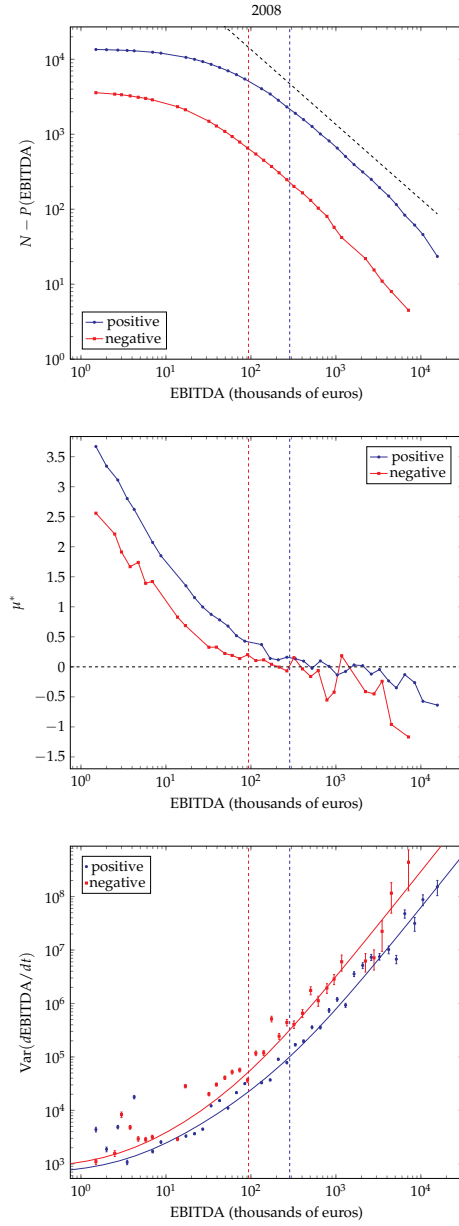

Figure 66: Canary islands

Rank plot, chemical potential and variance.

13784 Firms with positive EBITDA

$T_1 = 0.61 \pm 0.12$ ,  $T_{1/2} = 174.31 \pm 25.71$ , and  $T_0 = 636.54 \pm 412.86$

3833 Firms with negative EBITDA

Negative EBITDA:

$T_1 = 2.93 \pm 0.84$ ,  $T_{1/2} = 274.13 \pm 77.18$ , and  $T_0 = 798.06 \pm 515.96$ .

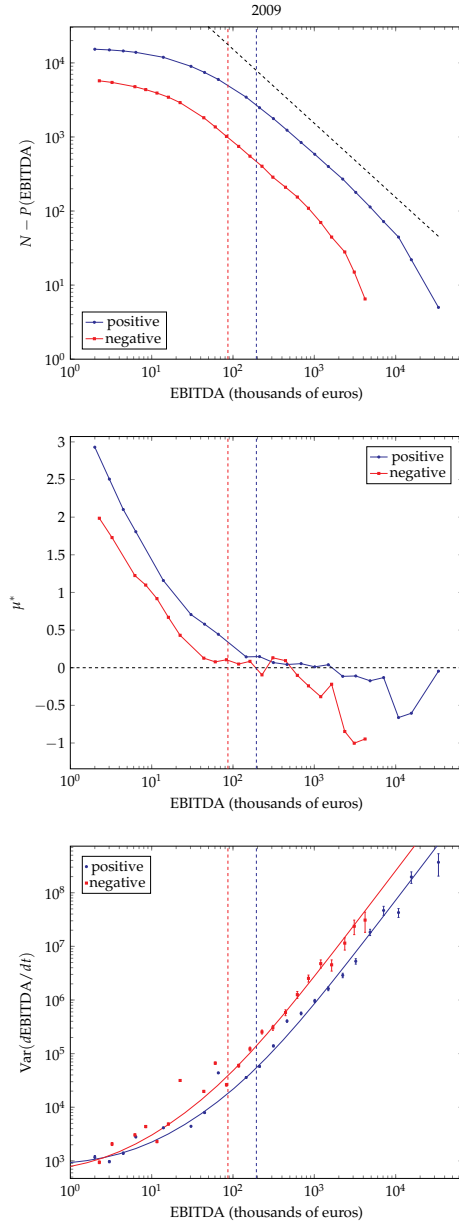

Figure 67: Canary islands

Rank plot, chemical potential and variance.

15869 Firms with positive EBITDA

$T_1 = 0.71 \pm 0.17$ ,  $T_{1/2} = 137.78 \pm 27.22$ , and  $T_0 = 791.26 \pm 303.37$

6463 Firms with negative EBITDA

Negative EBITDA:

$T_1 = 2.54 \pm 0.88$ ,  $T_{1/2} = 220.46 \pm 67.78$ , and  $T_0 = 564.82 \pm 423.27$ .

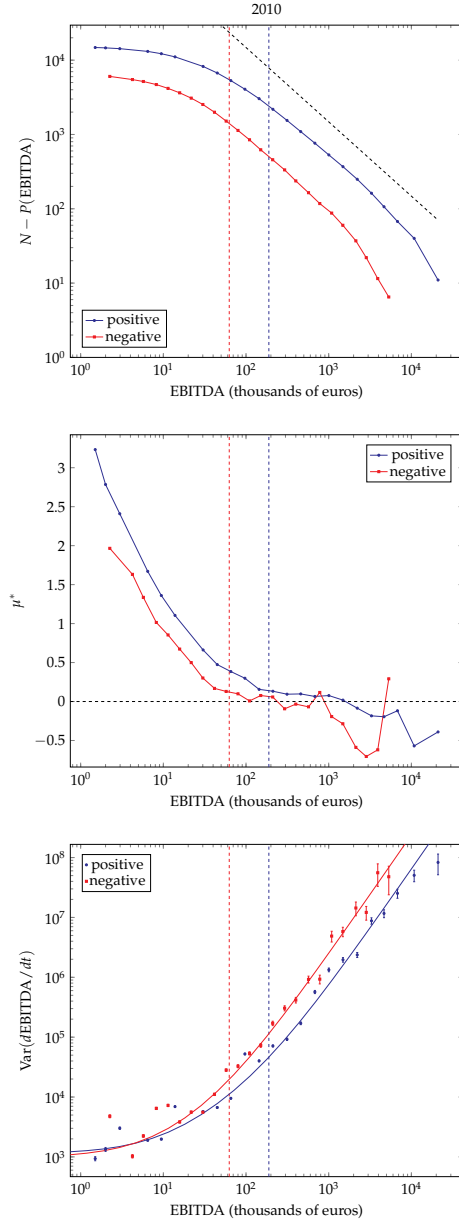

Figure 68: Canary islands

Rank plot, chemical potential and variance.

15248 Firms with positive EBITDA

$T_1 = 0.63 \pm 0.17$ ,  $T_{1/2} = 119.58 \pm 25.74$ , and  $T_0 = 1128.71 \pm 354.37$

6806 Firms with negative EBITDA

Negative EBITDA:

$T_1 = 2.38 \pm 0.71$ ,  $T_{1/2} = 149.10 \pm 51.03$ , and  $T_0 = 973.13 \pm 474.58$ .

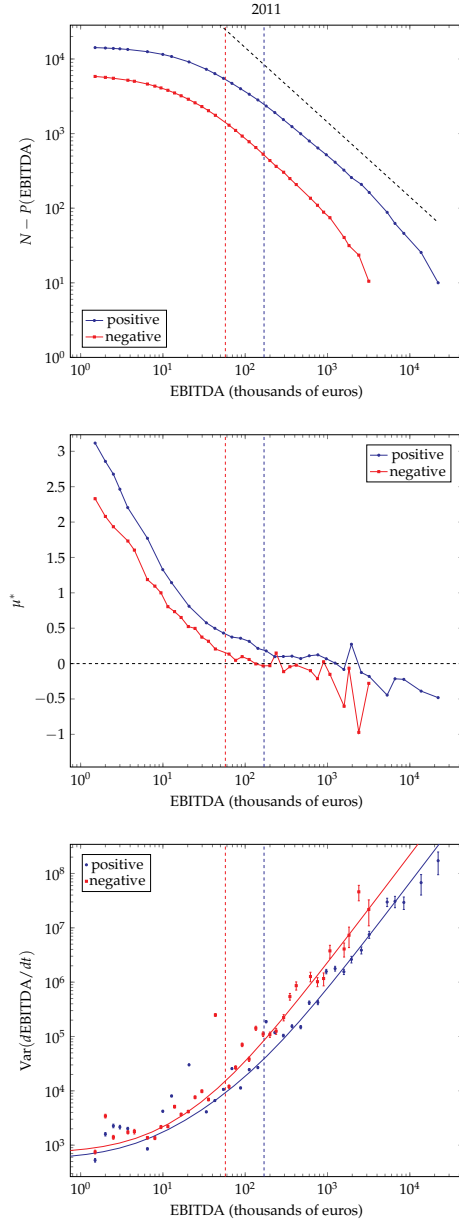

Figure 69: Canary islands

Rank plot, chemical potential and variance.

14625 Firms with positive EBITDA

$T_1 = 0.67 \pm 0.21$ ,  $T_{1/2} = 112.87 \pm 28.20$ , and  $T_0 = 542.27 \pm 280.52$

6288 Firms with negative EBITDA

Negative EBITDA:

$T_1 = 2.18 \pm 0.55$ ,  $T_{1/2} = 125.38 \pm 34.44$ , and  $T_0 = 701.78 \pm 243.11$ .

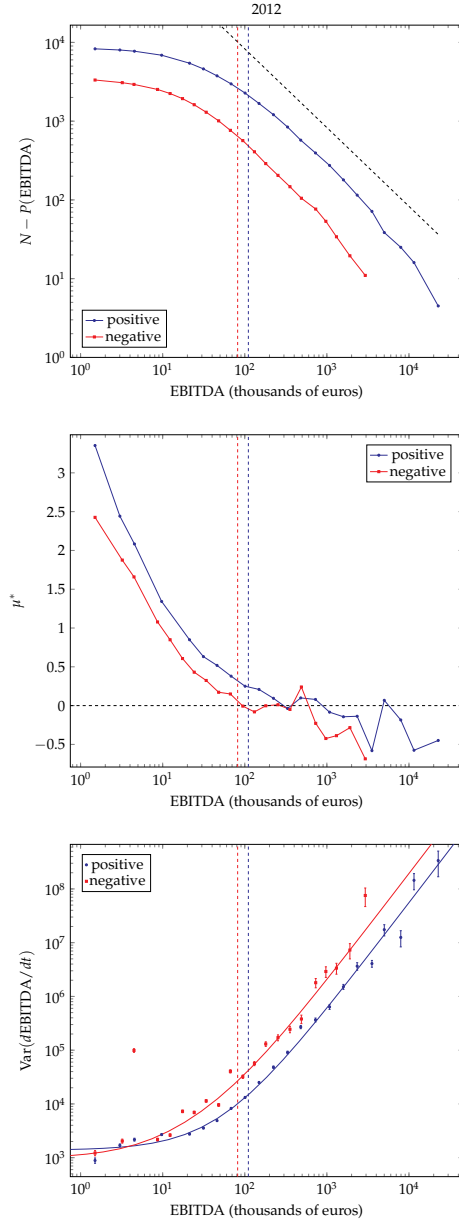

Figure 70: Canary islands

Rank plot, chemical potential and variance.

8495 Firms with positive EBITDA

$T_1 = 0.55 \pm 0.07$ ,  $T_{1/2} = 60.80 \pm 10.02$ , and  $T_0 = 1376.44 \pm 195.56$

3573 Firms with negative EBITDA

Negative EBITDA:

$T_1 = 1.92 \pm 0.62$ ,  $T_{1/2} = 157.43 \pm 50.40$ , and  $T_0 = 975.86 \pm 491.90$ .

# Cantabria

## Tables of Temperatures

### Positive EBITDA

| Year | $T_1$           | $T_{1/2}$          | $T_0$                | $T_{1/2}/T_1$ | Num. Firms |
|------|-----------------|--------------------|----------------------|---------------|------------|
| 2003 | $0.33 \pm 0.08$ | $41.88 \pm 9.49$   | $216.80 \pm 121.36$  | 127.3         | 3553       |
| 2004 | $0.24 \pm 0.09$ | $54.66 \pm 13.47$  | $236.89 \pm 172.46$  | 223.9         | 3475       |
| 2005 | $0.31 \pm 0.09$ | $40.75 \pm 13.67$  | $268.77 \pm 240.84$  | 131.7         | 3536       |
| 2006 | $0.30 \pm 0.10$ | $46.43 \pm 13.52$  | $120.19 \pm 165.38$  | 155.9         | 4011       |
| 2007 | $0.35 \pm 0.11$ | $26.80 \pm 14.29$  | $239.23 \pm 272.98$  | 76.1          | 4073       |
| 2008 | $0.26 \pm 0.11$ | $142.71 \pm 28.88$ | $708.99 \pm 426.21$  | 558.3         | 3769       |
| 2009 | $0.54 \pm 0.14$ | $57.94 \pm 18.50$  | $1096.54 \pm 311.02$ | 108.1         | 3937       |
| 2010 | $0.64 \pm 0.11$ | $35.76 \pm 11.89$  | $376.68 \pm 138.91$  | 55.7          | 4106       |
| 2011 | $0.76 \pm 0.20$ | $65.57 \pm 21.61$  | $738.68 \pm 277.06$  | 86.2          | 3374       |
| 2012 | $0.47 \pm 0.22$ | $32.48 \pm 19.05$  | $38.19 \pm 93.63$    | 68.4          | 791        |

### Negative EBITDA

| Year | $T_1$           | $T_{1/2}$          | $T_0$                 | $T_{1/2}/T_1$ | Num. Firms |
|------|-----------------|--------------------|-----------------------|---------------|------------|
| 2003 | $2.41 \pm 0.78$ | $151.23 \pm 43.99$ | $540.79 \pm 292.93$   | 62.6          | 675        |
| 2004 | $1.40 \pm 0.84$ | $127.96 \pm 78.19$ | $891.80 \pm 667.07$   | 91.2          | 647        |
| 2005 | $1.38 \pm 0.74$ | $49.91 \pm 49.16$  | $1589.95 \pm 432.50$  | 36.2          | 653        |
| 2006 | $1.52 \pm 0.48$ | $78.41 \pm 29.26$  | $818.69 \pm 249.74$   | 51.7          | 748        |
| 2007 | $1.50 \pm 0.86$ | $163.12 \pm 61.28$ | $0.01 \pm 149.71$     | 109.0         | 691        |
| 2008 | $0.25 \pm 0.37$ | $192.91 \pm 47.71$ | $347.68 \pm 301.65$   | 774.7         | 659        |
| 2009 | $3.68 \pm 2.56$ | $89.37 \pm 170.23$ | $4217.63 \pm 1477.89$ | 24.3          | 1108       |
| 2010 | $2.05 \pm 0.90$ | $189.12 \pm 45.37$ | $6.79 \pm 204.56$     | 92.4          | 1441       |
| 2011 | $4.39 \pm 1.64$ | $103.44 \pm 73.06$ | $1026.53 \pm 428.33$  | 23.6          | 1299       |
| 2012 | $0.21 \pm 0.31$ | $74.37 \pm 37.71$  | $301.65 \pm 492.52$   | 362.5         | 414        |

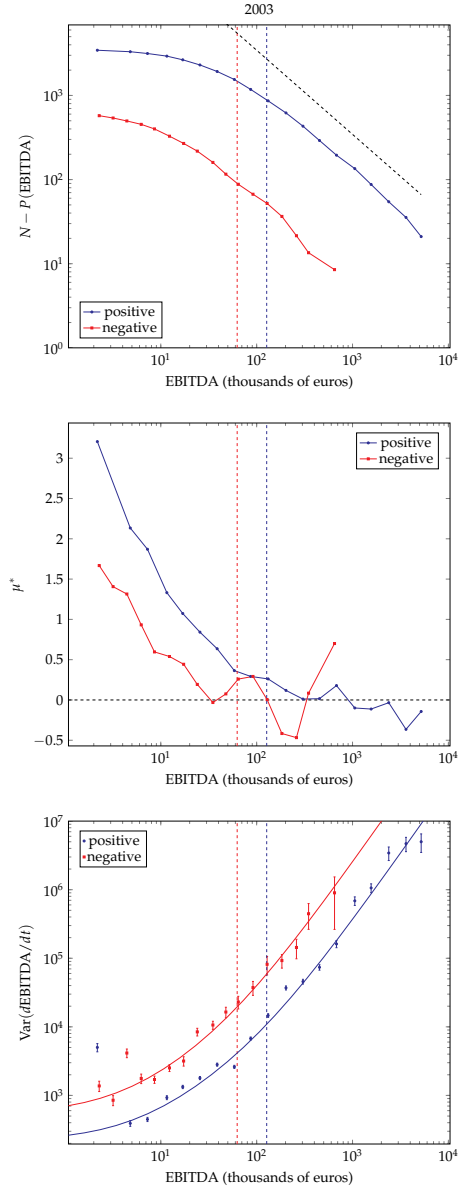

Figure 71: Cantabria

Rank plot, chemical potential and variance.

3553 Firms with positive EBITDA

$T_1 = 0.33 \pm 0.08$ ,  $T_{1/2} = 41.88 \pm 9.49$ , and  $T_0 = 216.80 \pm 121.36$

675 Firms with negative EBITDA

Negative EBITDA:

$T_1 = 2.41 \pm 0.78$ ,  $T_{1/2} = 151.23 \pm 43.99$ , and  $T_0 = 540.79 \pm 292.93$ .

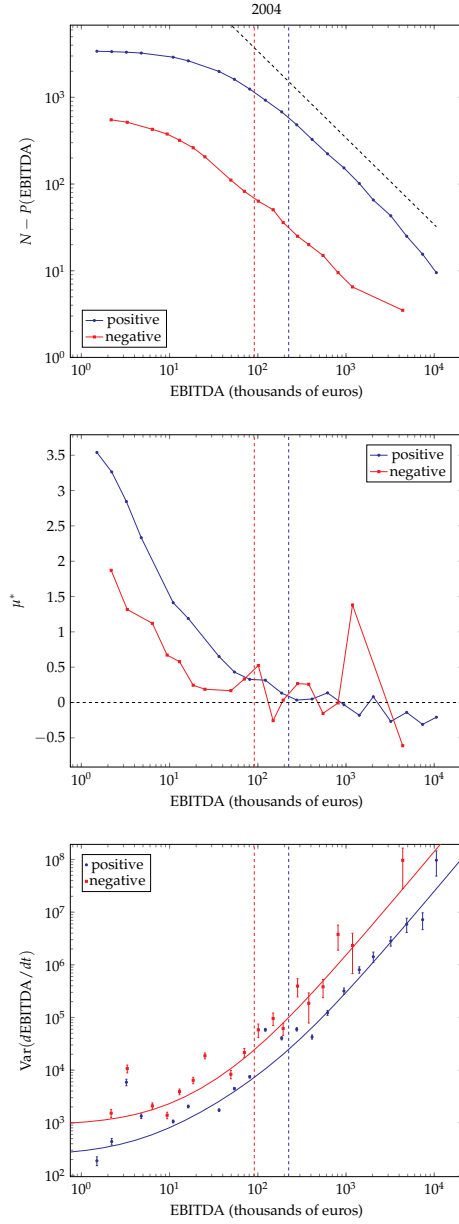

Figure 72: Cantabria

Rank plot, chemical potential and variance.

3475 Firms with positive EBITDA

$T_1 = 0.24 \pm 0.09$ ,  $T_{1/2} = 54.66 \pm 13.47$ , and  $T_0 = 236.89 \pm 172.46$

647 Firms with negative EBITDA

Negative EBITDA:

$T_1 = 1.40 \pm 0.84$ ,  $T_{1/2} = 127.96 \pm 78.19$ , and  $T_0 = 891.80 \pm 667.07$ .

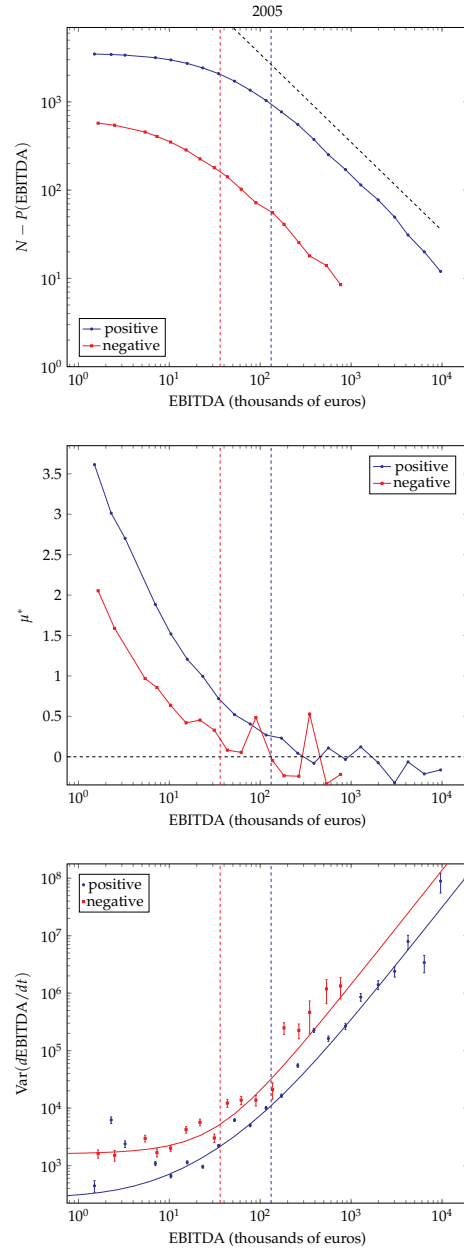

Figure 73: Cantabria

Rank plot, chemical potential and variance.

3536 Firms with positive EBITDA

$T_1 = 0.31 \pm 0.09$ ,  $T_{1/2} = 40.75 \pm 13.67$ , and  $T_0 = 268.77 \pm 240.84$

653 Firms with negative EBITDA

Negative EBITDA:

$T_1 = 1.38 \pm 0.74$ ,  $T_{1/2} = 49.91 \pm 49.16$ , and  $T_0 = 1589.95 \pm 432.50$ .

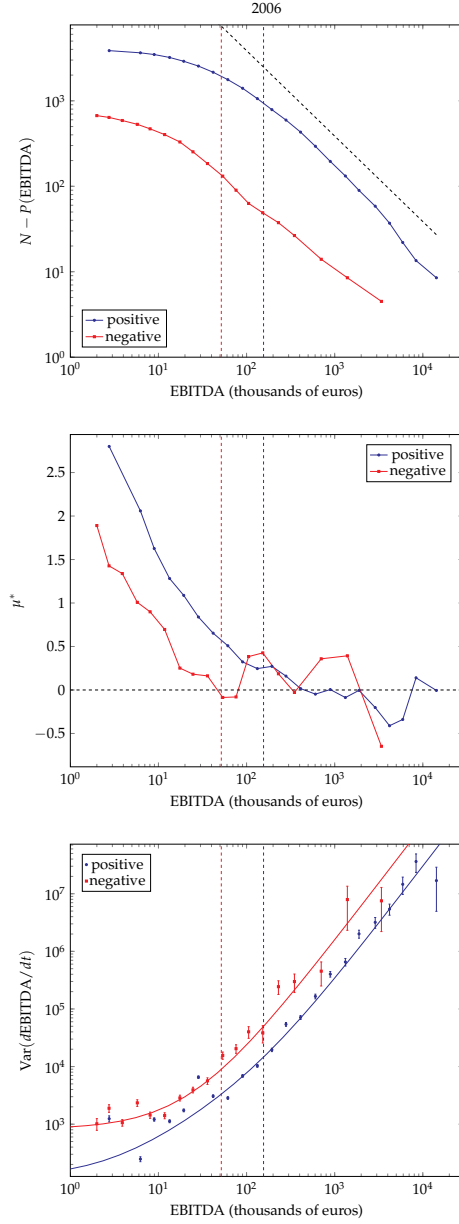

Figure 74: Cantabria

Rank plot, chemical potential and variance.

4011 Firms with positive EBITDA

$T_1 = 0.30 \pm 0.10$ ,  $T_{1/2} = 46.43 \pm 13.52$ , and  $T_0 = 120.19 \pm 165.38$

748 Firms with negative EBITDA

Negative EBITDA:

$T_1 = 1.52 \pm 0.48$ ,  $T_{1/2} = 78.41 \pm 29.26$ , and  $T_0 = 818.69 \pm 249.74$ .

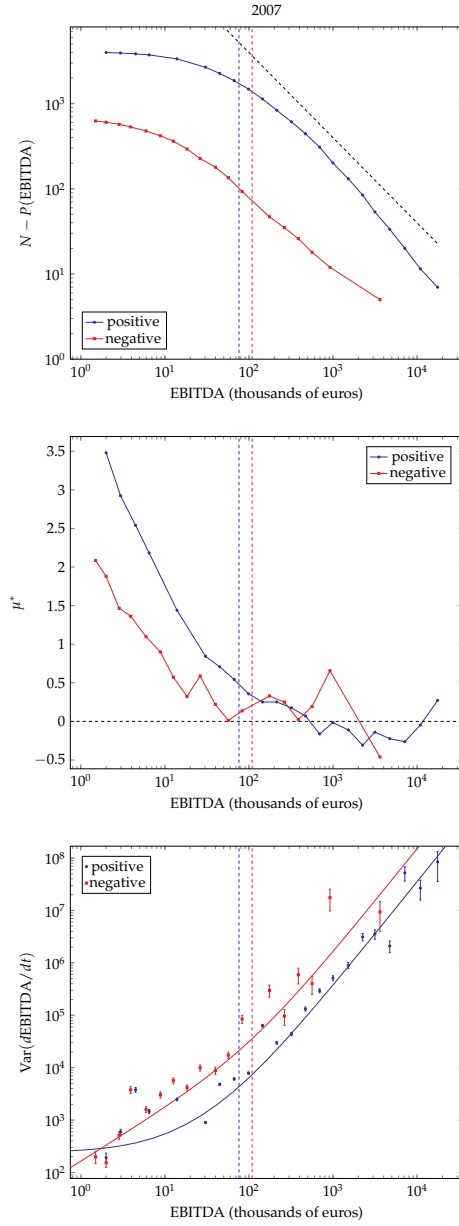

Figure 75: Cantabria

Rank plot, chemical potential and variance.

4073 Firms with positive EBITDA

 $T_1 = 0.35 \pm 0.11$ ,  $T_{1/2} = 26.80 \pm 14.29$ , and  $T_0 = 239.23 \pm 272.98$ 

691 Firms with negative EBITDA

Negative EBITDA:

 $T_1 = 1.50 \pm 0.86$ ,  $T_{1/2} = 163.12 \pm 61.28$ , and  $T_0 = 0.01 \pm 149.71$ .

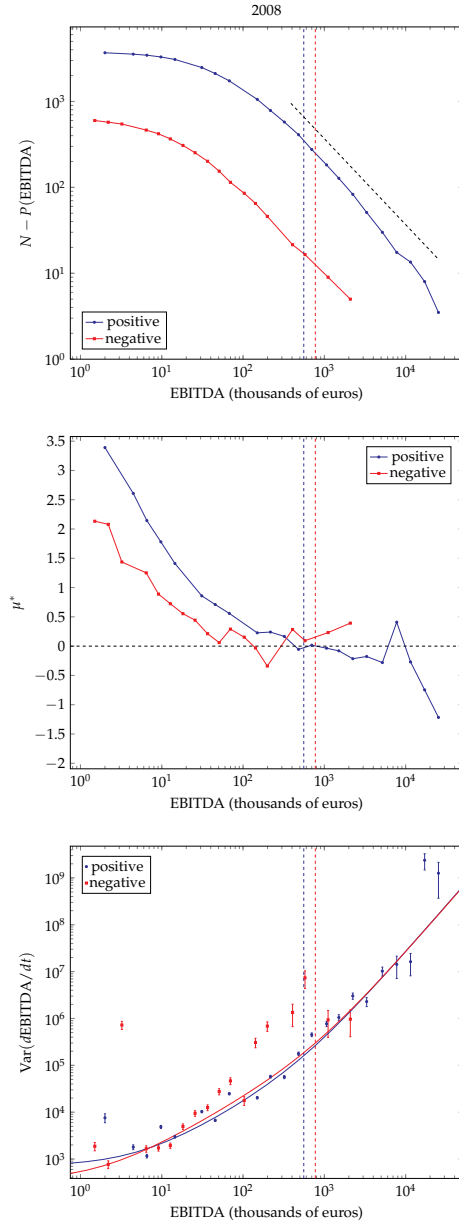

Figure 76: Cantabria

Rank plot, chemical potential and variance.

3769 Firms with positive EBITDA

$T_1 = 0.26 \pm 0.11$ ,  $T_{1/2} = 142.71 \pm 28.88$ , and  $T_0 = 708.99 \pm 426.21$

659 Firms with negative EBITDA

Negative EBITDA:

$T_1 = 0.25 \pm 0.37$ ,  $T_{1/2} = 192.91 \pm 47.71$ , and  $T_0 = 347.68 \pm 301.65$ .

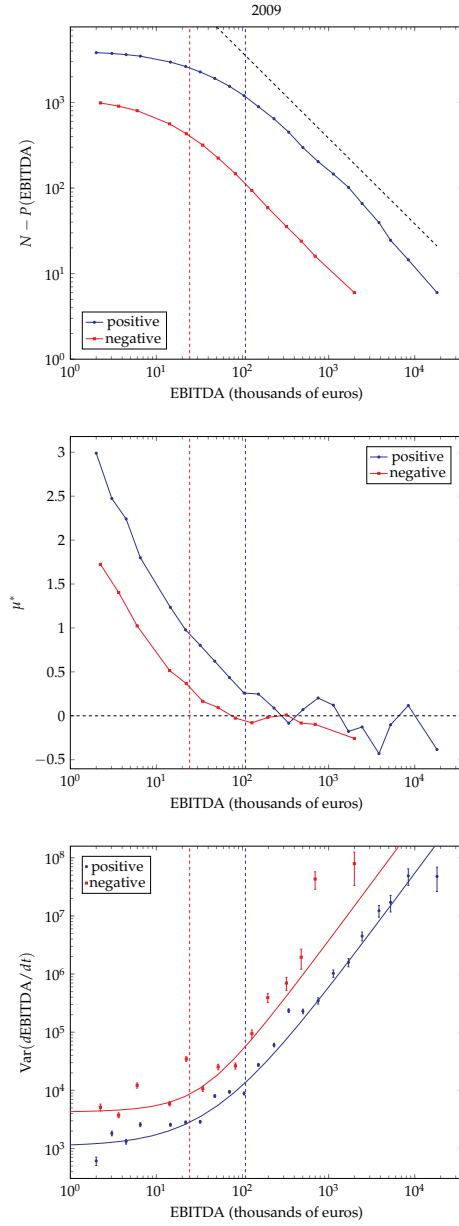

Figure 77: Cantabria

Rank plot, chemical potential and variance.

3937 Firms with positive EBITDA

$T_1 = 0.54 \pm 0.14$ ,  $T_{1/2} = 57.94 \pm 18.50$ , and  $T_0 = 1096.54 \pm 311.02$

1108 Firms with negative EBITDA

Negative EBITDA:

$T_1 = 3.68 \pm 2.56$ ,  $T_{1/2} = 89.37 \pm 170.23$ , and  $T_0 = 4217.63 \pm 1477.89$ .

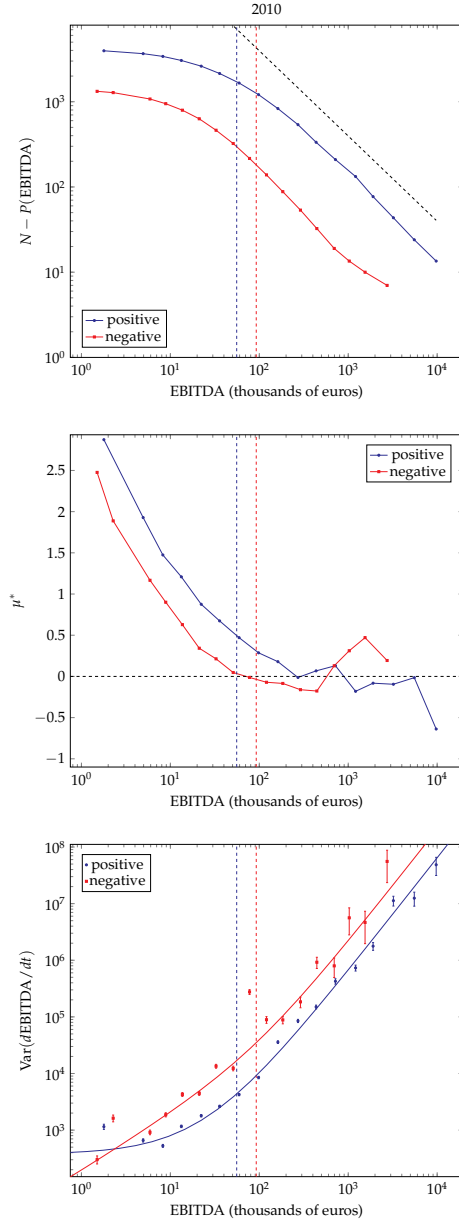

Figure 78: Cantabria

Rank plot, chemical potential and variance.

4106 Firms with positive EBITDA

$T_1 = 0.64 \pm 0.11$ ,  $T_{1/2} = 35.76 \pm 11.89$ , and  $T_0 = 376.68 \pm 138.91$

1441 Firms with negative EBITDA

Negative EBITDA:

$T_1 = 2.05 \pm 0.90$ ,  $T_{1/2} = 189.12 \pm 45.37$ , and  $T_0 = 6.79 \pm 204.56$ .

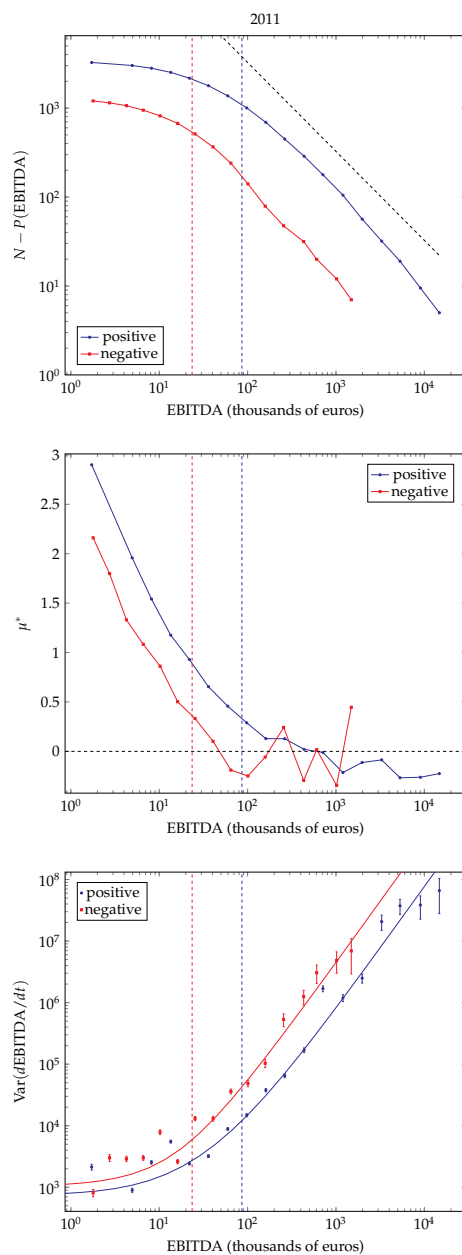

Figure 79: Cantabria

Rank plot, chemical potential and variance.

3374 Firms with positive EBITDA

$T_1 = 0.76 \pm 0.20$ ,  $T_{1/2} = 65.57 \pm 21.61$ , and  $T_0 = 738.68 \pm 277.06$

1299 Firms with negative EBITDA

Negative EBITDA:

$T_1 = 4.39 \pm 1.64$ ,  $T_{1/2} = 103.44 \pm 73.06$ , and  $T_0 = 1026.53 \pm 428.33$ .

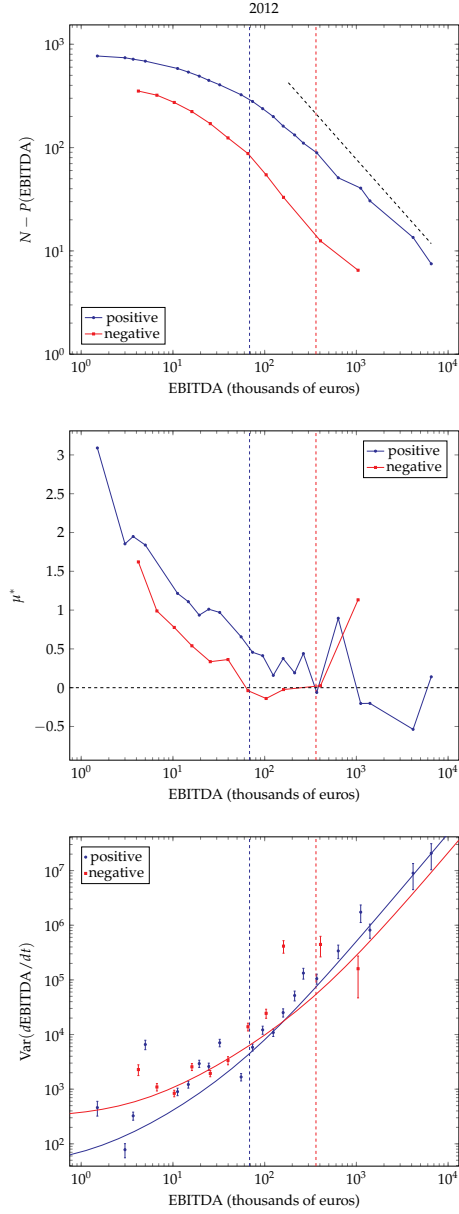

Figure 80: Cantabria

Rank plot, chemical potential and variance.

791 Firms with positive EBITDA

$T_1 = 0.47 \pm 0.22$ ,  $T_{1/2} = 32.48 \pm 19.05$ , and  $T_0 = 38.19 \pm 93.63$

414 Firms with negative EBITDA

Negative EBITDA:

$T_1 = 0.21 \pm 0.31$ ,  $T_{1/2} = 74.37 \pm 37.71$ , and  $T_0 = 301.65 \pm 492.52$ .

# Castile and Leon

## Tables of Temperatures

### Positive EBITDA

| Year | $T_1$           | $T_{1/2}$          | $T_0$               | $T_{1/2}/T_1$ | Num. Firms |
|------|-----------------|--------------------|---------------------|---------------|------------|
| 2003 | $0.41 \pm 0.07$ | $22.43 \pm 6.79$   | $338.56 \pm 85.10$  | 55.3          | 20859      |
| 2004 | $0.44 \pm 0.05$ | $23.50 \pm 4.84$   | $241.06 \pm 52.41$  | 53.5          | 21830      |
| 2005 | $0.44 \pm 0.06$ | $26.88 \pm 4.93$   | $219.83 \pm 43.97$  | 61.7          | 22848      |
| 2006 | $0.48 \pm 0.06$ | $21.55 \pm 5.42$   | $305.68 \pm 58.93$  | 45.3          | 23941      |
| 2007 | $0.61 \pm 0.10$ | $30.55 \pm 8.81$   | $273.84 \pm 94.43$  | 50.0          | 23346      |
| 2008 | $0.57 \pm 0.12$ | $54.60 \pm 15.18$  | $476.56 \pm 167.03$ | 95.4          | 21761      |
| 2009 | $0.84 \pm 0.15$ | $65.78 \pm 13.09$  | $363.25 \pm 133.60$ | 78.2          | 23026      |
| 2010 | $0.32 \pm 0.14$ | $79.42 \pm 18.88$  | $297.07 \pm 177.15$ | 250.4         | 24145      |
| 2011 | $0.63 \pm 0.18$ | $102.82 \pm 21.19$ | $324.56 \pm 162.43$ | 162.5         | 21393      |
| 2012 | $0.22 \pm 0.08$ | $61.29 \pm 9.93$   | $197.76 \pm 104.70$ | 281.8         | 9818       |

### Negative EBITDA

| Year | $T_1$           | $T_{1/2}$          | $T_0$                | $T_{1/2}/T_1$ | Num. Firms |
|------|-----------------|--------------------|----------------------|---------------|------------|
| 2003 | $1.15 \pm 0.55$ | $86.86 \pm 34.24$  | $1035.62 \pm 311.85$ | 75.3          | 4216       |
| 2004 | $1.44 \pm 0.38$ | $131.19 \pm 17.33$ | $165.40 \pm 70.79$   | 91.1          | 4329       |
| 2005 | $2.36 \pm 0.59$ | $63.93 \pm 28.75$  | $1030.09 \pm 209.03$ | 27.1          | 4534       |
| 2006 | $0.90 \pm 0.40$ | $128.81 \pm 24.92$ | $239.89 \pm 159.67$  | 143.9         | 4886       |
| 2007 | $2.03 \pm 0.69$ | $237.77 \pm 53.27$ | $595.33 \pm 351.77$  | 117.2         | 4256       |
| 2008 | $2.85 \pm 0.80$ | $265.33 \pm 41.63$ | $339.74 \pm 225.95$  | 93.2          | 4071       |
| 2009 | $4.39 \pm 0.99$ | $270.28 \pm 47.84$ | $233.28 \pm 187.86$  | 61.6          | 6309       |
| 2010 | $2.17 \pm 0.67$ | $152.61 \pm 32.36$ | $220.84 \pm 161.83$  | 70.4          | 8019       |
| 2011 | $2.06 \pm 1.23$ | $278.36 \pm 74.07$ | $341.26 \pm 370.82$  | 135.1         | 7519       |
| 2012 | $2.34 \pm 0.61$ | $57.58 \pm 27.73$  | $659.00 \pm 178.12$  | 24.6          | 4499       |

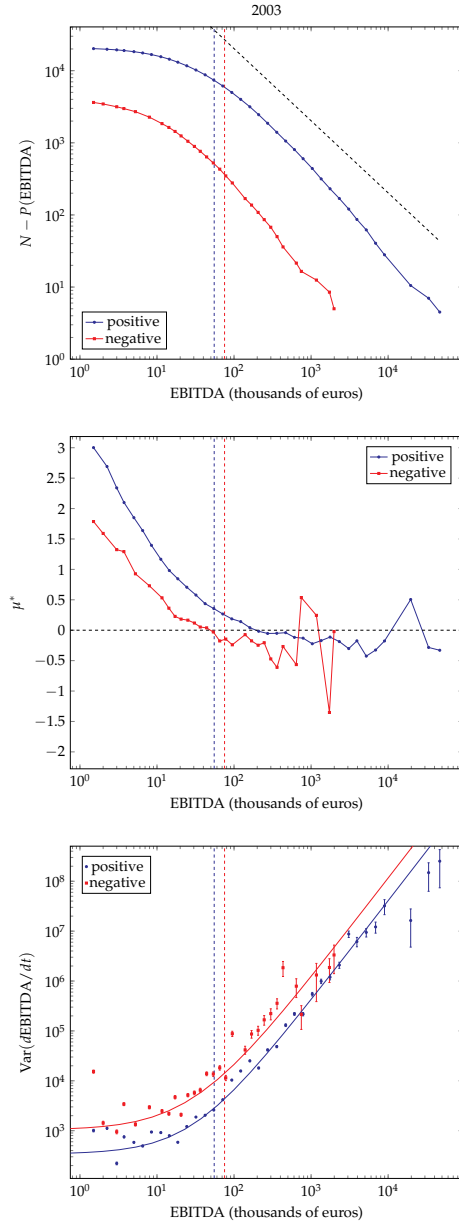

Figure 81: Castile and Leon

Rank plot, chemical potential and variance.

20859 Firms with positive EBITDA

$T_1 = 0.41 \pm 0.07$ ,  $T_{1/2} = 22.43 \pm 6.79$ , and  $T_0 = 338.56 \pm 85.10$

4216 Firms with negative EBITDA

Negative EBITDA:

$T_1 = 1.15 \pm 0.55$ ,  $T_{1/2} = 86.86 \pm 34.24$ , and  $T_0 = 1035.62 \pm 311.85$ .

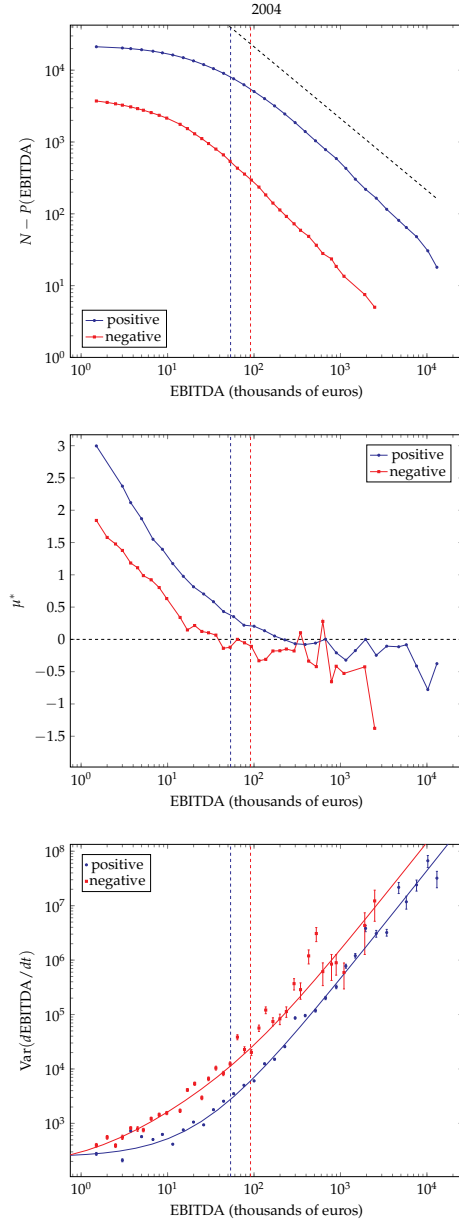

Figure 82: Castile and Leon

Rank plot, chemical potential and variance.

21830 Firms with positive EBITDA

$T_1 = 0.44 \pm 0.05$ ,  $T_{1/2} = 23.50 \pm 4.84$ , and  $T_0 = 241.06 \pm 52.41$

4329 Firms with negative EBITDA

Negative EBITDA:

$T_1 = 1.44 \pm 0.38$ ,  $T_{1/2} = 131.19 \pm 17.33$ , and  $T_0 = 165.40 \pm 70.79$ .

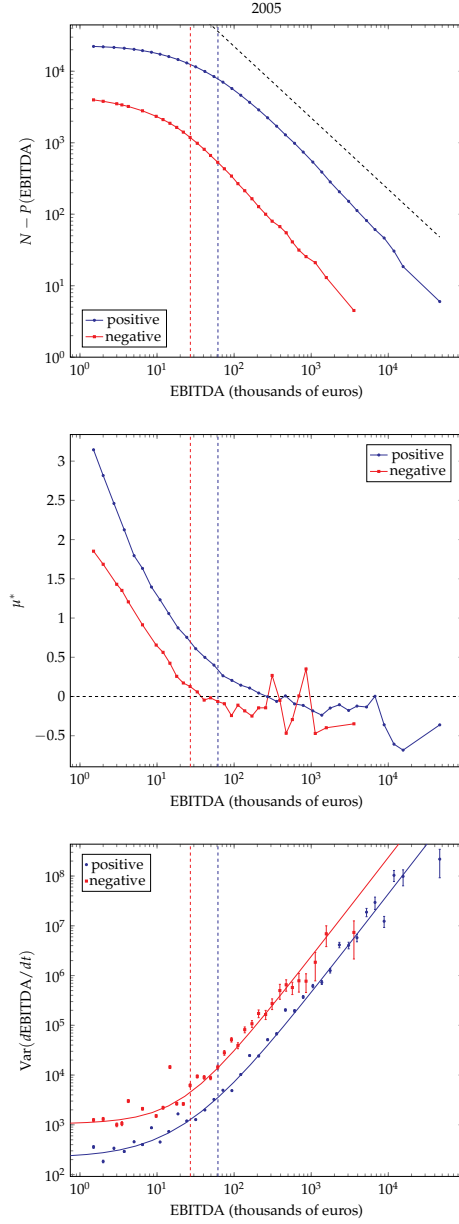

Figure 83: Castile and Leon

Rank plot, chemical potential and variance.

22848 Firms with positive EBITDA

 $T_1 = 0.44 \pm 0.06$ ,  $T_{1/2} = 26.88 \pm 4.93$ , and  $T_0 = 219.83 \pm 43.97$ 

4534 Firms with negative EBITDA

Negative EBITDA:

 $T_1 = 2.36 \pm 0.59$ ,  $T_{1/2} = 63.93 \pm 28.75$ , and  $T_0 = 1030.09 \pm 209.03$ .

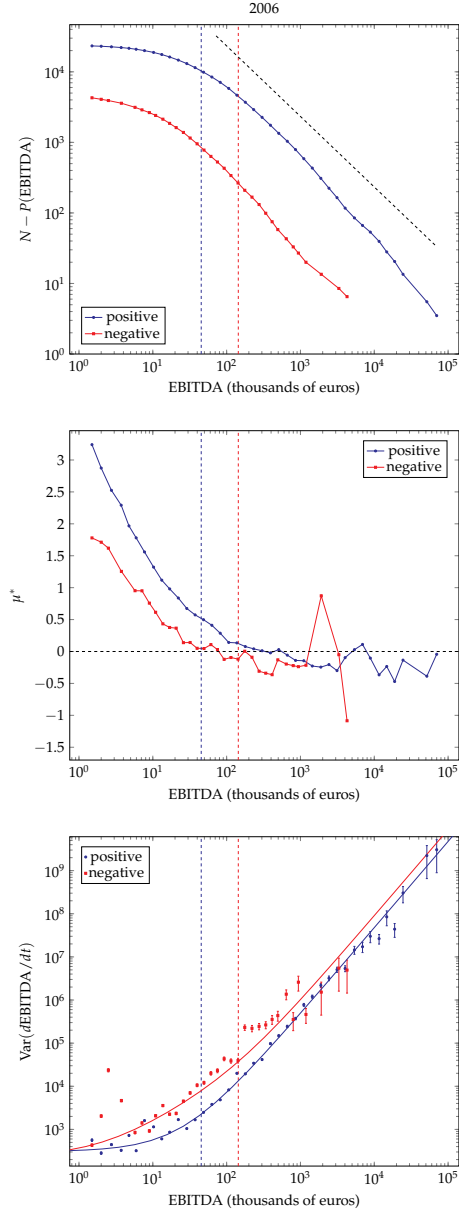

Figure 84: Castile and Leon

Rank plot, chemical potential and variance.

23941 Firms with positive EBITDA

$T_1 = 0.48 \pm 0.06$ ,  $T_{1/2} = 21.55 \pm 5.42$ , and  $T_0 = 305.68 \pm 58.93$

4886 Firms with negative EBITDA

Negative EBITDA:

$T_1 = 0.90 \pm 0.40$ ,  $T_{1/2} = 128.81 \pm 24.92$ , and  $T_0 = 239.89 \pm 159.67$ .

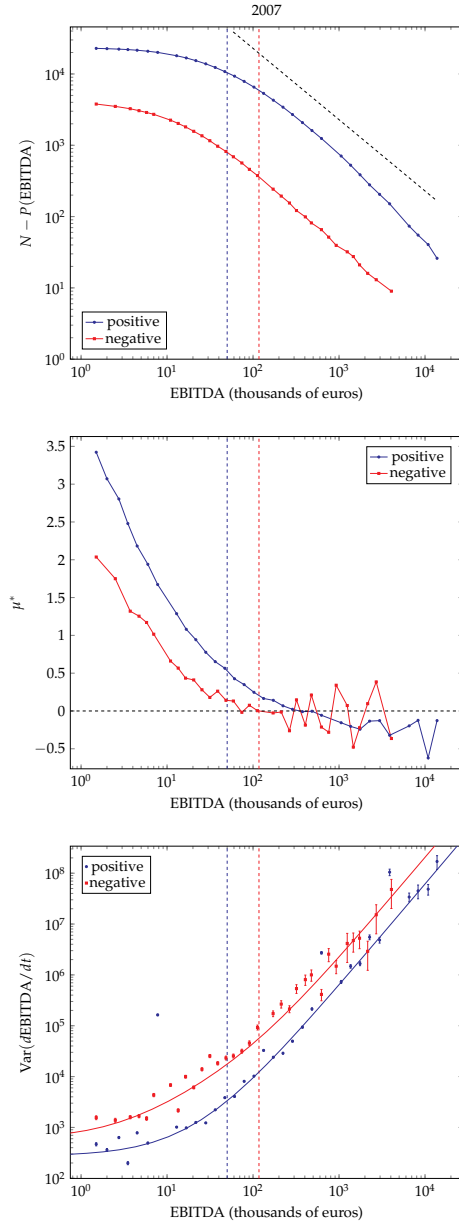

Figure 85: Castile and Leon

Rank plot, chemical potential and variance.

23346 Firms with positive EBITDA

$T_1 = 0.61 \pm 0.10$ ,  $T_{1/2} = 30.55 \pm 8.81$ , and  $T_0 = 273.84 \pm 94.43$

4256 Firms with negative EBITDA

Negative EBITDA:

$T_1 = 2.03 \pm 0.69$ ,  $T_{1/2} = 237.77 \pm 53.27$ , and  $T_0 = 595.33 \pm 351.77$ .

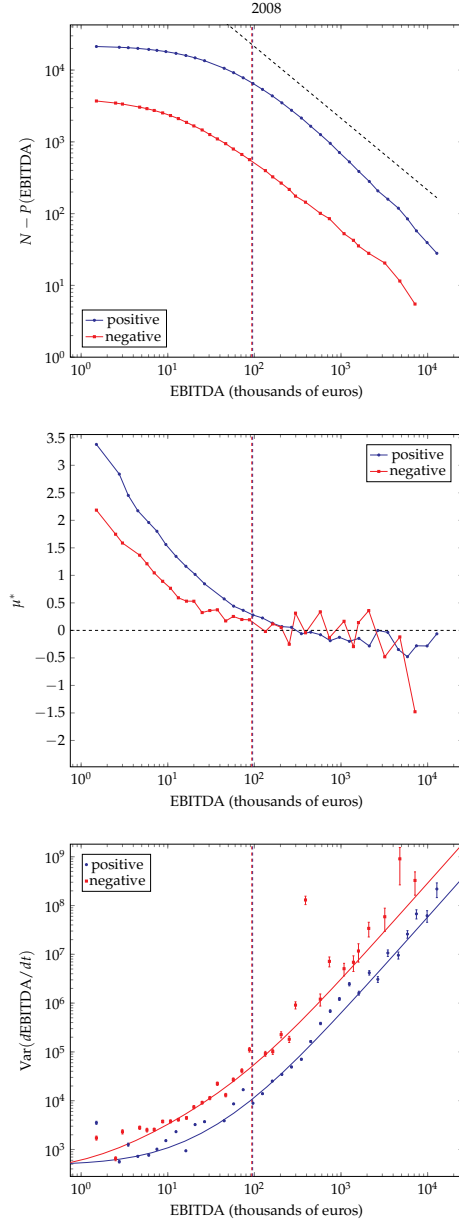

Figure 86: Castile and Leon

Rank plot, chemical potential and variance.

21761 Firms with positive EBITDA

$T_1 = 0.57 \pm 0.12$ ,  $T_{1/2} = 54.60 \pm 15.18$ , and  $T_0 = 476.56 \pm 167.03$

4071 Firms with negative EBITDA

Negative EBITDA:

$T_1 = 2.85 \pm 0.80$ ,  $T_{1/2} = 265.33 \pm 41.63$ , and  $T_0 = 339.74 \pm 225.95$ .

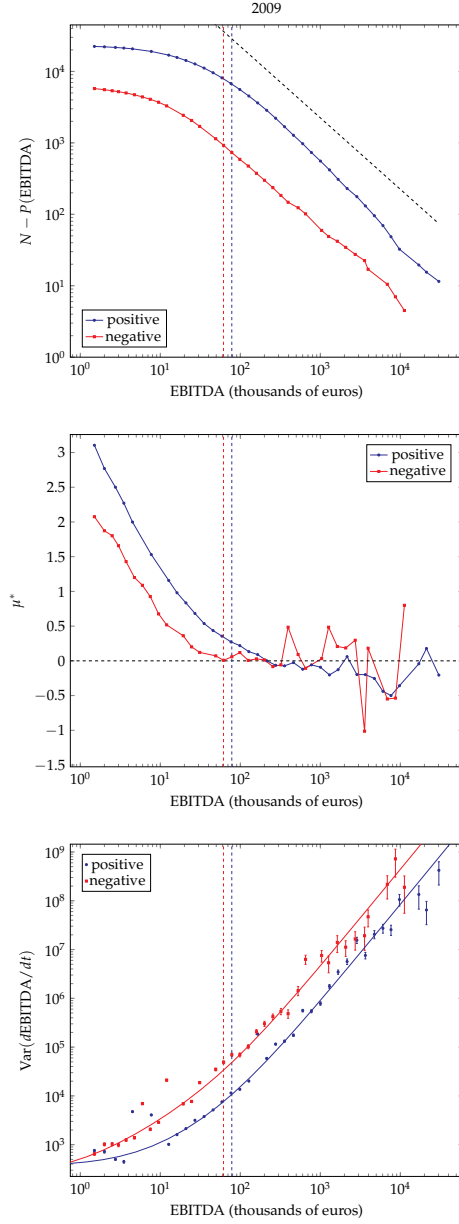

Figure 87: Castile and Leon

Rank plot, chemical potential and variance.

23026 Firms with positive EBITDA

$T_1 = 0.84 \pm 0.15$ ,  $T_{1/2} = 65.78 \pm 13.09$ , and  $T_0 = 363.25 \pm 133.60$

6309 Firms with negative EBITDA

Negative EBITDA:

$T_1 = 4.39 \pm 0.99$ ,  $T_{1/2} = 270.28 \pm 47.84$ , and  $T_0 = 233.28 \pm 187.86$ .

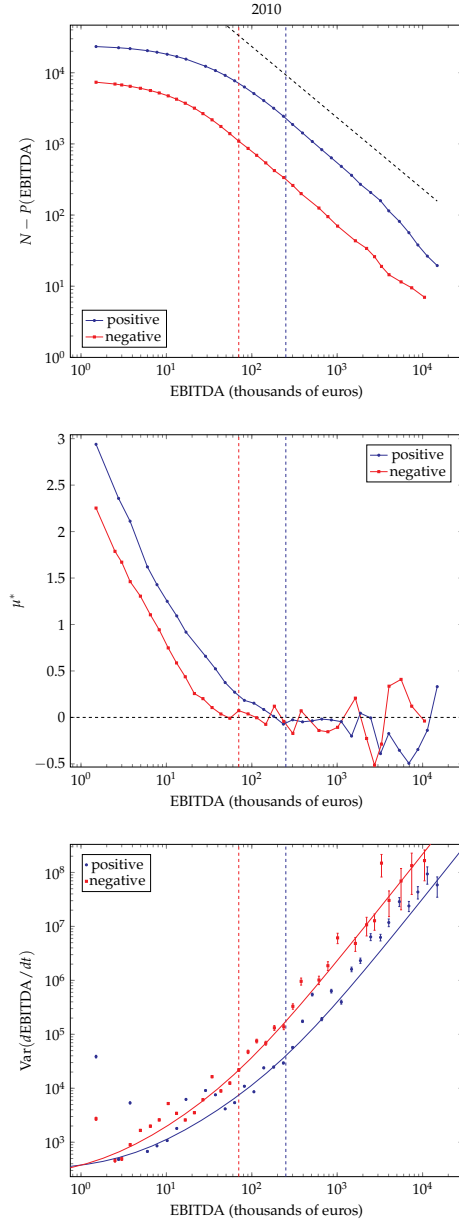

Figure 88: Castile and Leon

Rank plot, chemical potential and variance.

24145 Firms with positive EBITDA

$T_1 = 0.32 \pm 0.14$ ,  $T_{1/2} = 79.42 \pm 18.88$ , and  $T_0 = 297.07 \pm 177.15$

8019 Firms with negative EBITDA

Negative EBITDA:

$T_1 = 2.17 \pm 0.67$ ,  $T_{1/2} = 152.61 \pm 32.36$ , and  $T_0 = 220.84 \pm 161.83$ .

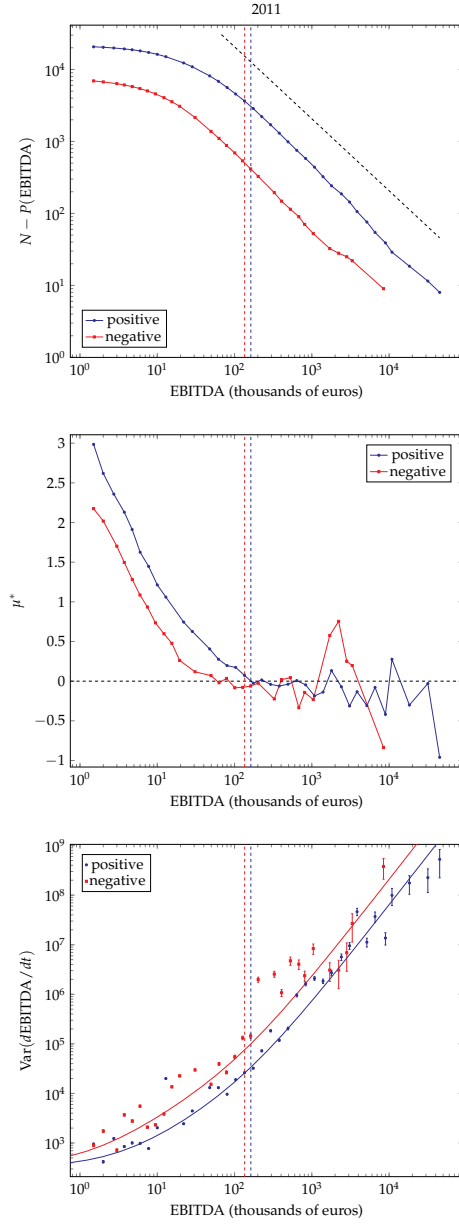

Figure 89: Castile and Leon

Rank plot, chemical potential and variance.

21393 Firms with positive EBITDA

$T_1 = 0.63 \pm 0.18$ ,  $T_{1/2} = 102.82 \pm 21.19$ , and  $T_0 = 324.56 \pm 162.43$

7519 Firms with negative EBITDA

Negative EBITDA:

$T_1 = 2.06 \pm 1.23$ ,  $T_{1/2} = 278.36 \pm 74.07$ , and  $T_0 = 341.26 \pm 370.82$ .

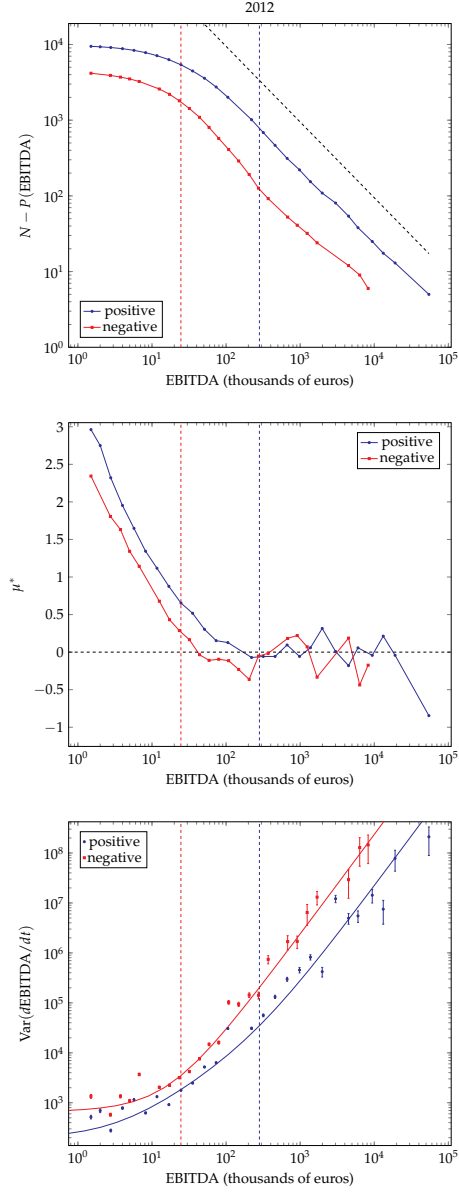

Figure 90: Castile and Leon

Rank plot, chemical potential and variance.

9818 Firms with positive EBITDA

$T_1 = 0.22 \pm 0.08$ ,  $T_{1/2} = 61.29 \pm 9.93$ , and  $T_0 = 197.76 \pm 104.70$

4499 Firms with negative EBITDA

Negative EBITDA:

$T_1 = 2.34 \pm 0.61$ ,  $T_{1/2} = 57.58 \pm 27.73$ , and  $T_0 = 659.00 \pm 178.12$ .

# Castile-La Mancha

## Tables of Temperatures

### Positive EBITDA

| Year | $T_1$           | $T_{1/2}$         | $T_0$               | $T_{1/2}/T_1$ | Num. Firms |
|------|-----------------|-------------------|---------------------|---------------|------------|
| 2003 | $0.33 \pm 0.12$ | $31.78 \pm 11.75$ | $236.95 \pm 103.45$ | 97.4          | 17315      |
| 2004 | $0.49 \pm 0.07$ | $19.84 \pm 4.94$  | $102.91 \pm 40.94$  | 40.3          | 17471      |
| 2005 | $0.48 \pm 0.08$ | $24.23 \pm 6.95$  | $201.33 \pm 72.71$  | 50.5          | 18584      |
| 2006 | $0.56 \pm 0.09$ | $19.15 \pm 8.01$  | $388.38 \pm 93.33$  | 33.9          | 20087      |
| 2007 | $0.61 \pm 0.12$ | $44.69 \pm 11.20$ | $223.59 \pm 101.33$ | 73.8          | 21278      |
| 2008 | $0.79 \pm 0.11$ | $33.63 \pm 9.15$  | $403.02 \pm 101.61$ | 42.6          | 19014      |
| 2009 | $0.98 \pm 0.16$ | $40.15 \pm 12.86$ | $580.38 \pm 134.05$ | 40.8          | 18793      |
| 2010 | $0.48 \pm 0.10$ | $48.10 \pm 9.57$  | $400.11 \pm 90.59$  | 100.1         | 19699      |
| 2011 | $0.65 \pm 0.12$ | $66.81 \pm 11.43$ | $346.91 \pm 117.65$ | 102.5         | 16739      |
| 2012 | $0.25 \pm 0.08$ | $39.78 \pm 8.05$  | $265.76 \pm 74.91$  | 160.6         | 7095       |

### Negative EBITDA

| Year | $T_1$           | $T_{1/2}$          | $T_0$                | $T_{1/2}/T_1$ | Num. Firms |
|------|-----------------|--------------------|----------------------|---------------|------------|
| 2003 | $1.41 \pm 0.80$ | $129.37 \pm 32.79$ | $65.43 \pm 112.82$   | 92.0          | 3183       |
| 2004 | $1.42 \pm 0.80$ | $151.59 \pm 42.10$ | $136.64 \pm 169.72$  | 107.0         | 3046       |
| 2005 | $0.58 \pm 0.56$ | $233.58 \pm 36.80$ | $101.29 \pm 106.82$  | 401.6         | 3389       |
| 2006 | $1.57 \pm 0.53$ | $141.86 \pm 30.41$ | $552.91 \pm 196.26$  | 90.3          | 3640       |
| 2007 | $2.74 \pm 0.99$ | $133.41 \pm 63.22$ | $1226.81 \pm 478.26$ | 48.7          | 3486       |
| 2008 | $4.40 \pm 1.21$ | $107.11 \pm 65.97$ | $1762.51 \pm 523.00$ | 24.4          | 3462       |
| 2009 | $3.09 \pm 0.63$ | $229.96 \pm 35.77$ | $824.55 \pm 231.80$  | 74.5          | 5344       |
| 2010 | $3.34 \pm 0.64$ | $90.26 \pm 26.99$  | $725.89 \pm 159.17$  | 27.0          | 7084       |
| 2011 | $4.44 \pm 0.84$ | $69.47 \pm 37.24$  | $1131.32 \pm 268.59$ | 15.7          | 6474       |
| 2012 | $2.93 \pm 1.35$ | $111.09 \pm 51.36$ | $90.62 \pm 156.06$   | 37.9          | 3443       |

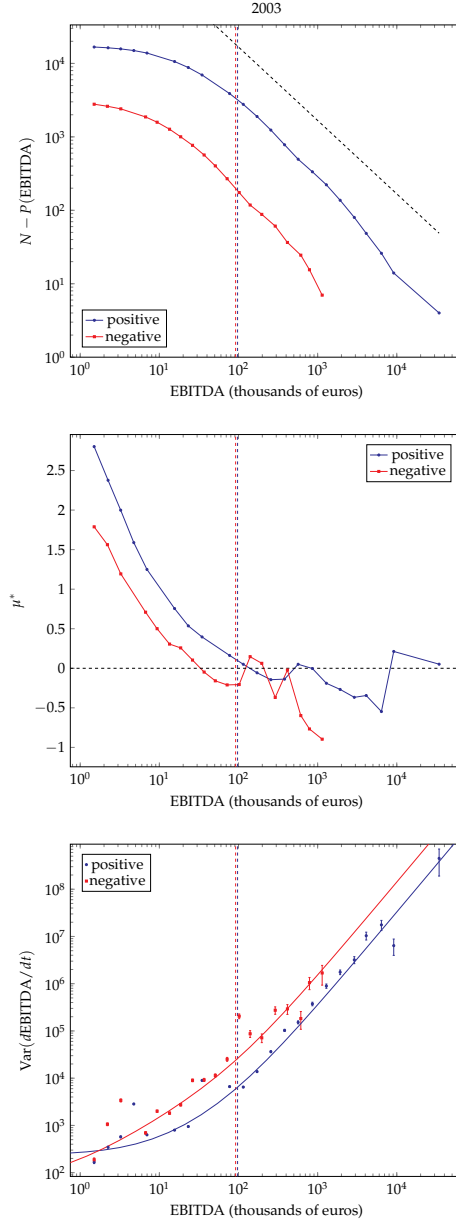

Figure 91: Castile-La Mancha

Rank plot, chemical potential and variance.

17315 Firms with positive EBITDA

$T_1 = 0.33 \pm 0.12$ ,  $T_{1/2} = 31.78 \pm 11.75$ , and  $T_0 = 236.95 \pm 103.45$

3183 Firms with negative EBITDA

Negative EBITDA:

$T_1 = 1.41 \pm 0.80$ ,  $T_{1/2} = 129.37 \pm 32.79$ , and  $T_0 = 65.43 \pm 112.82$ .

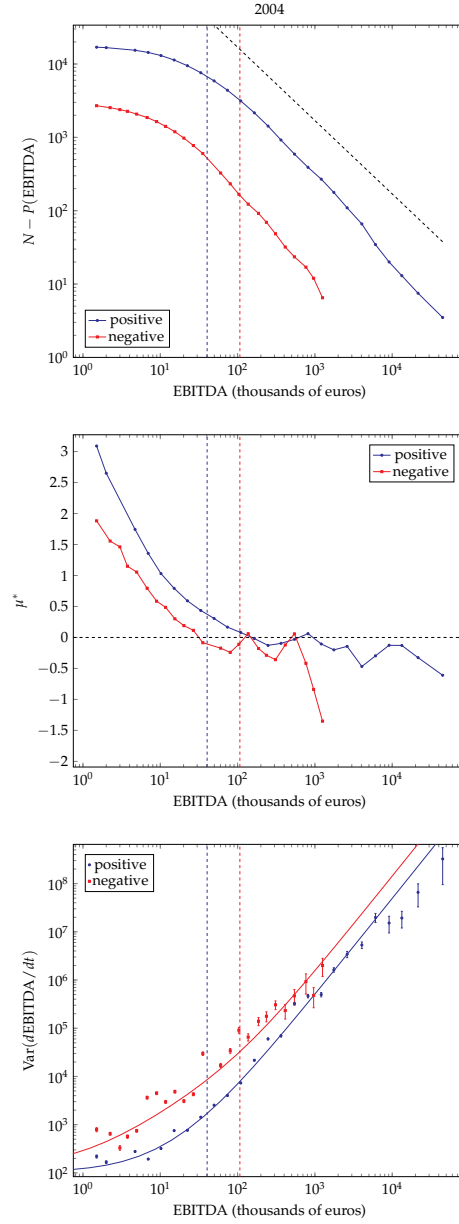

Figure 92: Castile-La Mancha

Rank plot, chemical potential and variance.

17471 Firms with positive EBITDA

$T_1 = 0.49 \pm 0.07$ ,  $T_{1/2} = 19.84 \pm 4.94$ , and  $T_0 = 102.91 \pm 40.94$

3046 Firms with negative EBITDA

Negative EBITDA:

$T_1 = 1.42 \pm 0.80$ ,  $T_{1/2} = 151.59 \pm 42.10$ , and  $T_0 = 136.64 \pm 169.72$ .

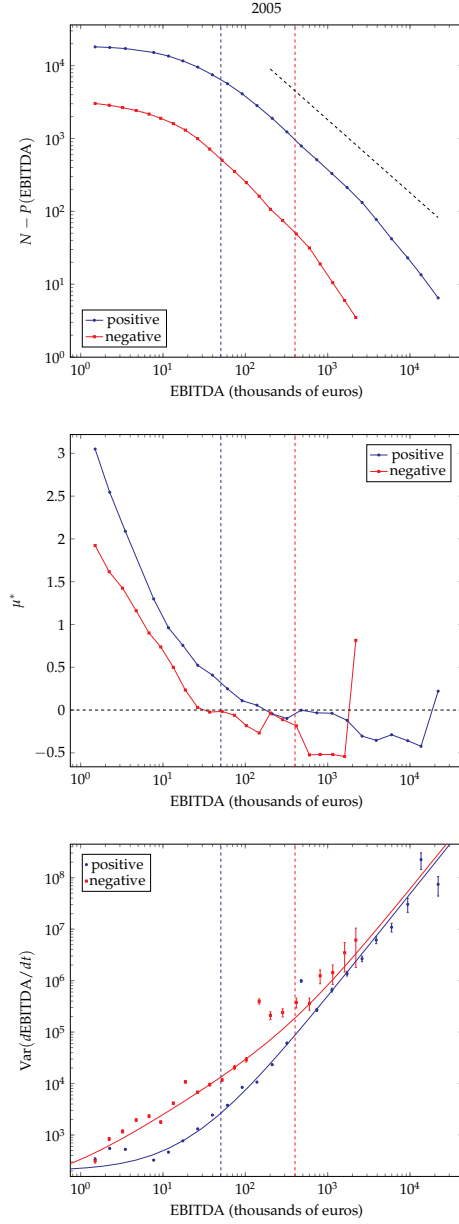

Figure 93: Castile-La Mancha

Rank plot, chemical potential and variance.

18584 Firms with positive EBITDA

$T_1 = 0.48 \pm 0.08$ ,  $T_{1/2} = 24.23 \pm 6.95$ , and  $T_0 = 201.33 \pm 72.71$

3389 Firms with negative EBITDA

Negative EBITDA:

$T_1 = 0.58 \pm 0.56$ ,  $T_{1/2} = 233.58 \pm 36.80$ , and  $T_0 = 101.29 \pm 106.82$ .

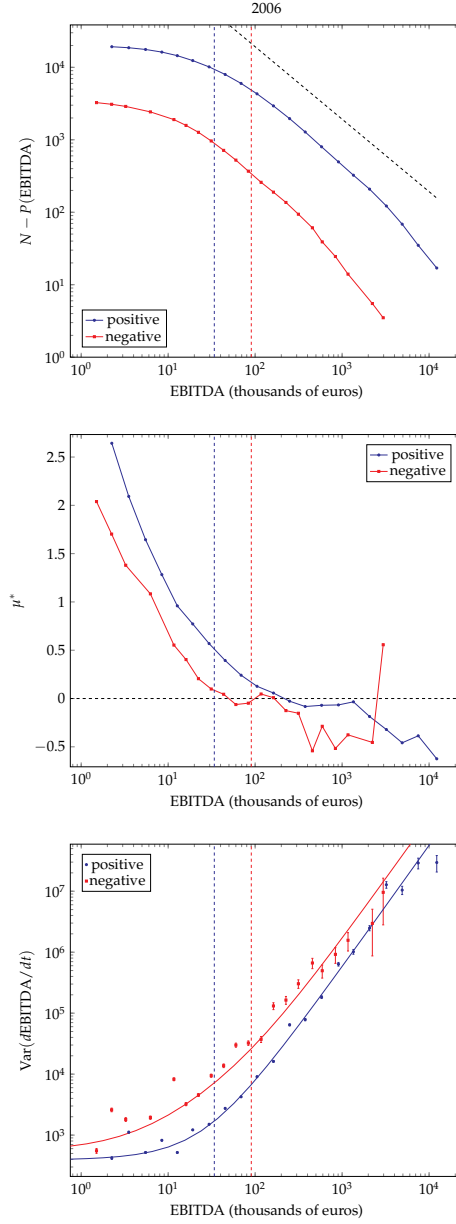

Figure 94: Castile-La Mancha

Rank plot, chemical potential and variance.

20087 Firms with positive EBITDA

$T_1 = 0.56 \pm 0.09$ ,  $T_{1/2} = 19.15 \pm 8.01$ , and  $T_0 = 388.38 \pm 93.33$

3640 Firms with negative EBITDA

Negative EBITDA:

$T_1 = 1.57 \pm 0.53$ ,  $T_{1/2} = 141.86 \pm 30.41$ , and  $T_0 = 552.91 \pm 196.26$ .

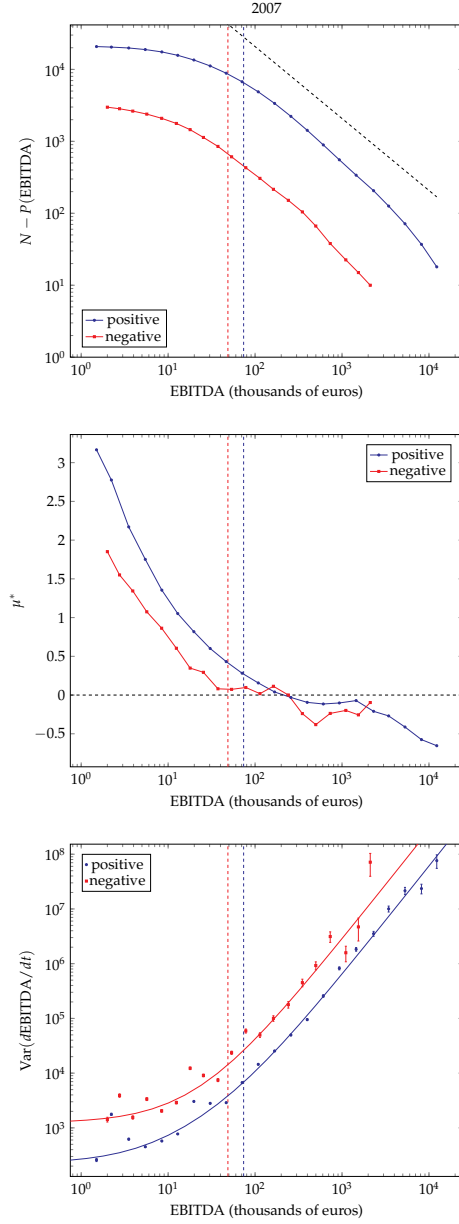

Figure 95: Castile-La Mancha

Rank plot, chemical potential and variance.

21278 Firms with positive EBITDA

$T_1 = 0.61 \pm 0.12$ ,  $T_{1/2} = 44.69 \pm 11.20$ , and  $T_0 = 223.59 \pm 101.33$

3486 Firms with negative EBITDA

Negative EBITDA:

$T_1 = 2.74 \pm 0.99$ ,  $T_{1/2} = 133.41 \pm 63.22$ , and  $T_0 = 1226.81 \pm 478.26$ .

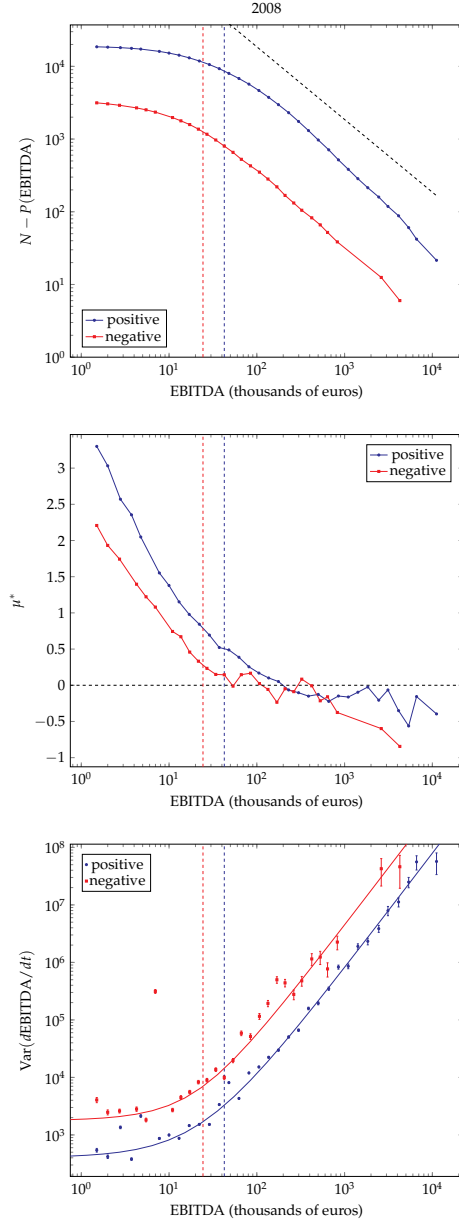

Figure 96: Castile-La Mancha

Rank plot, chemical potential and variance.

19014 Firms with positive EBITDA

$T_1 = 0.79 \pm 0.11$ ,  $T_{1/2} = 33.63 \pm 9.15$ , and  $T_0 = 403.02 \pm 101.61$

3462 Firms with negative EBITDA

Negative EBITDA:

$T_1 = 4.40 \pm 1.21$ ,  $T_{1/2} = 107.11 \pm 65.97$ , and  $T_0 = 1762.51 \pm 523.00$ .

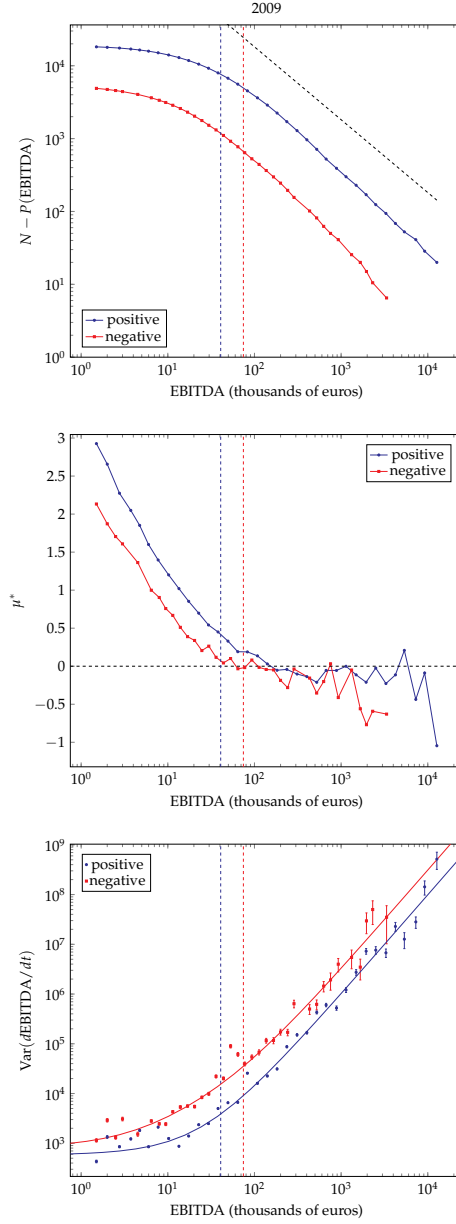

Figure 97: Castile-La Mancha

Rank plot, chemical potential and variance.

18793 Firms with positive EBITDA

$T_1 = 0.98 \pm 0.16$ ,  $T_{1/2} = 40.15 \pm 12.86$ , and  $T_0 = 580.38 \pm 134.05$

5344 Firms with negative EBITDA

Negative EBITDA:

$T_1 = 3.09 \pm 0.63$ ,  $T_{1/2} = 229.96 \pm 35.77$ , and  $T_0 = 824.55 \pm 231.80$ .

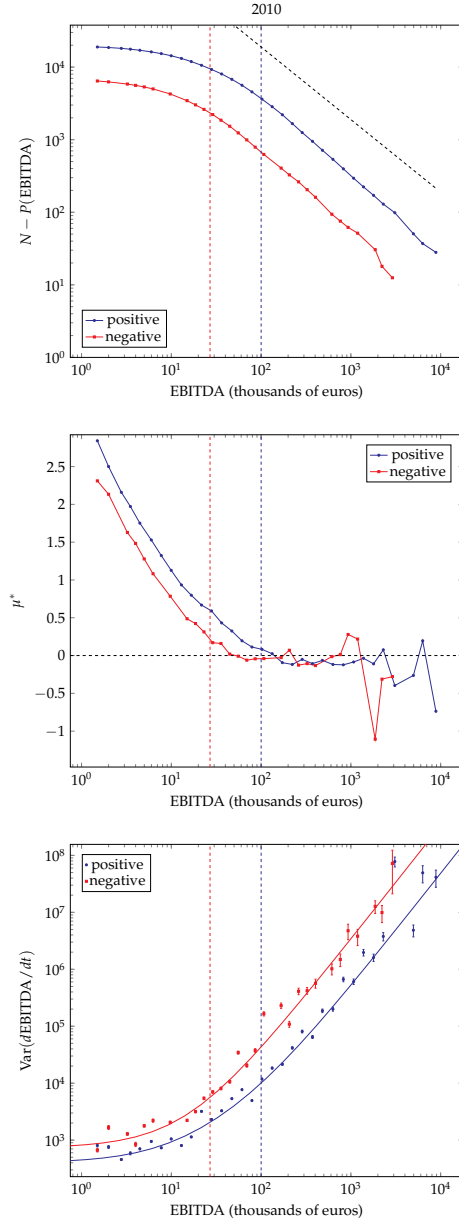

Figure 98: Castile-La Mancha

Rank plot, chemical potential and variance.

19699 Firms with positive EBITDA

$T_1 = 0.48 \pm 0.10$ ,  $T_{1/2} = 48.10 \pm 9.57$ , and  $T_0 = 400.11 \pm 90.59$

7084 Firms with negative EBITDA

Negative EBITDA:

$T_1 = 3.34 \pm 0.64$ ,  $T_{1/2} = 90.26 \pm 26.99$ , and  $T_0 = 725.89 \pm 159.17$ .

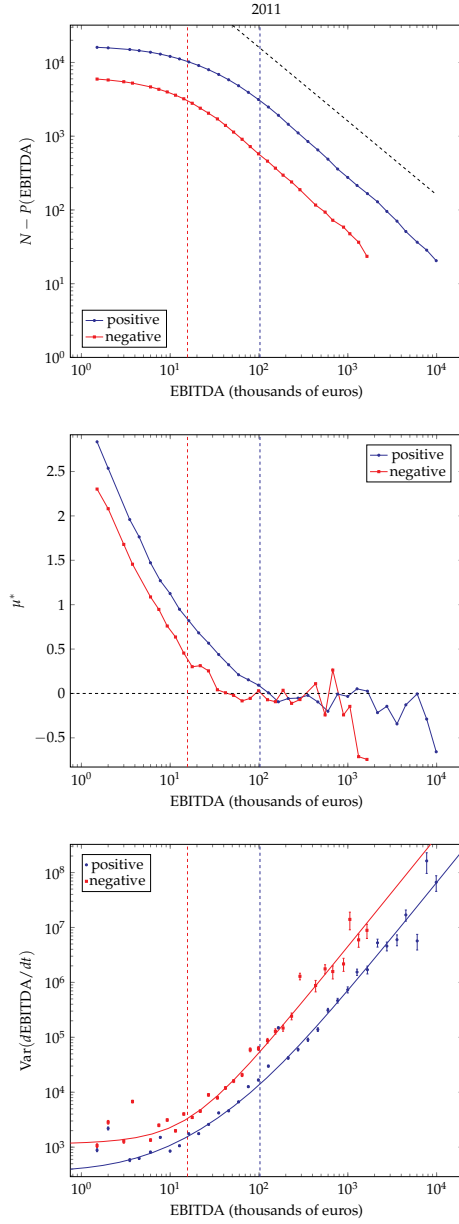

Figure 99: Castile-La Mancha

Rank plot, chemical potential and variance.

16739 Firms with positive EBITDA

$T_1 = 0.65 \pm 0.12$ ,  $T_{1/2} = 66.81 \pm 11.43$ , and  $T_0 = 346.91 \pm 117.65$

6474 Firms with negative EBITDA

Negative EBITDA:

$T_1 = 4.44 \pm 0.84$ ,  $T_{1/2} = 69.47 \pm 37.24$ , and  $T_0 = 1131.32 \pm 268.59$ .

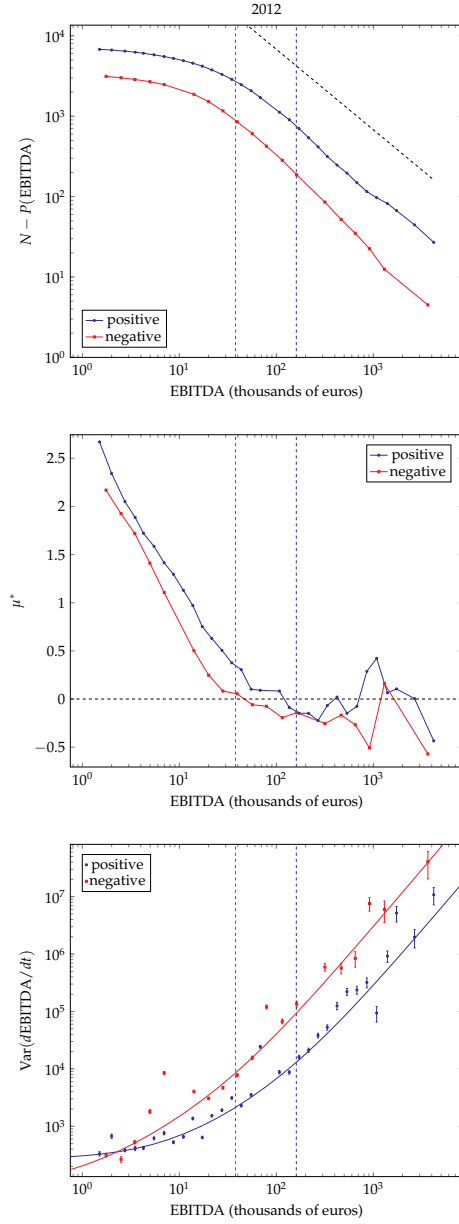

Figure 100: Castile-La Mancha

Rank plot, chemical potential and variance.

7095 Firms with positive EBITDA

$T_1 = 0.25 \pm 0.08$ ,  $T_{1/2} = 39.78 \pm 8.05$ , and  $T_0 = 265.76 \pm 74.91$

3443 Firms with negative EBITDA

Negative EBITDA:

$T_1 = 2.93 \pm 1.35$ ,  $T_{1/2} = 111.09 \pm 51.36$ , and  $T_0 = 90.62 \pm 156.06$ .

# Catalonia

## Tables of Temperatures

### Positive EBITDA

| Year | $T_1$           | $T_{1/2}$          | $T_0$               | $T_{1/2}/T_1$ | Num. Firms |
|------|-----------------|--------------------|---------------------|---------------|------------|
| 2003 | $0.50 \pm 0.07$ | $48.38 \pm 7.95$   | $466.66 \pm 102.50$ | 97.4          | 91748      |
| 2004 | $0.50 \pm 0.07$ | $44.21 \pm 8.53$   | $461.72 \pm 127.92$ | 87.8          | 93147      |
| 2005 | $0.52 \pm 0.08$ | $49.92 \pm 10.85$  | $804.09 \pm 177.05$ | 96.9          | 96104      |
| 2006 | $0.59 \pm 0.07$ | $72.39 \pm 8.81$   | $385.06 \pm 96.14$  | 123.4         | 100103     |
| 2007 | $0.58 \pm 0.14$ | $95.93 \pm 22.75$  | $614.89 \pm 257.65$ | 164.3         | 102128     |
| 2008 | $0.92 \pm 0.16$ | $96.05 \pm 21.44$  | $986.65 \pm 268.44$ | 104.1         | 89672      |
| 2009 | $1.13 \pm 0.18$ | $83.50 \pm 18.93$  | $679.47 \pm 182.65$ | 74.1          | 97832      |
| 2010 | $0.70 \pm 0.14$ | $86.53 \pm 17.41$  | $832.39 \pm 242.79$ | 124.0         | 95302      |
| 2011 | $0.61 \pm 0.11$ | $101.46 \pm 13.29$ | $351.91 \pm 113.49$ | 167.6         | 90294      |
| 2012 | $0.56 \pm 0.10$ | $75.48 \pm 14.07$  | $257.72 \pm 189.78$ | 135.6         | 49057      |

### Negative EBITDA

| Year | $T_1$           | $T_{1/2}$          | $T_0$                | $T_{1/2}/T_1$ | Num. Firms |
|------|-----------------|--------------------|----------------------|---------------|------------|
| 2003 | $2.83 \pm 0.33$ | $196.49 \pm 16.02$ | $199.59 \pm 68.38$   | 69.5          | 21739      |
| 2004 | $3.45 \pm 0.65$ | $159.71 \pm 35.77$ | $742.85 \pm 206.23$  | 46.3          | 21780      |
| 2005 | $1.79 \pm 0.44$ | $234.10 \pm 31.04$ | $530.45 \pm 190.00$  | 131.0         | 22515      |
| 2006 | $2.50 \pm 0.50$ | $210.02 \pm 31.61$ | $653.80 \pm 180.02$  | 83.9          | 23536      |
| 2007 | $2.40 \pm 0.93$ | $388.94 \pm 91.91$ | $327.31 \pm 439.99$  | 162.3         | 22162      |
| 2008 | $5.46 \pm 1.20$ | $323.96 \pm 77.06$ | $883.21 \pm 343.57$  | 59.3          | 21846      |
| 2009 | $3.41 \pm 0.75$ | $288.27 \pm 48.87$ | $913.16 \pm 288.99$  | 84.6          | 36525      |
| 2010 | $3.93 \pm 0.94$ | $221.44 \pm 58.41$ | $483.90 \pm 350.03$  | 56.3          | 38469      |
| 2011 | $3.14 \pm 0.62$ | $176.12 \pm 30.97$ | $405.63 \pm 144.13$  | 56.1          | 37913      |
| 2012 | $2.67 \pm 0.44$ | $96.67 \pm 29.39$  | $1588.39 \pm 270.19$ | 36.2          | 20407      |

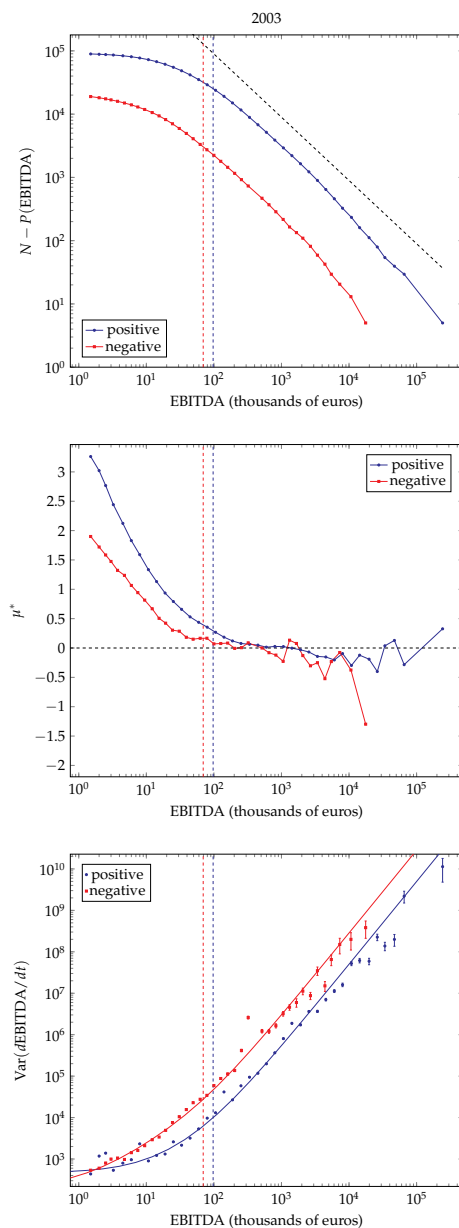

Figure 101: Catalonia

Rank plot, chemical potential and variance.

91748 Firms with positive EBITDA

 $T_1 = 0.50 \pm 0.07$ ,  $T_{1/2} = 48.38 \pm 7.95$ , and  $T_0 = 466.66 \pm 102.50$ 

21739 Firms with negative EBITDA

Negative EBITDA:

 $T_1 = 2.83 \pm 0.33$ ,  $T_{1/2} = 196.49 \pm 16.02$ , and  $T_0 = 199.59 \pm 68.38$ .

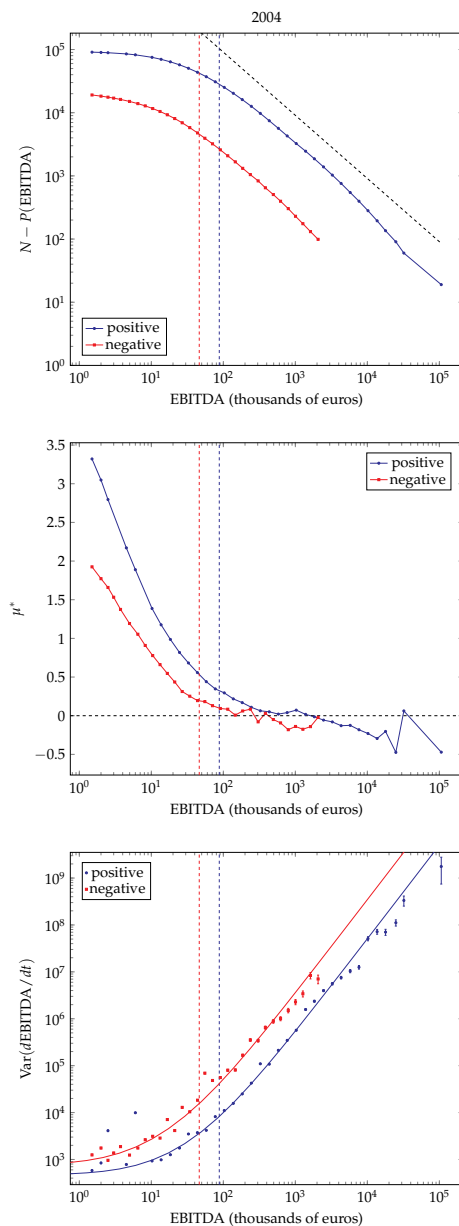

Figure 102: Catalonia

Rank plot, chemical potential and variance.

93147 Firms with positive EBITDA

$T_1 = 0.50 \pm 0.07$ ,  $T_{1/2} = 44.21 \pm 8.53$ , and  $T_0 = 461.72 \pm 127.92$

21780 Firms with negative EBITDA

Negative EBITDA:

$T_1 = 3.45 \pm 0.65$ ,  $T_{1/2} = 159.71 \pm 35.77$ , and  $T_0 = 742.85 \pm 206.23$ .

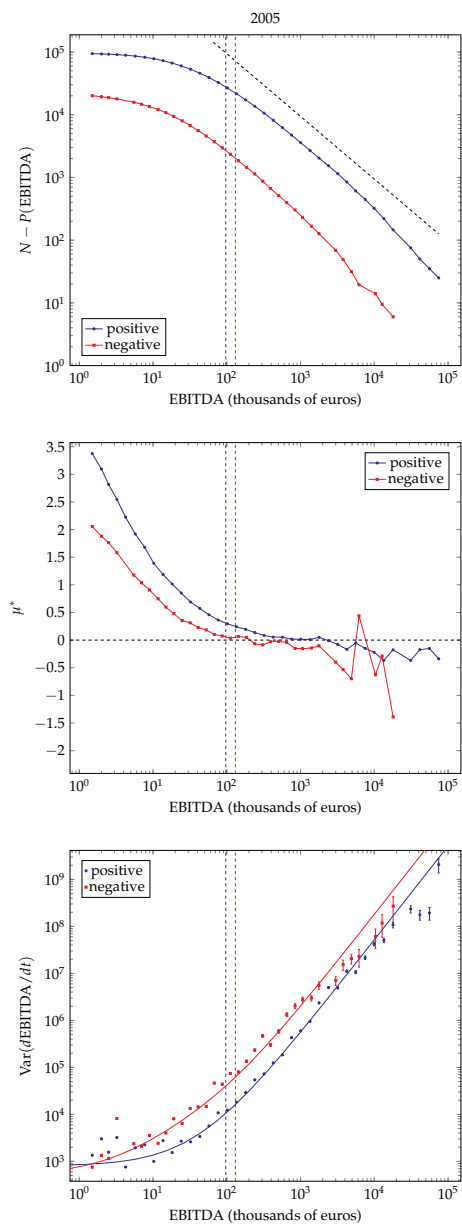

Figure 103: Catalonia

Rank plot, chemical potential and variance.

96104 Firms with positive EBITDA

$T_1 = 0.52 \pm 0.08$ ,  $T_{1/2} = 49.92 \pm 10.85$ , and  $T_0 = 804.09 \pm 177.05$

22515 Firms with negative EBITDA

Negative EBITDA:

$T_1 = 1.79 \pm 0.44$ ,  $T_{1/2} = 234.10 \pm 31.04$ , and  $T_0 = 530.45 \pm 190.00$ .

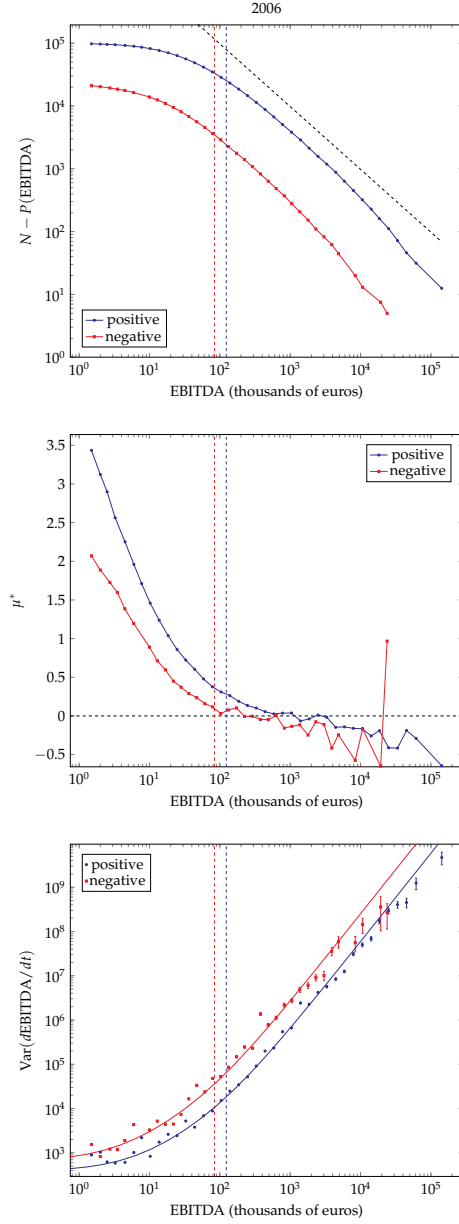

Figure 104: Catalonia

Rank plot, chemical potential and variance.

100103 Firms with positive EBITDA

$T_1 = 0.59 \pm 0.07$ ,  $T_{1/2} = 72.39 \pm 8.81$ , and  $T_0 = 385.06 \pm 96.14$

23536 Firms with negative EBITDA

Negative EBITDA:

$T_1 = 2.50 \pm 0.50$ ,  $T_{1/2} = 210.02 \pm 31.61$ , and  $T_0 = 653.80 \pm 180.02$ .

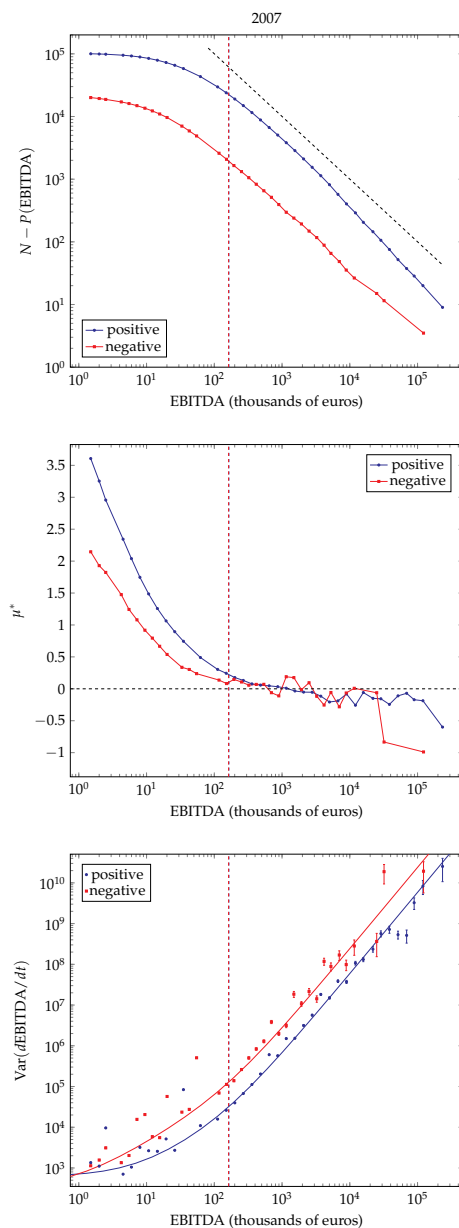

Figure 105: Catalonia

Rank plot, chemical potential and variance.

102128 Firms with positive EBITDA

 $T_1 = 0.58 \pm 0.14$ ,  $T_{1/2} = 95.93 \pm 22.75$ , and  $T_0 = 614.89 \pm 257.65$ 

22162 Firms with negative EBITDA

Negative EBITDA:

 $T_1 = 2.40 \pm 0.93$ ,  $T_{1/2} = 388.94 \pm 91.91$ , and  $T_0 = 327.31 \pm 439.99$ .

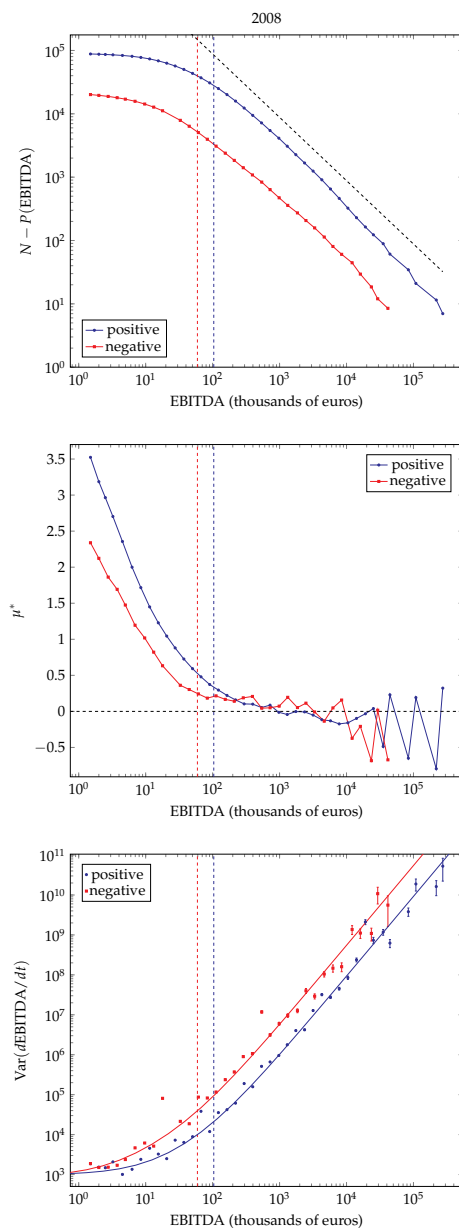

Figure 106: Catalonia

Rank plot, chemical potential and variance.

89672 Firms with positive EBITDA

$T_1 = 0.92 \pm 0.16$ ,  $T_{1/2} = 96.05 \pm 21.44$ , and  $T_0 = 986.65 \pm 268.44$

21846 Firms with negative EBITDA

Negative EBITDA:

$T_1 = 5.46 \pm 1.20$ ,  $T_{1/2} = 323.96 \pm 77.06$ , and  $T_0 = 883.21 \pm 343.57$ .

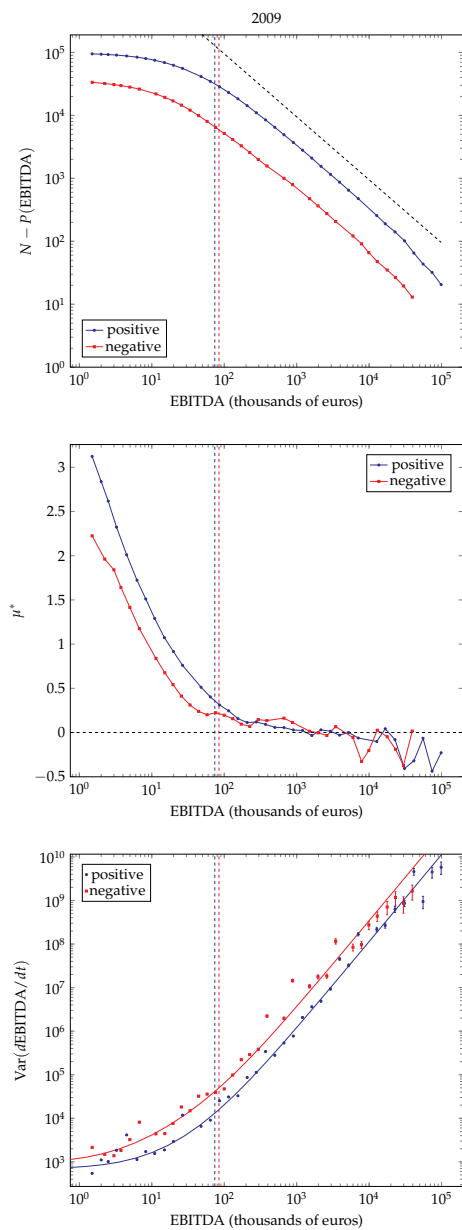

Figure 107: Catalonia

Rank plot, chemical potential and variance.

97832 Firms with positive EBITDA

 $T_1 = 1.13 \pm 0.18$ ,  $T_{1/2} = 83.50 \pm 18.93$ , and  $T_0 = 679.47 \pm 182.65$ 

36525 Firms with negative EBITDA

Negative EBITDA:

 $T_1 = 3.41 \pm 0.75$ ,  $T_{1/2} = 288.27 \pm 48.87$ , and  $T_0 = 913.16 \pm 288.99$ .

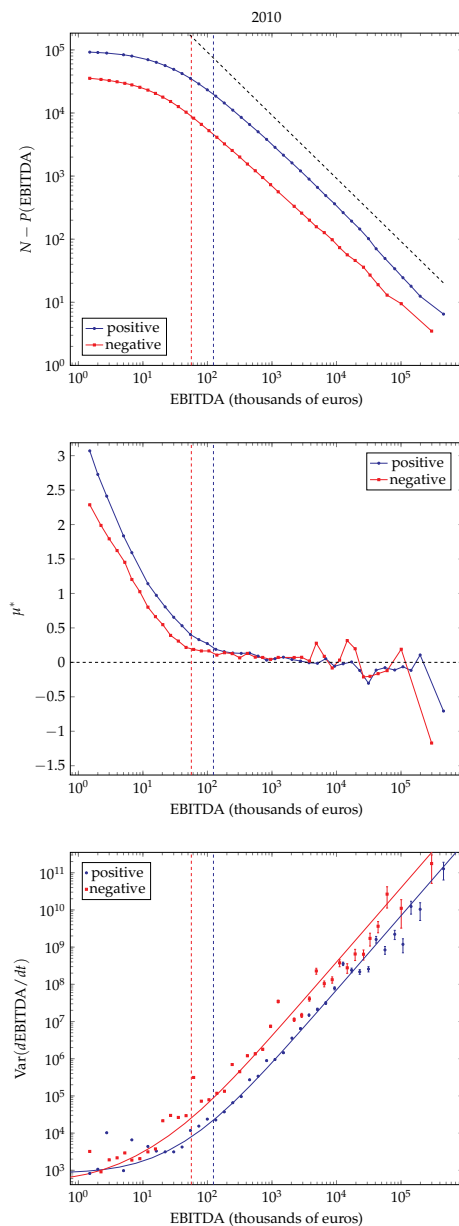

Figure 108: Catalonia

Rank plot, chemical potential and variance.

95302 Firms with positive EBITDA

 $T_1 = 0.70 \pm 0.14$ ,  $T_{1/2} = 86.53 \pm 17.41$ , and  $T_0 = 832.39 \pm 242.79$ 

38469 Firms with negative EBITDA

Negative EBITDA:

 $T_1 = 3.93 \pm 0.94$ ,  $T_{1/2} = 221.44 \pm 58.41$ , and  $T_0 = 483.90 \pm 350.03$ .

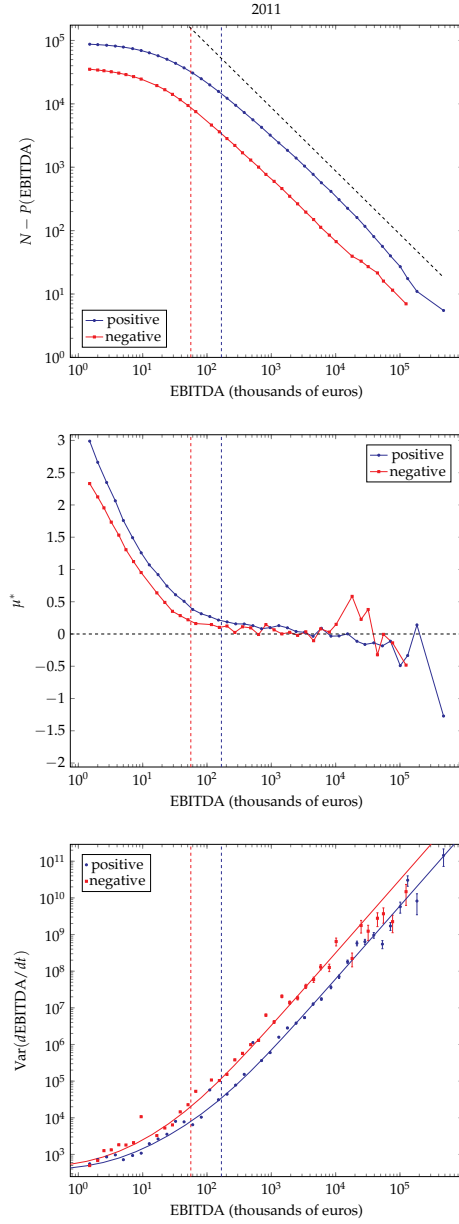

Figure 109: Catalonia

Rank plot, chemical potential and variance.

90294 Firms with positive EBITDA

 $T_1 = 0.61 \pm 0.11$ ,  $T_{1/2} = 101.46 \pm 13.29$ , and  $T_0 = 351.91 \pm 113.49$ 

37913 Firms with negative EBITDA

Negative EBITDA:

 $T_1 = 3.14 \pm 0.62$ ,  $T_{1/2} = 176.12 \pm 30.97$ , and  $T_0 = 405.63 \pm 144.13$ .

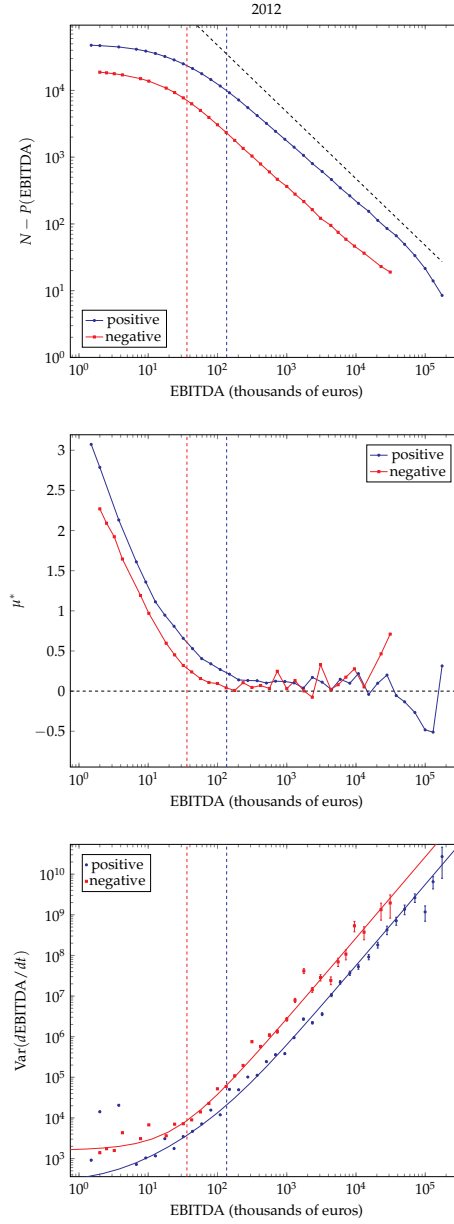

Figure 110: Catalonia

Rank plot, chemical potential and variance.

49057 Firms with positive EBITDA

$T_1 = 0.56 \pm 0.10$ ,  $T_{1/2} = 75.48 \pm 14.07$ , and  $T_0 = 257.72 \pm 189.78$

20407 Firms with negative EBITDA

Negative EBITDA:

$T_1 = 2.67 \pm 0.44$ ,  $T_{1/2} = 96.67 \pm 29.39$ , and  $T_0 = 1588.39 \pm 270.19$ .

# Extremadura

## Tables of Temperatures

### Positive EBITDA

| Year | $T_1$           | $T_{1/2}$         | $T_0$               | $T_{1/2}/T_1$ | Num. Firms |
|------|-----------------|-------------------|---------------------|---------------|------------|
| 2003 | $0.46 \pm 0.13$ | $21.56 \pm 10.63$ | $263.25 \pm 106.72$ | 47.2          | 7186       |
| 2004 | $0.45 \pm 0.15$ | $35.03 \pm 8.92$  | $141.39 \pm 61.93$  | 78.5          | 7582       |
| 2005 | $0.31 \pm 0.11$ | $38.66 \pm 9.19$  | $153.63 \pm 67.79$  | 123.0         | 7825       |
| 2006 | $0.49 \pm 0.08$ | $22.72 \pm 6.24$  | $412.86 \pm 66.23$  | 46.3          | 8027       |
| 2007 | $0.43 \pm 0.07$ | $30.41 \pm 6.85$  | $128.97 \pm 72.52$  | 71.3          | 8285       |
| 2008 | $0.72 \pm 0.12$ | $41.82 \pm 8.87$  | $93.89 \pm 70.69$   | 58.2          | 7281       |
| 2009 | $0.68 \pm 0.32$ | $80.84 \pm 31.85$ | $93.19 \pm 222.26$  | 118.8         | 7457       |
| 2010 | $0.39 \pm 0.15$ | $72.76 \pm 15.72$ | $264.30 \pm 111.82$ | 184.4         | 8285       |
| 2011 | $0.54 \pm 0.12$ | $88.64 \pm 11.57$ | $108.44 \pm 73.93$  | 162.9         | 7137       |
| 2012 | $0.08 \pm 0.14$ | $61.13 \pm 15.95$ | $97.61 \pm 101.52$  | 780.6         | 3135       |

### Negative EBITDA

| Year | $T_1$           | $T_{1/2}$          | $T_0$               | $T_{1/2}/T_1$ | Num. Firms |
|------|-----------------|--------------------|---------------------|---------------|------------|
| 2003 | $0.79 \pm 0.48$ | $112.91 \pm 28.61$ | $142.39 \pm 150.82$ | 142.7         | 1437       |
| 2004 | $0.56 \pm 0.62$ | $90.97 \pm 28.21$  | $123.42 \pm 92.76$  | 161.0         | 1472       |
| 2005 | $1.82 \pm 0.85$ | $60.16 \pm 36.70$  | $146.13 \pm 207.76$ | 33.0          | 1634       |
| 2006 | $0.85 \pm 0.87$ | $174.98 \pm 39.92$ | $24.49 \pm 86.54$   | 206.7         | 1595       |
| 2007 | $0.93 \pm 0.79$ | $179.37 \pm 44.57$ | $169.82 \pm 138.86$ | 192.8         | 1562       |
| 2008 | $4.28 \pm 1.18$ | $142.39 \pm 52.28$ | $590.59 \pm 279.17$ | 33.2          | 1375       |
| 2009 | $3.90 \pm 1.60$ | $180.33 \pm 89.57$ | $572.47 \pm 442.14$ | 46.2          | 2029       |
| 2010 | $2.18 \pm 0.79$ | $124.36 \pm 30.63$ | $235.15 \pm 109.38$ | 57.0          | 2558       |
| 2011 | $2.57 \pm 1.23$ | $216.50 \pm 54.59$ | $153.63 \pm 187.54$ | 84.2          | 2360       |
| 2012 | $1.22 \pm 0.36$ | $115.45 \pm 20.90$ | $124.21 \pm 95.86$  | 94.9          | 1311       |

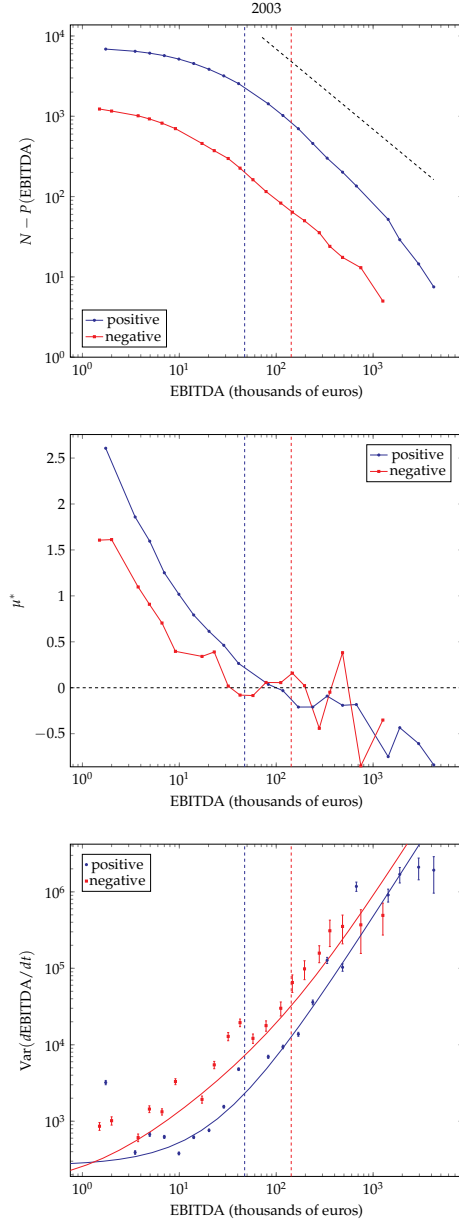

Figure 111: Extremadura

Rank plot, chemical potential and variance.

7186 Firms with positive EBITDA

$T_1 = 0.46 \pm 0.13$ ,  $T_{1/2} = 21.56 \pm 10.63$ , and  $T_0 = 263.25 \pm 106.72$

1437 Firms with negative EBITDA

Negative EBITDA:

$T_1 = 0.79 \pm 0.48$ ,  $T_{1/2} = 112.91 \pm 28.61$ , and  $T_0 = 142.39 \pm 150.82$ .

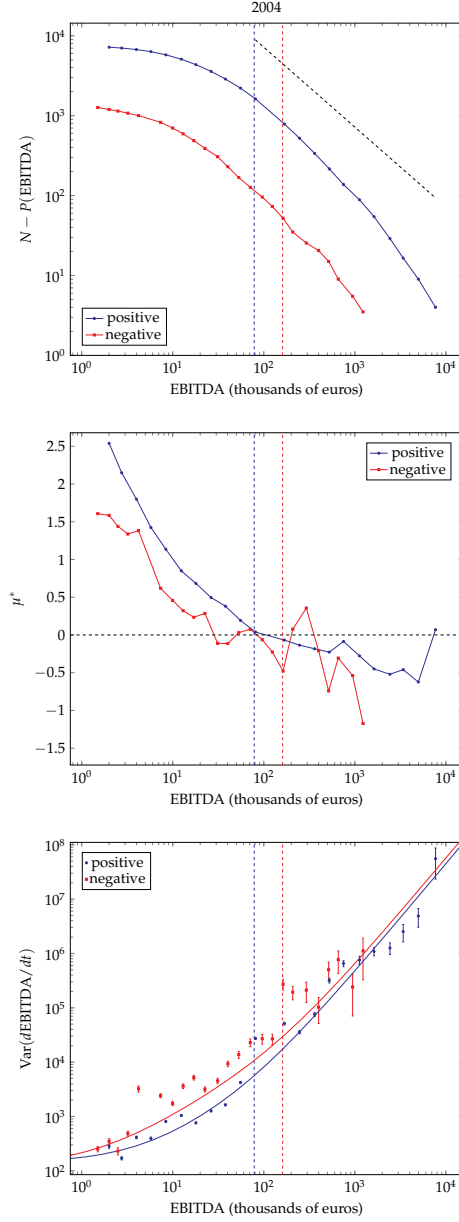

Figure 112: Extremadura

Rank plot, chemical potential and variance.

7582 Firms with positive EBITDA

$T_1 = 0.45 \pm 0.15$ ,  $T_{1/2} = 35.03 \pm 8.92$ , and  $T_0 = 141.39 \pm 61.93$

1472 Firms with negative EBITDA

Negative EBITDA:

$T_1 = 0.56 \pm 0.62$ ,  $T_{1/2} = 90.97 \pm 28.21$ , and  $T_0 = 123.42 \pm 92.76$ .

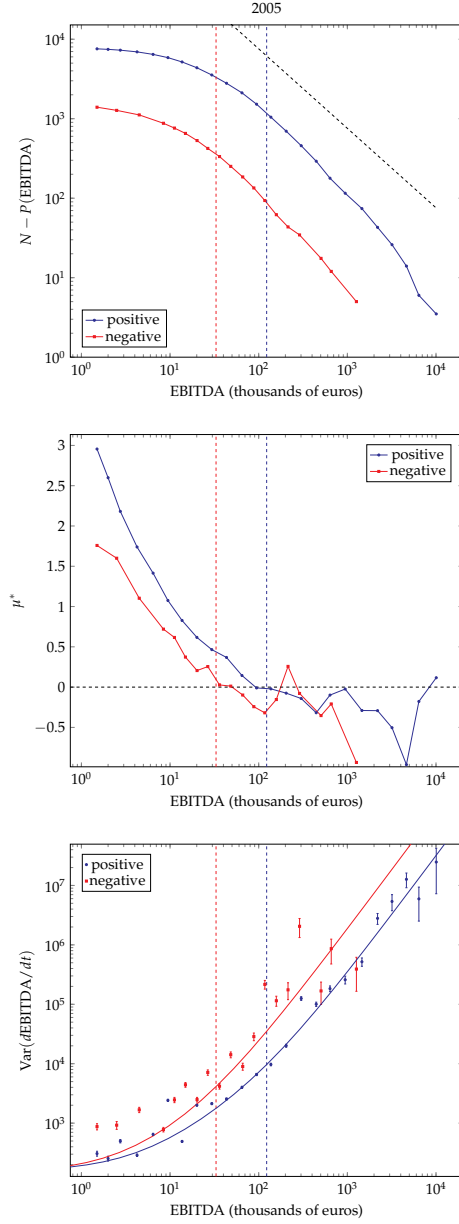

Figure 113: Extremadura

Rank plot, chemical potential and variance.

7825 Firms with positive EBITDA

$T_1 = 0.31 \pm 0.11$ ,  $T_{1/2} = 38.66 \pm 9.19$ , and  $T_0 = 153.63 \pm 67.79$

1634 Firms with negative EBITDA

Negative EBITDA:

$T_1 = 1.82 \pm 0.85$ ,  $T_{1/2} = 60.16 \pm 36.70$ , and  $T_0 = 146.13 \pm 207.76$ .

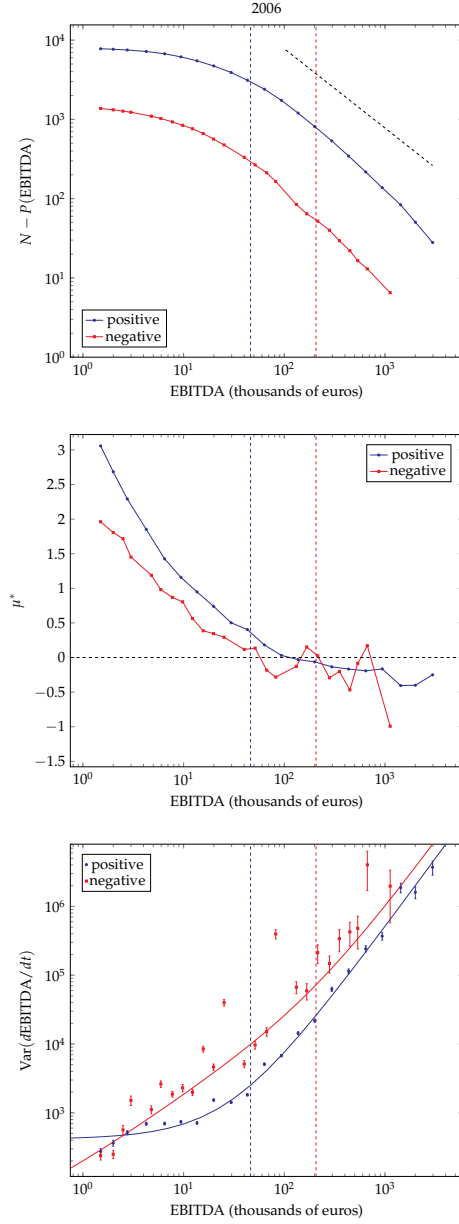

Figure 114: Extremadura

Rank plot, chemical potential and variance.

8027 Firms with positive EBITDA

$T_1 = 0.49 \pm 0.08$ ,  $T_{1/2} = 22.72 \pm 6.24$ , and  $T_0 = 412.86 \pm 66.23$

1595 Firms with negative EBITDA

Negative EBITDA:

$T_1 = 0.85 \pm 0.87$ ,  $T_{1/2} = 174.98 \pm 39.92$ , and  $T_0 = 24.49 \pm 86.54$ .

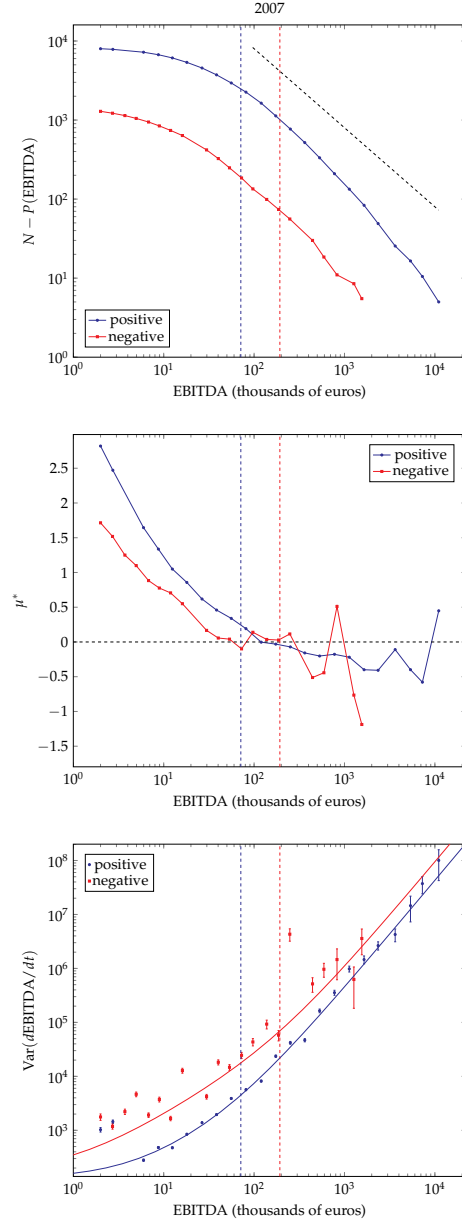

Figure 115: Extremadura

Rank plot, chemical potential and variance.

8285 Firms with positive EBITDA

$T_1 = 0.43 \pm 0.07$ ,  $T_{1/2} = 30.41 \pm 6.85$ , and  $T_0 = 128.97 \pm 72.52$

1562 Firms with negative EBITDA

Negative EBITDA:

$T_1 = 0.93 \pm 0.79$ ,  $T_{1/2} = 179.37 \pm 44.57$ , and  $T_0 = 169.82 \pm 138.86$ .

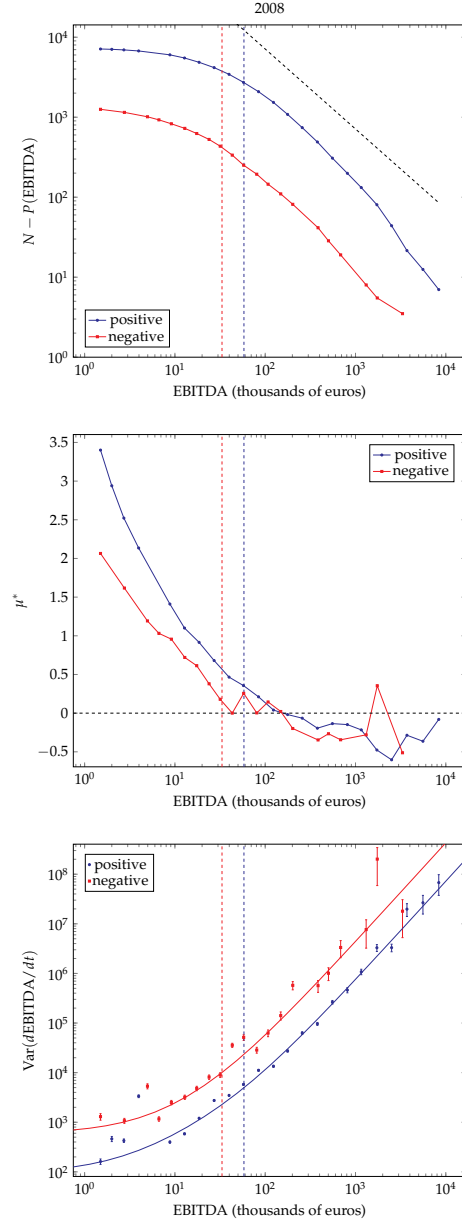

Figure 116: Extremadura

Rank plot, chemical potential and variance.

7281 Firms with positive EBITDA

$T_1 = 0.72 \pm 0.12$ ,  $T_{1/2} = 41.82 \pm 8.87$ , and  $T_0 = 93.89 \pm 70.69$

1375 Firms with negative EBITDA

Negative EBITDA:

$T_1 = 4.28 \pm 1.18$ ,  $T_{1/2} = 142.39 \pm 52.28$ , and  $T_0 = 590.59 \pm 279.17$ .

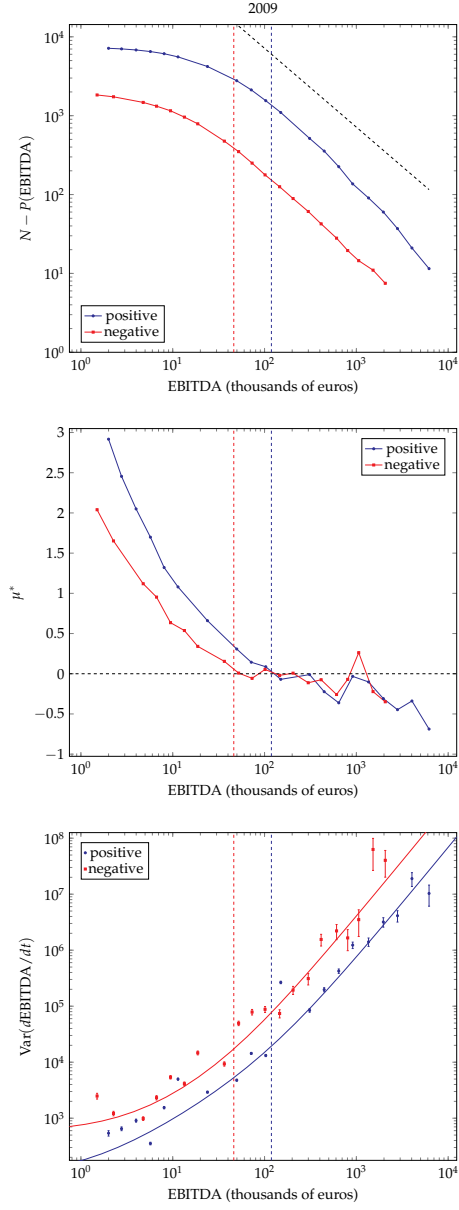

Figure 117: Extremadura

Rank plot, chemical potential and variance.

7457 Firms with positive EBITDA

$T_1 = 0.68 \pm 0.32$ ,  $T_{1/2} = 80.84 \pm 31.85$ , and  $T_0 = 93.19 \pm 222.26$

2029 Firms with negative EBITDA

Negative EBITDA:

$T_1 = 3.90 \pm 1.60$ ,  $T_{1/2} = 180.33 \pm 89.57$ , and  $T_0 = 572.47 \pm 442.14$ .

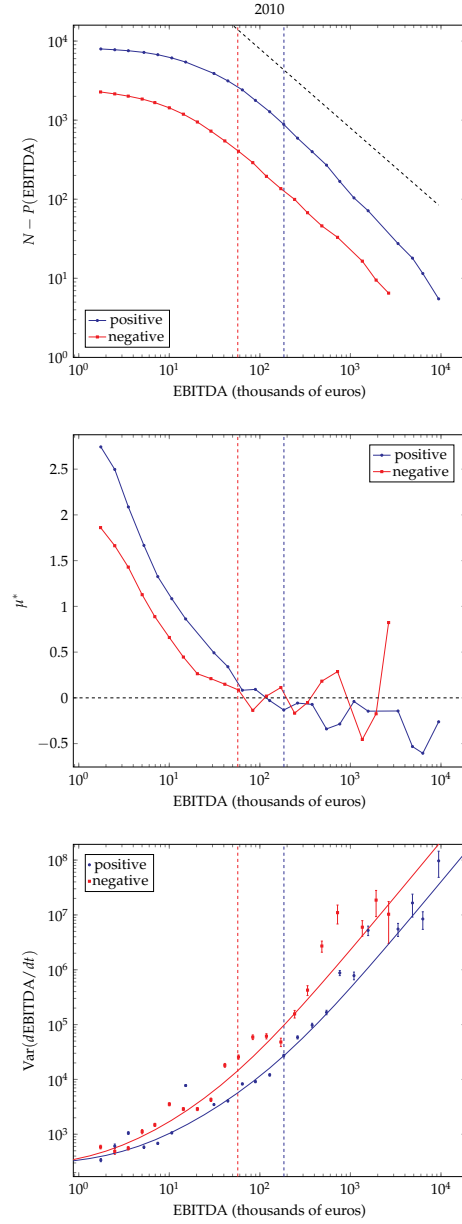

Figure 118: Extremadura

Rank plot, chemical potential and variance.

8285 Firms with positive EBITDA

$T_1 = 0.39 \pm 0.15$ ,  $T_{1/2} = 72.76 \pm 15.72$ , and  $T_0 = 264.30 \pm 111.82$

2558 Firms with negative EBITDA

Negative EBITDA:

$T_1 = 2.18 \pm 0.79$ ,  $T_{1/2} = 124.36 \pm 30.63$ , and  $T_0 = 235.15 \pm 109.38$ .

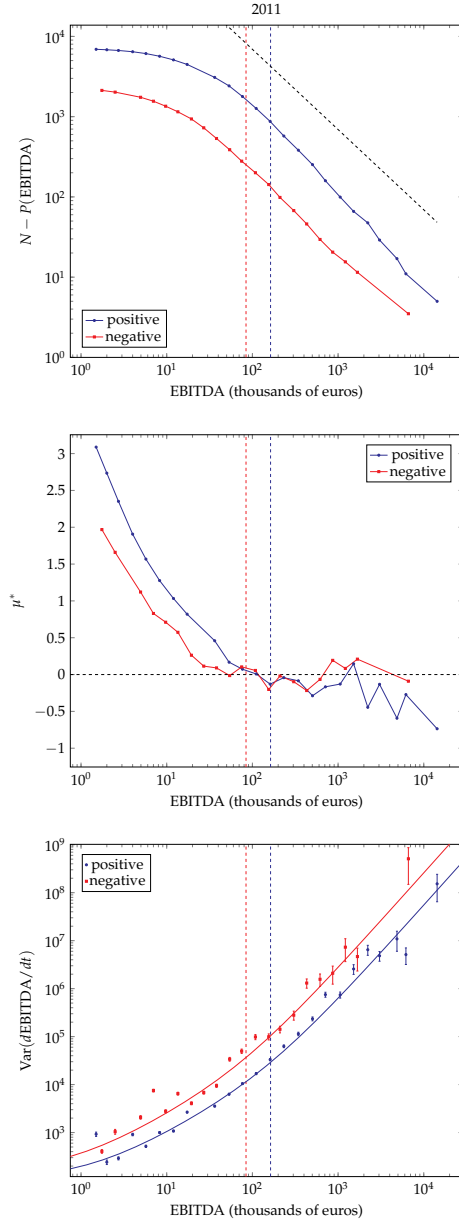

Figure 119: Extremadura

Rank plot, chemical potential and variance.

7137 Firms with positive EBITDA

$T_1 = 0.54 \pm 0.12$ ,  $T_{1/2} = 88.64 \pm 11.57$ , and  $T_0 = 108.44 \pm 73.93$

2360 Firms with negative EBITDA

Negative EBITDA:

$T_1 = 2.57 \pm 1.23$ ,  $T_{1/2} = 216.50 \pm 54.59$ , and  $T_0 = 153.63 \pm 187.54$ .

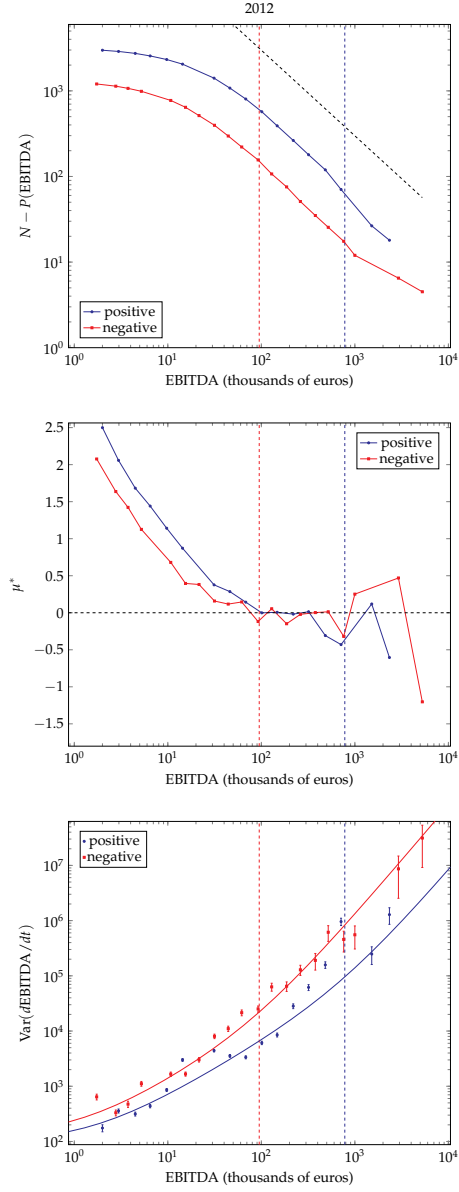

Figure 120: Extremadura

Rank plot, chemical potential and variance.

3135 Firms with positive EBITDA

$T_1 = 0.08 \pm 0.14$ ,  $T_{1/2} = 61.13 \pm 15.95$ , and  $T_0 = 97.61 \pm 101.52$

1311 Firms with negative EBITDA

Negative EBITDA:

$T_1 = 1.22 \pm 0.36$ ,  $T_{1/2} = 115.45 \pm 20.90$ , and  $T_0 = 124.21 \pm 95.86$ .

# Galicia

## Tables of Temperatures

### Positive EBITDA

| Year | $T_1$           | $T_{1/2}$         | $T_0$               | $T_{1/2}/T_1$ | Num. Firms |
|------|-----------------|-------------------|---------------------|---------------|------------|
| 2003 | $0.25 \pm 0.06$ | $33.70 \pm 6.74$  | $229.03 \pm 81.85$  | 134.5         | 24528      |
| 2004 | $0.43 \pm 0.08$ | $31.69 \pm 6.98$  | $118.56 \pm 65.73$  | 73.4          | 25688      |
| 2005 | $0.48 \pm 0.06$ | $25.87 \pm 4.66$  | $197.16 \pm 45.44$  | 53.8          | 27216      |
| 2006 | $0.37 \pm 0.09$ | $40.04 \pm 8.65$  | $217.42 \pm 80.87$  | 106.8         | 29185      |
| 2007 | $0.59 \pm 0.07$ | $43.12 \pm 5.17$  | $84.55 \pm 32.87$   | 73.7          | 35512      |
| 2008 | $0.64 \pm 0.14$ | $56.61 \pm 12.01$ | $245.10 \pm 97.54$  | 88.9          | 34380      |
| 2009 | $0.66 \pm 0.13$ | $79.38 \pm 11.39$ | $174.25 \pm 80.32$  | 120.1         | 32216      |
| 2010 | $0.58 \pm 0.08$ | $47.30 \pm 6.88$  | $275.14 \pm 56.16$  | 82.2          | 33708      |
| 2011 | $0.72 \pm 0.16$ | $69.00 \pm 15.74$ | $181.76 \pm 143.96$ | 95.6          | 29566      |
| 2012 | $0.11 \pm 0.05$ | $63.75 \pm 7.83$  | $165.64 \pm 68.27$  | 567.8         | 20251      |

### Negative EBITDA

| Year | $T_1$           | $T_{1/2}$          | $T_0$               | $T_{1/2}/T_1$ | Num. Firms |
|------|-----------------|--------------------|---------------------|---------------|------------|
| 2003 | $2.26 \pm 0.71$ | $110.32 \pm 24.55$ | $107.56 \pm 84.97$  | 48.9          | 5344       |
| 2004 | $1.14 \pm 0.56$ | $174.17 \pm 33.79$ | $199.95 \pm 175.92$ | 153.4         | 5509       |
| 2005 | $1.84 \pm 0.76$ | $178.30 \pm 28.63$ | $72.46 \pm 94.03$   | 96.8          | 5926       |
| 2006 | $2.81 \pm 0.72$ | $100.23 \pm 24.71$ | $193.86 \pm 107.56$ | 35.7          | 6740       |
| 2007 | $2.46 \pm 0.86$ | $116.17 \pm 38.36$ | $219.49 \pm 141.23$ | 47.3          | 9015       |
| 2008 | $3.18 \pm 1.03$ | $89.71 \pm 37.06$  | $337.28 \pm 156.64$ | 28.2          | 9000       |
| 2009 | $5.15 \pm 1.21$ | $175.08 \pm 43.46$ | $177.36 \pm 150.86$ | 34.0          | 10933      |
| 2010 | $1.57 \pm 0.48$ | $118.46 \pm 20.01$ | $316.71 \pm 97.18$  | 75.7          | 13500      |
| 2011 | $3.39 \pm 0.97$ | $170.52 \pm 33.00$ | $18.25 \pm 106.91$  | 50.3          | 12371      |
| 2012 | $2.56 \pm 0.53$ | $48.01 \pm 19.70$  | $246.85 \pm 105.05$ | 18.8          | 10958      |

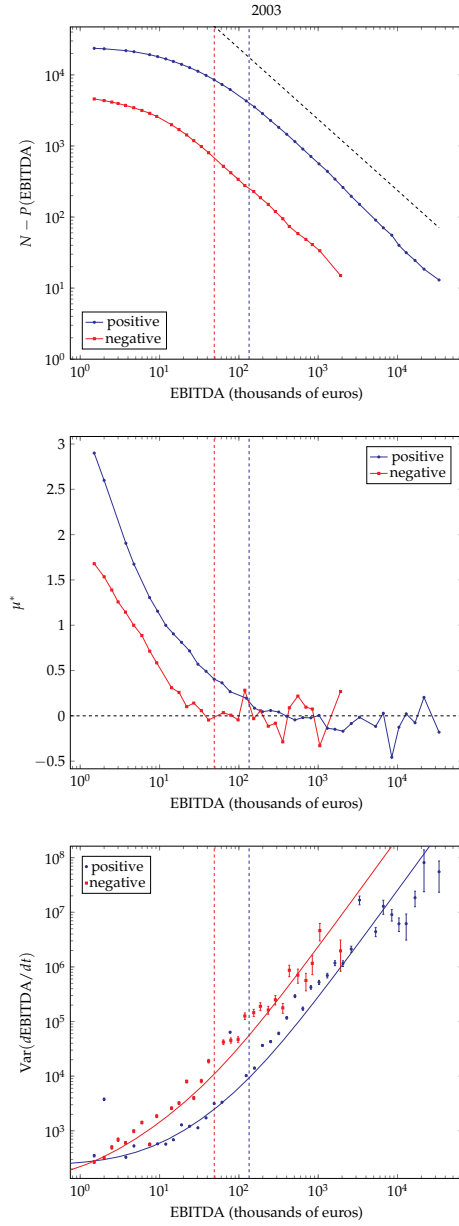

Figure 121: Galicia

Rank plot, chemical potential and variance.

24528 Firms with positive EBITDA

$T_1 = 0.25 \pm 0.06$ ,  $T_{1/2} = 33.70 \pm 6.74$ , and  $T_0 = 229.03 \pm 81.85$

5344 Firms with negative EBITDA

Negative EBITDA:

$T_1 = 2.26 \pm 0.71$ ,  $T_{1/2} = 110.32 \pm 24.55$ , and  $T_0 = 107.56 \pm 84.97$ .

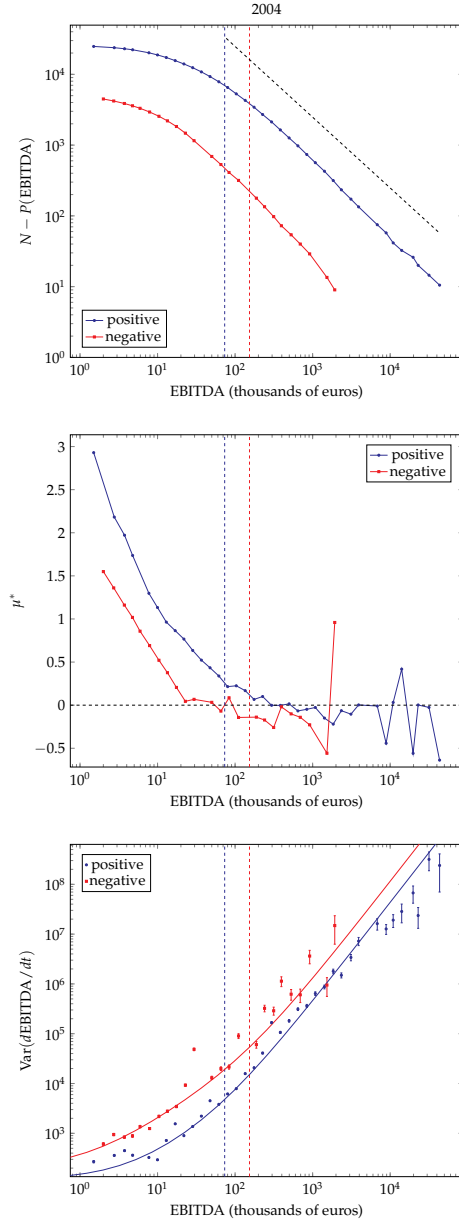

Figure 122: Galicia

Rank plot, chemical potential and variance.

25688 Firms with positive EBITDA

$T_1 = 0.43 \pm 0.08$ ,  $T_{1/2} = 31.69 \pm 6.98$ , and  $T_0 = 118.56 \pm 65.73$

5509 Firms with negative EBITDA

Negative EBITDA:

$T_1 = 1.14 \pm 0.56$ ,  $T_{1/2} = 174.17 \pm 33.79$ , and  $T_0 = 199.95 \pm 175.92$ .

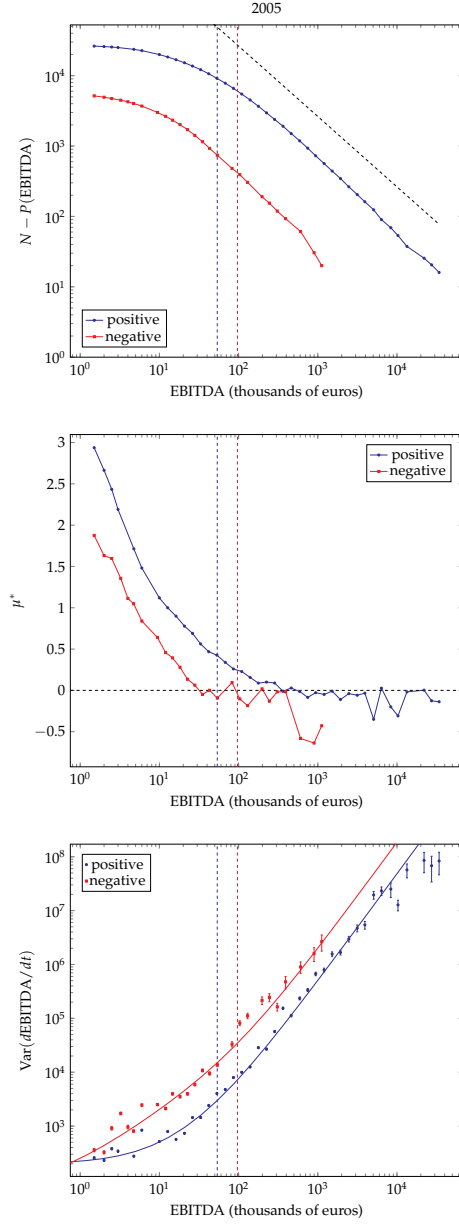

Figure 123: Galicia

Rank plot, chemical potential and variance.

27216 Firms with positive EBITDA

$T_1 = 0.48 \pm 0.06$ ,  $T_{1/2} = 25.87 \pm 4.66$ , and  $T_0 = 197.16 \pm 45.44$

5926 Firms with negative EBITDA

Negative EBITDA:

$T_1 = 1.84 \pm 0.76$ ,  $T_{1/2} = 178.30 \pm 28.63$ , and  $T_0 = 72.46 \pm 94.03$ .

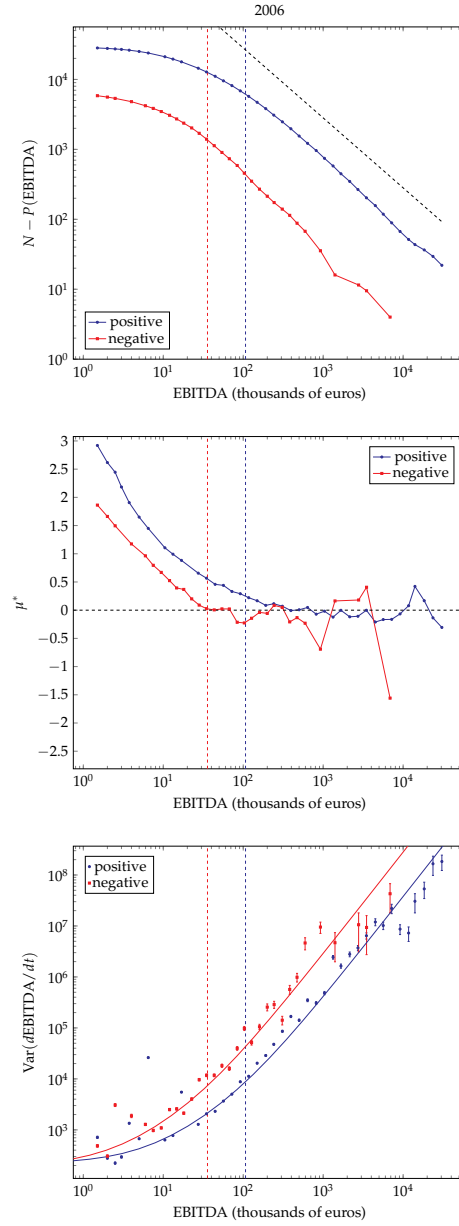

Figure 124: Galicia

Rank plot, chemical potential and variance.

29185 Firms with positive EBITDA

$T_1 = 0.37 \pm 0.09$ ,  $T_{1/2} = 40.04 \pm 8.65$ , and  $T_0 = 217.42 \pm 80.87$

6740 Firms with negative EBITDA

Negative EBITDA:

$T_1 = 2.81 \pm 0.72$ ,  $T_{1/2} = 100.23 \pm 24.71$ , and  $T_0 = 193.86 \pm 107.56$ .

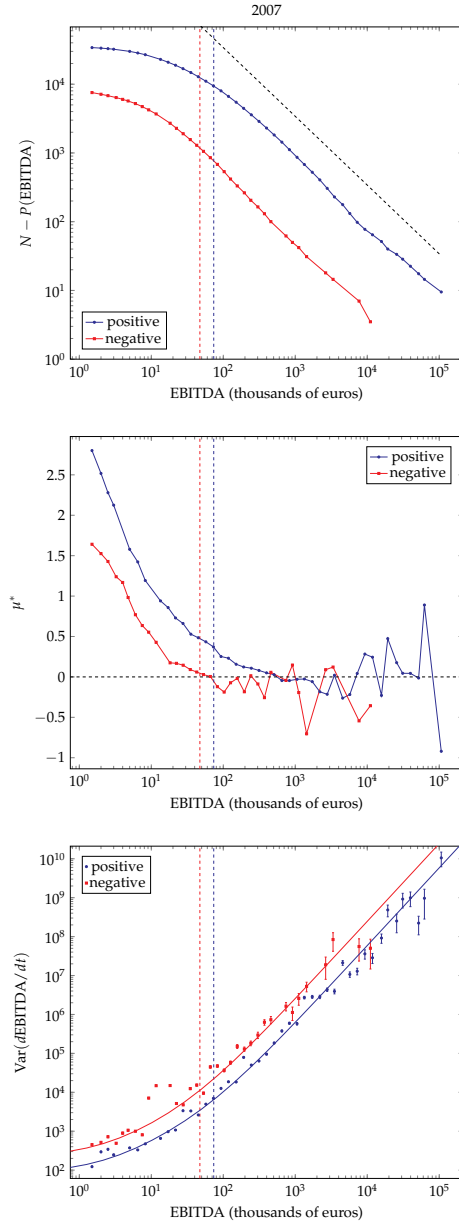

Figure 125: Galicia

Rank plot, chemical potential and variance.

35512 Firms with positive EBITDA

$T_1 = 0.59 \pm 0.07$ ,  $T_{1/2} = 43.12 \pm 5.17$ , and  $T_0 = 84.55 \pm 32.87$

9015 Firms with negative EBITDA

Negative EBITDA:

$T_1 = 2.46 \pm 0.86$ ,  $T_{1/2} = 116.17 \pm 38.36$ , and  $T_0 = 219.49 \pm 141.23$ .

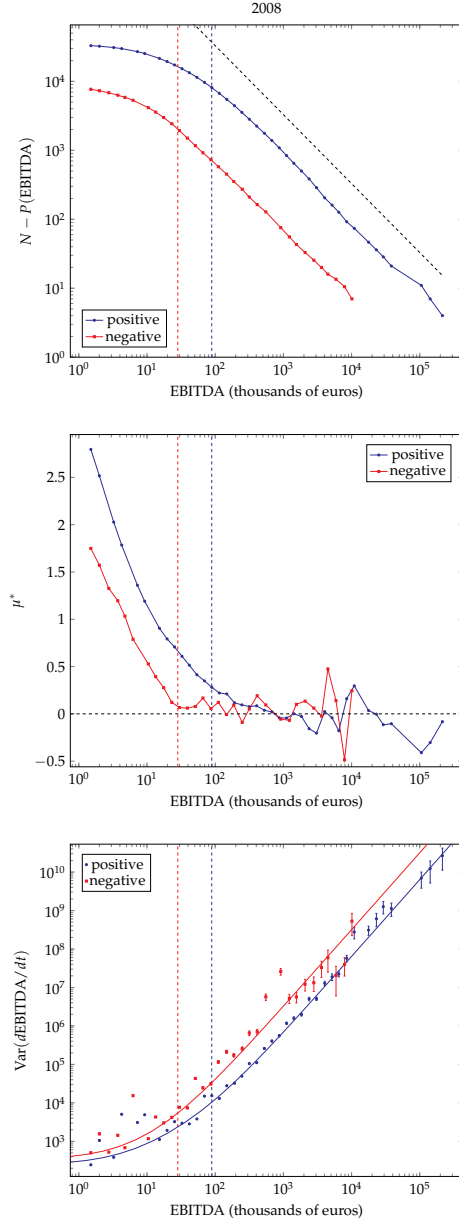

Figure 126: Galicia

Rank plot, chemical potential and variance.

34380 Firms with positive EBITDA

$T_1 = 0.64 \pm 0.14$ ,  $T_{1/2} = 56.61 \pm 12.01$ , and  $T_0 = 245.10 \pm 97.54$

9000 Firms with negative EBITDA

Negative EBITDA:

$T_1 = 3.18 \pm 1.03$ ,  $T_{1/2} = 89.71 \pm 37.06$ , and  $T_0 = 337.28 \pm 156.64$ .

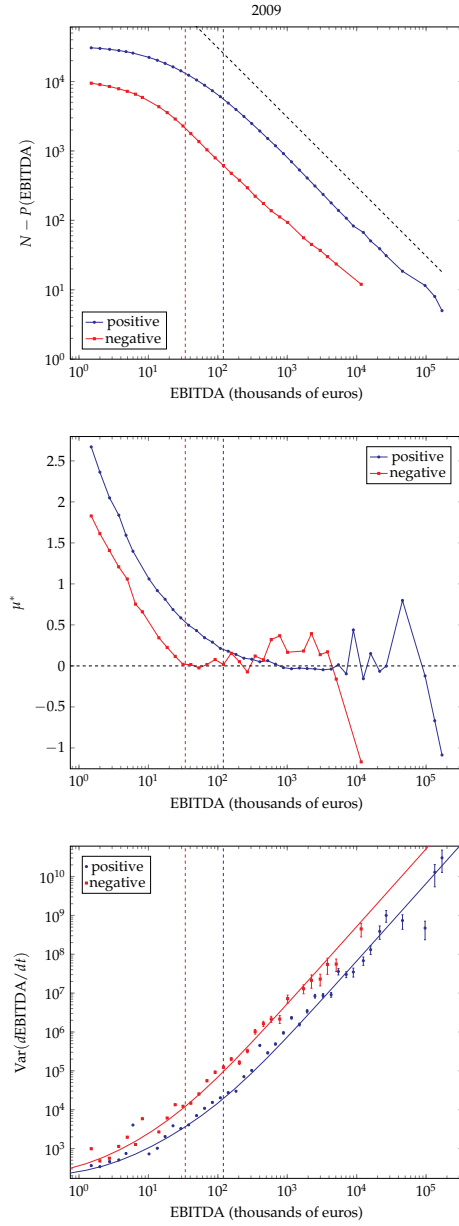

Figure 127: Galicia

Rank plot, chemical potential and variance.

32216 Firms with positive EBITDA

$T_1 = 0.66 \pm 0.13$ ,  $T_{1/2} = 79.38 \pm 11.39$ , and  $T_0 = 174.25 \pm 80.32$

10933 Firms with negative EBITDA

Negative EBITDA:

$T_1 = 5.15 \pm 1.21$ ,  $T_{1/2} = 175.08 \pm 43.46$ , and  $T_0 = 177.36 \pm 150.86$ .

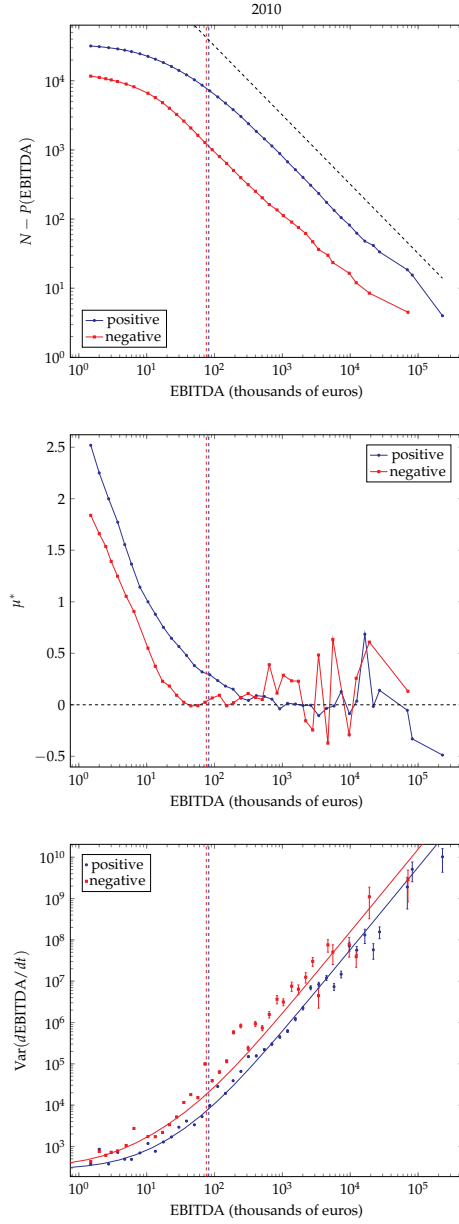

Figure 128: Galicia

Rank plot, chemical potential and variance.

33708 Firms with positive EBITDA

$T_1 = 0.58 \pm 0.08$ ,  $T_{1/2} = 47.30 \pm 6.88$ , and  $T_0 = 275.14 \pm 56.16$

13500 Firms with negative EBITDA

Negative EBITDA:

$T_1 = 1.57 \pm 0.48$ ,  $T_{1/2} = 118.46 \pm 20.01$ , and  $T_0 = 316.71 \pm 97.18$ .

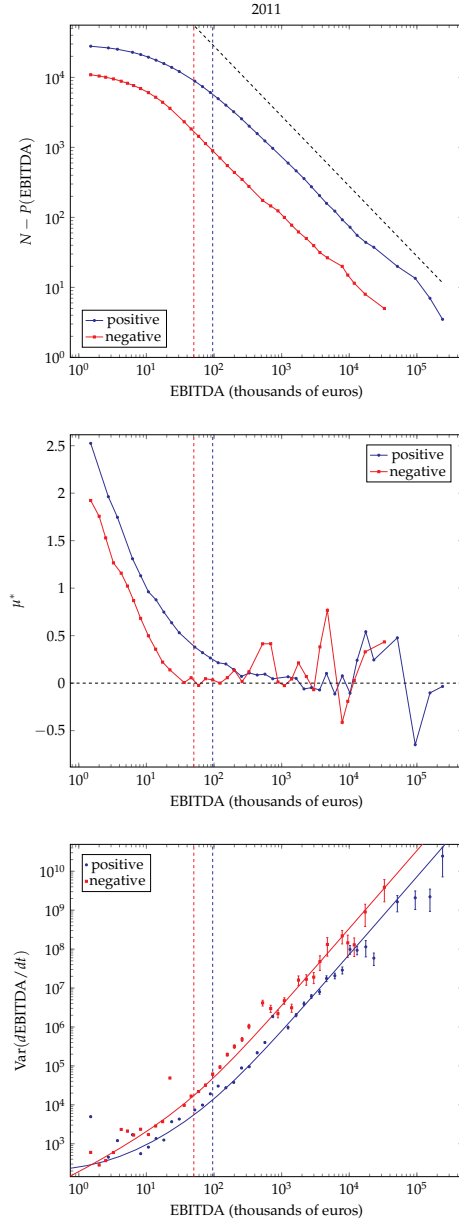

Figure 129: Galicia

Rank plot, chemical potential and variance.

29566 Firms with positive EBITDA

$T_1 = 0.72 \pm 0.16$ ,  $T_{1/2} = 69.00 \pm 15.74$ , and  $T_0 = 181.76 \pm 143.96$

12371 Firms with negative EBITDA

Negative EBITDA:

$T_1 = 3.39 \pm 0.97$ ,  $T_{1/2} = 170.52 \pm 33.00$ , and  $T_0 = 18.25 \pm 106.91$ .

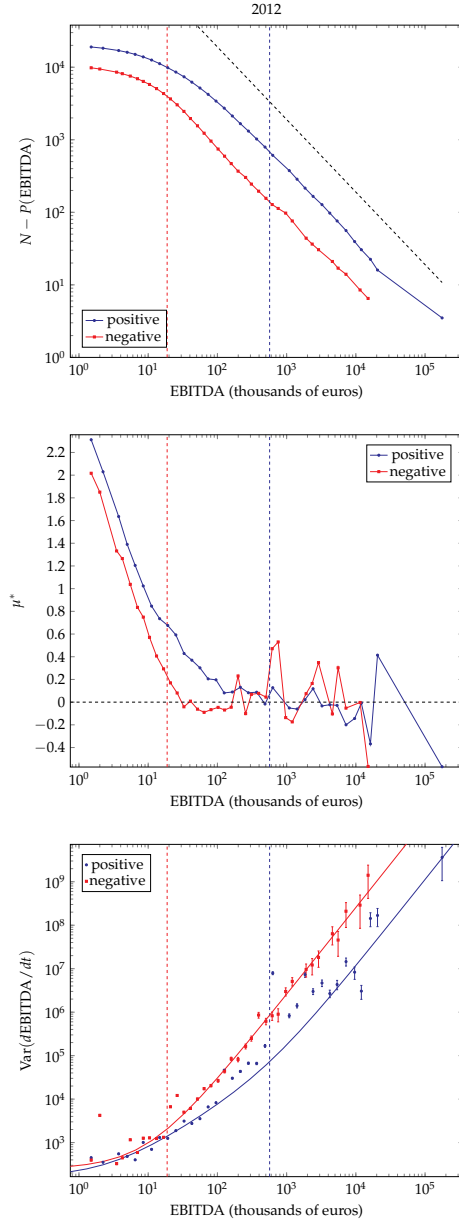

Figure 130: Galicia

Rank plot, chemical potential and variance.

20251 Firms with positive EBITDA

$T_1 = 0.11 \pm 0.05$ ,  $T_{1/2} = 63.75 \pm 7.83$ , and  $T_0 = 165.64 \pm 68.27$

10958 Firms with negative EBITDA

Negative EBITDA:

$T_1 = 2.56 \pm 0.53$ ,  $T_{1/2} = 48.01 \pm 19.70$ , and  $T_0 = 246.85 \pm 105.05$ .

# La Rioja

## Tables of Temperatures

### Positive EBITDA

| Year | $T_1$           | $T_{1/2}$          | $T_0$               | $T_{1/2}/T_1$ | Num. Firms |
|------|-----------------|--------------------|---------------------|---------------|------------|
| 2003 | $0.24 \pm 0.04$ | $23.68 \pm 5.48$   | $168.05 \pm 65.12$  | 98.0          | 3067       |
| 2004 | $0.43 \pm 0.08$ | $16.09 \pm 8.15$   | $300.94 \pm 115.71$ | 37.3          | 3247       |
| 2005 | $0.34 \pm 0.10$ | $33.72 \pm 9.86$   | $102.50 \pm 75.98$  | 100.5         | 3571       |
| 2006 | $0.32 \pm 0.09$ | $54.06 \pm 11.06$  | $0.09 \pm 54.02$    | 167.1         | 3696       |
| 2007 | $0.31 \pm 0.09$ | $41.74 \pm 11.80$  | $94.52 \pm 127.88$  | 133.0         | 3505       |
| 2008 | $0.56 \pm 0.11$ | $44.52 \pm 13.29$  | $526.28 \pm 192.17$ | 79.4          | 3068       |
| 2009 | $0.61 \pm 0.15$ | $84.86 \pm 24.43$  | $682.68 \pm 401.72$ | 138.0         | 3120       |
| 2010 | $0.30 \pm 0.11$ | $71.80 \pm 17.09$  | $144.98 \pm 252.77$ | 241.6         | 3395       |
| 2011 | $0.11 \pm 0.07$ | $123.72 \pm 20.37$ | $124.54 \pm 276.77$ | 1127.4        | 3048       |
| 2012 | $0.24 \pm 0.07$ | $61.82 \pm 10.45$  | $257.44 \pm 146.59$ | 256.9         | 1768       |

### Negative EBITDA

| Year | $T_1$           | $T_{1/2}$          | $T_0$                | $T_{1/2}/T_1$ | Num. Firms |
|------|-----------------|--------------------|----------------------|---------------|------------|
| 2003 | $0.41 \pm 0.38$ | $106.23 \pm 33.30$ | $196.33 \pm 155.80$  | 257.1         | 583        |
| 2004 | $1.27 \pm 0.71$ | $62.86 \pm 36.37$  | $592.68 \pm 244.70$  | 49.5          | 605        |
| 2005 | $2.84 \pm 1.79$ | $92.19 \pm 54.54$  | $171.41 \pm 141.06$  | 32.5          | 739        |
| 2006 | $0.62 \pm 0.72$ | $157.42 \pm 55.13$ | $371.77 \pm 418.25$  | 254.8         | 691        |
| 2007 | $2.19 \pm 0.63$ | $129.59 \pm 31.54$ | $111.19 \pm 161.42$  | 59.2          | 603        |
| 2008 | $1.24 \pm 0.70$ | $66.77 \pm 53.98$  | $1028.34 \pm 721.60$ | 53.7          | 554        |
| 2009 | $5.23 \pm 1.70$ | $168.65 \pm 73.35$ | $270.71 \pm 319.10$  | 32.3          | 891        |
| 2010 | $0.53 \pm 0.52$ | $165.20 \pm 42.05$ | $351.62 \pm 214.35$  | 311.2         | 1273       |
| 2011 | $1.75 \pm 1.06$ | $258.96 \pm 58.97$ | $74.14 \pm 223.85$   | 148.4         | 1140       |
| 2012 | $1.84 \pm 0.58$ | $73.28 \pm 33.31$  | $428.62 \pm 235.21$  | 39.9          | 739        |

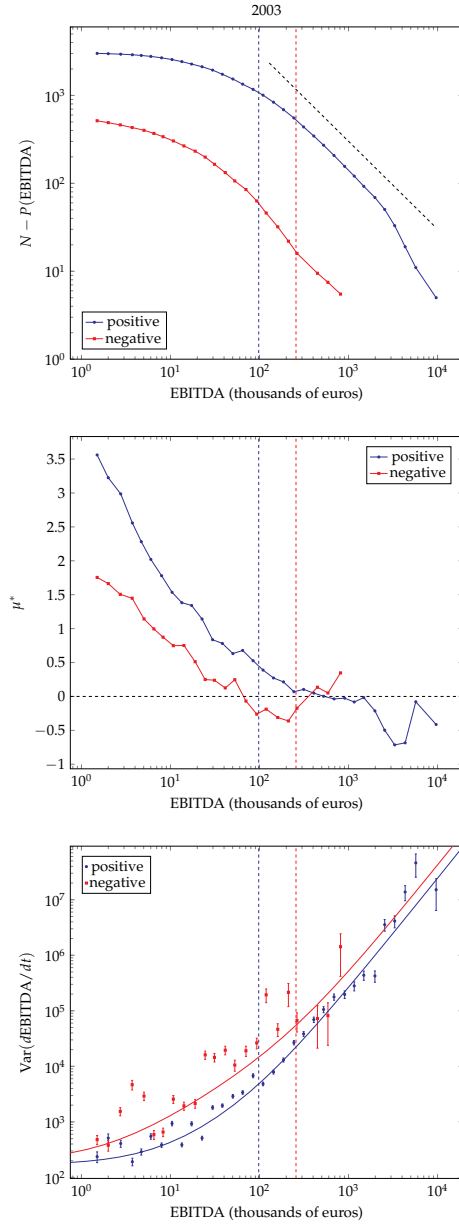

Figure 131: La Rioja

Rank plot, chemical potential and variance.

3067 Firms with positive EBITDA

$T_1 = 0.24 \pm 0.04$ ,  $T_{1/2} = 23.68 \pm 5.48$ , and  $T_0 = 168.05 \pm 65.12$

583 Firms with negative EBITDA

Negative EBITDA:

$T_1 = 0.41 \pm 0.38$ ,  $T_{1/2} = 106.23 \pm 33.30$ , and  $T_0 = 196.33 \pm 155.80$ .

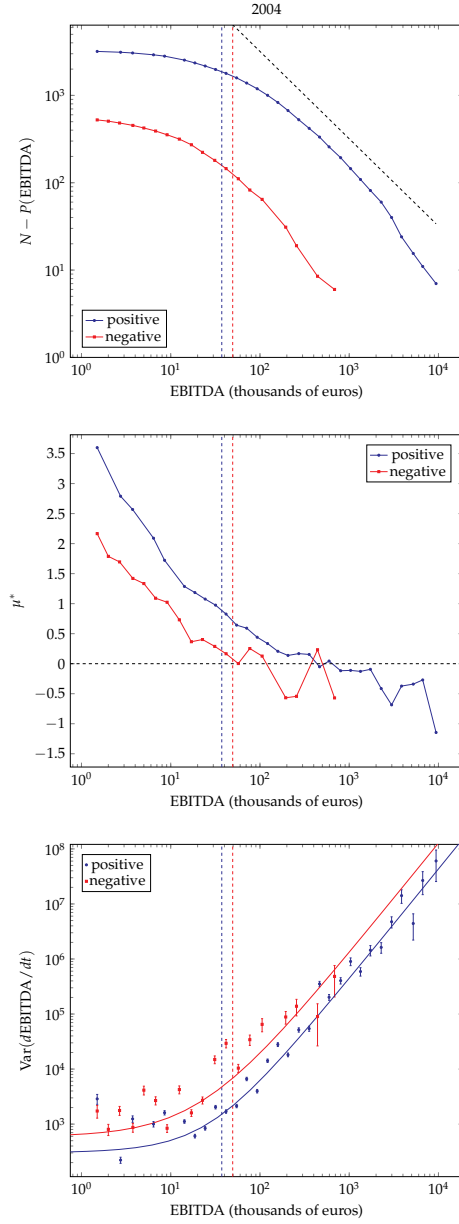

Figure 132: La Rioja

Rank plot, chemical potential and variance.

3247 Firms with positive EBITDA

$T_1 = 0.43 \pm 0.08$ ,  $T_{1/2} = 16.09 \pm 8.15$ , and  $T_0 = 300.94 \pm 115.71$

605 Firms with negative EBITDA

Negative EBITDA:

$T_1 = 1.27 \pm 0.71$ ,  $T_{1/2} = 62.86 \pm 36.37$ , and  $T_0 = 592.68 \pm 244.70$ .

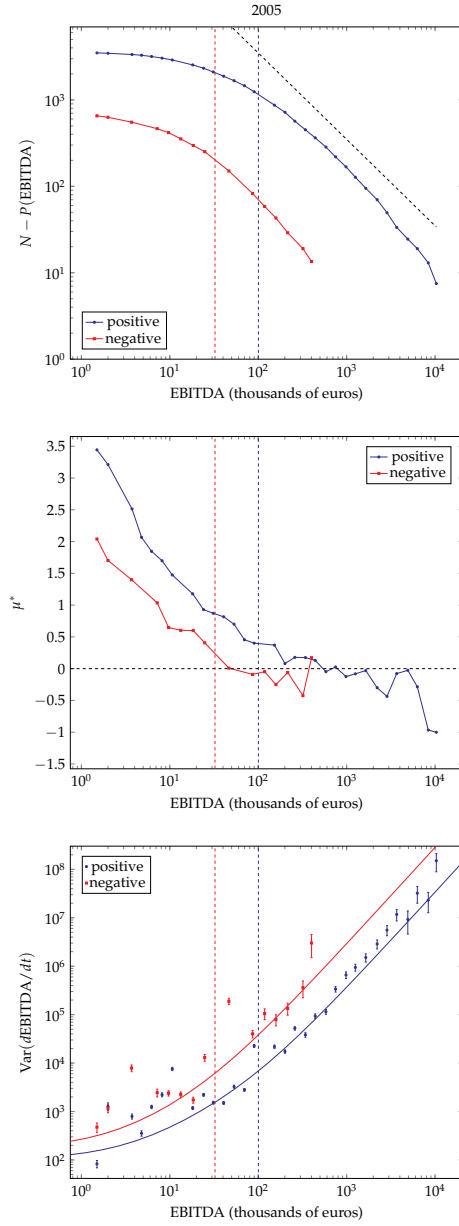

Figure 133: La Rioja

Rank plot, chemical potential and variance.

3571 Firms with positive EBITDA

$T_1 = 0.34 \pm 0.10$ ,  $T_{1/2} = 33.72 \pm 9.86$ , and  $T_0 = 102.50 \pm 75.98$

739 Firms with negative EBITDA

Negative EBITDA:

$T_1 = 2.84 \pm 1.79$ ,  $T_{1/2} = 92.19 \pm 54.54$ , and  $T_0 = 171.41 \pm 141.06$ .

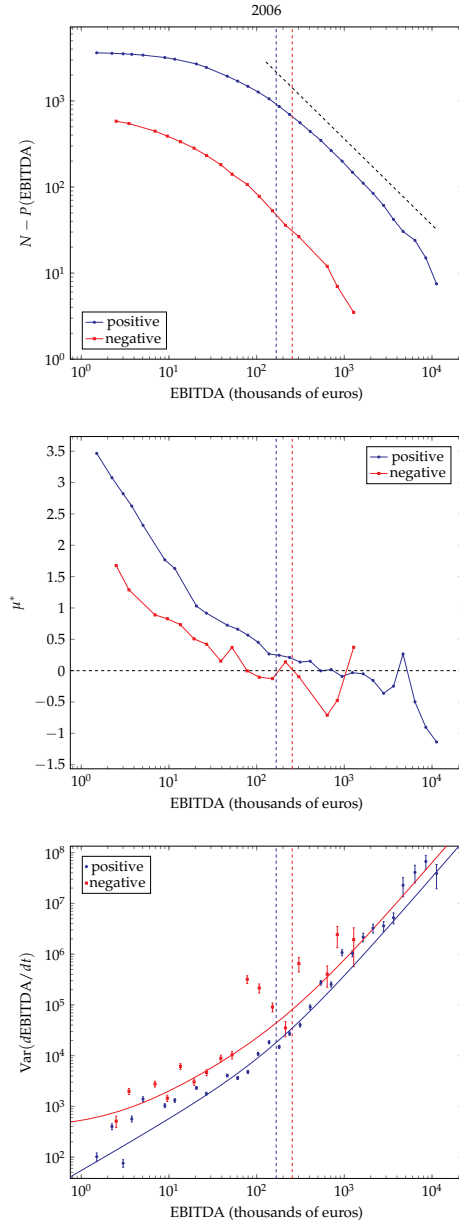

Figure 134: La Rioja

Rank plot, chemical potential and variance.

3696 Firms with positive EBITDA

$T_1 = 0.32 \pm 0.09$ ,  $T_{1/2} = 54.06 \pm 11.06$ , and  $T_0 = 0.09 \pm 54.02$

691 Firms with negative EBITDA

Negative EBITDA:

$T_1 = 0.62 \pm 0.72$ ,  $T_{1/2} = 157.42 \pm 55.13$ , and  $T_0 = 371.77 \pm 418.25$ .

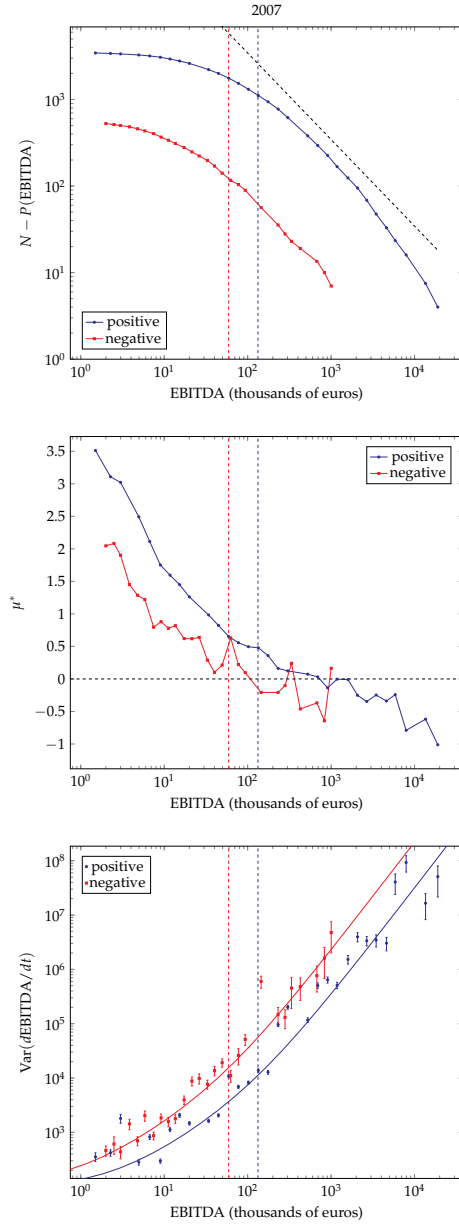

Figure 135: La Rioja

Rank plot, chemical potential and variance.

3505 Firms with positive EBITDA

$T_1 = 0.31 \pm 0.09$ ,  $T_{1/2} = 41.74 \pm 11.80$ , and  $T_0 = 94.52 \pm 127.88$

603 Firms with negative EBITDA

Negative EBITDA:

$T_1 = 2.19 \pm 0.63$ ,  $T_{1/2} = 129.59 \pm 31.54$ , and  $T_0 = 111.19 \pm 161.42$ .

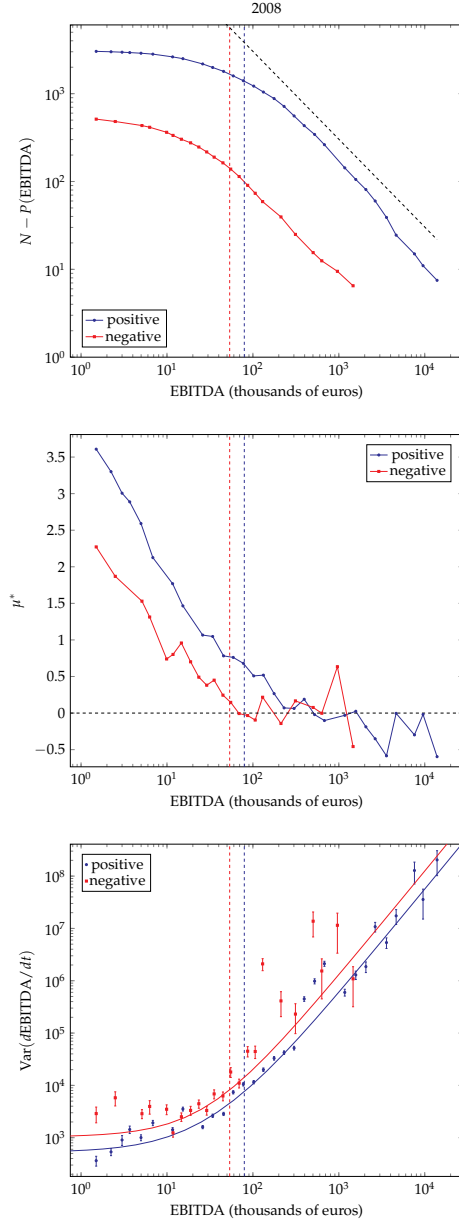

Figure 136: La Rioja

Rank plot, chemical potential and variance.

3068 Firms with positive EBITDA

$T_1 = 0.56 \pm 0.11$ ,  $T_{1/2} = 44.52 \pm 13.29$ , and  $T_0 = 526.28 \pm 192.17$

554 Firms with negative EBITDA

Negative EBITDA:

$T_1 = 1.24 \pm 0.70$ ,  $T_{1/2} = 66.77 \pm 53.98$ , and  $T_0 = 1028.34 \pm 721.60$ .

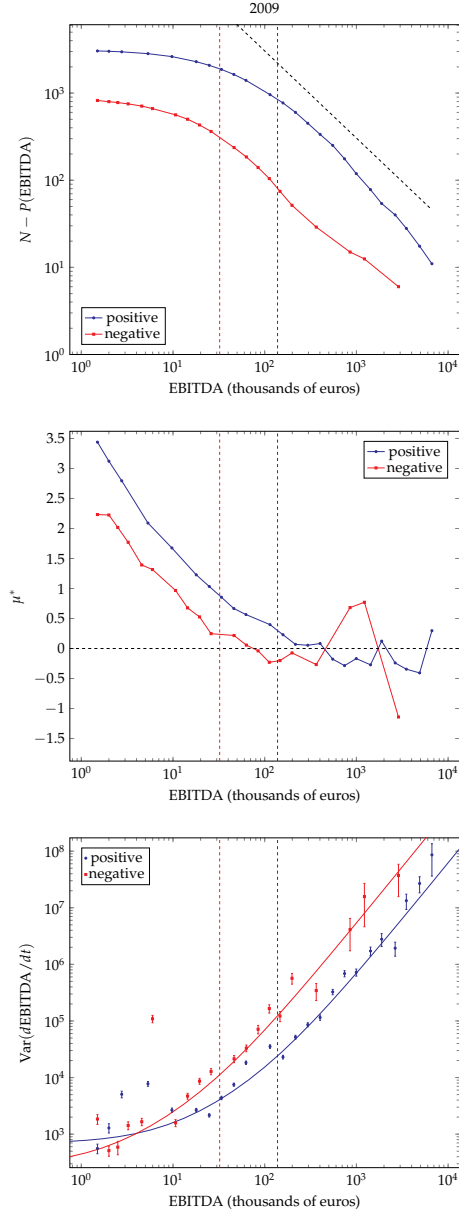

Figure 137: La Rioja

Rank plot, chemical potential and variance.

3120 Firms with positive EBITDA

$T_1 = 0.61 \pm 0.15$ ,  $T_{1/2} = 84.86 \pm 24.43$ , and  $T_0 = 682.68 \pm 401.72$

891 Firms with negative EBITDA

Negative EBITDA:

$T_1 = 5.23 \pm 1.70$ ,  $T_{1/2} = 168.65 \pm 73.35$ , and  $T_0 = 270.71 \pm 319.10$ .

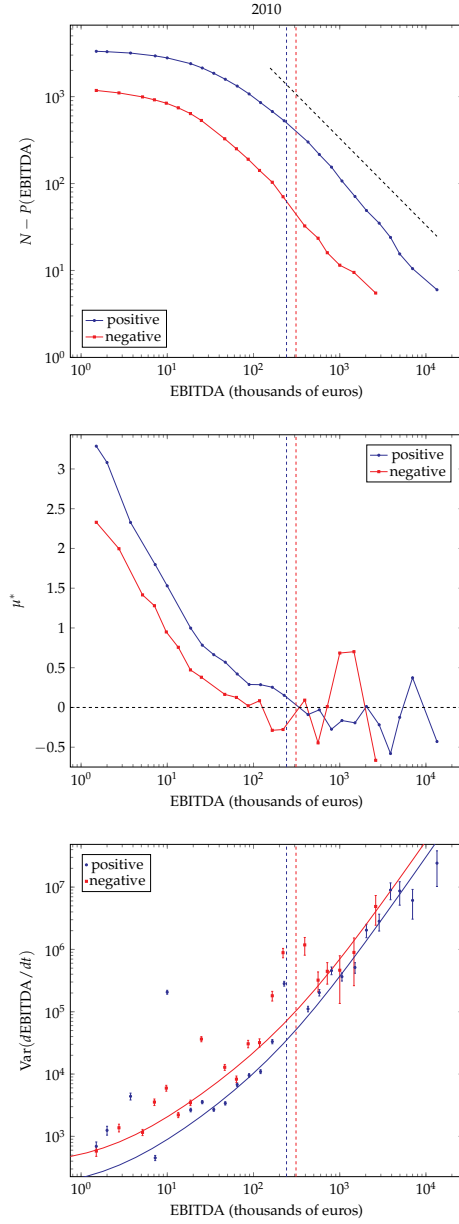

Figure 138: La Rioja

Rank plot, chemical potential and variance.

3395 Firms with positive EBITDA

$T_1 = 0.30 \pm 0.11$ ,  $T_{1/2} = 71.80 \pm 17.09$ , and  $T_0 = 144.98 \pm 252.77$

1273 Firms with negative EBITDA

Negative EBITDA:

$T_1 = 0.53 \pm 0.52$ ,  $T_{1/2} = 165.20 \pm 42.05$ , and  $T_0 = 351.62 \pm 214.35$ .

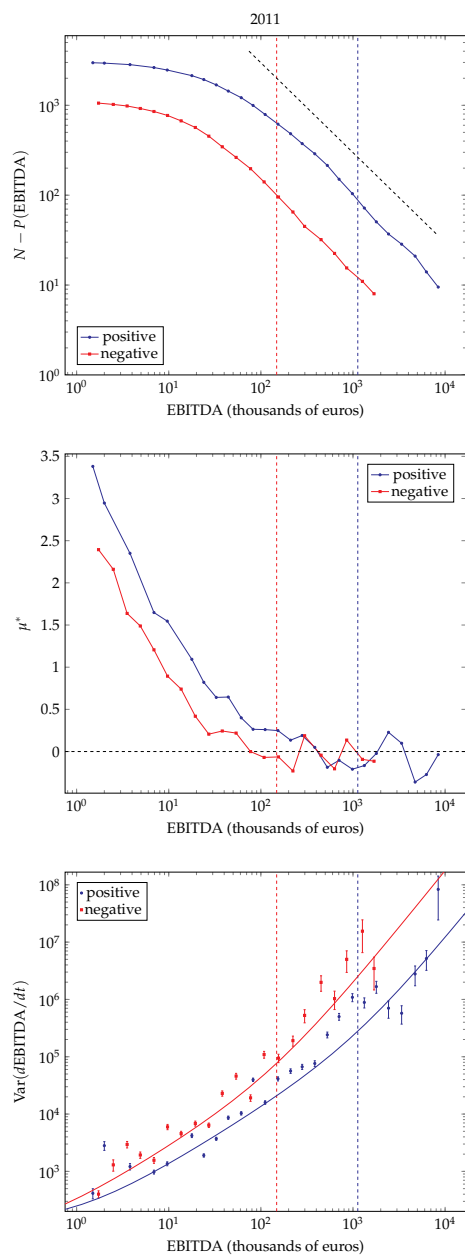

Figure 139: La Rioja

Rank plot, chemical potential and variance.

3048 Firms with positive EBITDA

$T_1 = 0.11 \pm 0.07$ ,  $T_{1/2} = 123.72 \pm 20.37$ , and  $T_0 = 124.54 \pm 276.77$

1140 Firms with negative EBITDA

Negative EBITDA:

$T_1 = 1.75 \pm 1.06$ ,  $T_{1/2} = 258.96 \pm 58.97$ , and  $T_0 = 74.14 \pm 223.85$ .

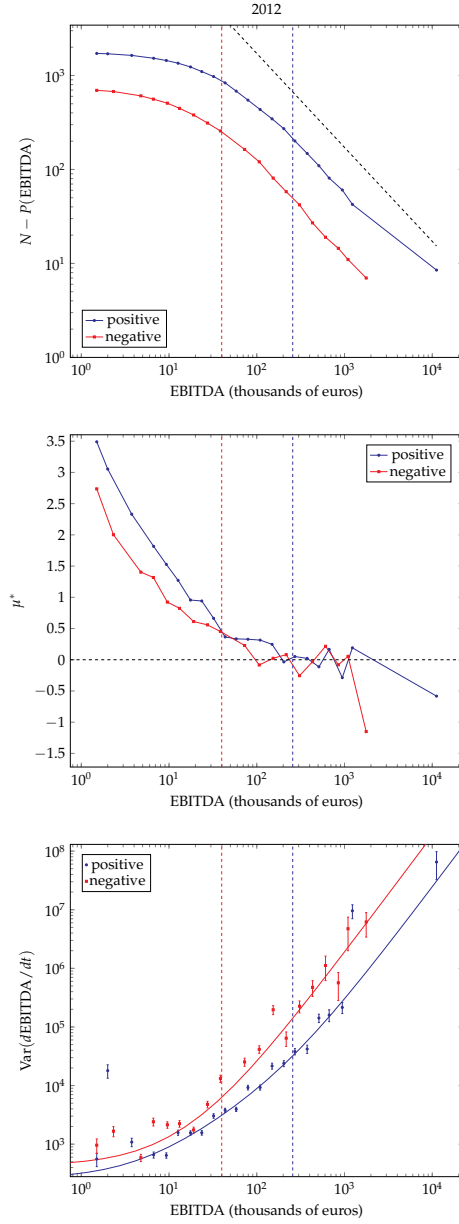

Figure 140: La Rioja

Rank plot, chemical potential and variance.

1768 Firms with positive EBITDA

$T_1 = 0.24 \pm 0.07$ ,  $T_{1/2} = 61.82 \pm 10.45$ , and  $T_0 = 257.44 \pm 146.59$

739 Firms with negative EBITDA

Negative EBITDA:

$T_1 = 1.84 \pm 0.58$ ,  $T_{1/2} = 73.28 \pm 33.31$ , and  $T_0 = 428.62 \pm 235.21$ .

# Madrid

## Tables of Temperatures

### Positive EBITDA

| Year | $T_1$           | $T_{1/2}$          | $T_0$                | $T_{1/2}/T_1$ | Num. Firms |
|------|-----------------|--------------------|----------------------|---------------|------------|
| 2003 | $0.51 \pm 0.11$ | $120.93 \pm 17.66$ | $404.70 \pm 173.98$  | 239.2         | 63272      |
| 2004 | $0.34 \pm 0.10$ | $131.80 \pm 24.24$ | $445.28 \pm 270.12$  | 383.4         | 63896      |
| 2005 | $0.49 \pm 0.09$ | $140.43 \pm 19.08$ | $564.32 \pm 246.27$  | 289.1         | 67493      |
| 2006 | $0.64 \pm 0.09$ | $137.37 \pm 15.85$ | $928.25 \pm 213.18$  | 213.4         | 69605      |
| 2007 | $0.91 \pm 0.18$ | $129.65 \pm 26.41$ | $1315.18 \pm 352.96$ | 142.7         | 73353      |
| 2008 | $1.24 \pm 0.27$ | $186.11 \pm 39.53$ | $635.65 \pm 363.65$  | 149.5         | 64799      |
| 2009 | $1.68 \pm 0.32$ | $134.26 \pm 33.75$ | $704.12 \pm 285.89$  | 79.7          | 71911      |
| 2010 | $1.29 \pm 0.31$ | $119.41 \pm 32.69$ | $744.29 \pm 358.01$  | 92.7          | 71282      |
| 2011 | $0.68 \pm 0.19$ | $177.59 \pm 27.52$ | $406.46 \pm 282.19$  | 262.5         | 65043      |
| 2012 | $0.71 \pm 0.22$ | $122.89 \pm 32.92$ | $996.40 \pm 354.17$  | 172.7         | 25097      |

### Negative EBITDA

| Year | $T_1$           | $T_{1/2}$           | $T_0$                | $T_{1/2}/T_1$ | Num. Firms |
|------|-----------------|---------------------|----------------------|---------------|------------|
| 2003 | $1.81 \pm 0.54$ | $233.03 \pm 41.20$  | $351.00 \pm 202.84$  | 128.9         | 24052      |
| 2004 | $1.74 \pm 0.56$ | $166.01 \pm 43.71$  | $1116.15 \pm 331.37$ | 95.5          | 23852      |
| 2005 | $1.22 \pm 0.54$ | $193.72 \pm 43.49$  | $929.96 \pm 345.28$  | 158.4         | 24932      |
| 2006 | $0.93 \pm 0.30$ | $249.91 \pm 31.24$  | $1058.23 \pm 298.15$ | 270.1         | 25407      |
| 2007 | $1.84 \pm 0.84$ | $366.22 \pm 56.65$  | $399.13 \pm 256.97$  | 199.1         | 24975      |
| 2008 | $5.29 \pm 1.97$ | $295.38 \pm 104.53$ | $1751.56 \pm 670.94$ | 55.8          | 23474      |
| 2009 | $4.08 \pm 1.24$ | $176.40 \pm 61.72$  | $997.68 \pm 326.66$  | 43.2          | 36135      |
| 2010 | $4.85 \pm 1.03$ | $206.94 \pm 54.08$  | $806.19 \pm 336.75$  | 42.7          | 38530      |
| 2011 | $4.00 \pm 0.89$ | $221.07 \pm 61.15$  | $1076.12 \pm 513.77$ | 55.3          | 36191      |
| 2012 | $2.07 \pm 0.74$ | $237.96 \pm 52.82$  | $234.55 \pm 272.39$  | 114.9         | 13874      |

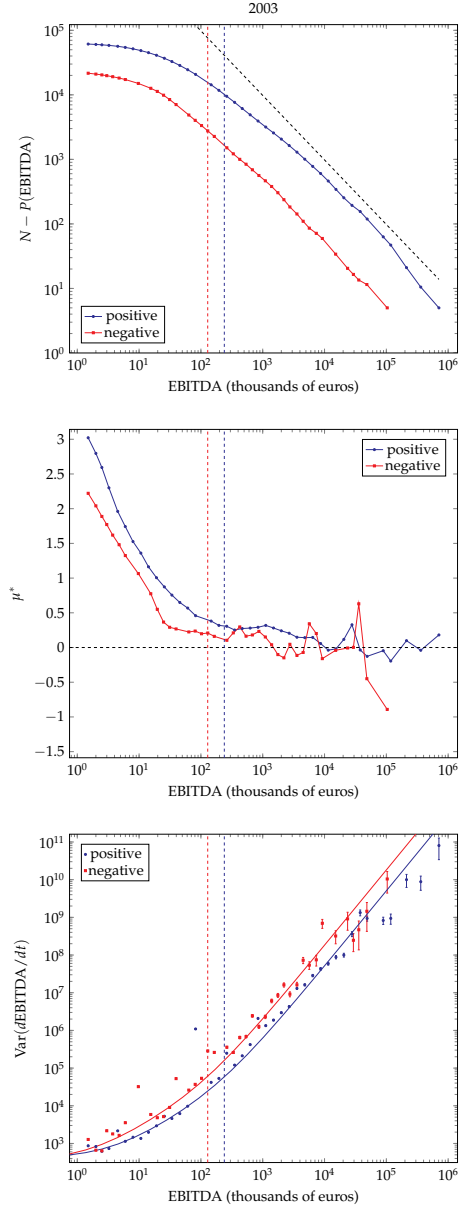

Figure 141: Madrid

Rank plot, chemical potential and variance.

63272 Firms with positive EBITDA

$T_1 = 0.51 \pm 0.11$ ,  $T_{1/2} = 120.93 \pm 17.66$ , and  $T_0 = 404.70 \pm 173.98$

24052 Firms with negative EBITDA

Negative EBITDA:

$T_1 = 1.81 \pm 0.54$ ,  $T_{1/2} = 233.03 \pm 41.20$ , and  $T_0 = 351.00 \pm 202.84$ .

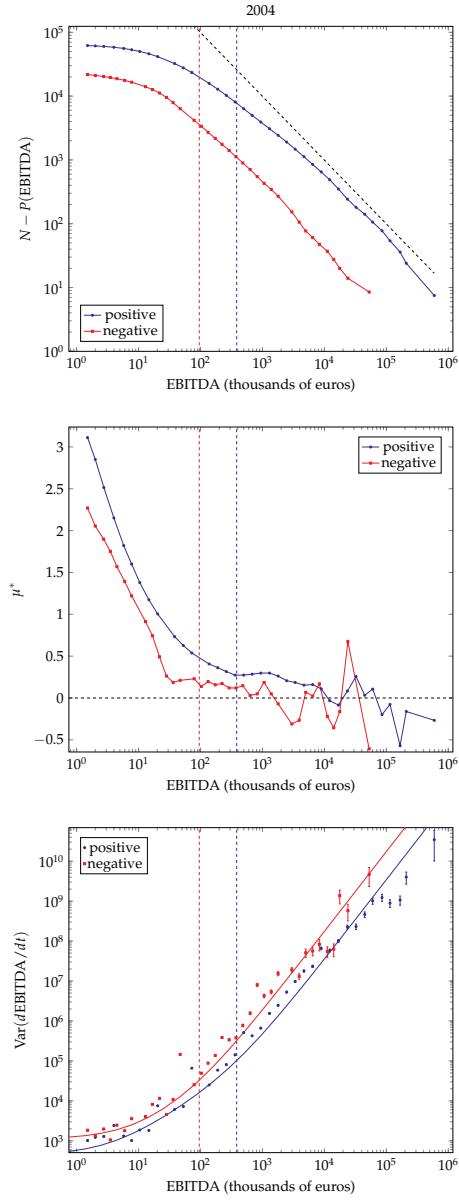

Figure 142: Madrid

Rank plot, chemical potential and variance.

63896 Firms with positive EBITDA

 $T_1 = 0.34 \pm 0.10$ ,  $T_{1/2} = 131.80 \pm 24.24$ , and  $T_0 = 445.28 \pm 270.12$ 

23852 Firms with negative EBITDA

Negative EBITDA:

 $T_1 = 1.74 \pm 0.56$ ,  $T_{1/2} = 166.01 \pm 43.71$ , and  $T_0 = 1116.15 \pm 331.37$ .

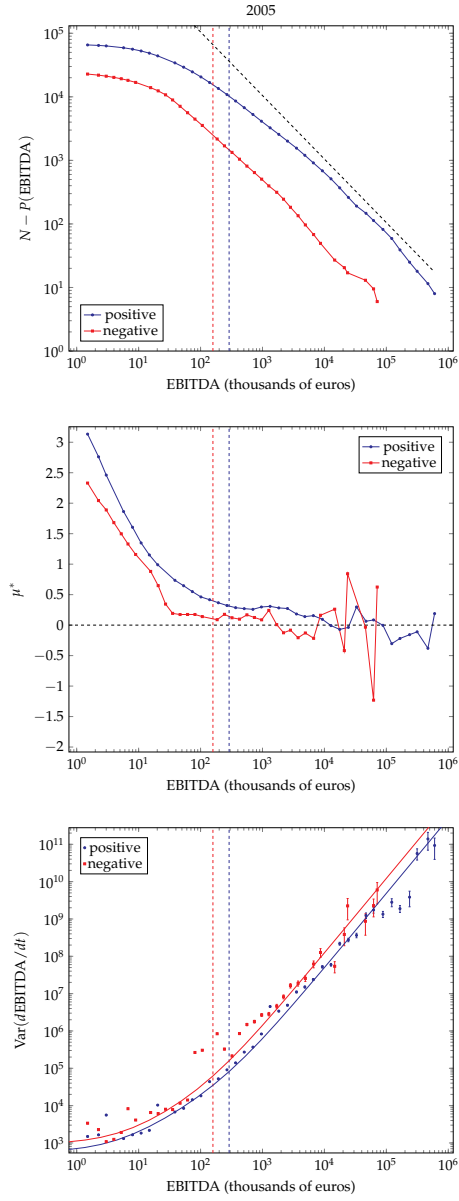

Figure 143: Madrid

Rank plot, chemical potential and variance.

67493 Firms with positive EBITDA

$T_1 = 0.49 \pm 0.09$ ,  $T_{1/2} = 140.43 \pm 19.08$ , and  $T_0 = 564.32 \pm 246.27$

24932 Firms with negative EBITDA

Negative EBITDA:

$T_1 = 1.22 \pm 0.54$ ,  $T_{1/2} = 193.72 \pm 43.49$ , and  $T_0 = 929.96 \pm 345.28$ .

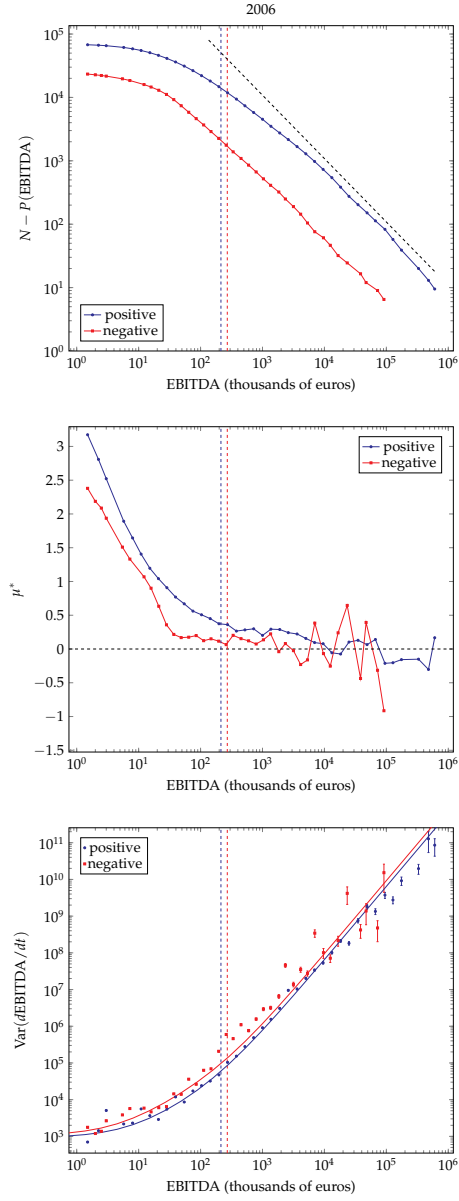

Figure 144: Madrid

Rank plot, chemical potential and variance.

69605 Firms with positive EBITDA

$T_1 = 0.64 \pm 0.09$ ,  $T_{1/2} = 137.37 \pm 15.85$ , and  $T_0 = 928.25 \pm 213.18$

25407 Firms with negative EBITDA

Negative EBITDA:

$T_1 = 0.93 \pm 0.30$ ,  $T_{1/2} = 249.91 \pm 31.24$ , and  $T_0 = 1058.23 \pm 298.15$ .

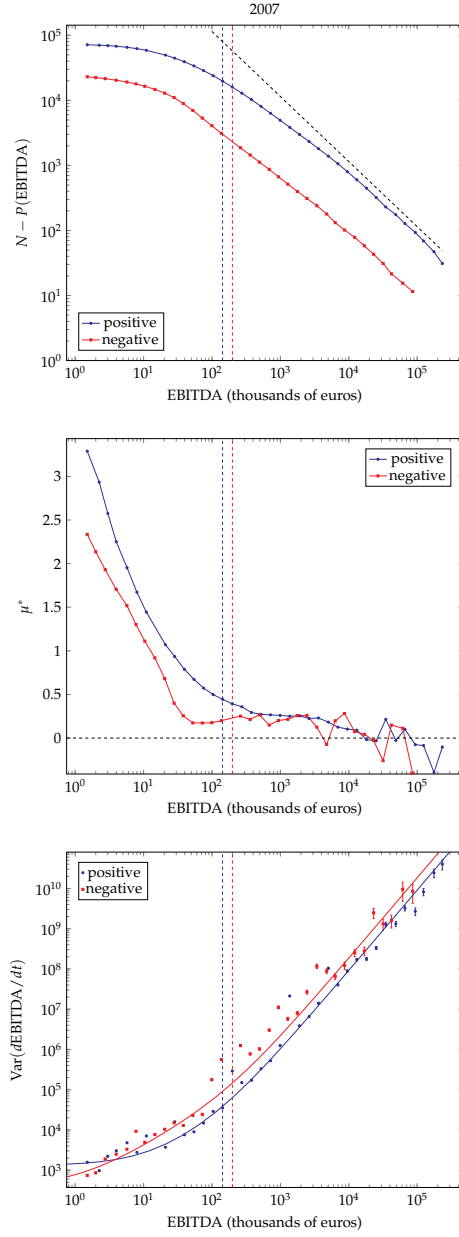

Figure 145: Madrid

Rank plot, chemical potential and variance.

73353 Firms with positive EBITDA

 $T_1 = 0.91 \pm 0.18$ ,  $T_{1/2} = 129.65 \pm 26.41$ , and  $T_0 = 1315.18 \pm 352.96$ 

24975 Firms with negative EBITDA

Negative EBITDA:

 $T_1 = 1.84 \pm 0.84$ ,  $T_{1/2} = 366.22 \pm 56.65$ , and  $T_0 = 399.13 \pm 256.97$ .

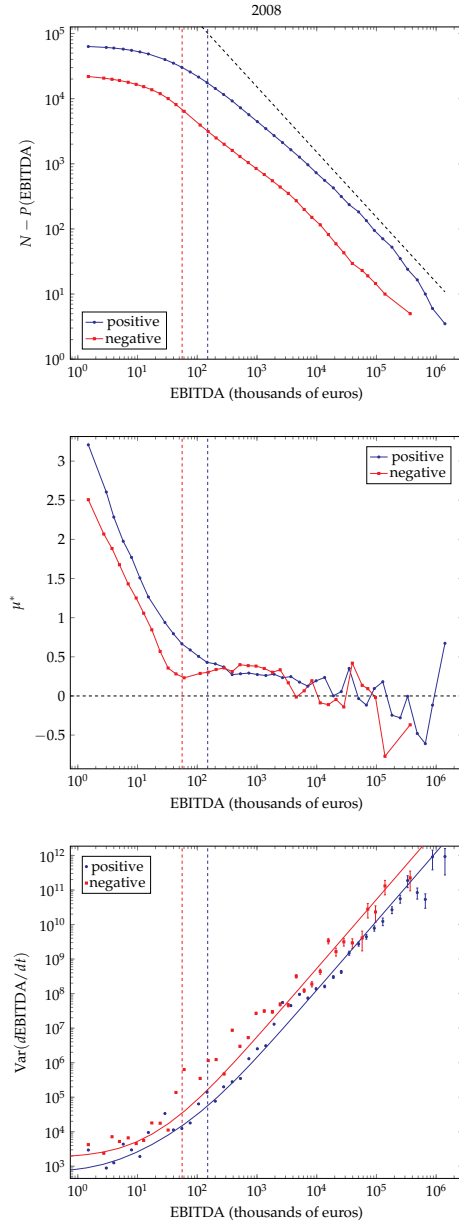

Figure 146: Madrid

Rank plot, chemical potential and variance.

64799 Firms with positive EBITDA

$T_1 = 1.24 \pm 0.27$ ,  $T_{1/2} = 186.11 \pm 39.53$ , and  $T_0 = 635.65 \pm 363.65$

23474 Firms with negative EBITDA

Negative EBITDA:

$T_1 = 5.29 \pm 1.97$ ,  $T_{1/2} = 295.38 \pm 104.53$ , and  $T_0 = 1751.56 \pm 670.94$ .

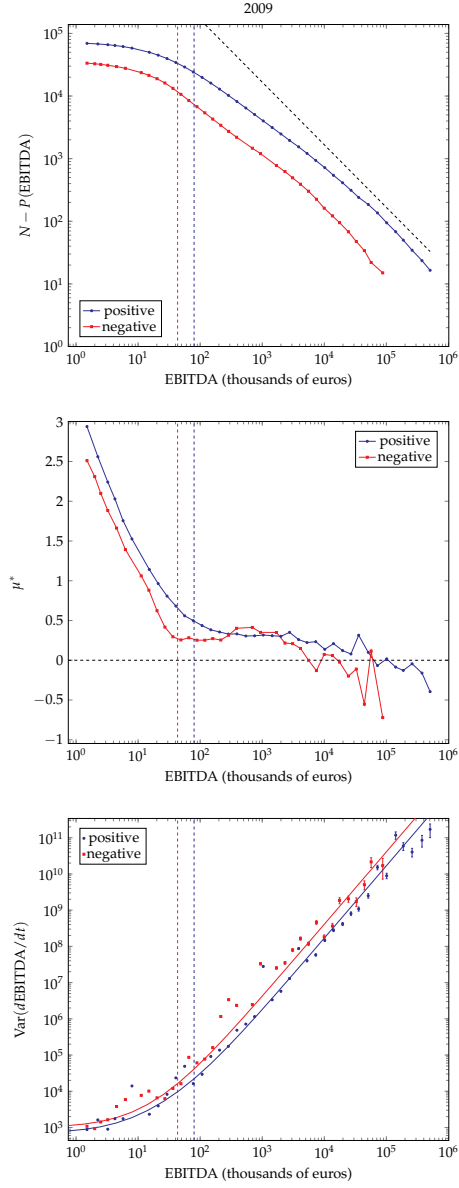

Figure 147: Madrid

Rank plot, chemical potential and variance.

71911 Firms with positive EBITDA

 $T_1 = 1.68 \pm 0.32$ ,  $T_{1/2} = 134.26 \pm 33.75$ , and  $T_0 = 704.12 \pm 285.89$ 

36135 Firms with negative EBITDA

Negative EBITDA:

 $T_1 = 4.08 \pm 1.24$ ,  $T_{1/2} = 176.40 \pm 61.72$ , and  $T_0 = 997.68 \pm 326.66$ .

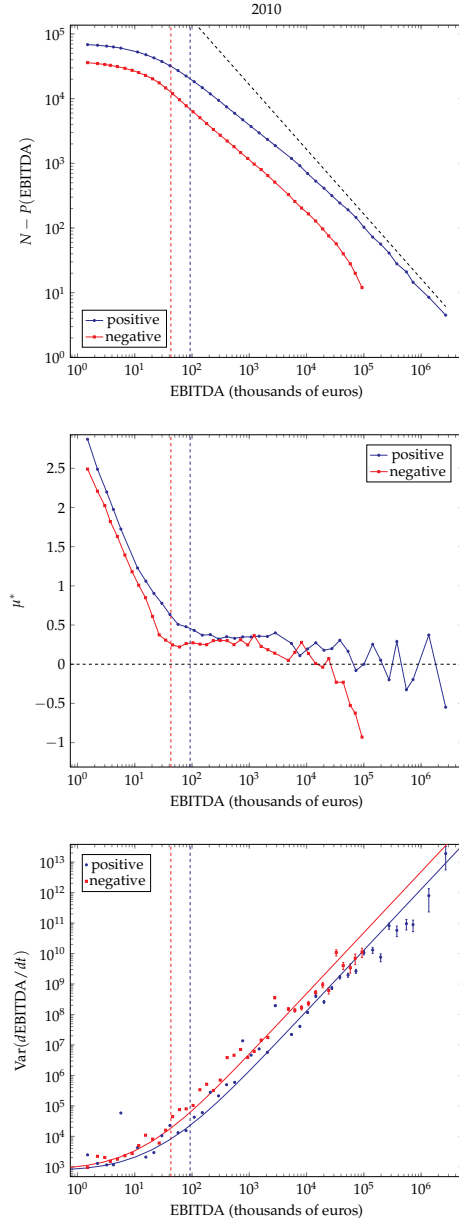

Figure 148: Madrid

Rank plot, chemical potential and variance.

71282 Firms with positive EBITDA

 $T_1 = 1.29 \pm 0.31$ ,  $T_{1/2} = 119.41 \pm 32.69$ , and  $T_0 = 744.29 \pm 358.01$ 

38530 Firms with negative EBITDA

Negative EBITDA:

 $T_1 = 4.85 \pm 1.03$ ,  $T_{1/2} = 206.94 \pm 54.08$ , and  $T_0 = 806.19 \pm 336.75$ .

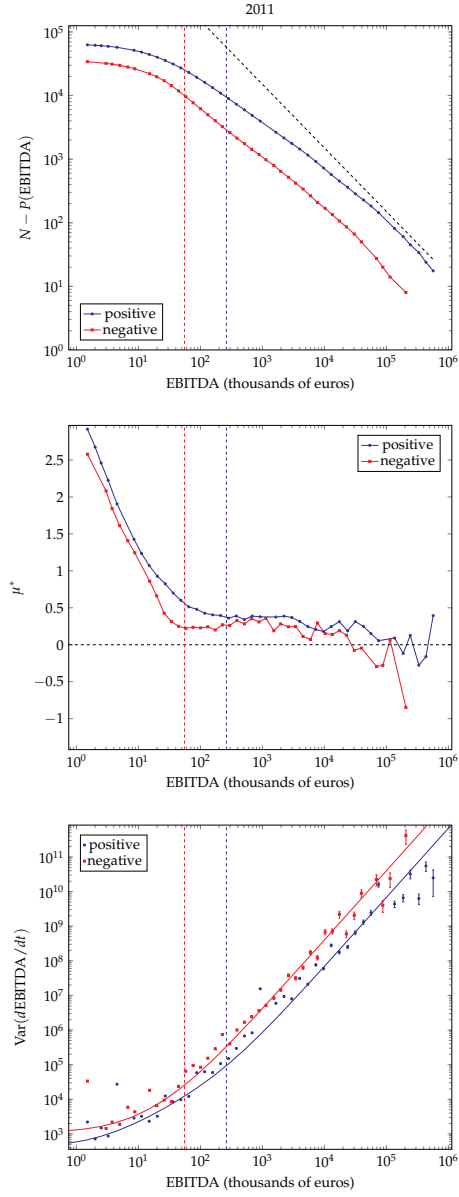

Figure 149: Madrid

Rank plot, chemical potential and variance.

65043 Firms with positive EBITDA

 $T_1 = 0.68 \pm 0.19$ ,  $T_{1/2} = 177.59 \pm 27.52$ , and  $T_0 = 406.46 \pm 282.19$ 

36191 Firms with negative EBITDA

Negative EBITDA:

 $T_1 = 4.00 \pm 0.89$ ,  $T_{1/2} = 221.07 \pm 61.15$ , and  $T_0 = 1076.12 \pm 513.77$ .

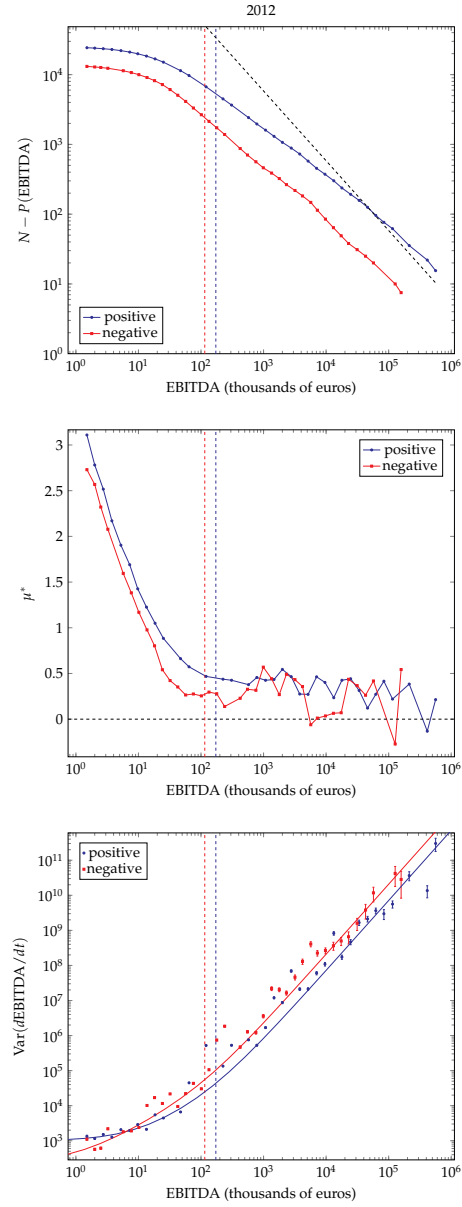

Figure 150: Madrid

Rank plot, chemical potential and variance.

25097 Firms with positive EBITDA

 $T_1 = 0.71 \pm 0.22$ ,  $T_{1/2} = 122.89 \pm 32.92$ , and  $T_0 = 996.40 \pm 354.17$ 

13874 Firms with negative EBITDA

Negative EBITDA:

 $T_1 = 2.07 \pm 0.74$ ,  $T_{1/2} = 237.96 \pm 52.82$ , and  $T_0 = 234.55 \pm 272.39$ .

# Murcia

## Tables of Temperatures

### Positive EBITDA

| Year | $T_1$           | $T_{1/2}$          | $T_0$               | $T_{1/2}/T_1$ | Num. Firms |
|------|-----------------|--------------------|---------------------|---------------|------------|
| 2003 | $0.35 \pm 0.07$ | $40.29 \pm 9.74$   | $224.87 \pm 125.94$ | 113.9         | 11716      |
| 2004 | $0.51 \pm 0.09$ | $26.27 \pm 8.32$   | $312.07 \pm 101.52$ | 51.9          | 12667      |
| 2005 | $0.52 \pm 0.08$ | $34.72 \pm 8.99$   | $455.55 \pm 122.14$ | 66.5          | 13434      |
| 2006 | $0.57 \pm 0.09$ | $47.30 \pm 10.18$  | $226.09 \pm 99.77$  | 82.6          | 14319      |
| 2007 | $0.57 \pm 0.08$ | $45.19 \pm 8.19$   | $284.60 \pm 83.12$  | 79.8          | 15930      |
| 2008 | $0.60 \pm 0.14$ | $73.09 \pm 18.67$  | $346.33 \pm 211.16$ | 121.8         | 13813      |
| 2009 | $0.69 \pm 0.21$ | $76.10 \pm 23.86$  | $416.38 \pm 186.66$ | 109.7         | 12492      |
| 2010 | $0.58 \pm 0.13$ | $44.76 \pm 12.87$  | $414.71 \pm 141.79$ | 76.7          | 12949      |
| 2011 | $0.49 \pm 0.16$ | $141.34 \pm 18.34$ | $66.66 \pm 98.75$   | 287.8         | 11421      |
| 2012 | $0.22 \pm 0.07$ | $64.88 \pm 8.27$   | $244.37 \pm 75.51$  | 292.5         | 6442       |

### Negative EBITDA

| Year | $T_1$           | $T_{1/2}$          | $T_0$                | $T_{1/2}/T_1$ | Num. Firms |
|------|-----------------|--------------------|----------------------|---------------|------------|
| 2003 | $2.30 \pm 0.86$ | $127.13 \pm 62.04$ | $768.06 \pm 432.30$  | 55.3          | 1854       |
| 2004 | $0.81 \pm 0.58$ | $282.02 \pm 53.79$ | $276.06 \pm 283.43$  | 347.5         | 2022       |
| 2005 | $2.82 \pm 1.01$ | $297.05 \pm 75.47$ | $696.04 \pm 586.16$  | 105.5         | 2190       |
| 2006 | $1.32 \pm 0.53$ | $375.51 \pm 54.46$ | $274.78 \pm 384.66$  | 283.9         | 2403       |
| 2007 | $3.33 \pm 0.99$ | $213.97 \pm 63.47$ | $651.14 \pm 364.35$  | 64.3          | 2852       |
| 2008 | $1.76 \pm 0.73$ | $263.33 \pm 55.91$ | $842.89 \pm 367.39$  | 149.5         | 2645       |
| 2009 | $3.29 \pm 1.06$ | $246.46 \pm 90.02$ | $2011.52 \pm 878.32$ | 74.8          | 3402       |
| 2010 | $2.88 \pm 0.67$ | $147.50 \pm 43.37$ | $632.58 \pm 335.98$  | 51.2          | 4418       |
| 2011 | $2.01 \pm 0.79$ | $308.07 \pm 52.42$ | $242.24 \pm 324.10$  | 153.1         | 3982       |
| 2012 | $3.07 \pm 0.68$ | $19.01 \pm 40.45$  | $1656.00 \pm 377.90$ | 6.2           | 2503       |

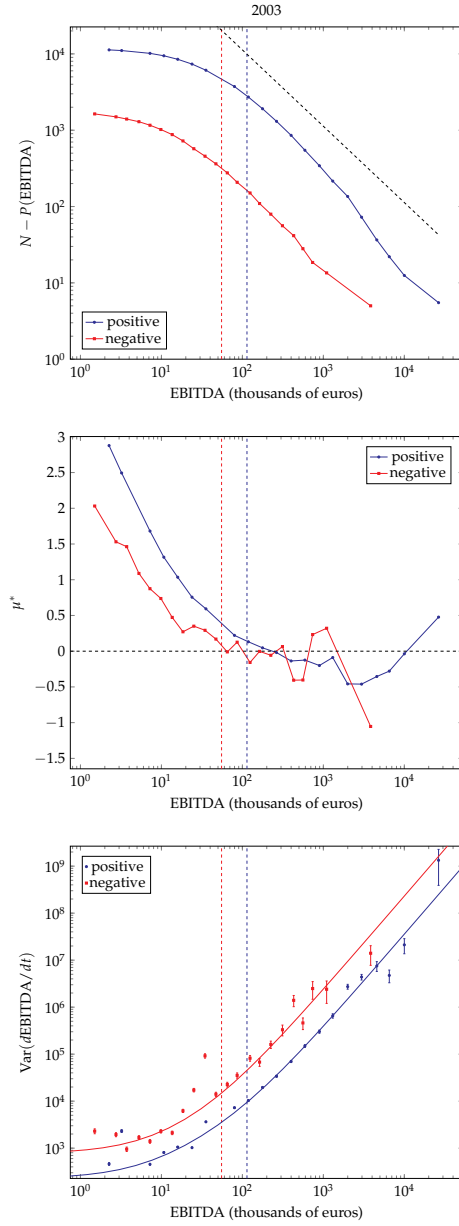

Figure 151: Murcia

Rank plot, chemical potential and variance.

11716 Firms with positive EBITDA

$T_1 = 0.35 \pm 0.07$ ,  $T_{1/2} = 40.29 \pm 9.74$ , and  $T_0 = 224.87 \pm 125.94$

1854 Firms with negative EBITDA

Negative EBITDA:

$T_1 = 2.30 \pm 0.86$ ,  $T_{1/2} = 127.13 \pm 62.04$ , and  $T_0 = 768.06 \pm 432.30$ .

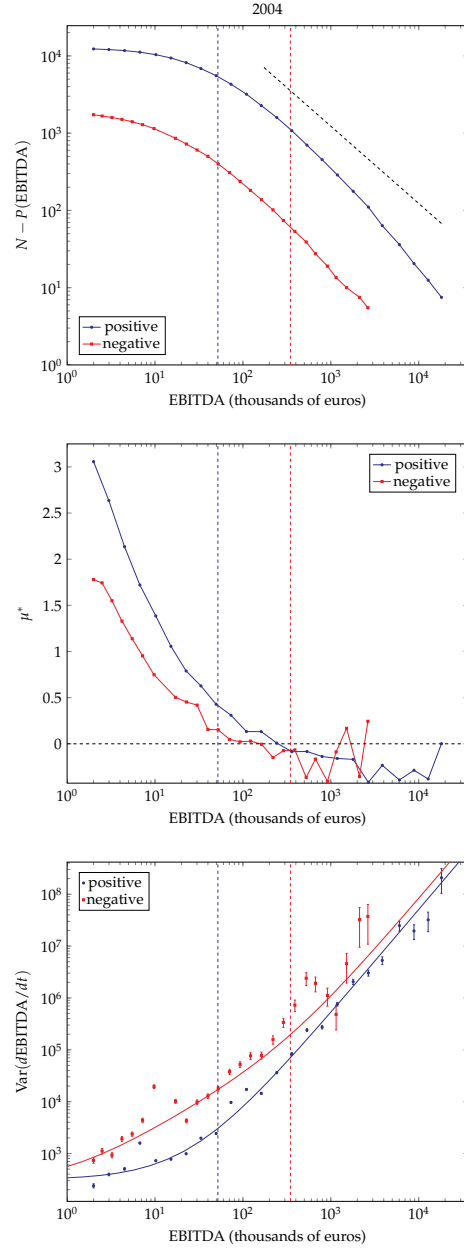

Figure 152: Murcia

Rank plot, chemical potential and variance.

12667 Firms with positive EBITDA

$T_1 = 0.51 \pm 0.09$ ,  $T_{1/2} = 26.27 \pm 8.32$ , and  $T_0 = 312.07 \pm 101.52$

2022 Firms with negative EBITDA

Negative EBITDA:

$T_1 = 0.81 \pm 0.58$ ,  $T_{1/2} = 282.02 \pm 53.79$ , and  $T_0 = 276.06 \pm 283.43$ .

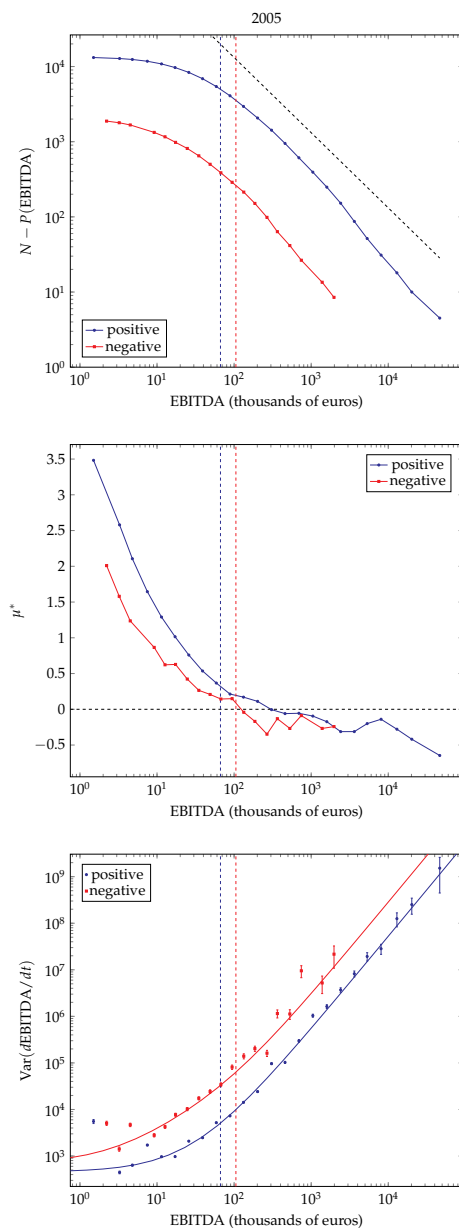

Figure 153: Murcia

Rank plot, chemical potential and variance.

13434 Firms with positive EBITDA

$T_1 = 0.52 \pm 0.08$ ,  $T_{1/2} = 34.72 \pm 8.99$ , and  $T_0 = 455.55 \pm 122.14$

2190 Firms with negative EBITDA

Negative EBITDA:

$T_1 = 2.82 \pm 1.01$ ,  $T_{1/2} = 297.05 \pm 75.47$ , and  $T_0 = 696.04 \pm 586.16$ .

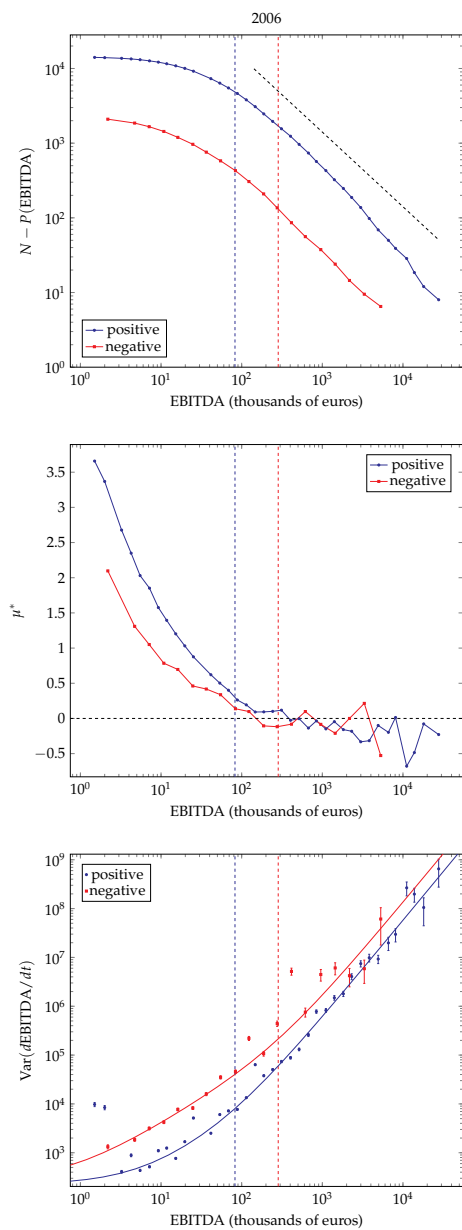

Figure 154: Murcia

Rank plot, chemical potential and variance.

14319 Firms with positive EBITDA

 $T_1 = 0.57 \pm 0.09$ ,  $T_{1/2} = 47.30 \pm 10.18$ , and  $T_0 = 226.09 \pm 99.77$ 

2403 Firms with negative EBITDA

Negative EBITDA:

 $T_1 = 1.32 \pm 0.53$ ,  $T_{1/2} = 375.51 \pm 54.46$ , and  $T_0 = 274.78 \pm 384.66$ .

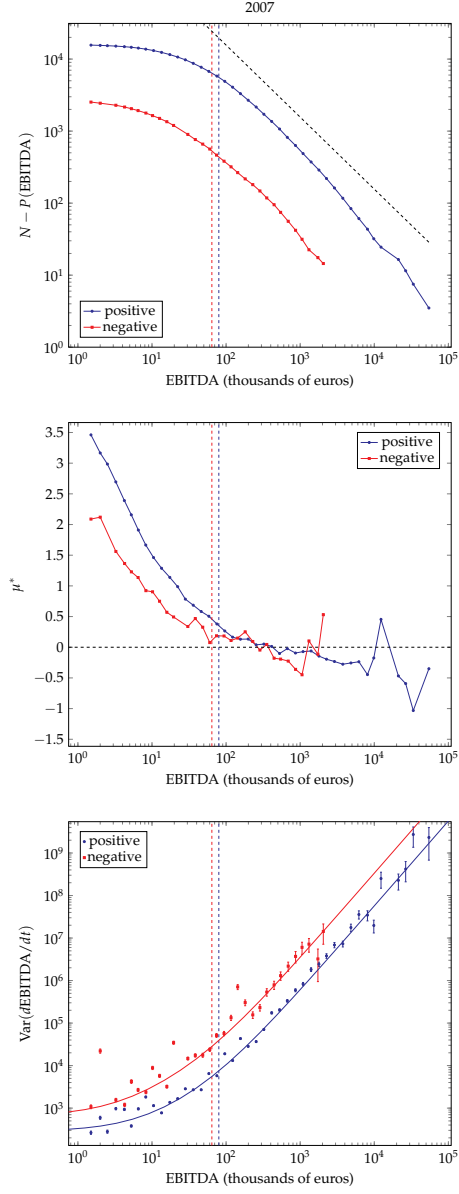

Figure 155: Murcia

Rank plot, chemical potential and variance.

15930 Firms with positive EBITDA

$T_1 = 0.57 \pm 0.08$ ,  $T_{1/2} = 45.19 \pm 8.19$ , and  $T_0 = 284.60 \pm 83.12$

2852 Firms with negative EBITDA

Negative EBITDA:

$T_1 = 3.33 \pm 0.99$ ,  $T_{1/2} = 213.97 \pm 63.47$ , and  $T_0 = 651.14 \pm 364.35$ .

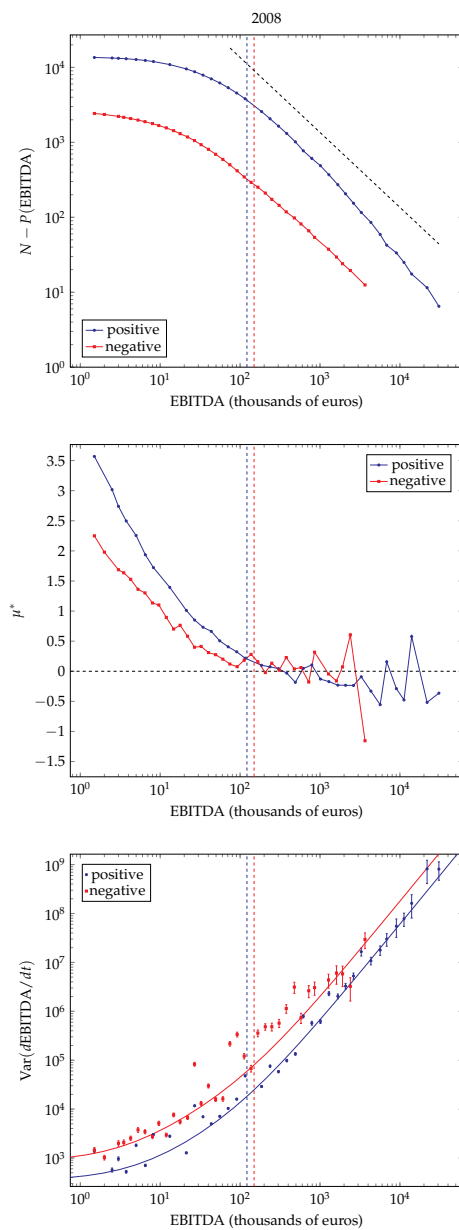

Figure 156: Murcia

Rank plot, chemical potential and variance.

13813 Firms with positive EBITDA

 $T_1 = 0.60 \pm 0.14$ ,  $T_{1/2} = 73.09 \pm 18.67$ , and  $T_0 = 346.33 \pm 211.16$ 

2645 Firms with negative EBITDA

Negative EBITDA:

 $T_1 = 1.76 \pm 0.73$ ,  $T_{1/2} = 263.33 \pm 55.91$ , and  $T_0 = 842.89 \pm 367.39$ .

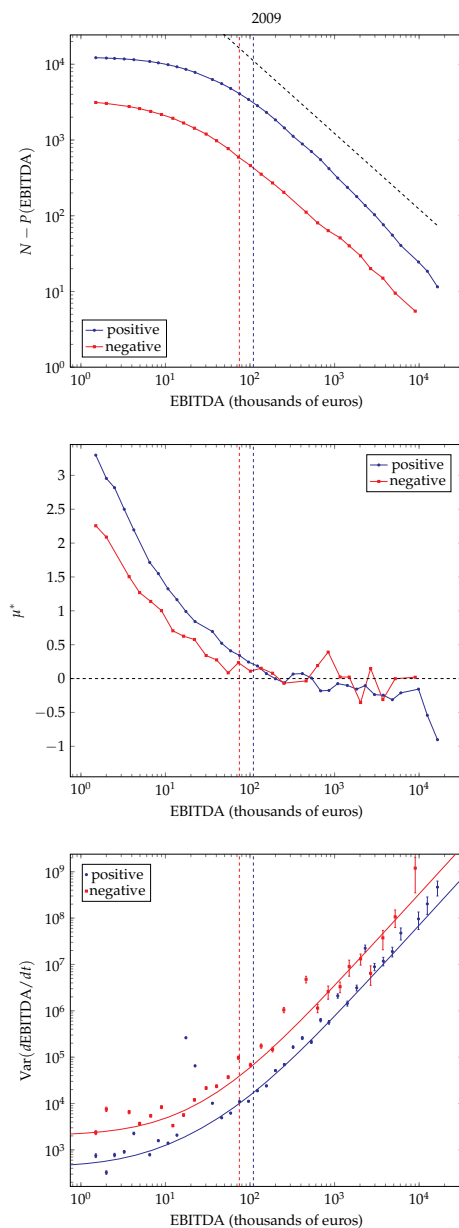

Figure 157: Murcia

Rank plot, chemical potential and variance.

12492 Firms with positive EBITDA

$T_1 = 0.69 \pm 0.21$ ,  $T_{1/2} = 76.10 \pm 23.86$ , and  $T_0 = 416.38 \pm 186.66$

3402 Firms with negative EBITDA

Negative EBITDA:

$T_1 = 3.29 \pm 1.06$ ,  $T_{1/2} = 246.46 \pm 90.02$ , and  $T_0 = 2011.52 \pm 878.32$ .

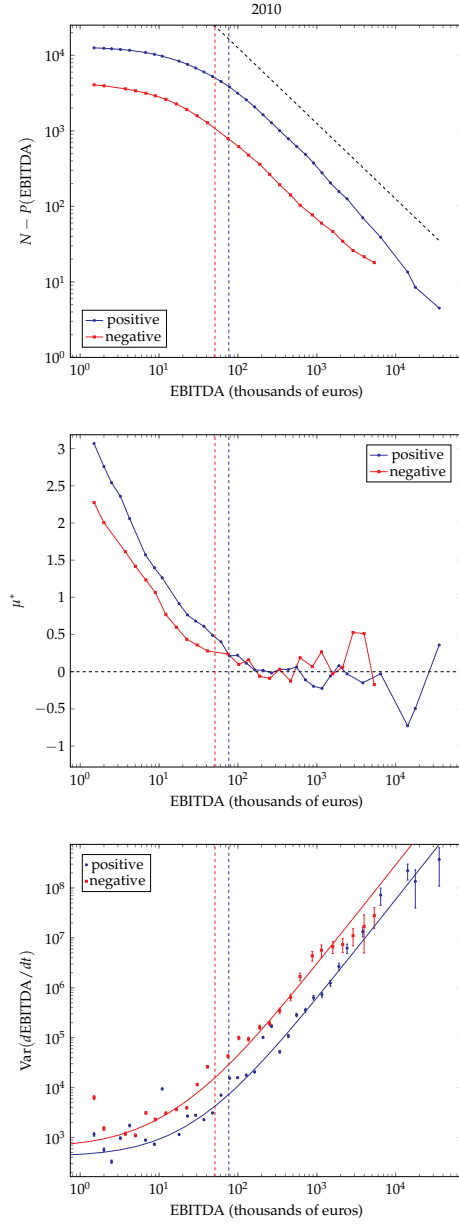

Figure 158: Murcia

Rank plot, chemical potential and variance.

12949 Firms with positive EBITDA

$T_1 = 0.58 \pm 0.13$ ,  $T_{1/2} = 44.76 \pm 12.87$ , and  $T_0 = 414.71 \pm 141.79$

4418 Firms with negative EBITDA

Negative EBITDA:

$T_1 = 2.88 \pm 0.67$ ,  $T_{1/2} = 147.50 \pm 43.37$ , and  $T_0 = 632.58 \pm 335.98$ .

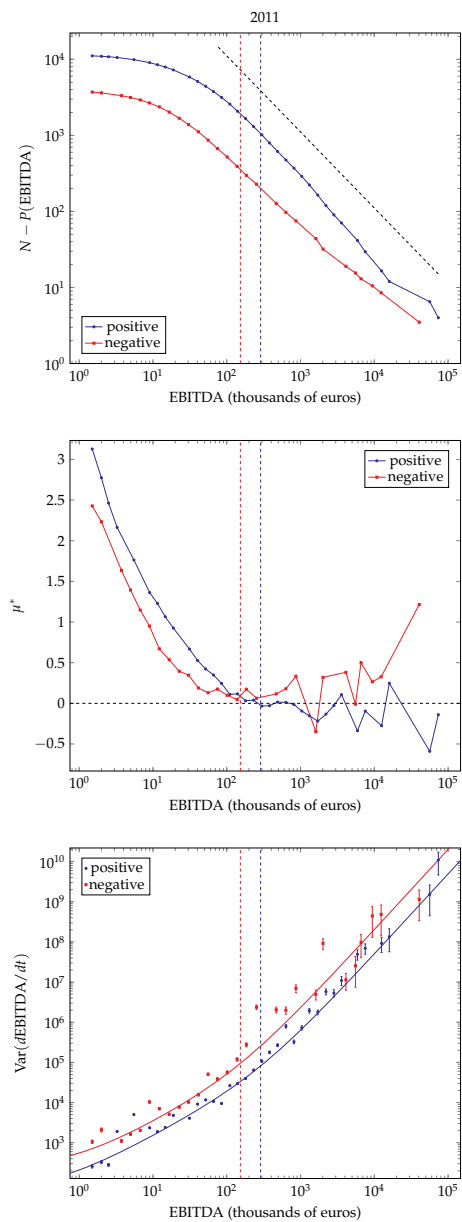

Figure 159: Murcia

Rank plot, chemical potential and variance.

11421 Firms with positive EBITDA

$T_1 = 0.49 \pm 0.16$ ,  $T_{1/2} = 141.34 \pm 18.34$ , and  $T_0 = 66.66 \pm 98.75$

3982 Firms with negative EBITDA

Negative EBITDA:

$T_1 = 2.01 \pm 0.79$ ,  $T_{1/2} = 308.07 \pm 52.42$ , and  $T_0 = 242.24 \pm 324.10$ .

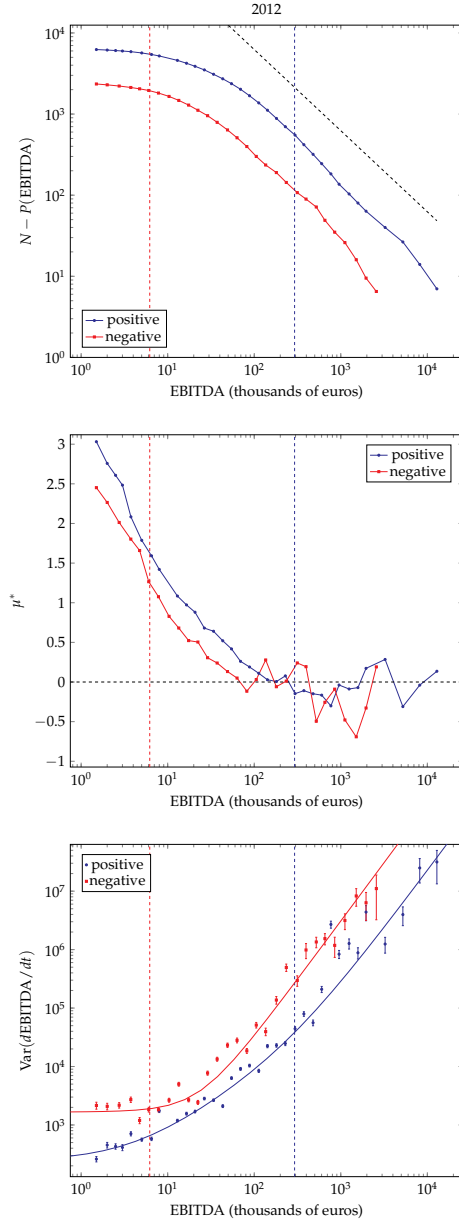

Figure 160: Murcia

Rank plot, chemical potential and variance.

6442 Firms with positive EBITDA

 $T_1 = 0.22 \pm 0.07$ ,  $T_{1/2} = 64.88 \pm 8.27$ , and  $T_0 = 244.37 \pm 75.51$ 

2503 Firms with negative EBITDA

Negative EBITDA:

 $T_1 = 3.07 \pm 0.68$ ,  $T_{1/2} = 19.01 \pm 40.45$ , and  $T_0 = 1656.00 \pm 377.90$ .

# Navarre

## Tables of Temperatures

### Positive EBITDA

| Year | $T_1$           | $T_{1/2}$          | $T_0$                | $T_{1/2}/T_1$ | Num. Firms |
|------|-----------------|--------------------|----------------------|---------------|------------|
| 2003 | $0.29 \pm 0.05$ | $43.50 \pm 7.31$   | $300.36 \pm 87.47$   | 150.5         | 5857       |
| 2004 | $0.37 \pm 0.11$ | $62.78 \pm 17.38$  | $317.42 \pm 178.36$  | 169.6         | 6076       |
| 2005 | $0.33 \pm 0.07$ | $38.98 \pm 9.42$   | $234.72 \pm 127.24$  | 119.2         | 6436       |
| 2006 | $0.38 \pm 0.08$ | $49.23 \pm 17.05$  | $369.14 \pm 291.73$  | 131.3         | 6821       |
| 2007 | $0.33 \pm 0.08$ | $54.92 \pm 11.74$  | $276.61 \pm 172.09$  | 165.8         | 6987       |
| 2008 | $0.35 \pm 0.13$ | $99.01 \pm 25.46$  | $159.62 \pm 263.98$  | 284.5         | 6390       |
| 2009 | $0.39 \pm 0.13$ | $114.84 \pm 23.92$ | $253.30 \pm 323.13$  | 292.7         | 6594       |
| 2010 | $0.79 \pm 0.17$ | $28.08 \pm 20.16$  | $1107.93 \pm 337.68$ | 35.5          | 6690       |
| 2011 | $0.80 \pm 0.22$ | $94.25 \pm 30.70$  | $980.95 \pm 474.29$  | 118.2         | 6077       |
| 2012 | $0.21 \pm 0.07$ | $67.64 \pm 14.58$  | $338.38 \pm 212.76$  | 315.5         | 4120       |

### Negative EBITDA

| Year | $T_1$           | $T_{1/2}$          | $T_0$                | $T_{1/2}/T_1$ | Num. Firms |
|------|-----------------|--------------------|----------------------|---------------|------------|
| 2003 | $1.80 \pm 0.92$ | $75.99 \pm 66.87$  | $311.50 \pm 584.37$  | 42.3          | 1020       |
| 2004 | $0.53 \pm 0.41$ | $130.31 \pm 29.14$ | $63.61 \pm 88.51$    | 245.9         | 1039       |
| 2005 | $1.26 \pm 0.79$ | $147.81 \pm 59.46$ | $176.30 \pm 210.04$  | 117.0         | 1137       |
| 2006 | $1.31 \pm 0.72$ | $149.81 \pm 78.89$ | $211.85 \pm 650.33$  | 114.7         | 1207       |
| 2007 | $1.12 \pm 0.66$ | $198.69 \pm 61.86$ | $43.45 \pm 330.91$   | 176.9         | 1163       |
| 2008 | $1.42 \pm 0.75$ | $160.07 \pm 54.31$ | $928.51 \pm 401.14$  | 113.0         | 1137       |
| 2009 | $3.61 \pm 1.22$ | $202.52 \pm 80.91$ | $721.28 \pm 525.93$  | 56.2          | 1624       |
| 2010 | $1.24 \pm 1.00$ | $245.04 \pm 68.56$ | $1039.04 \pm 496.24$ | 197.6         | 2266       |
| 2011 | $0.38 \pm 0.34$ | $331.47 \pm 56.99$ | $268.88 \pm 447.96$  | 861.8         | 2018       |
| 2012 | $2.31 \pm 1.07$ | $27.99 \pm 49.04$  | $854.52 \pm 320.07$  | 12.1          | 1710       |

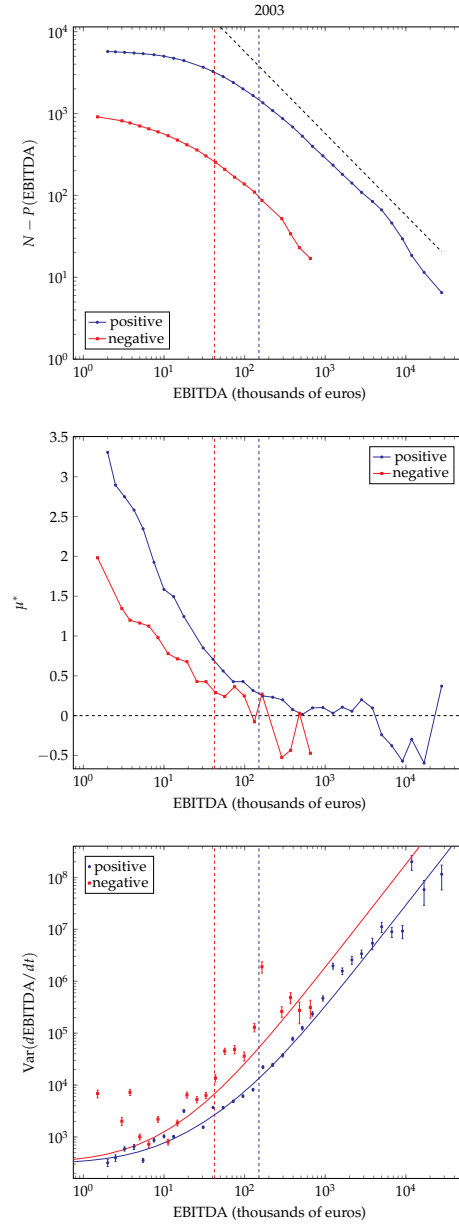

Figure 161: Navarre

Rank plot, chemical potential and variance.

5857 Firms with positive EBITDA

$T_1 = 0.29 \pm 0.05$ ,  $T_{1/2} = 43.50 \pm 7.31$ , and  $T_0 = 300.36 \pm 87.47$

1020 Firms with negative EBITDA

Negative EBITDA:

$T_1 = 1.80 \pm 0.92$ ,  $T_{1/2} = 75.99 \pm 66.87$ , and  $T_0 = 311.50 \pm 584.37$ .

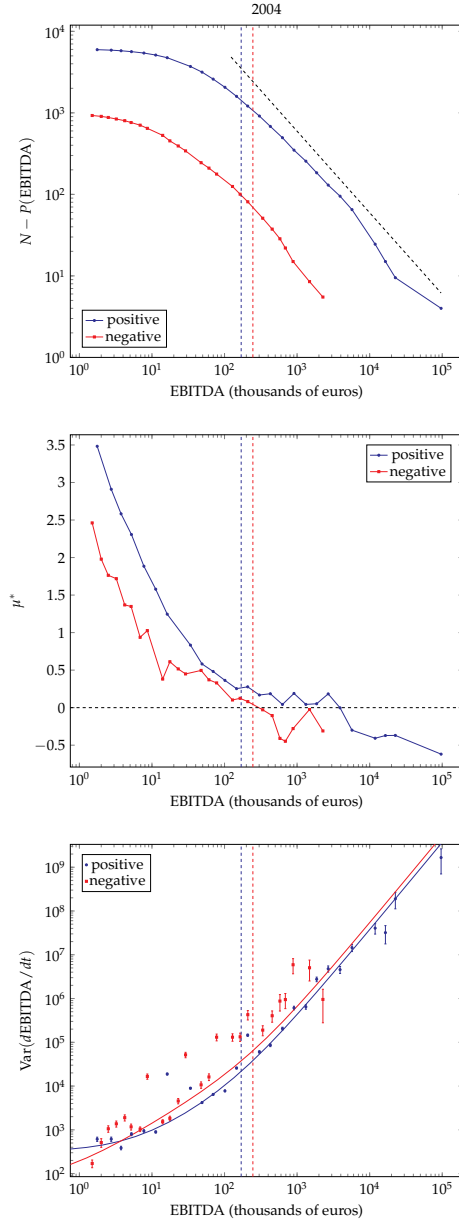

Figure 162: Navarre

Rank plot, chemical potential and variance.

6076 Firms with positive EBITDA

$T_1 = 0.37 \pm 0.11$ ,  $T_{1/2} = 62.78 \pm 17.38$ , and  $T_0 = 317.42 \pm 178.36$

1039 Firms with negative EBITDA

Negative EBITDA:

$T_1 = 0.53 \pm 0.41$ ,  $T_{1/2} = 130.31 \pm 29.14$ , and  $T_0 = 63.61 \pm 88.51$ .

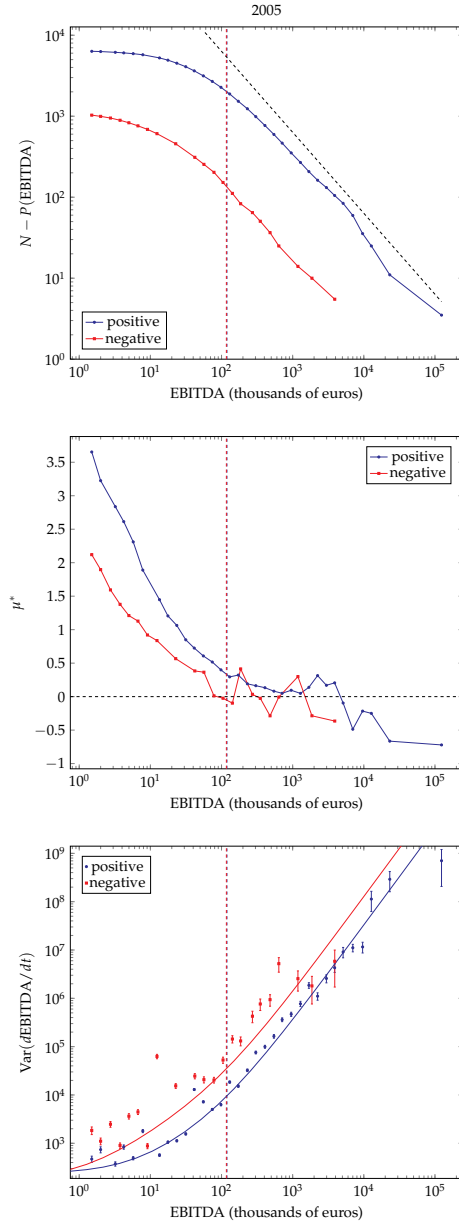

Figure 163: Navarre

Rank plot, chemical potential and variance.

6436 Firms with positive EBITDA

$T_1 = 0.33 \pm 0.07$ ,  $T_{1/2} = 38.98 \pm 9.42$ , and  $T_0 = 234.72 \pm 127.24$

1137 Firms with negative EBITDA

Negative EBITDA:

$T_1 = 1.26 \pm 0.79$ ,  $T_{1/2} = 147.81 \pm 59.46$ , and  $T_0 = 176.30 \pm 210.04$ .

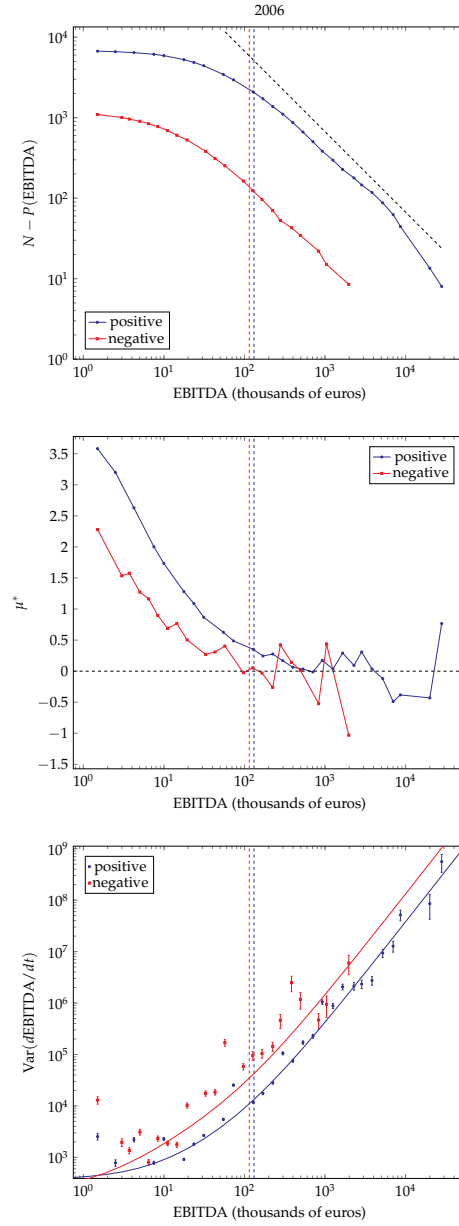

Figure 164: Navarre

Rank plot, chemical potential and variance.

6821 Firms with positive EBITDA

$T_1 = 0.38 \pm 0.08$ ,  $T_{1/2} = 49.23 \pm 17.05$ , and  $T_0 = 369.14 \pm 291.73$

1207 Firms with negative EBITDA

Negative EBITDA:

$T_1 = 1.31 \pm 0.72$ ,  $T_{1/2} = 149.81 \pm 78.89$ , and  $T_0 = 211.85 \pm 650.33$ .

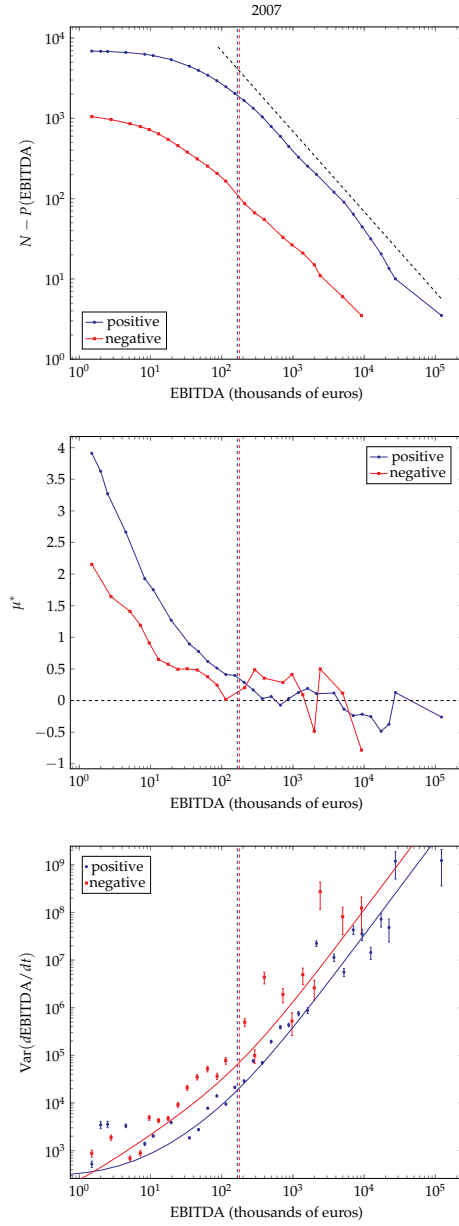

Figure 165: Navarre

Rank plot, chemical potential and variance.

6987 Firms with positive EBITDA

$T_1 = 0.33 \pm 0.08$ ,  $T_{1/2} = 54.92 \pm 11.74$ , and  $T_0 = 276.61 \pm 172.09$

1163 Firms with negative EBITDA

Negative EBITDA:

$T_1 = 1.12 \pm 0.66$ ,  $T_{1/2} = 198.69 \pm 61.86$ , and  $T_0 = 43.45 \pm 330.91$ .

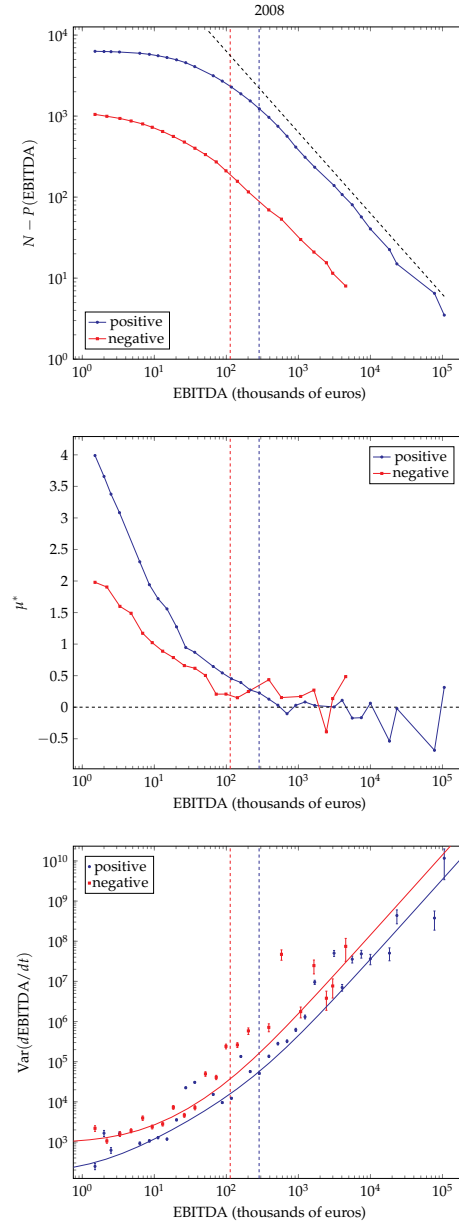

Figure 166: Navarre

Rank plot, chemical potential and variance.

6390 Firms with positive EBITDA

$T_1 = 0.35 \pm 0.13$ ,  $T_{1/2} = 99.01 \pm 25.46$ , and  $T_0 = 159.62 \pm 263.98$

1137 Firms with negative EBITDA

Negative EBITDA:

$T_1 = 1.42 \pm 0.75$ ,  $T_{1/2} = 160.07 \pm 54.31$ , and  $T_0 = 928.51 \pm 401.14$ .

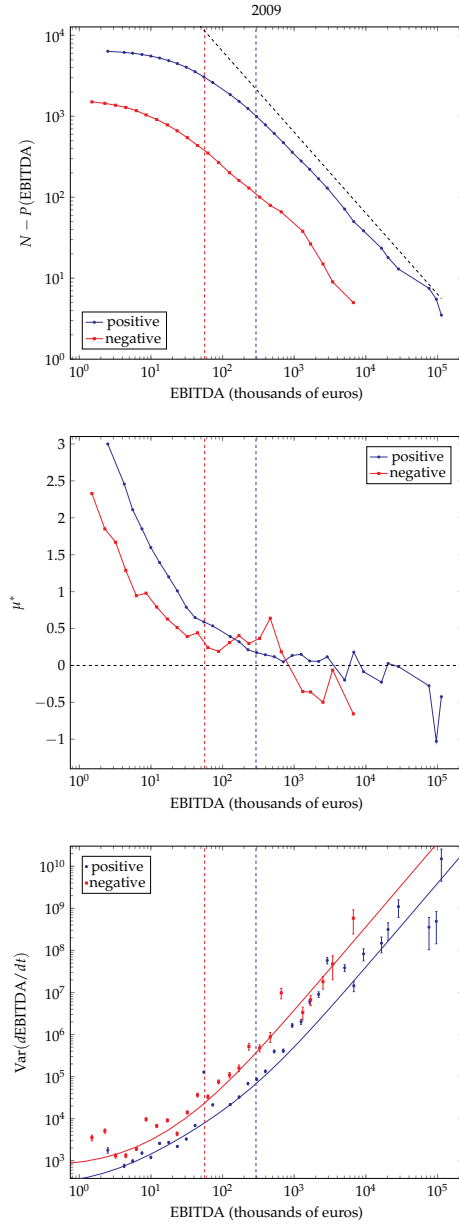

Figure 167: Navarre

Rank plot, chemical potential and variance.

6594 Firms with positive EBITDA

$T_1 = 0.39 \pm 0.13$ ,  $T_{1/2} = 114.84 \pm 23.92$ , and  $T_0 = 253.30 \pm 323.13$

1624 Firms with negative EBITDA

Negative EBITDA:

$T_1 = 3.61 \pm 1.22$ ,  $T_{1/2} = 202.52 \pm 80.91$ , and  $T_0 = 721.28 \pm 525.93$ .

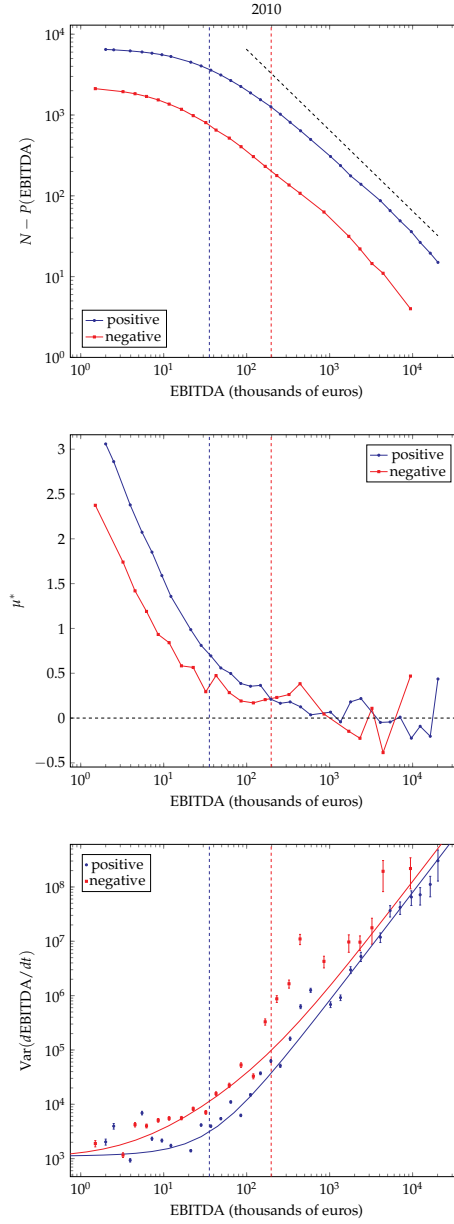

Figure 168: Navarre

Rank plot, chemical potential and variance.

6690 Firms with positive EBITDA

$T_1 = 0.79 \pm 0.17$ ,  $T_{1/2} = 28.08 \pm 20.16$ , and  $T_0 = 1107.93 \pm 337.68$

2266 Firms with negative EBITDA

Negative EBITDA:

$T_1 = 1.24 \pm 1.00$ ,  $T_{1/2} = 245.04 \pm 68.56$ , and  $T_0 = 1039.04 \pm 496.24$ .

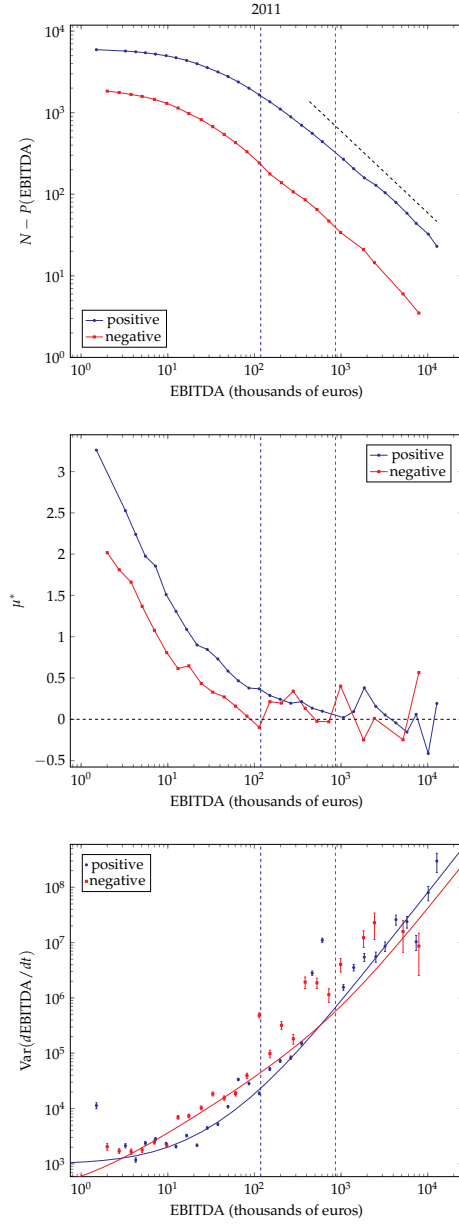

Figure 169: Navarre

Rank plot, chemical potential and variance.

6077 Firms with positive EBITDA

$T_1 = 0.80 \pm 0.22$ ,  $T_{1/2} = 94.25 \pm 30.70$ , and  $T_0 = 980.95 \pm 474.29$

2018 Firms with negative EBITDA

Negative EBITDA:

$T_1 = 0.38 \pm 0.34$ ,  $T_{1/2} = 331.47 \pm 56.99$ , and  $T_0 = 268.88 \pm 447.96$ .

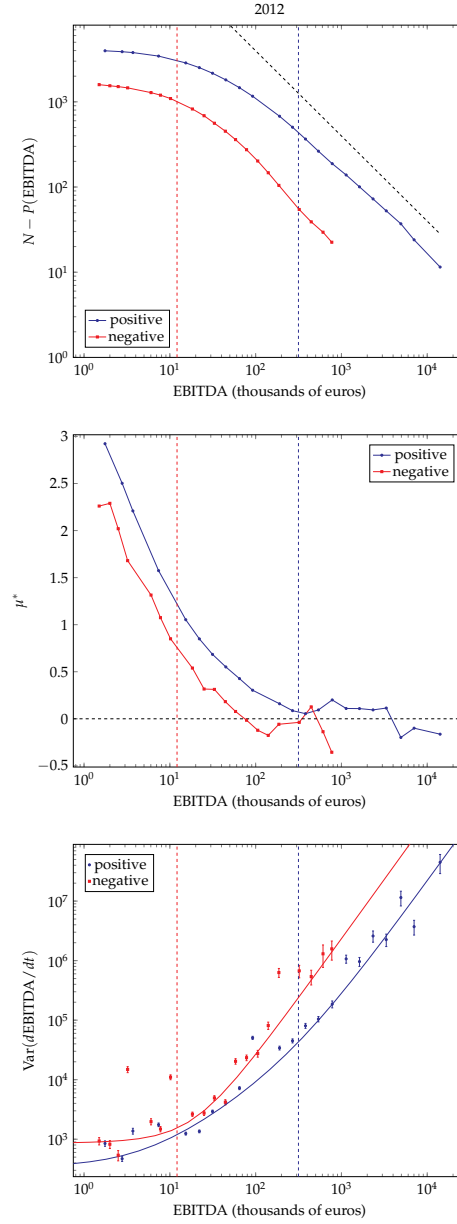

Figure 170: Navarre

Rank plot, chemical potential and variance.

4120 Firms with positive EBITDA

$T_1 = 0.21 \pm 0.07$ ,  $T_{1/2} = 67.64 \pm 14.58$ , and  $T_0 = 338.38 \pm 212.76$

1710 Firms with negative EBITDA

Negative EBITDA:

$T_1 = 2.31 \pm 1.07$ ,  $T_{1/2} = 27.99 \pm 49.04$ , and  $T_0 = 854.52 \pm 320.07$ .

# Valencian community

## Tables of Temperatures

### Positive EBITDA

| Year | $T_1$           | $T_{1/2}$          | $T_0$                | $T_{1/2}/T_1$ | Num. Firms |
|------|-----------------|--------------------|----------------------|---------------|------------|
| 2003 | $0.47 \pm 0.08$ | $36.88 \pm 9.27$   | $396.90 \pm 104.54$  | 78.3          | 50870      |
| 2004 | $0.53 \pm 0.08$ | $34.79 \pm 7.77$   | $339.74 \pm 84.24$   | 66.0          | 52966      |
| 2005 | $0.52 \pm 0.07$ | $46.94 \pm 7.09$   | $353.35 \pm 64.24$   | 91.0          | 54255      |
| 2006 | $0.68 \pm 0.09$ | $42.56 \pm 9.73$   | $462.03 \pm 110.66$  | 62.2          | 55714      |
| 2007 | $0.70 \pm 0.12$ | $45.13 \pm 14.10$  | $675.31 \pm 163.73$  | 64.4          | 57891      |
| 2008 | $0.79 \pm 0.16$ | $138.95 \pm 20.42$ | $453.43 \pm 199.30$  | 175.8         | 49916      |
| 2009 | $1.31 \pm 0.25$ | $71.52 \pm 26.71$  | $890.53 \pm 357.87$  | 54.5          | 49888      |
| 2010 | $0.72 \pm 0.11$ | $81.83 \pm 10.71$  | $443.04 \pm 91.69$   | 112.9         | 51731      |
| 2011 | $1.18 \pm 0.24$ | $72.68 \pm 22.45$  | $1020.11 \pm 297.19$ | 61.5          | 44563      |
| 2012 | $0.48 \pm 0.10$ | $65.21 \pm 9.91$   | $324.49 \pm 88.67$   | 134.9         | 28351      |

### Negative EBITDA

| Year | $T_1$           | $T_{1/2}$          | $T_0$                | $T_{1/2}/T_1$ | Num. Firms |
|------|-----------------|--------------------|----------------------|---------------|------------|
| 2003 | $2.63 \pm 0.74$ | $155.00 \pm 36.85$ | $298.14 \pm 224.55$  | 58.9          | 10229      |
| 2004 | $2.64 \pm 0.78$ | $160.38 \pm 34.72$ | $411.42 \pm 176.90$  | 60.7          | 10911      |
| 2005 | $1.29 \pm 0.39$ | $251.33 \pm 26.71$ | $235.76 \pm 124.70$  | 195.0         | 11138      |
| 2006 | $1.61 \pm 0.52$ | $243.08 \pm 34.10$ | $226.84 \pm 187.29$  | 151.0         | 12030      |
| 2007 | $1.48 \pm 0.56$ | $300.25 \pm 42.72$ | $336.88 \pm 270.06$  | 203.0         | 11926      |
| 2008 | $3.81 \pm 1.32$ | $493.35 \pm 73.72$ | $227.39 \pm 218.65$  | 129.6         | 12089      |
| 2009 | $1.11 \pm 0.60$ | $245.57 \pm 54.63$ | $1177.26 \pm 495.38$ | 221.0         | 17965      |
| 2010 | $3.04 \pm 0.69$ | $129.04 \pm 31.55$ | $698.36 \pm 172.99$  | 42.4          | 23094      |
| 2011 | $5.27 \pm 1.06$ | $179.69 \pm 53.33$ | $961.02 \pm 308.77$  | 34.1          | 20526      |
| 2012 | $2.31 \pm 0.39$ | $146.30 \pm 21.28$ | $384.42 \pm 135.29$  | 63.3          | 14009      |

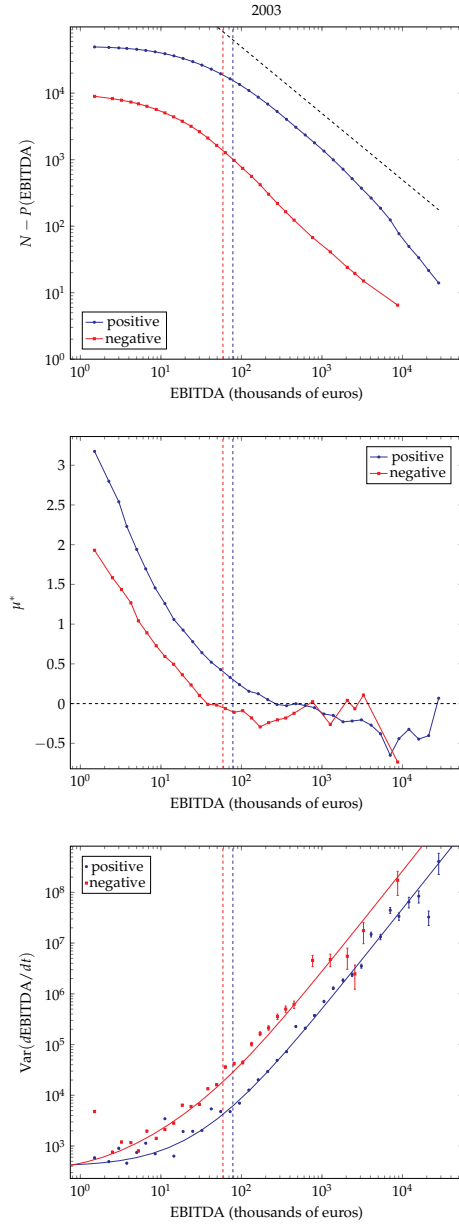

Figure 171: Valencian community

Rank plot, chemical potential and variance.

50870 Firms with positive EBITDA

$T_1 = 0.47 \pm 0.08$ ,  $T_{1/2} = 36.88 \pm 9.27$ , and  $T_0 = 396.90 \pm 104.54$

10229 Firms with negative EBITDA

Negative EBITDA:

$T_1 = 2.63 \pm 0.74$ ,  $T_{1/2} = 155.00 \pm 36.85$ , and  $T_0 = 298.14 \pm 224.55$ .

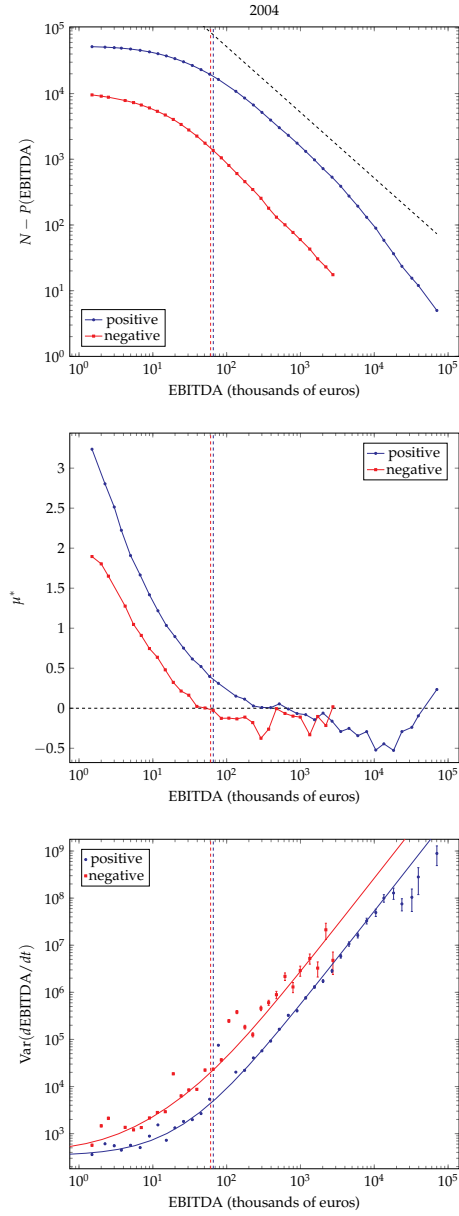

Figure 172: Valencian community

Rank plot, chemical potential and variance.

52966 Firms with positive EBITDA

$T_1 = 0.53 \pm 0.08$ ,  $T_{1/2} = 34.79 \pm 7.77$ , and  $T_0 = 339.74 \pm 84.24$

10911 Firms with negative EBITDA

Negative EBITDA:

$T_1 = 2.64 \pm 0.78$ ,  $T_{1/2} = 160.38 \pm 34.72$ , and  $T_0 = 411.42 \pm 176.90$ .

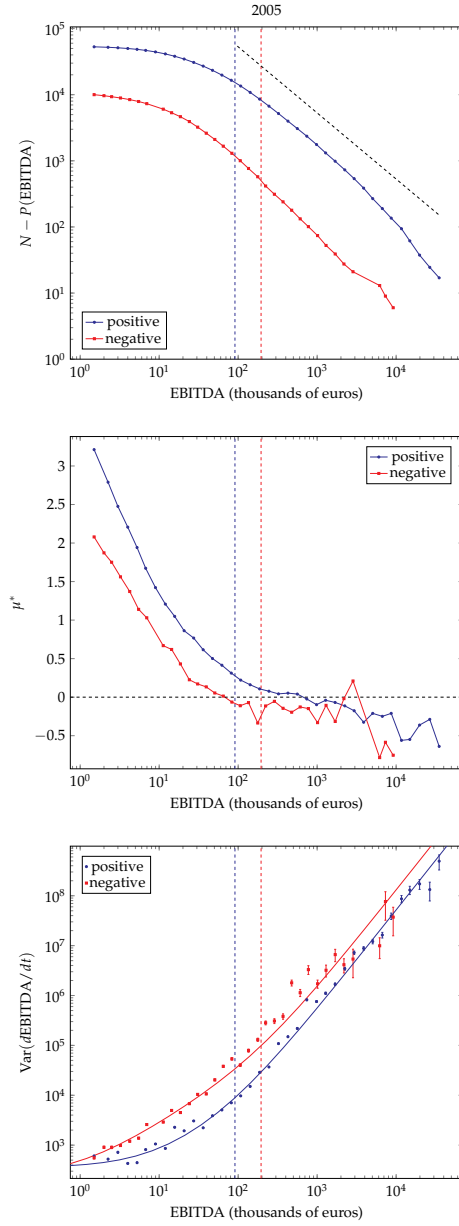

Figure 173: Valencian community

Rank plot, chemical potential and variance.

54255 Firms with positive EBITDA

$T_1 = 0.52 \pm 0.07$ ,  $T_{1/2} = 46.94 \pm 7.09$ , and  $T_0 = 353.35 \pm 64.24$

11138 Firms with negative EBITDA

Negative EBITDA:

$T_1 = 1.29 \pm 0.39$ ,  $T_{1/2} = 251.33 \pm 26.71$ , and  $T_0 = 235.76 \pm 124.70$ .

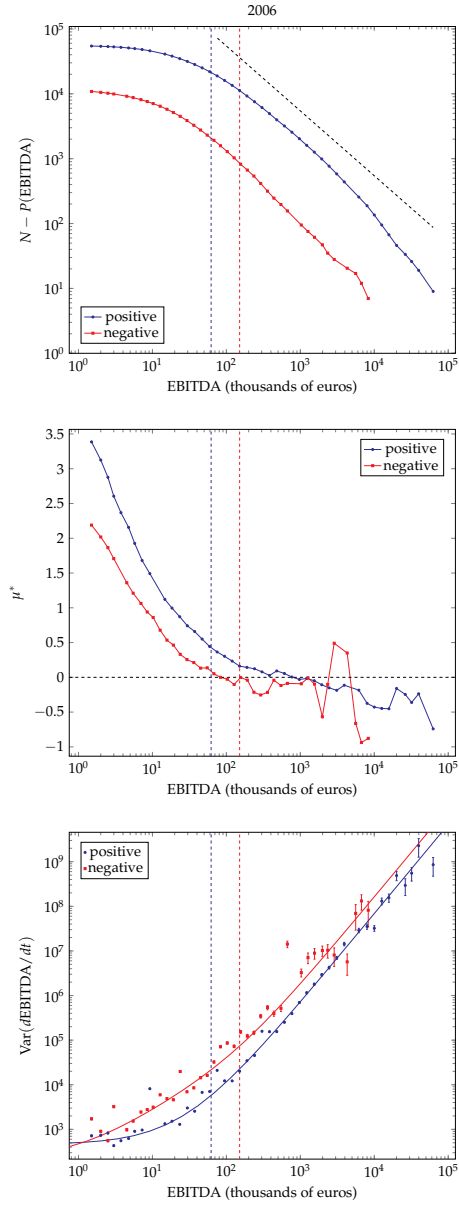

Figure 174: Valencian community

Rank plot, chemical potential and variance.

55714 Firms with positive EBITDA

$T_1 = 0.68 \pm 0.09$ ,  $T_{1/2} = 42.56 \pm 9.73$ , and  $T_0 = 462.03 \pm 110.66$

12030 Firms with negative EBITDA

Negative EBITDA:

$T_1 = 1.61 \pm 0.52$ ,  $T_{1/2} = 243.08 \pm 34.10$ , and  $T_0 = 226.84 \pm 187.29$ .

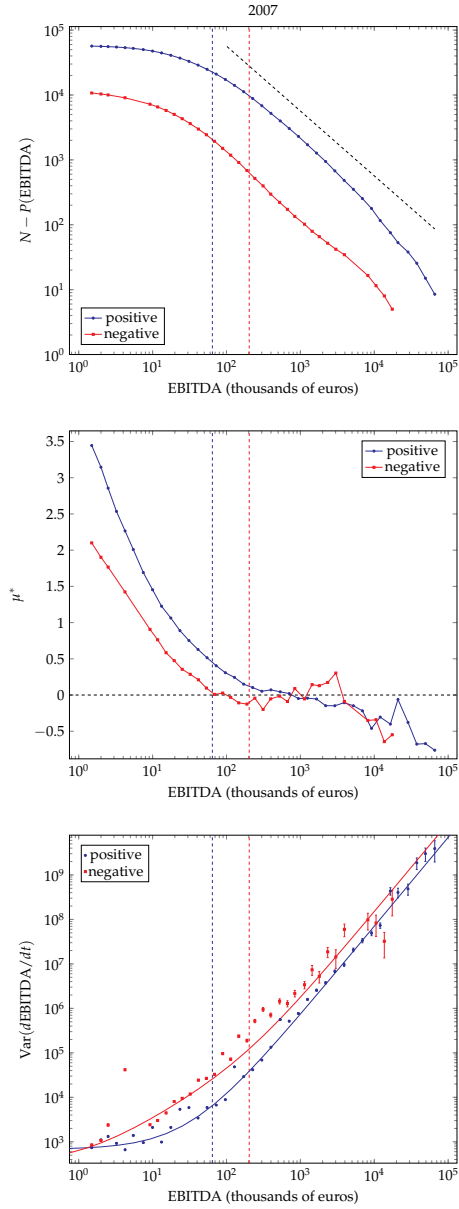

Figure 175: Valencian community

Rank plot, chemical potential and variance.

57891 Firms with positive EBITDA

$T_1 = 0.70 \pm 0.12$ ,  $T_{1/2} = 45.13 \pm 14.10$ , and  $T_0 = 675.31 \pm 163.73$

11926 Firms with negative EBITDA

Negative EBITDA:

$T_1 = 1.48 \pm 0.56$ ,  $T_{1/2} = 300.25 \pm 42.72$ , and  $T_0 = 336.88 \pm 270.06$ .

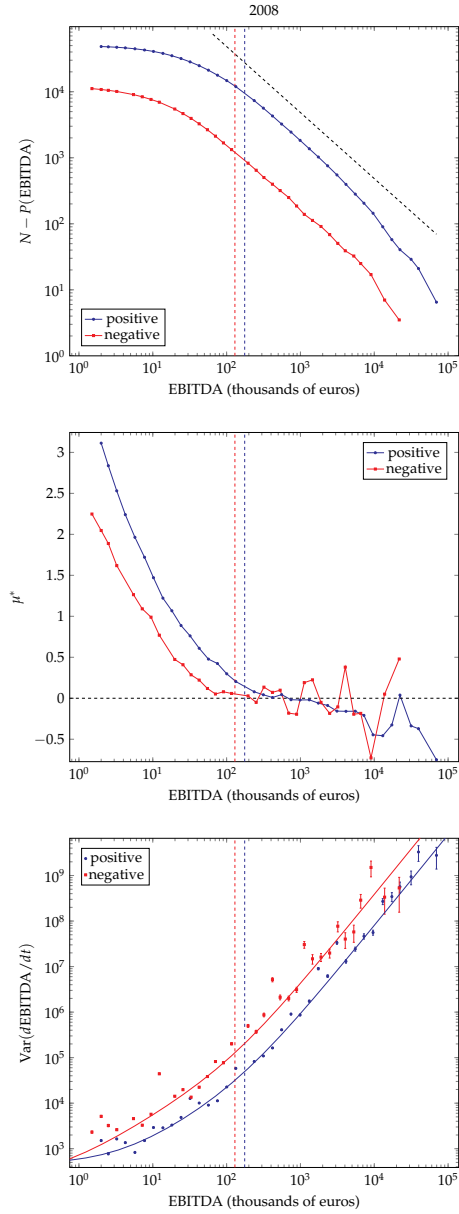

Figure 176: Valencian community

Rank plot, chemical potential and variance.

49916 Firms with positive EBITDA

$T_1 = 0.79 \pm 0.16$ ,  $T_{1/2} = 138.95 \pm 20.42$ , and  $T_0 = 453.43 \pm 199.30$

12089 Firms with negative EBITDA

Negative EBITDA:

$T_1 = 3.81 \pm 1.32$ ,  $T_{1/2} = 493.35 \pm 73.72$ , and  $T_0 = 227.39 \pm 218.65$ .

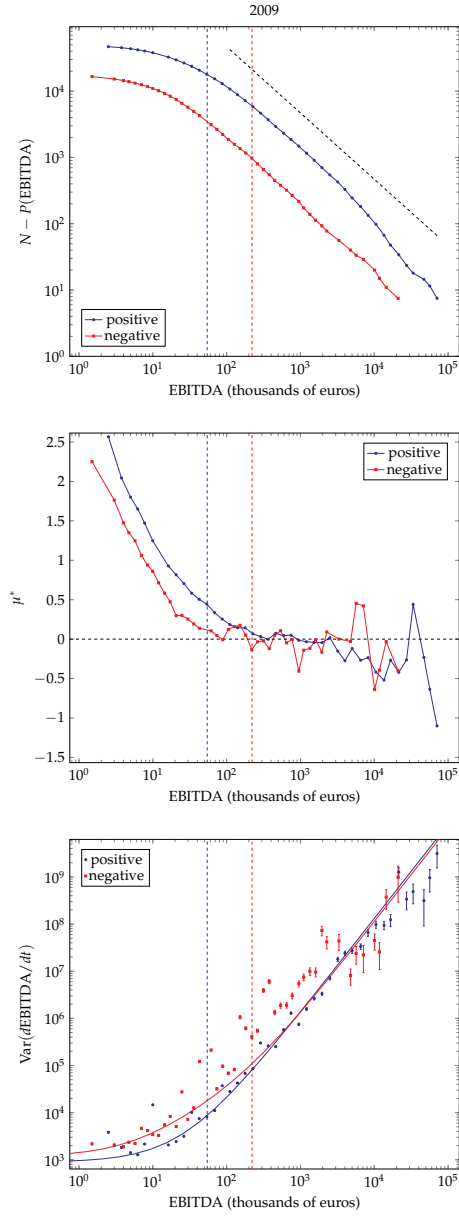

Figure 177: Valencian community

Rank plot, chemical potential and variance.

49888 Firms with positive EBITDA

$T_1 = 1.31 \pm 0.25$ ,  $T_{1/2} = 71.52 \pm 26.71$ , and  $T_0 = 890.53 \pm 357.87$

17965 Firms with negative EBITDA

Negative EBITDA:

$T_1 = 1.11 \pm 0.60$ ,  $T_{1/2} = 245.57 \pm 54.63$ , and  $T_0 = 1177.26 \pm 495.38$ .

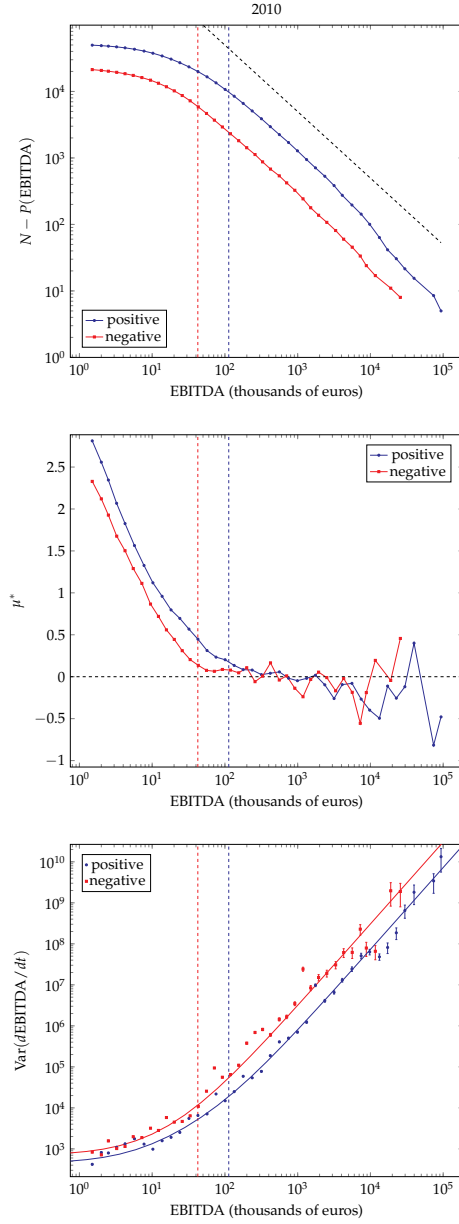

Figure 178: Valencian community

Rank plot, chemical potential and variance.

51731 Firms with positive EBITDA

$T_1 = 0.72 \pm 0.11$ ,  $T_{1/2} = 81.83 \pm 10.71$ , and  $T_0 = 443.04 \pm 91.69$

23094 Firms with negative EBITDA

Negative EBITDA:

$T_1 = 3.04 \pm 0.69$ ,  $T_{1/2} = 129.04 \pm 31.55$ , and  $T_0 = 698.36 \pm 172.99$ .

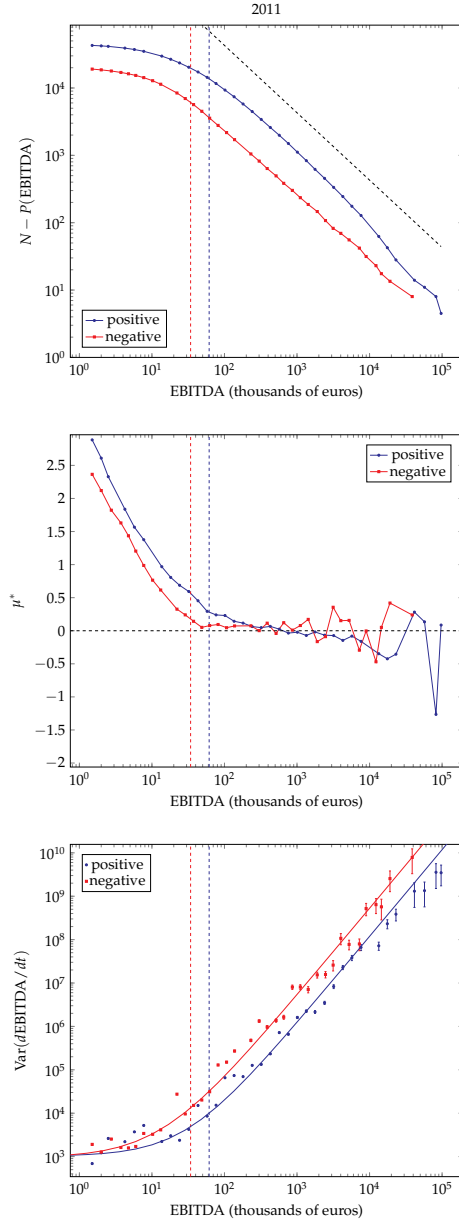

Figure 179: Valencian community

Rank plot, chemical potential and variance.

44563 Firms with positive EBITDA

$T_1 = 1.18 \pm 0.24$ ,  $T_{1/2} = 72.68 \pm 22.45$ , and  $T_0 = 1020.11 \pm 297.19$

20526 Firms with negative EBITDA

Negative EBITDA:

$T_1 = 5.27 \pm 1.06$ ,  $T_{1/2} = 179.69 \pm 53.33$ , and  $T_0 = 961.02 \pm 308.77$ .

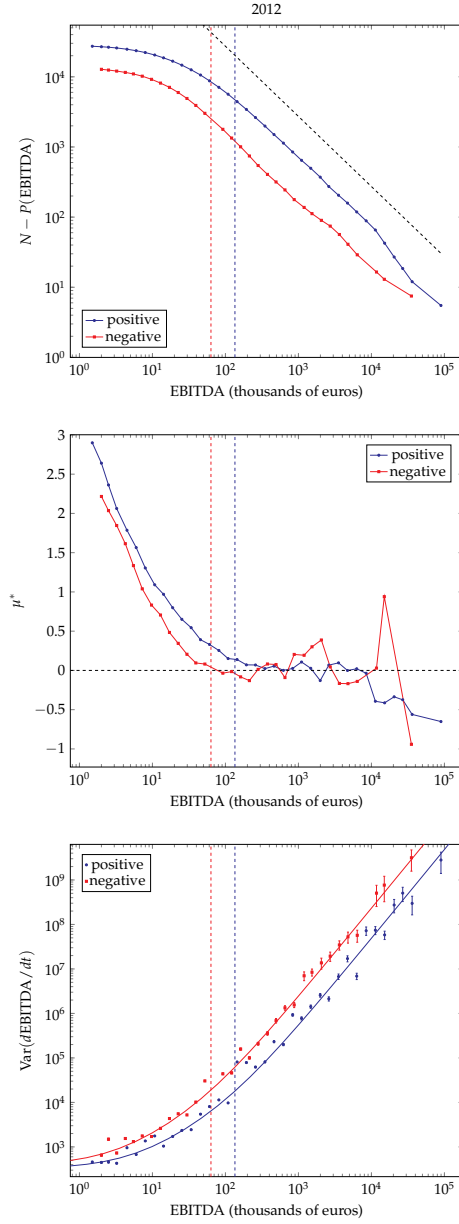

Figure 180: Valencian community

Rank plot, chemical potential and variance.

28351 Firms with positive EBITDA

$T_1 = 0.48 \pm 0.10$ ,  $T_{1/2} = 65.21 \pm 9.91$ , and  $T_0 = 324.49 \pm 88.67$

14009 Firms with negative EBITDA

Negative EBITDA:

$T_1 = 2.31 \pm 0.39$ ,  $T_{1/2} = 146.30 \pm 21.28$ , and  $T_0 = 384.42 \pm 135.29$ .
